# Supplementary material for: Reductions in Higher-Order Rewriting and Their Equivalence
Source: arXiv:2210.15654 source file (2023-08-15)
Supplement: Supplementary file 1 [file a01-terms_and_rewrites.tex]

\begin{defi}[Notions of contexts]
\ldef{notions_of_contexts}
\quad
\begin{enumerate}
\item
  A {\em rewrite context} is a rewrite $\rctx$
  with a single free occurrence of a distinguished variable $\ctxhole$
  called the {\em hole}. Inductively, rewrite contexts are given by
  the grammar:
  \[
    \rctx ::= \ctxhole
         \mid \lam{\var}{\rctx}
         \mid \rctx\,\redseq
         \mid \redseq\,\rctx
         \mid \rctx\seq\redseq
         \mid \redseq\seq\rctx
  \]
  The capturing substitution of the hole of a rewrite context $\rctx$
  by the rewrite $\redseq$
  is a rewrite, written as $\rctxof{\redseq}$.
\item
  The set of {\em composition contexts} is a subset of the set
  of rewrite contexts, given by the grammar:
  \[
    \sctx ::= \ctxhole
         \mid \sctx\seq\redseq
         \mid \redseq\seq\sctx
  \]
\item
  The set of {\em composition trees} is given by
  the grammar:
  \[
    \kctx ::= \ctxhole
         \mid \kctx\seq\kctx
  \]
  For each $n \geq 1$, an {\em $n$-hole composition tree}
  is a composition tree with $n$ occurrences of the {\em hole} $\ctxhole$.
  If $\kctx$ is an $n$-hole composition tree,
  we write $\kctxof{\redseq_1,\hdots,\redseq_n}$ to stand for the
  rewrite that results from replacing the $i$-th hole of $\kctx$ for $\redseq_i$
  for each $1 \leq i \leq n$.
  \smallskip\\
  For example $((\ctxhole\seq\ctxhole)\seq\ctxhole)$ is a 3-hole
  composition tree and
  $((\ctxhole\seq\ctxhole)\seq\ctxhole)\ctxof{\redseq,\redseqtwo,\redseqthree} =
   (\redseq\seq\redseqtwo)\seq\redseqthree$.
\item
  A rewrite context $\rctx$ is {\em applicative}
  if it is of the form $\rctx = \rctx'\ctxof{\sctxof{\ctxhole}\,\redseq}$.
\end{enumerate}
\end{defi}

\begin{lem}[Source/target decomposition]
\llem{source_target_contextual_decomposition}
Define the source and the target of a context $\rctx$
by declaring $\rsrc{\ctxhole} = \ctxhole$ and $\rtgt{\ctxhole} = \ctxhole$.
Let us write $\rendpoint{-}$
to stand for either $\rsrc{-}$ or $\rtgt{-}$.
If $\rendpoint{\redseq} = \cctxof{\tm}$ then there are two possibilities:
\begin{itemize}
\item[(A)]
  $\redseq = \rctxof{\iredseq}$
  where $\rendpoint{\rctx} = \cctx$
  and $\iredseq$ is a rewrite such that $\rendpoint{\iredseq} = \tm$.
\item[(B)]
  $\redseq = \rctxof{\rulewit}$
  where $\rendpoint{\rctx} = \cctx_1$
  and $\rulewit$ is a rule symbol such that
  $\rendpoint{\rulewit} = \cctx_2\ctxof{\tm}$
  and $\cctx = \cctx_1\ctxof{\cctx_2}$.
\end{itemize}
\end{lem}
\begin{proof}
We prove the property for the source; the proof for the target is similar.
We proceed by induction on $\redseq$:
\begin{enumerate}
\item {\bf Variable, $\redseq = \var$.}
  Then $\rsrc{\var} = \var = \cctxof{\tm}$
  so $\cctx = \ctxhole$ and $\tm = \var$.
  Taking $\rctx = \ctxhole$ and $\iredseq = \var$
  we are in situation (A).
\item {\bf Constant, $\redseq = \cons$.}
  Similar to the previous case.
\item {\bf Rule symbol, $\redseq = \rulewit$.}
  Then $\rsrc{\rulewit} = \cctxof{\tm}$.
  Taking $\rctx = \ctxhole$ we are in situation (B).
\item {\bf Abstraction, $\redseq = \lam{\var}{\redseqtwo}$.}
  Then $\lam{\var}{\rsrc{\redseqtwo}} = \cctxof{\tm}$.
  If $\cctx$ is empty, taking $\rctx = \ctxhole$ and
  $\iredseq = \lam{\var}{\redseqtwo}$ we are in situation (A).
  If $\cctx$ is non-empty, then $\cctx = \lam{\var}{\cctx'}$
  and $\redseqtwo = \cctx'\ctxof{\tm}$.
  By \ih there are two possibilities:
  \begin{enumerate}
  \item[(A)]
    $\redseqtwo = \rctx'\ctxof{\iredseq}$ where
    $\rsrc{\rctx'} = \cctx'$ and $\rsrc{\iredseq} = \tm$.
    Taking $\rctx := \lam{\var}{\rctx'}$ we are again in situation (A).
  \item[(B)]
    $\redseqtwo = \rctx'\ctxof{\rulewit}$ where
    $\rsrc{\rctx'} = \cctx'_1$ and $\rsrc{\rulewit} = \cctx_2\ctxof{\tm}$
    such that $\cctx' = \cctx'_1\ctxof{\cctx_2}$.
    Taking $\rctx := \lam{\var}{\rctx'}$ we are again in situation (B).
  \end{enumerate}
\item {\bf Application, $\redseq = \redseq_1\,\redseq_2$.}
  Then $\rsrc{\redseq_1}\rsrc{\redseq_2} = \cctxof{\tm}$.
  If $\cctx$ is empty,
  taking $\rctx = \ctxhole$ and $\iredseq = \redseq_1\,\redseq_2$
  we are in situation (A).
  If $\cctx$ is non-empty, there are two cases, depending on whether
  the hole is to the left or to the right of the application:
  \begin{enumerate}
  \item {\bf Left of the application.}
    Then $\cctx = \cctx'\,\rsrc{\redseq_2}$
    and $\rsrc{\redseq_1} = \cctx'\ctxof{\tm}$.
    Then by \ih there are two possibilities:
    \begin{itemize}
    \item[(A)]
      $\redseq_1 = \rctx'\ctxof{\iredseq}$
      with $\rsrc{\rctx'} = \cctx'$ and $\rsrc{\iredseq} = \tm$.
      Taking $\rctx = \rctx'\,\redseq_2$ we are again in situation~(A).
    \item[(B)]
      $\redseq_1 = \rctx'\ctxof{\rulewit}$
      with $\rsrc{\rctx'} = \cctx'_1$
      and $\rsrc{\rulewit} = \cctx_2\ctxof{\tm}$
      such that $\cctx' = \cctx'_1\ctxof{\cctx_2}$.
      Taking $\rctx = \rctx'\,\redseq_2$ we are again in situation (B).
    \end{itemize}
  \item {\bf Right of the application.}
    Then $\cctx = \rsrc{\redseq_1}\,\cctx'$.
    The proof is similar to the previous case.
  \end{enumerate}
\item {\bf Composition, $\redseq = \redseq_1\seq\redseq_2$.}
  Then $\rsrc{\redseq_1} = \cctxof{\tm}$.
  By \ih on $\redseq_1$ there are two possibilities:
  \begin{itemize}
  \item[(A)]
    $\redseq_1 = \rctx'\ctxof{\iredseq}$
    with $\rsrc{\rctx'} = \cctx$ and $\rsrc{\iredseq} = \tm$.
    Taking $\rctx := \rctx'\seq\redseq_2$
    we are again in situation (A).
  \item[(B)]
    $\redseq_1 = \rctx'\ctxof{\rulewit}$
    with $\rsrc{\rctx'} = \cctx_1$ and $\rsrc{\rulewit} = \cctx_2\ctxof{\tm}$
    such that $\cctx = \cctx_1\ctxof{\cctx_2}$.
    Taking $\rctx := \rctx'\seq\redseq_2$
    we are again in situation (B).
  \end{itemize}
\end{enumerate}
\end{proof}

We formulate a variant of the standard substitution lemma:
\begin{lem}[Substitution Lemma]
\llem{substitution_lemma}
The equation
$
  X\subt{\var}{\tm}\subt{\vartwo}{\tmtwo}
  =
  X\subt{\vartwo}{\tmtwo}\subt{\var}{\tm\subt{\vartwo}{\tmtwo}}
$
holds for any term or rewrite $X$
as long as $\var \neq \vartwo$ and $\var \notin \fv{\tmtwo}$.
\end{lem}
\begin{proof}
By induction on $X$.
\end{proof}

\begin{lem}[Weakening]
\llem{weakening}
Let $\var \notin \tenv$. Then:
\begin{enumerate}
\item
  If $\judgTerm{\tenv}{\tm}{\typ}$
  then $\judgTerm{\tenv,\var:\typtwo}{\tm}{\typ}$.
\item
  If $\judgTermEq{\tenv}{\tm}{\tmtwo}{\typ}$
  then $\judgTermEq{\tenv,\var:\typtwo}{\tm}{\tmtwo}{\typ}$.
\item
  If $\judgRewr{\tenv}{\redseq}{\tm}{\tmtwo}{\typ}$
  then $\judgRewr{\tenv,\var:\typtwo}{\redseq}{\tm}{\tmtwo}{\typ}$.
\end{enumerate}
\end{lem}
\begin{proof}
Straightfoward by induction on the derivation of the target judgment.
\end{proof}

\begin{lem}[Endpoint coherence]
\llem{endpoint:coherence}
Let $\judgRewr{\tenv}{\redseq}{\tmfour_0}{\tmfour_1}{\typ}$.
Then $\judgTermEq{\tenv}{\tmfour_0}{\rsrc{\redseq}}{\typ}$
and $\judgTermEq{\tenv}{\tmfour_0}{\rtgt{\redseq}}{\typ}$.
\end{lem}
\begin{proof}
By induction on the derivation of
$\judgRewr{\tenv}{\redseq}{\tmfour_0}{\tmfour_1}{\typ}$.
\begin{enumerate}
\item \indrulename{RVar}, \indrulename{RCon}:
  Immediate by \indrulename{EqRefl}.
\item \indrulename{RRule}:
  Let
    $\judgRewr{\tenv}{\rulewit}{\tm}{\tmtwo}{\typ}$
  be derived from
    $\judgTerm{\noenv}{\tm}{\typ}$
  and
    $\judgTerm{\noenv}{\tmtwo}{\typ}$
  where $(\rewr{\rulewit}{\tm}{\tmtwo}{\typ})\in\ruleset$.
  Then by weakening~\rlem{weakening}
  we have that $\judgTerm{\tenv}{\tm}{\typ}$
  and $\judgTerm{\tenv}{\tmtwo}{\typ}$.
  Applying \indrulename{EqRefl} we have that
  $\judgTermEq{\tenv}{\tm}{\tm}{\typ}$
  and $\judgTermEq{\tenv}{\tmtwo}{\tmtwo}{\typ}$,
  as required.
\item \indrulename{RAbs}:
  Straightforward by \ih.
  More precisely, let
    $\judgRewr{\tenv}{
      \lam{\var}{\redseq}
    }{
      \lam{\var}{\tm_0}
    }{
      \lam{\var}{\tm_1}
    }{\typ \imp \typtwo}$
  be derived from
    $\judgRewr{\tenv,\var:\typ}{
      \redseq
    }{
      \tm_0
    }{
      \tm_1
    }{\typtwo}$.
  By \ih we have that
  $\judgTermEq{\tenv,\var:\typ}{\tm_0}{\rsrc{\redseq}}{\typtwo}$ 
  and $\judgTermEq{\tenv,\var:\typ}{\tm_1}{\rtgt{\redseq}}{\typtwo}$.
  Applying \indrulename{EqCongLam} 
  we have that
  $\judgTermEq{\tenv}{
     \lam{\var}{\tm_0}
   }{
     \lam{\var}{\rsrc{\redseq}}
   }{\typ \imp \typtwo}$ 
  and
  $\judgTermEq{\tenv}{
     \lam{\var}{\tm_1}
   }{
     \lam{\var}{\rtgt{\redseq}}
   }{\typ \imp \typtwo}$ 
  as required.
\item \indrulename{RApp}:
  Straightforward by \ih, using \indrulename{EqCongApp}.
\item \indrulename{RTrans}:
  Let
    $\judgRewr{\tenv}{
      \redseq\seq\redseqtwo
    }{
      \tm_0
    }{
      \tm_2
    }{
      \typ
    }$
  be derived from
    $\judgRewr{\tenv}{
      \redseq
    }{
      \tm_0
    }{
      \tm_1
    }{
      \typ
    }$
  and
    $\judgRewr{\tenv}{
      \redseqtwo
    }{
      \tm_1
    }{
      \tm_2
    }{
      \typ
    }$.
  By \ih we have that
  $\judgTermEq{\tenv}{\tm_0}{\rsrc{\redseq}}{\typ}$
  and
  $\judgTermEq{\tenv}{\tm_2}{\rtgt{\redseqtwo}}{\typ}$.
  Hence
  $\judgTermEq{\tenv}{\tm_0}{\rsrc{(\redseq\seq\redseqtwo)}}{\typ}$
  and
  $\judgTermEq{\tenv}{\tm_2}{\rtgt{(\redseq\seq\redseqtwo)}}{\typ}$.
\item \indrulename{RConv}:
  Let
    $\judgRewr{\tenv}{
      \redseq
    }{
      \tm
    }{
      \tmtwo
    }{
      \typ
    }$
  be derived from
    $\judgRewr{\tenv}{
      \redseq
    }{
      \tm'
    }{
      \tmtwo'
    }{
      \typ
    }$
  where
    $\judgTermEq{\tenv}{\tm}{\tm'}{\typ}$
  and
    $\judgTermEq{\tenv}{\tmtwo'}{\tmtwo}{\typ}$.
  By \ih we have that 
    $\judgTermEq{\tenv}{\tm'}{\rsrc{\redseq}}{\typ}$
  and
    $\judgTermEq{\tenv}{\tmtwo'}{\rtgt{\redseq}}{\typ}$,
  so applying \indrulename{EqTrans} we have that
    $\judgTermEq{\tenv}{\tm}{\rsrc{\redseq}}{\typ}$
  and
    $\judgTermEq{\tenv}{\tmtwo}{\rtgt{\redseq}}{\typ}$,
  as required.
\end{enumerate}
\end{proof}

\begin{lem}[Strengthening]
\llem{strengthening}
Let $\var \notin \fv{\tm}$.
If $\judgTerm{\tenv,\var:\typ}{\tm}{\typtwo}$
then $\judgTerm{\tenv}{\tm}{\typtwo}$.
\end{lem}
\begin{proof}
Straightfoward by induction on the derivation of the target judgment.
\end{proof}

\begin{lem}[Free variables must be typed]
\llem{free_variables_typed}
\quad
\begin{enumerate}
\item
  If $\judgTerm{\tenv}{\tm}{\typ}$
  then $\fv{\tm} \subseteq \dom{\tenv}$.
\item
  If $\judgRewr{\tenv}{\redseq}{\tm}{\tmtwo}{\typ}$
  then $\fv{\redseq} \cup \fv{\tm} \cup \fv{\tmtwo} \subseteq \dom{\tenv}$.
\end{enumerate}
\end{lem}
\begin{proof}
Straightfoward by induction on the derivation of the judgment.
\end{proof}

\begin{lem}[Free term variables of endpoints]
\llem{free_variables_of_endpoints}
Let $\judgRewr{\tenv}{\redseq}{\tm}{\tmtwo}{\typ}$.
Then $\fvt{\tm},\fvt{\tmtwo} \subseteq \fvt{\redseq}$.
\end{lem}
\begin{proof}
Straightforward by induction on the derivation of
$\judgRewr{\tenv}{\redseq}{\tm}{\tmtwo}{\typ}$.
In the \indrulename{RRule} case, note that
$\judgRewr{\tenv}{\rulewit}{\tm}{\tmtwo}{\typ}$
is derived from $\judgTerm{\noenv}{\tm}{\typ}$
and $\judgTerm{\noenv}{\tmtwo}{\typ}$
so by \rlem{free_variables_typed}
we have that $\tm,\tmtwo$ are closed terms.
\end{proof}

\begin{lem}[Reflexivity]
\llem{reflexivity}
If $\judgTerm{\tenv}{\tm}{\typ}$
then $\judgRewr{\tenv}{\refl{\tm}}{\tm}{\tm}{\typ}$.
\end{lem}
\begin{proof}
Straightforward by induction on the derivation of the judgment.
\end{proof}

\begin{lem}[Substitution]
\llem{substitution_term_variables}
Let $\judgTerm{\tenv}{\tmfive}{\typ}$. Then:
\begin{enumerate}
\item
  If $\judgTerm{\tenv,\var:\typ}{\tm}{\typtwo}$
  then $\judgTerm{\tenv}{\tm\subt{\var}{\tmfive}}{\typtwo}$.
\item
  If $\judgTermEq{\tenv,\var:\typ}{\tm}{\tmtwo}{\typtwo}$
  then $\judgTermEq{\tenv}{\tm\subt{\var}{\tmfive}}{\tmtwo\subt{\var}{\tmfive}}{\typtwo}$.
\item
  If $\judgRewr{\tenv,\var:\typ}{\redseq}{\tm}{\tmtwo}{\typtwo}$
  then $\judgRewr{\tenv}{\redseq\subt{\var}{\tmfive}}{\tm\subt{\var}{\tmfive}}{\tmtwo\subt{\var}{\tmfive}}{\typtwo}$.
\end{enumerate}
\end{lem}
\begin{proof}
Each item is by induction on the derivation of the target judgment:
\begin{enumerate}
\item
  \indrulename{Var}, \indrulename{Con}: immediate.
\item
  \indrulename{Abs}:
  let $\judgTerm{\tenv,\var:\typ}{\lam{\vartwo}{\tm}}{\typtwo \imp \typthree}$
  be derived from
  $\judgTerm{\tenv,\var:\typ,\vartwo:\typtwo}{\tm}{\typthree}$.
  Note that the hypothesis $\judgTerm{\tenv}{\tmfive}{\typ}$
  may be weakened to
  $\judgTerm{\tenv,\vartwo:\typtwo}{\tmfive}{\typ}$.
  using \rlem{weakening}.
  Hence we may apply the \ih to obtain
  $\judgTerm{\tenv,\vartwo:\typtwo}{\tm\subt{\var}{\tmfive}}{\typthree}$.
  Applying the \indrulename{Abs} rule
  $\judgTerm{\tenv}{
     \lam{\var}{\tm\subt{\var}{\tmfive}}
   }{\typtwo \imp \typthree}$.
\item
  \indrulename{App}:
  let $\judgTerm{\tenv,\var:\typ}{\tm\,\tmtwo}{\typthree}$
  be derived from
  $\judgTerm{\tenv,\var:\typ}{\tm}{\typtwo \imp \typthree}$
  and
  $\judgTerm{\tenv,\var:\typ}{\tmtwo}{\typtwo}$.
  By \ih
  $\judgTerm{\tenv}{\tm\subt{\var}{\tmfive}}{\typtwo \imp \typthree}$
  and
  $\judgTerm{\tenv}{\tmtwo\subt{\var}{\tmfive}}{\typtwo}$.
  Applying the \indrulename{App} rule,
  $\judgTerm{\tenv}{\tm\subt{\var}{\tmfive}\,\tmtwo\subt{\var}{\tmfive}}{\typthree}$.
\item
  \indrulename{EqBeta}:
  let
    $\judgTermEq{\tenv,\var:\typ}{(\lam{\vartwo}{\tm})\,\tmtwo}{\tm\subt{\vartwo}{\tmtwo}}{\typthree}$
  be derived from
    $\judgTerm{\tenv,\var:\typ,\vartwo:\typtwo}{\tm}{\typthree}$
  and
    $\judgTerm{\tenv,\var:\typ}{\tmtwo}{\typtwo}$.
  By the first item of this lemma,
    $\judgTerm{\tenv,\vartwo:\typtwo}{\tm\subt{\var}{\tmfive}}{\typthree}$
  and
    $\judgTerm{\tenv}{\tmtwo\subt{\var}{\tmfive}}{\typtwo}$,
  so applying the \indrulename{EqBeta} rule we have that
    $\judgTermEq{\tenv}{
       ((\lam{\vartwo}{\tm})\,\tmtwo)\subt{\var}{\tmfive}
     }{
       \tm\subt{\var}{\tmfive}\subt{\vartwo}{\tmtwo\subt{\var}{\tmfive}}
     }{\typthree}$.
  Moreover, by the Substitution Lemma~(\rlem{substitution_lemma}),
  $\tm\subt{\var}{\tmfive}\subt{\vartwo}{\tmtwo\subt{\var}{\tmfive}}
   =
   \tm\subt{\vartwo}{\tmtwo}\subt{\var}{\tmfive}$
  so we are done.
\item
  \indrulename{EqEta}:
  let
    $\judgTermEq{\tenv,\var:\typ}{\lam{\vartwo}{\tm\,\vartwo}}{\tm}{\typthree}$
  be derived from
    $\judgTerm{\tenv,\var:\typ,\vartwo:\typtwo}{\tm}{\typthree}$
  with $\vartwo\notin\fv{\tm}$.
  By the first item of this lemma,
    $\judgTerm{\tenv,\vartwo:\typtwo}{\tm\subt{\var}{\tmfive}}{\typthree}$.
  Note that by Barendregt's convention, we may assume that
  $\vartwo \notin \fv{\tmfive}$,
  hence $\vartwo \notin \fv{\tm\subt{\var}{\tmfive}}$,
  and we may apply the \indrulename{EqEta} rule to conclude
    $\judgTermEq{\tenv,\vartwo:\typtwo}{\lam{\vartwo}{\tm\subt{\var}{\tmfive}\,\vartwo}}{\tm\subt{\var}{\tmfive}}{\typthree}$.
\item
  \indrulename{EqRefl}, \indrulename{EqSym}, \indrulename{EqTrans},
  \indrulename{EqCongLam}, \indrulename{EqCongApp}:
  straightforward by \ih.
\item
  \indrulename{RVar}:
  let
    $\judgRewr{\tenv,\var:\typ}{\vartwo}{\vartwo}{\vartwo}{\typtwo}$
  with $(\vartwo:\typtwo) \in (\tenv,\var:\typ)$.
  There are two cases, depending on whether $\var = \vartwo$ or not.
  If $\var = \vartwo$, then
  by reflexivity (\rlem{reflexivity})
  we have that
  $\judgRewr{\tenv}{\tmfive}{\tmfive}{\tmfive}{\typtwo}$.
  If $\var \neq \vartwo$ then $\tenv = \tenv',\vartwo:\typtwo$.
  and applying the \indrulename{RVar} rule
  $\judgRewr{\tenv',\vartwo:\typtwo}{\vartwo}{\vartwo}{\vartwo}{\typtwo}$.
\item
  \indrulename{RCon}:
  let $\judgRewr{\tenv,\var:\typ}{\cons}{\cons}{\cons}{\typtwo}$
  with $(\cons:\typtwo) \in \constantset$.
  Applying the \indrulename{RCon} rule,
  we have that $\judgRewr{\tenv}{\cons}{\cons}{\cons}{\typtwo}$.
\item
  \indrulename{RRule}:
  let
  $\judgRewr{\tenv,\var:\typ}{\rulewit}{\tm}{\tmtwo}{\typtwo}$
  be derived from
  $\judgTerm{\noenv}{\tm}{\typtwo}$
  and $\judgTerm{\noenv}{\tmtwo}{\typtwo}$
  where
  $(\rewr{\rulewit}{\tm}{\tmtwo}{\typtwo})\in\ruleset$.
  Note that, by \rlem{free_variables_typed},
  we have that
  $\redseq$, $\tm$ and $\tmtwo$ have no free occurrences of $\var$.
  Applying the \indrulename{RRule} rule on the (unchanged) premises,
  we have that
  $\judgRewr{\tenv}{\rulewit}{\tm}{\tmtwo}{\typtwo}$,
  that is
  $\judgRewr{\tenv}{\rulewit}{\tm\subt{\var}{\tmfive}}{\tmtwo\subt{\var}{\tmfive}}{\typtwo}$,
  as required.
\item
  \indrulename{RAbs}, \indrulename{RApp}:
  similar to the
  \indrulename{Abs} and \indrulename{App}
  cases respectively.
\item
  \indrulename{RTrans}:
  Let
  $\judgRewr{\tenv,\var:\typ}{
    \redseq\seq\redseqtwo
  }{
    \tm_0
  }{
    \tm_2
  }{
    \typtwo
  }$
  be derived from
  $\judgRewr{\tenv,\var:\typ}{
    \redseq
  }{
    \tm_0
  }{
    \tm_1
  }{
    \typtwo
  }$
  and
  $\judgRewr{\tenv,\var:\typ}{
    \redseqtwo
  }{
    \tm_1
  }{
    \tm_2
  }{
    \typtwo
  }$.
  Then by \ih
  $\judgRewr{\tenv}{
    \redseq\subt{\var}{\tmfive}
  }{
    \tm_0\subt{\var}{\tmfive}
  }{
    \tm_1\subt{\var}{\tmfive}
  }{
    \typtwo
  }$
  and
  $\judgRewr{\tenv}{
    \redseqtwo\subt{\var}{\tmfive}
  }{
    \tm_1\subt{\var}{\tmfive}
  }{
    \tm_2\subt{\var}{\tmfive}
  }{
    \typtwo
  }$.
  Applying the \indrulename{RTrans} rule,
  $\judgRewr{\tenv}{
    \redseq\subt{\var}{\tmfive}\seq\redseqtwo\subt{\var}{\tmfive}
  }{
    \tm_0\subt{\var}{\tmfive}
  }{
    \tm_2\subt{\var}{\tmfive}
  }{
    \typtwo
  }$
\item
  \indrulename{RConv}:
  Let
    $\judgRewr{\tenv,\var:\typ}{
      \redseq
    }{
      \tm
    }{
      \tmtwo
    }{
      \typtwo
    }$
  be derived from
    $\judgRewr{\tenv,\var:\typ}{
      \redseq
    }{
      \tm'
    }{
      \tmtwo'
    }{
      \typtwo
    }$,
  where
    $\judgTermEq{\tenv,\var:\typ}{\tm}{\tm'}{\typtwo}$
  and
    $\judgTermEq{\tenv,\var:\typ}{\tmtwo'}{\tmtwo}{\typtwo}$.
  Then by \ih
    $\judgRewr{\tenv}{
      \redseq\subt{\var}{\tmfive}
    }{
      \tm'\subt{\var}{\tmfive}
    }{
      \tmtwo'\subt{\var}{\tmfive}
    }{
      \typtwo
    }$.
  Moreover, by the second item of this lemma,
  we have that
    $\judgTermEq{\tenv}{\tm\subt{\var}{\tmfive}}{\tm'\subt{\var}{\tmfive}}{\typtwo}$
  and
    $\judgTermEq{\tenv}{\tmtwo'\subt{\var}{\tmfive}}{\tmtwo\subt{\var}{\tmfive}}{\typtwo}$.
  Applying the \indrulename{RConv} rule,
    $\judgRewr{\tenv}{
      \redseq\subt{\var}{\tmfive}
    }{
      \tm\subt{\var}{\tmfive}
    }{
      \tmtwo\subt{\var}{\tmfive}
    }{
      \typtwo
    }$.
\end{enumerate}
\end{proof}

\begin{lem}[Equal terms are typable]
\llem{equal_terms_are_typable}
If $\judgTermEq{\tenv}{\tm}{\tmtwo}{\typ}$
then $\judgTerm{\tenv}{\tm}{\typ}$
and $\judgTerm{\tenv}{\tmtwo}{\typ}$.
\end{lem}
\begin{proof}
By induction on the derivation of $\judgTermEq{\tenv}{\tm}{\tmtwo}{\typ}$.
\begin{enumerate}
\item
  \indrulename{EqBeta}:
  let
    $\judgTermEq{\tenv}{(\lam{\var}{\tm})\,\tmtwo}{\tm\subt{\var}{\tmtwo}}{\typtwo}$
  be derived from
    $\judgTerm{\tenv,\var:\typ}{\tm}{\typtwo}$
  and
    $\judgTerm{\tenv}{\tmtwo}{\typ}$.
  Applying the \indrulename{Abs} and \indrulename{App} rules,
  we have that
  $\judgTerm{\tenv}{(\lam{\var}{\tm})\,\tmtwo}{\typtwo}$.
  Moreover, by \rlem{substitution_term_variables}
  we have that
  $\judgTerm{\tenv}{\tm\subt{\var}{\tmtwo}}{\typtwo}$.
\item
  \indrulename{EqEta}:
  let
    $\judgTermEq{\tenv}{\lam{\var}{\tm\,\var}}{\tm}{\typtwo}$
  be derived from
    $\judgTerm{\tenv,\var:\typ}{\tm}{\typtwo}$
  and $\var\notin\fv{\tm}$.
  Applying the \indrulename{App} and \indrulename{Abs} rules,
  we have that
    $\judgTerm{\tenv}{\lam{\var}{\tm\,\var}}{\typtwo}$.
  Moreover, by \rlem{strengthening}, $\judgTerm{\tenv}{\tm}{\typtwo}$.
\item
  \indrulename{EqRefl}, \indrulename{EqSym}, \indrulename{EqTrans},
  \indrulename{EqCongLam}, \indrulename{EqCongApp}:
  straightforward by \ih.
\end{enumerate}
\end{proof}

\begin{lem}[Source and target inversion]
\llem{source_target_inversion}
If $\judgRewr{\tenv}{\redseq}{\tm}{\tmtwo}{\typ}$
then
$\judgTerm{\tenv}{\tm}{\typ}$
and
$\judgTerm{\tenv}{\tmtwo}{\typ}$.
\end{lem}
\begin{proof}
By induction on the derivation of
$\judgRewr{\tenv}{\redseq}{\tm}{\tmtwo}{\typ}$.
\begin{enumerate}
\item
  \indrulename{RVar}:
  let $\judgRewr{\tenv,\var:\typ}{\var}{\var}{\var}{\typ}$.
  Then indeed $\judgTerm{\tenv,\var:\typ}{\var}{\typ}$.
\item
  \indrulename{RCon}:
  let $\judgRewr{\tenv}{\cons}{\cons}{\cons}{\typ}$
  with $(\cons:\typ) \in \constantset$.
  Then indeed $\judgTerm{\tenv}{\cons}{\typ}$.
\item
  \indrulename{RRule}:
  let
    $\judgRewr{\tenv}{\rulewit}{\tm}{\tmtwo}{\typ}$
  be derived from
    $\judgTerm{\noenv}{\tm}{\typ}$
  and
    $\judgTerm{\noenv}{\tmtwo}{\typ}$
  with $(\rewr{\rulewit}{\tm}{\tmtwo}{\typ})\in\ruleset$.
  Then it suffices to apply
  weakening (\rlem{weakening})
  to conclude.
\item
  \indrulename{RAbs}:
  let
  $\judgRewr{\tenv}{
    \lam{\var}{\redseq}
  }{
    \lam{\var}{\tm_0}
  }{
    \lam{\var}{\tm_1}
  }{\typ \imp \typtwo}$
  be derived from
  $\judgRewr{\tenv,\var:\typ}{
    \redseq
  }{
    \tm_0
  }{
    \tm_1
  }{\typtwo}$.
  Then by \ih the source of the premise is typable, \ie
  $\judgTerm{\tenv,\var:\typ}{\tm_0}{\typtwo}$.
  Appying the \indrulename{Abs} rule we are able to type
  the source of the conclusion, \ie
  $\judgTerm{\tenv}{\lam{\var}{\tm_0}}{\typ \imp \typtwo}$.
  The proof for the target is similar.
\item
  \indrulename{RApp}:
  let 
  $\judgRewr{\tenv}{
     \redseq\,\redseqtwo
   }{
     \tm_0\,\tmtwo_0
   }{
     \tm_1\,\tmtwo_1
   }{\typtwo}$
  be derived from
   $\judgRewr{\tenv}{
      \redseq
    }{
      \tm_0
    }{
      \tm_1
    }{\typ \imp \typtwo}$
  and
   $\judgRewr{\tenv}{
      \redseqtwo
    }{
      \tmtwo_0
    }{
      \tmtwo_1
    }{\typ}$.
  By \ih we have that the sources of the premises are typable,
  \ie
  that $\judgTerm{\tenv}{\tm_0}{\typ \imp \typtwo}$
  and $\judgTerm{\tenv}{\tmtwo_0}{\typ}$.
  Applying the \indrulename{App} rule, we are able to type the source
  of the conclusion, \ie
  $\judgTerm{\tenv}{\tm_0\,\tmtwo_0}{\typ \imp \typtwo}$.
  The proof for the target is similar.
\item
  \indrulename{RTrans}:
  let
   $\judgRewr{\tenv}{
      \redseq\seq\redseqtwo
    }{
      \tm_0
    }{
      \tm_2
    }{
      \typ
    }$
  be derived from
   $\judgRewr{\tenv}{
      \redseq
    }{
      \tm_0
    }{
      \tm_1
    }{
      \typ
    }$
  and
   $\judgRewr{\tenv}{
      \redseqtwo
    }{
      \tm_1
    }{
      \tm_2
    }{
      \typ
    }$.
  By \ih on the first premise,
  we have that $\judgTerm{\tenv}{\tm_0}{\typ}$,
  and by \ih on the second premise,
  we have that $\judgTerm{\tenv}{\tm_2}{\typ}$.
\item
  \indrulename{RConv}:
  let
    $\judgRewr{\tenv}{
      \redseq
    }{
      \tm
    }{
      \tmtwo
    }{
      \typ
    }$
  be derived from
    $\judgRewr{\tenv}{
      \redseq
    }{
      \tm'
    }{
      \tmtwo'
    }{
      \typ
    }$
  with
    $\judgTermEq{\tenv}{\tm}{\tm'}{\typ}$
  and
    $\judgTermEq{\tenv}{\tmtwo'}{\tmtwo}{\typ}$.
  Then by \rlem{equal_terms_are_typable}
  we have that
    $\judgTerm{\tenv}{\tm}{\typ}$
  and
    $\judgTerm{\tenv}{\tmtwo}{\typ}$.
\end{enumerate}
\end{proof}

\subsection{Term/rewrite substitution}

\begin{lem}[Typing rule for term/rewrite substitution]
\llem{fundamental_property_of_term_lifting}
If $\judgTerm{\tenv,\var:\typ}{\tm}{\typtwo}$
and $\judgRewr{\tenv}{\redseq}{\tmfive_0}{\tmfive_1}{\typ}$
then
$\judgRewr{\tenv}{
    \tm\subtr{\var}{\redseq}
  }{
    \tm\subt{\var}{\tmfive_0}
  }{
    \tm\subt{\var}{\tmfive_1}
  }{\typtwo}$.
\end{lem}
\begin{proof}
By induction on the derivation of
$\judgTerm{\tenv,\var:\typ}{\tm}{\typtwo}$:
\begin{enumerate}
\item
  \indrulename{Var}:
  let
    $\judgTerm{\tenv,\var:\typ}{\vartwo}{\typtwo}$
  with
    $\vartwo:\typtwo \in (\tenv,\var:\typ)$.
  We consider two subcases, depending on whether $\var = \vartwo$ or not:
  \begin{enumerate}
  \item
    If $\var = \vartwo$,
    then $\judgRewr{\tenv}{\redseq}{\tm_0}{\tm_1}{\typ}$
    holds by hypothesis.
  \item
    If $\var \neq \vartwo$,
    then note that $\vartwo:\typtwo\in\tenv$
    so $\judgTerm{\tenv}{\vartwo}{\typtwo}$
    and applying the \indrulename{RVar} rule, we have that
    $\judgRewr{\tenv}{\vartwo}{\vartwo}{\vartwo}{\typtwo}$.
  \end{enumerate}
\item
  \indrulename{Con}:
  immediate applying the \indrulename{RCon} rule.
\item
  \indrulename{Abs}:
  let
    $\judgTerm{\tenv,\var:\typ}{\lam{\vartwo}{\tm}}{\typtwo \imp \typthree}$
  be derived from 
    $\judgTerm{\tenv,\var:\typ,\vartwo:\typtwo}{\tm}{\typthree}$.
  By \ih we have that
    $\judgRewr{\tenv,\vartwo:\typtwo}{
       \tm\subtr{\var}{\redseq}
     }{
       \tm\subt{\var}{\tmfive_0}
     }{
       \tm\subt{\var}{\tmfive_1}
     }{\typthree}$.
  Applying the \indrulename{RAbs} rule, we obtain
    $\judgRewr{\tenv}{
       \lam{\vartwo}{\tm\subtr{\var}{\redseq}}
     }{
       \lam{\vartwo}{\tm\subt{\var}{\tmfive_0}}
     }{
       \lam{\vartwo}{\tm\subt{\var}{\tmfive_1}}
     }{\typtwo \imp \typthree}$
  as required.
\item
  \indrulename{App}:
  let
    $\judgTerm{\tenv,\var:\typ}{\tm\,\tmtwo}{\typthree}$
  be derived from
    $\judgTerm{\tenv,\var:\typ}{\tm}{\typtwo \imp \typthree}$
  and
    $\judgTerm{\tenv,\var:\typ}{\tmtwo}{\typtwo}$.
  By \ih we have that
    $\judgRewr{\tenv}{\tm\subtr{\var}{\redseq}}{\tm\subt{\var}{\tmfive_0}}{\tm\subt{\var}{\tmfive_1}}{\typtwo \imp \typthree}$
  and
    $\judgRewr{\tenv}{\tmtwo\subtr{\var}{\redseq}}{\tmtwo\subt{\var}{\tmfive_0}}{\tmtwo\subt{\var}{\tmfive_1}}{\typtwo}$.
  Applying the \indrulename{RApp} rule, we obtain
    $\judgRewr{\tenv}{
       \tm\subtr{\var}{\redseq}\,
       \tmtwo\subtr{\var}{\redseq}
     }{
       \tm\subt{\var}{\tmfive_0}\,
       \tmtwo\subt{\var}{\tmfive_0}
     }{
       \tm\subt{\var}{\tmfive_1}\,
       \tmtwo\subt{\var}{\tmfive_1}
     }{\typthree}$ as required.
\end{enumerate}
\end{proof}

\begin{lem}[Commutation of lifting and term substitution (I)]
\llem{subtr_subt_commutation_I}
If
$\judgTerm{\tenv,\var:\typ,\vartwo:\typtwo}{\tm}{\typthree}$
and
$\judgRewr{\tenv,\vartwo:\typtwo}{\redseqthree}{\tmfour_0}{\tmfour_1}{\typ}$
and
$\judgTerm{\tenv}{\tmfive}{\typtwo}$
then:
\[
  \tm
    \subtr{\var}{\redseqthree}
    \subt{\vartwo}{\tmfive}
  =
  \tm
    \subt{\vartwo}{\tmfive}
    \subtr{\var}{\redseqthree\subt{\vartwo}{\tmfive}}
\]
In particular, if $\vartwo$ does not occur free in $\redseqthree$,
then
$
\tm\subtr{\var}{\redseqthree}\subt{\vartwo}{\tmfive}
=
\tm\subt{\vartwo}{\tmfive}\subtr{\var}{\redseqthree}
$.
\end{lem}
\begin{proof}
By induction on the derivation of
$\judgTerm{\tenv,\var:\typ,\vartwo:\typtwo}{\tm}{\typthree}$:
\begin{enumerate}
\item
  \indrulename{Var}:
  let $\judgTerm{\tenv,\var:\typ,\vartwo:\typtwo}{\varthree}{\typthree}$
  with $\varthree:\typthree \in \tenv$.
  We consider three subcases, depending on whether
  $\varthree = \var$, $\varthree = \vartwo$, or
  $\varthree \notin \set{\var,\vartwo}$.
  \begin{enumerate}
  \item
    {\bf If $\varthree = \var$:}
    the left and the right-hand sides are
    both $\redseqthree\subt{\vartwo}{\tmfive}$
    by definition, so we are done.
  \item
    {\bf If $\varthree = \vartwo$:}
    then the left-hand side is $\tmfive$,
    and the right-hand side is $\tmfive\subt{\var}{\redseqthree}$.
    By \rlem{free_variables_typed},
    $\var$ does not occur free in $\tmfive$,
    so $\tmfive = \tmfive\subt{\var}{\redseqthree}$.
  \item
    {\bf If $\varthree \notin \set{\var,\vartwo}$:}
    then the left and the right-hand sides are both $\varthree$
    so we are done.
  \end{enumerate}
\item
  \indrulename{Con}:
  let $\judgTerm{\tenv,\var:\typ,\vartwo:\typtwo}{\cons}{\typthree}$
  with $(\cons:\typthree) \in \constantset$.
  Then the left and the right-hand sides are both
  $\cons$ so we are done.
\item
  \indrulename{Abs}:
  let $\judgTerm{\tenv,\var:\typ,\vartwo:\typtwo}{
         \lam{\varthree}{\tm}}{\typthree \imp \typfour}$
  be derived from
    $\judgTerm{
       \tenv,\var:\typ,\vartwo:\typtwo,\varthree:\typthree
     }{\tm}{\typfour}$.
  Then:
  \[
    \begin{array}{rcll}
      (\lam{\varthree}{\tm})\subtr{\var}{\redseqthree}\subt{\vartwo}{\tmfive}
    & = &
      \lam{\varthree}{\tm\subtr{\var}{\redseqthree}\subt{\vartwo}{\tmfive}}
    \\
    & = &
      \lam{\varthree}{\tm\subt{\vartwo}{\tmfive}\subtr{\var}{\redseqthree\subt{\vartwo}{\tmfive}}}
      & \text{by \ih}
    \\
    & = &
      (\lam{\varthree}{\tm})\subt{\vartwo}{\tmfive}\subtr{\var}{\redseqthree\subt{\vartwo}{\tmfive}}
    \end{array}
  \]
  To apply the \ih we use congruence of equivalence under abstractions,
  and weakening (\rlem{weakening}) on the hypotheses.
\item
  \indrulename{App}:
  let
    $\judgTerm{\tenv,\var:\typ,\vartwo:\typtwo}{\tm\,\tmtwo}{\typfour}$
  be derived from
    $\judgTerm{\tenv,\var:\typ,\vartwo:\typtwo}{\tm}{\typthree \imp \typfour}$
  and
    $\judgTerm{\tenv,\var:\typ,\vartwo:\typtwo}{\tmtwo}{\typthree}$.
  Then:
  \[
    \begin{array}{rcll}
      (\tm\,\tmtwo)
        \subtr{\var}{\redseqthree}\subt{\vartwo}{\tmfive}
    & = &
      \tm\subtr{\var}{\redseqthree}\subt{\vartwo}{\tmfive}\,
      \tmtwo\subtr{\var}{\redseqthree}\subt{\vartwo}{\tmfive}
    \\
    & = &
      \tm
        \subt{\vartwo}{\tmfive}
        \subtr{\var}{\redseqthree\subt{\vartwo}{\tmfive}}\,
      \tmtwo
        \subt{\vartwo}{\tmfive}
        \subtr{\var}{\redseqthree\subt{\vartwo}{\tmfive}}
      & \text{by \ih}
    \\
    & = & (\tm\,\tmtwo)
            \subt{\vartwo}{\tmfive}
            \subtr{\var}{\redseqthree\subt{\vartwo}{\tmfive}}
    \end{array}
  \]
  To apply the \ih we use congruence of equivalence under applications.
\end{enumerate}
\end{proof}

\begin{rem}
$\refl{\tm}\subt{\var}{\tmtwo} = \refl{\tm\subt{\var}{\tmtwo}}$
\end{rem}

\begin{lem}[Lifting reflexivity]
\llem{lifting_reflexivity}
Let $\judgTerm{\tenv,\var:\typ}{\tm}{\typtwo}$
and $\judgTerm{\tenv}{\tmtwo}{\typ}$.
Then $\refl{\tm\subt{\var}{\tmtwo}} = \tm\subtr{\var}{\refl{\tmtwo}}$.
\end{lem}
\begin{proof}
By induction on the derivation of
$\judgTerm{\tenv,\var:\typ}{\tm}{\typtwo}$.
\end{proof}

\begin{lem}[Source and target of rewrite/term substitution]
\llem{source_and_target_of_subrt}
If $\judgRewr{\tenv,\var:\typ}{\redseq}{\tmfive_0}{\tmfive_1}{\typtwo}$
and $\judgTerm{\tenv}{\tm}{\typ}$
then $\rsrc{\redseq\subt{\var}{\tm}} = \rsrc{\redseq}\subt{\var}{\tm}$
and $\rtgt{\redseq\subt{\var}{\tm}} = \rtgt{\redseq}\subt{\var}{\tm}$.
\end{lem}
\begin{proof}
Straightforward by induction on $\redseq$.
\end{proof}

\begin{lem}[Source and target of term/rewrite substitution]
\llem{source_and_target_of_subtr}
If $\judgTerm{\tenv,\var:\typ}{\tm}{\typtwo}$
and $\judgRewr{\tenv}{\redseq}{\tmfive_0}{\tmfive_1}{\typ}$
then $\rsrc{\tm\subtr{\var}{\redseq}} = \tm\subtr{\var}{\rsrc{\redseq}}$
and $\rtgt{\tm\subtr{\var}{\redseq}} = \tm\subtr{\var}{\rtgt{\redseq}}$.
\end{lem}
\begin{proof}
Straightforward by induction on $\tm$.
\end{proof}

%%% Local Variables:
%%% mode: latex
%%% TeX-master: "main"
%%% End:
