# Supplementary material for: Reductions in Higher-Order Rewriting and Their Equivalence
Source: arXiv:2210.15654 source file (2023-08-15)
Supplement: Supplementary file 2 [file a02-permutation_equivalence.tex]

\begin{lem}[Term equivalence implies permutation equivalence]
\llem{termeq_implies_permeq}
If $\judgTermEq{\tenv}{\tm}{\tm'}{\typ}$
then $\refl{\tm} \permeq \refl{\tm'}$.
\end{lem}
\begin{proof}
By induction on the derivation of $\judgTermEq{\tenv}{\tm}{\tm'}{\typ}$.
Reflexivity, symmetry, transitivity, and congruence under term constructors
are immediate. The interesting cases are:
\begin{enumerate}
\item \indrulename{EqBeta}:
  Let $\tm = (\lam{\var}{\tmtwo})\,\tmthree$
  and $\tm' = \tmtwo\subt{\var}{\tmthree}$.
  Then:
  \[
    \begin{array}{rcll}
      (\lam{\var}{\refl{\tmtwo}})\,\refl{\tmthree}
    & \permeq &
      \tmtwo\subtr{\var}{\refl{\tmthree}}
      & \text{by \permeqRule{BetaTR}}
    \\
    & = &
      \refl{\tmtwo\subt{\var}{\tmthree}}
      & \text{by \rlem{lifting_reflexivity}}
    \end{array}
  \]
\item \indrulename{EqEta}:
  Let $\tm = \lam{\var}{\tm'\,\var}$
  with $\var \notin \fv{\tm'}$. Then:
  \[
    \begin{array}{rcll}
      \lam{\var}{\refl{\tm'}\,\var}
    & \permeq &
      \refl{\tm'}
      & \text{by \permeqRule{Eta}}
    \end{array}
  \]
\end{enumerate}
\end{proof}

\begin{lem}[Generalized \permeqRule{IdL} and \permeqRule{IdR} rules]
\llem{generalized_permeq_IdL_IdR}
Let $\judgRewr{\tenv}{\redseq}{\tmfour}{\tmfive}{\typ}$.
Then the following generalized variants
of \permeqRule{IdL} and \permeqRule{IdR} hold:
\begin{enumerate}
\item If $\judgTermEq{\tenv}{\tm}{\rsrc{\redseq}}{\typ}$,
      then $(\refl{\tm}\seq\redseq) \permeq \redseq$.
\item If $\judgTermEq{\tenv}{\tm}{\rtgt{\redseq}}{\typ}$,
      then $(\redseq\seq\refl{\tm}) \permeq \redseq$.
\end{enumerate}
Sometimes by abuse we call these generalized rules
\permeqRule{IdL} and \permeqRule{IdR},
without explicit reference to this lemma.
\end{lem}
\begin{proof}
Item~1. is immediate given that:
\[
  \begin{array}{rcll}
    (\refl{\tm}\seq\redseq)
  & \permeq &
    (\refl{\rsrc{\redseq}}\seq\redseq)
    & \text{by \rlem{termeq_implies_permeq}}
  \\
  & \permeq &
    \redseq
    & \text{by \permeqRule{IdL}}
  \end{array}
\]
Item~2. is similar.
\end{proof}

\begin{lem}[Term contexts distribute over composition]
\llem{permeq_distribute_cctx_over_seq}
$\cctxof{\redseq\seq\redseqtwo} \permeq \cctxof{\redseq}\seq\cctxof{\redseqtwo}$
\end{lem}
\begin{proof}
By induction on $\cctx$:
\begin{enumerate}
\item {\bf Empty, $\cctx = \ctxhole$.}
  Immediate.
\item {\bf Abstraction, $\cctx = \lam{\var}{\cctx'}$.}
  \[
    \begin{array}{rcll}
      \lam{\var}{\cctx'\ctxof{\redseq\seq\redseqtwo}}
    & \permeq &
      \lam{\var}{(\cctx'\ctxof{\redseq})\seq\cctx'\ctxof{\redseqtwo})}
      & \text{by \ih}
    \\
    & \permeq &
      (\lam{\var}{\cctx'\ctxof{\redseq}})\seq
      (\lam{\var}{\cctx'\ctxof{\redseqtwo}})
      & \text{by \permeqRule{Abs}}
    \end{array}
  \]
\item {\bf Left of an application, $\cctx = \cctx'\,\tm$.}
  \[
    \begin{array}{rcll}
      \cctx'\ctxof{\redseq\seq\redseqtwo}\,\tm
    & \permeq &
      (\cctx'\ctxof{\redseq}\seq\cctx'\ctxof{\redseqtwo})\,\tm
      & \text{by \ih}
    \\
    & \permeq &
      (\cctx'\ctxof{\redseq}\seq\cctx'\ctxof{\redseqtwo})\,(\tm\seq\tm)
      & \text{by \permeqRule{IdL}}
    \\
    & \permeq &
      (\cctx'\ctxof{\redseq}\,\tm)\seq(\cctx'\ctxof{\redseqtwo}\,\tm)
      & \text{by \permeqRule{App}}
    \end{array}
  \]
\item {\bf Right of an application, $\cctx = \tm\,\cctx'$.}
  Similar to the previous case.
\end{enumerate}
\end{proof}

\subsection{Properties of term/rewrite substitution, up to permutation equivalence}

\begin{lem}[Transitivity under lifting substitution]
\llem{transitivity_lifting}
Let $\judgTerm{\tenv,\var:\typ}{\tm}{\typtwo}$
and
$\judgRewr{\tenv}{\redseq}{\tmfour_0}{\tmfour_1}{\typ}$
and
$\judgRewr{\tenv}{\redseqtwo}{\tmfour_1}{\tmfour_2}{\typ}$.
Then:
\[
  \tm\subtr{\var}{\redseq}\seq\tm\subtr{\var}{\redseqtwo}
  \permeq
  \tm\subtr{\var}{\redseq\seq\redseqtwo}
\]
\end{lem}
\begin{proof}
By induction on the derivation of
$\judgTerm{\tenv,\var:\typ}{\tm}{\typtwo}$:
\begin{enumerate}
\item \indrulename{Var}:
  let
    $\judgTerm{\tenv,\var:\typ}{\vartwo}{\typtwo}$
  with $\vartwo:\typtwo \in (\tenv,\var:\typ)$.
  We consider two subcases, depending on whether $\var = \vartwo$
  or not:
  \begin{enumerate}
  \item {\bf If $\var = \vartwo$}:
    then the left and the right-hand sides are both
    $\redseq\seq\redseqtwo$, so we are done.
  \item {\bf If $\var \neq \vartwo$}:
    then the left-hand side is $\vartwo\seq\vartwo$
    and the right-hand side is $\vartwo$,
    and $\vartwo\seq\vartwo \permeq \vartwo$
    by the \permeqRule{IdL} rule.
  \end{enumerate}
\item
  \indrulename{Con}:
  let $\judgTerm{\tenv,\var:\typ}{\cons}{\typtwo}$
  with $(\cons:\typtwo) \in \constantset$.
  Then the left-hand side is $\cons\seq\cons$
  and the right-hand side is $\cons$,
  and $\cons\seq\cons \permeq \cons$
  by the \permeqRule{IdL} rule.
\item
  \indrulename{Abs}:
  let
    $\judgTerm{\tenv}{\lam{\vartwo}{\tm}}{\typtwo \imp \typthree}$
  be derived from
    $\judgTerm{\tenv,\var:\typ,\vartwo:\typtwo}{\tm}{\typthree}$.
  Then:
  \[
    \begin{array}{rcll}
      (\lam{\vartwo}{\tm})\subtr{\var}{\redseq}
      \seq
      (\lam{\vartwo}{\tm})\subtr{\var}{\redseqtwo}
    & = &
      (\lam{\vartwo}{\tm\subtr{\var}{\redseq}})
      \seq
      (\lam{\vartwo}{\tm\subtr{\var}{\redseqtwo}})
    \\
    & \permeq &
      \lam{\vartwo}{
         (\tm\subtr{\var}{\redseq}\seq\tm\subtr{\var}{\redseqtwo})
      }
      & \text{by \permeqRule{Abs}}
    \\
    & \permeq &
      \lam{\vartwo}{\tm\subtr{\var}{\redseq\seq\redseqtwo}}
      & \text{by \ih}
    \\
    & = &
      (\lam{\vartwo}{\tm})\subtr{\var}{\redseq\seq\redseqtwo}
      & \text{by \ih}
    \end{array}
  \]
\item
  \indrulename{App}:
  let
    $\judgTerm{\tenv,\var:\typ}{\tm\,\tmtwo}{\typthree}$
  be derived from
    $\judgTerm{\tenv,\var:\typ}{\tm}{\typtwo \imp \typthree}$
  and
    $\judgTerm{\tenv,\var:\typ}{\tmtwo}{\typtwo}$.
  Then:
  \[
    \begin{array}{rcll}
      (\tm\,\tmtwo)\subtr{\var}{\redseq} \seq
      (\tm\,\tmtwo)\subtr{\var}{\redseqtwo}
    & = &
      (\tm\subtr{\var}{\redseq}\,\tmtwo\subtr{\var}{\redseq}) \seq
      (\tm\subtr{\var}{\redseqtwo}\,\tmtwo\subtr{\var}{\redseqtwo})
    \\
    & \permeq &
      (\tm\subtr{\var}{\redseq} \seq \tm\subtr{\var}{\redseqtwo})\,
      (\tmtwo\subtr{\var}{\redseq} \seq \tmtwo\subtr{\var}{\redseqtwo})
      & \text{by \permeqRule{App}}
    \\
    & \permeq &
      \tm\subtr{\var}{\redseq\seq\redseqtwo}\,
      \tmtwo\subtr{\var}{\redseq\seq\redseqtwo}
      & \text{by \ih}
    \\
    & = &
      (\tm\,\tmtwo)\subtr{\var}{\redseq\seq\redseqtwo}
    \end{array}
  \]
\end{enumerate}
\end{proof}

\subsection{Rewrite/rewrite substitution}
\lsec{appendix:rewrite_rewrite_substitution}

% In this subsection we show that
% a notion of ``rewrite/rewrite substitution''
% $\redseq\subrr{\var}{\redseqtwo}$
% can be defined in such a way that
% $(\lam{\var}{\redseq})\,\redseqtwo \permeq \redseq\subrr{\var}{\redseqtwo}$
% can be proved as a theorem.
% 
% \begin{defi}[Rewrite/rewrite substitution]
% If
% $\judgRewr{\tenv,\var:\typ}{\redseq}{\tm}{\tm'}{\typtwo}$
% and
% $\judgRewr{\tenv}{\redseqtwo}{\tmtwo}{\tmtwo'}{\typ}$
% then:
% \[
%   \redseq\subrr{\var}{\redseqtwo} \eqdef
%   \redseq\subt{\var}{\tmtwo}\seq
%   \tm'\subtr{\var}{\redseqtwo}
% \]
% \end{defi}

\begin{rem}
Note that $\redseq\subrr{\var}{\redseqtwo}$
depends on $\tm'$ and $\tmtwo$,
and hence on the particular typing derivations
for $\redseq$ and $\redseqtwo$.
These particular derivations will usually be clear from the context.
If there is any confusion we may write
  $\redseq\subt{\var}{\tmtwo}\seq
  \tm'\subtr{\var}{\redseqtwo}$
explicitly.
We shall prove congruence results
(in particular, \rlem{congruence_termeq_subrt}
and \rlem{congruence_termeq_subtr})
which ensure that the value of $\redseq\subrr{\var}{\redseqtwo}$
does not depend, up to permutation equivalence, on the particular typing
derivations chosen.
\end{rem}

% \begin{lem}[Rewrite/rewrite $\beta$-reduction rule]
% \llem{betaRR}
% Let $\judgRewr{\tenv,\var:\typ}{\redseq}{\tm_0}{\tm_1}{\typtwo}$
% and $\judgRewr{\tenv}{\redseqtwo}{\tmtwo_0}{\tmtwo_1}{\typ}$.
% Then the following equivalence, called \permeqRule{BetaRR}, holds:
% \[
%   (\lam{\var}{\redseq})\,\redseqtwo
%   \permeq
%   \redseq\subrr{\var}{\redseqtwo}
%   \HS\HS (\permeqRule{BetaRR})
% \]
% \end{lem}
% \begin{proof}
% \[
%   \begin{array}{rcll}
%     (\lam{\var}{\redseq})\,\redseqtwo
%   & \permeq &
%     ((\lam{\var}{\redseq})\seq(\lam{\var}{\tm_1}))\,\redseqtwo
%     & \permeqRule{IdR}
%   \\
%   & \permeq &
%     ((\lam{\var}{\redseq})\seq(\lam{\var}{\tm_1}))\,(\tmtwo_0\seq\redseqtwo)
%     & \permeqRule{IdL}
%   \\
%   & \permeq &
%     (\lam{\var}{\redseq})\,\tmtwo_0 \seq (\lam{\var}{\tm_1})\,\redseqtwo
%     & \permeqRule{App}
%   \\
%   & \permeq &
%     \redseq\subt{\var}{\tmtwo_0} \seq (\lam{\var}{\tm_1})\,\redseqtwo
%     & \permeqRule{BetaRT}
%   \\
%   & \permeq &
%     \redseq\subt{\var}{\tmtwo_0} \seq \tm_1\subtr{\var}{\redseqtwo}
%     & \permeqRule{BetaTR}
%   \\
%   & = &
%     \redseq\subrr{\var}{\redseqtwo}
%   \end{array}
% \]
% \end{proof}

\begin{lem}[Typing rule for rewrite/rewrite substitution]
If
$\judgRewr{\tenv,\var:\typ}{\redseq}{\tm}{\tm'}{\typtwo}$
and
$\judgRewr{\tenv}{\redseqtwo}{\tmtwo}{\tmtwo'}{\typ}$
then:
\[
  \judgRewr{\tenv}{
    \redseq\subrr{\var}{\redseqtwo}
  }{
    \tm\subt{\var}{\tmtwo}
  }{
    \tm'\subt{\var}{\tmtwo'}
  }{
    \typtwo
  }
\]
\end{lem}
\begin{proof}
An immediate consequence of
\rlem{substitution_term_variables}
and
\rlem{fundamental_property_of_term_lifting}.
\end{proof}

The notion of rewrite/rewrite substitution generalizes the notions
of rewrite/term and term/rewrite (lifting) substitution,
as noted in the two following remarks:

\begin{rem}[Rewrite/rewrite generalizes rewrite/term substitution]
\lremark{subrr_refl_R}
If
$\judgRewr{\tenv,\var:\typ}{\redseq}{\tm}{\tm'}{\typtwo}$
and
$\judgTerm{\tenv}{\tmtwo}{\typ}$
then:
\[
  \redseq\subt{\var}{\tmtwo} \permeq \redseq\subrr{\var}{\refl{\tmtwo}}
\]
Indeed:
\[
  \begin{array}{rcll}
    \redseq\subt{\var}{\tmtwo}
  & \permeq &
    \redseq\subt{\var}{\tmtwo} \seq \refl{\tm'\subt{\var}{\tmtwo}}
    & \text{by \permeqRule{IdR}}
  \\
  & = &
    \redseq\subt{\var}{\tmtwo}
    \seq
    \tm'\subtr{\var}{\refl{\tmtwo}}
    & \text{by \rlem{lifting_reflexivity}}
  \\
  & = &
    \redseq\subrr{\var}{\refl{\tmtwo}}
  \end{array}
\]
\end{rem}

\begin{rem}[Rewrite/rewrite generalizes term/rewrite substitution]
\lremark{subrr_refl_L}
If
$\judgTerm{\tenv,\var:\typ}{\tm}{\typtwo}$
and
$\judgRewr{\tenv}{\redseq}{\tmtwo}{\tmtwo'}{\typ}$
then:
\[
  \tm\subtr{\var}{\redseq} \permeq \refl{\tm}\subrr{\var}{\redseq}
\]
Indeed:
\[
  \begin{array}{rcll}
    \tm\subtr{\var}{\redseq}
  & \permeq &
    \refl{\tm\subt{\var}{\tmtwo}}\seq\tm\subtr{\var}{\redseq}
  & \text{by \permeqRule{IdL}}
  \\
  & = &
    \refl{\tm}\subt{\var}{\tmtwo}\seq\tm\subtr{\var}{\redseq}
    & \text{since $\refl{\tm}\subt{\var}{\tmtwo} = \refl{\tm\subt{\var}{\tmtwo}}$ by definition}
  \\
  & = &
    \refl{\tm}\subrr{\var}{\redseq}
    & \text{by definition of $\refl{\tm}\subtr{\var}{\redseq}$}
  \end{array}
\]
\end{rem}

\begin{lem}[Trivial rewrite/rewrite substitution]
\llem{trivial_subrr_substitution}
Let $\judgRewr{\tenv,\var:\typ}{\redseq}{\tm_0}{\tm_1}{\typtwo}$
be such that $\var\notin\fv{\redseq}$,
and let
$\judgRewr{\tenv}{\redseqtwo}{\tmtwo_0}{\tmtwo_1}{\typ}$.
Then $\redseq\subrr{\var}{\redseqtwo} \permeq \redseq$.
\end{lem}
\begin{proof}
Note that $\var \notin \fv{\tm_1}$ by \rlem{free_variables_of_endpoints}.
\[
  \begin{array}{rcll}
    \redseq\subrr{\var}{\redseqtwo}
  & = &
    \redseq\subt{\var}{\tmtwo_0}
    \seq
    \tm_1\subtr{\var}{\redseqtwo}
    & \text{by definition}
  \\
  & = &
    \redseq
    \seq
    \tm_1\subtr{\var}{\redseqtwo}
    & \text{since $\var \notin \fv{\redseq}$}
  \\
  & = &
    \redseq
    \seq
    \refl{\tm_1}
    & \text{since $\var \notin \fv{\tm_1}$}
  \\
  & \permeq &
    \redseq
    & \text{by \permeqRule{IdR}}
  \end{array}
\]
\end{proof}

\begin{lem}[Recursive equations for rewrite/rewrite substitution]
\llem{subrr_recursion}
Let $\judgRewr{\tenv}{\redseqtwo}{\tmfive_0}{\tmfive_1}{\typ}$.
The following recursive equations hold for rewrite/rewrite substitution:
\begin{enumerate}
\item If $\judgRewr{\tenv,\var:\typ,\vartwo:\typtwo}{\redseq}{\tm_0}{\tm_1}{\typthree}$, then:
      \[
        (\lam{\vartwo}{\redseq})\subrr{\var}{\redseqtwo}
        \permeq
        \lam{\vartwo}{\redseq\subrr{\vartwo}{\redseqtwo}}
      \]
\item If $\judgRewr{\tenv,\var:\typ}{\redseq_1}{\tm_0}{\tm_1}{\typtwo \imp \typthree}$
      and $\judgRewr{\tenv,\var:\typ}{\redseq_2}{\tmtwo_0}{\tmtwo_1}{\typtwo}$,
      then:
      \[
        (\redseq_1\,\redseq_2)\subrr{\var}{\redseqtwo}
        \permeq
        \redseq_1\subrr{\var}{\redseqtwo}\,\redseq_2\subrr{\var}{\redseqtwo}
      \]
\end{enumerate}
\end{lem}
\begin{proof}
We check each item separately:
\begin{enumerate}
\item Abstraction:
  \[
    \begin{array}{rcll}
          (\lam{\vartwo}{\redseq})\subrr{\var}{\redseqtwo}
    & = & (\lam{\vartwo}{\redseq})\subt{\var}{\tmfive_0} \seq
          (\lam{\vartwo}{\tm_1})\subtr{\var}{\redseqtwo}
    \\
    & = & (\lam{\vartwo}{\redseq\subt{\var}{\tmfive_0}}) \seq
          (\lam{\vartwo}{\tm_1\subtr{\var}{\redseqtwo}})
    \\
    & \permeq &
          \lam{\vartwo}{(\redseq\subt{\var}{\tmfive_0} \seq
                          \tm_1\subtr{\var}{\redseqtwo})}
      & \text{by \permeqRule{Abs}}
    \\
    & = & \lam{\vartwo}{\redseq\subrr{\var}{\redseqtwo}}
    \end{array}
  \]
\item Application:
  similar to the previous case, using the \permeqRule{App} rule.
\end{enumerate}
\end{proof}

\begin{lem}[Commutation of lifting and term substitution (II)]
\llem{subtr_subt_commutation_II}
If $\judgTerm{\tenv,\var:\typ,\vartwo:\typtwo}{\tm}{\typthree}$
and $\judgTerm{\tenv,\vartwo:\typtwo}{\tmfive}{\typ}$
and $\judgRewr{\tenv}{\redseqthree}{\tmfour_0}{\tmfour_1}{\typtwo}$
then:
\[
  \tm\subt{\var}{\tmfive}\subtr{\vartwo}{\redseqthree}
  \permeq
  \tm\subtr{\vartwo}{\redseqthree}\subrr{\var}{\tmfive\subtr{\vartwo}{\redseqthree}}
\]
\end{lem}
\begin{proof}
By induction on the derivation of
$\judgTerm{\tenv,\var:\typ,\vartwo:\typtwo}{\tm}{\typthree}$.
\begin{enumerate}
\item
  \indrulename{Var}:
  let $\judgTerm{\tenv,\var:\typ,\vartwo:\typtwo}{\varthree}{\typthree}$
  with $\varthree:\typthree \in (\tenv,\var:\typ,\vartwo:\typtwo)$.
  We consider three subcases, depending on whether
  $\varthree = \var$, $\varthree = \vartwo$,
  or $\varthree \notin \set{\var,\vartwo}$:
  \begin{enumerate}
  \item {\bf If $\varthree = \var$}:
    Then the left and the right-hand sides are both
    $\tmfive\subtr{\vartwo}{\redseqthree}$, so it is immediate
    to conclude.
  \item {\bf If $\varthree = \vartwo$}:
    Then the left-hand side is $\redseqthree$
    and the right-hand side is
    $\redseqthree\subrr{\var}{\tmfive\subtr{\vartwo}{\redseqthree}}$
    Note that by \rlem{free_variables_typed},
    $\var$ does not occur free in $\redseqthree$,
    so by \rlem{trivial_subrr_substitution} we conclude.
  \item {\bf If $\varthree \notin \set{\var,\vartwo}$}:
    Then the left and the right-hand sides are both $\varthree$
    so we are done.
  \end{enumerate}
\item
  \indrulename{Con}:
  let
    $\judgTerm{\tenv,\var:\typ,\var:\typtwo}{\cons}{\typthree}$
  with
    $(\cons:\typthree) \in \constantset$.
  Then the left and the right-hand sides are both $\cons$,
  so we are done.
\item
  \indrulename{Abs}:
  let
    $\judgTerm{\tenv,\var:\typ,\vartwo:\typtwo}{\lam{\varthree}{\tm}}{\typthree \imp \typfour}$
  be derived from
    $\judgTerm{\tenv,\var:\typ,\vartwo:\typtwo,\varthree:\typthree}{\tm}{\typfour}$.
  Then:
  \[
    \begin{array}{rcll}
      (\lam{\varthree}{\tm})
        \subt{\var}{\tmfive}
        \subtr{\vartwo}{\redseqthree}
    & = &
      \lam{\varthree}{\tm
        \subt{\var}{\tmfive}
        \subtr{\vartwo}{\redseqthree}
      }
    \\
    & \permeq &
      \lam{\varthree}{\tm
        \subtr{\vartwo}{\redseqthree}
        \subrr{\var}{\tmfive\subtr{\vartwo}{\redseqthree}}
      }
      & \text{by \ih}
    \\
    & \permeq &
      (\lam{\varthree}{\tm})
        \subtr{\vartwo}{\redseqthree}
        \subrr{\var}{\tmfive\subtr{\vartwo}{\redseqthree}}
      & \text{by \rlem{subrr_recursion}}
    \end{array}
  \]
\item
  \indrulename{App}:
  let
    $\judgTerm{\tenv,\var:\typ,\vartwo:\typtwo}{\tm\,\tmtwo}{\typfour}$
  be derived from
    $\judgTerm{\tenv,\var:\typ,\vartwo:\typtwo}{\tm}{\typthree \imp \typfour}$
  and
    $\judgTerm{\tenv,\var:\typ,\vartwo:\typtwo}{\tmtwo}{\typthree}$
  Then:
  \[
    \begin{array}{rcll}
      (\tm\,\tmtwo)
        \subt{\var}{\tmfive}
        \subtr{\vartwo}{\redseqthree}
    & = &
      \tm
        \subt{\var}{\tmfive}
        \subtr{\vartwo}{\redseqthree}
      \,
      \tmtwo
        \subt{\var}{\tmfive}
        \subtr{\vartwo}{\redseqthree}
    \\
    & \permeq &
      \tm
        \subtr{\vartwo}{\redseqthree}
        \subrr{\var}{\tmfive\subtr{\vartwo}{\redseqthree}}
      \,
      \tmtwo
        \subtr{\vartwo}{\redseqthree}
        \subrr{\var}{\tmfive\subtr{\vartwo}{\redseqthree}}
      & \text{by \ih}
    \\
    & \permeq &
      (\tm\,\tmtwo)
        \subtr{\vartwo}{\redseqthree}
        \subrr{\var}{\tmfive\subtr{\vartwo}{\redseqthree}}
      & \text{by \rlem{subrr_recursion}}
    \end{array}
  \]
\end{enumerate}
\end{proof}

\subsection{Congruence properties}

\subsection{Permutation lemma}

\begin{prop}[Transitivity under rewrite/rewrite substitution]
\lprop{transitivity_subrr}
Suppose that:
\begin{itemize}
\item
  $\judgRewr{\tenv,\var:\typ}{\redseq_1}{\tm_0}{\tm_1}{\typtwo}$
  and
  $\judgRewr{\tenv,\var:\typ}{\redseq_2}{\tm_1}{\tm_2}{\typtwo}$
\item
  $\judgRewr{\tenv}{\redseqtwo_1}{\tmtwo_0}{\tmtwo_1}{\typtwo}$
  and
  $\judgRewr{\tenv}{\redseqtwo_2}{\tmtwo_1}{\tmtwo_2}{\typtwo}$
\end{itemize}
Then:
\[
  (\redseq_1\seq\redseq_2)\subrr{\var}{\redseqtwo_1\seq\redseqtwo_2}
  \permeq
  \redseq_1\subrr{\var}{\redseqtwo_1}\seq\redseq_2\subrr{\var}{\redseqtwo_2}
\]
\end{prop}
\begin{proof}
We work implicitly modulo associativity of composition (``$\seq$''),
using the \permeqRule{Assoc} rule:
\[
  \begin{array}{rcll}
    (\redseq_1\seq\redseq_2)\subrr{\var}{\redseqtwo_1\seq\redseqtwo_2}
  & = &
         (\redseq_1\seq\redseq_2)\subt{\var}{\tmtwo_0}
    \seq \tm_2\subtr{\var}{\redseqtwo_1\seq\redseqtwo_2}
  \\
  & = &
         \redseq_1\subt{\var}{\tmtwo_0}
    \seq \redseq_2\subt{\var}{\tmtwo_0}
    \seq \tm_2\subtr{\var}{\redseqtwo_1\seq\redseqtwo_2}
  \\
  & \permeq &
         \redseq_1\subt{\var}{\tmtwo_0}
    \seq \redseq_2\subt{\var}{\tmtwo_0}
    \seq \tm_2\subtr{\var}{\redseqtwo_1}
    \seq \tm_2\subtr{\var}{\redseqtwo_2}
    & \text{by \rlem{transitivity_lifting}}
  \\
  & \permeq &
         \redseq_1\subt{\var}{\tmtwo_0}
    \seq \tm_1\subtr{\var}{\redseqtwo_1}
    \seq \redseq_2\subt{\var}{\tmtwo_1}
    \seq \tm_2\subtr{\var}{\redseqtwo_2}
    & \text{by \rlem{coherence}}
  \\
  & \permeq &
         \redseq_1\subrr{\var}{\redseqtwo_1}
    \seq \redseq_2\subrr{\var}{\redseqtwo_2}
  \end{array}
\]
\end{proof}

\begin{prop}[Substitution property for rewrite/rewrite substitution]
\lprop{substitution_property_for_subrr}
Suppose that:
\begin{itemize}
\item $\judgRewr{\tenv,\var:\typ,\vartwo:\typtwo}{\redseq}{\tm_0}{\tm_1}{\typthree}$
\item $\judgRewr{\tenv,\vartwo:\typtwo}{\redseqtwo}{\tmtwo_0}{\tmtwo_1}{\typ}$
\item $\judgRewr{\tenv}{\redseqthree}{\tmthree_0}{\tmthree_1}{\typtwo}$
\end{itemize}
Then:
\[
  \redseq
    \subrr{\var}{\redseqtwo}
    \subrr{\vartwo}{\redseqthree}
  \permeq
  \redseq
    \subrr{\vartwo}{\redseqthree}
    \subrr{\var}{\redseqtwo\subrr{\vartwo}{\redseqthree}}
\]
\end{prop}
\begin{proof}
We work implicitly modulo associativity of composition (``$\seq$''),
using the \permeqRule{Assoc} rule:
\[
{\small
  \begin{array}{rcll}
  &&
    \redseq
      \subrr{\var}{\redseqtwo}
      \subrr{\vartwo}{\redseqthree}
  \\
  & = &
    (\redseq\subt{\var}{\tmtwo_0}
     \seq
     \tm_1\subtr{\var}{\redseqtwo})
     \subrr{\vartwo}{\redseqthree}
     & \text{by definition of $\subrr{\var}{\redseqtwo}$}
  \\
  & = &
    (\redseq\subt{\var}{\tmtwo_0}
     \seq
     \tm_1\subtr{\var}{\redseqtwo})
     \subt{\vartwo}{\tmthree_0}
    \seq
    \tm_1\subt{\var}{\tmtwo_1}\subtr{\vartwo}{\redseqthree}
     & \text{by definition of $\subrr{\vartwo}{\redseqthree}$}
  \\
  & = &
    \redseq\subt{\var}{\tmtwo_0}
           \subt{\vartwo}{\tmthree_0}
    \seq
    \tm_1\subtr{\var}{\redseqtwo}
         \subt{\vartwo}{\tmthree_0}
    \seq
    \tm_1\subt{\var}{\tmtwo_1}\subtr{\vartwo}{\redseqthree}
  \\
  & = &
    \redseq\subt{\vartwo}{\tmthree_0}
           \subt{\var}{\tmtwo_0\subt{\vartwo}{\tmthree_0}}
    \seq
    \tm_1\subtr{\var}{\redseqtwo}
         \subt{\vartwo}{\tmthree_0}
    \seq
    \tm_1\subt{\var}{\tmtwo_1}\subtr{\vartwo}{\redseqthree}
     & \text{Substitution Lemma ($\star$)}
  \\
  & \permeq &
    \redseq\subt{\vartwo}{\tmthree_0}
           \subt{\var}{\tmtwo_0\subt{\vartwo}{\tmthree_0}}
    \seq
    \tm_1\subt{\vartwo}{\tmthree_0}
         \subtr{\var}{\redseqtwo\subt{\vartwo}{\tmthree_0}}
    \seq
    \tm_1\subt{\var}{\tmtwo_1}\subtr{\vartwo}{\redseqthree}
    & \text{\rlem{subtr_subt_commutation_I}}
  \\
  & \permeq &
    \redseq\subt{\vartwo}{\tmthree_0}
           \subt{\var}{\tmtwo_0\subt{\vartwo}{\tmthree_0}}
    \seq
    \tm_1\subt{\vartwo}{\tmthree_0}
         \subtr{\var}{\redseqtwo\subt{\vartwo}{\tmthree_0}}
    \seq
    \tm_1\subtr{\vartwo}{\redseqthree}
         \subrr{\var}{\tmtwo_1\subtr{\vartwo}{\redseqthree}}
    & \text{\rlem{subtr_subt_commutation_II}}
  \\
  & = &
    \redseq\subt{\vartwo}{\tmthree_0}
           \subrr{\var}{\tmtwo_0\subt{\vartwo}{\tmthree_0}}
    \seq
    \tm_1\subt{\vartwo}{\tmthree_0}
         \subtr{\var}{\redseqtwo\subt{\vartwo}{\tmthree_0}}
    \seq
    \tm_1\subtr{\vartwo}{\redseqthree}
         \subrr{\var}{\tmtwo_1\subtr{\vartwo}{\redseqthree}}
    & \text{\rremark{subrr_refl_R}}
  \\
  & \permeq &
    \redseq\subt{\vartwo}{\tmthree_0}
           \subrr{\var}{\refl{\tmtwo_0\subt{\vartwo}{\tmthree_0}}}
    \seq
    \refl{\tm_1\subt{\vartwo}{\tmthree_0}}
         \subrr{\var}{\redseqtwo\subt{\vartwo}{\tmthree_0}}
    \seq
    \tm_1\subtr{\vartwo}{\redseqthree}
         \subrr{\var}{\tmtwo_1\subtr{\vartwo}{\redseqthree}}
    & \text{\rremark{subrr_refl_L}}
  \\
    & \permeq &
    (\redseq\subt{\vartwo}{\tmthree_0}
    \seq
    \refl{\tm_1\subt{\vartwo}{\tmthree_0}}
    \seq
    \tm_1\subtr{\vartwo}{\redseqthree})
      \subrr{\var}{
        \refl{\tmtwo_0\subt{\vartwo}{\tmthree_0}}
        \seq \redseqtwo\subt{\vartwo}{\tmthree_0}
        \seq \tmtwo_1\subtr{\vartwo}{\redseqthree}
      }
    & \text{\rprop{transitivity_subrr} (twice)}
  \\
    & \permeq &
    (\redseq\subt{\vartwo}{\tmthree_0}
    \seq
    \tm_1\subtr{\vartwo}{\redseqthree})
      \subrr{\var}{
             \redseqtwo\subt{\vartwo}{\tmthree_0}
        \seq \tmtwo_1\subtr{\vartwo}{\redseqthree}
      }
    & \text{by \permeqRule{IdL} ($\star\star$)}
  \\
    & \permeq &
    \redseq\subrr{\vartwo}{\redseqthree}
      \subrr{\var}{\redseqtwo\subrr{\vartwo}{\redseqthree}}
    & \text{by \permeqRule{IdL}}
  \end{array}
}
\]
In the step marked with ($\star$) we use a
variant of the standard Substitution Lemma for
capture-avoiding substitution of a variable for a term.
In the step marked with ($\star\star$)
we use the fact that permutation equivalence is compatible with
rewrite/rewrite substitution~(\rprop{congruence_permeq_subrr}).
\end{proof}

\begin{lem}[Generalized \permeqRule{App}]
\llem{generalized_seqr_transapp_rule}
Suppose that:
\begin{itemize}
\item $\judgRewr{\tenv}{\redseq}{\tm}{\tm'}{
        \typ_1 \imp \hdots \imp \typ_n \imp \typtwo
      }$
      and
      $\judgRewr{\tenv}{\redseq'}{\tm'}{\tm''}{
        \typ_1 \imp \hdots \imp \typ_n \imp \typtwo
      }$,
\item $\judgRewr{\tenv}{\redseqtwo_i}{\tmtwo_i}{\tmtwo'_i}{\typ_i}$
      and
      $\judgRewr{\tenv}{\redseqtwo_i}{\tmtwo'_i}{\tmtwo''_i}{\typ_i}$
      for all $1 \leq i \leq n$.
\end{itemize}
Then:
  \[
    (\redseq\,\redseqtwo_1\hdots\redseqtwo_n) \seq
    (\redseq'\,\redseqtwo'_1\hdots\redseqtwo'_n)
    \permeq
    (\redseq\seq\redseq')\,
    (\redseqtwo_1\seq\redseqtwo'_1)\hdots
    (\redseqtwo_n\seq\redseqtwo'_n)
  \]
\end{lem}
\begin{proof}
By induction on $n$.
The base case when $n = 0$ is immediate. In the inductive case:
  \[
    \begin{array}{rcll}
    &&
      (\redseq\,\redseqtwo_1\hdots\redseqtwo_n\,\redseqtwo_{n+1}) \seq
      (\redseq'\,\redseqtwo'_1\hdots\redseqtwo'_n\,\redseqtwo_{n+1})
    \\
    & \permeq &
      (\redseq\,\redseqtwo_1\hdots\redseqtwo_n\seq
       \redseq'\,\redseqtwo'_1\hdots\redseqtwo'_n)\,
      (\redseqtwo_{n+1}\seq\redseqtwo_{n+1})
      & \text{by \permeqRule{App}}
    \\
    & \permeq &
      (\redseq\seq\redseq')\,
      (\redseqtwo_1\seq\redseqtwo'_1)
      \hdots
      (\redseqtwo_n\seq\redseqtwo'_n)\,
      (\redseqtwo_{n+1}\seq\redseqtwo_{n+1})
      & \text{by \ih}
    \end{array}
  \]
\end{proof}

\begin{lem}[Generalized \permeqRule{BetaRR} rule]
\llem{generalized_peqr_beta_rule}
Suppose that:
\begin{itemize}
\item
   $\judgRewr{\tenv,\var_1:\typ_1,\hdots,\var_n:\typ_n}{
       \redseq}{\tm}{\tm'}{\typtwo}$
\item
   $\judgRewr{\tenv}{\redseqtwo_i}{\tmtwo_i}{\tmtwo_i'}{\typtwo_i}$
   for all $1 \leq i \leq n$
\end{itemize}
Then:
\[
  (\lam{\var_1\hdots\var_n}{\redseq})\,\redseqtwo_1\hdots\redseqtwo_n
  \permeq
  \redseq\subrr{\var_1}{\redseqtwo_1}\hdots\subrr{\var_n}{\redseqtwo_n}
\]
\end{lem}
\begin{proof}
By induction on $n$.
The base case when $n = 0$ is immediate. In the inductive case:
\[
  \begin{array}{rcll}
  &&
    (\lam{\var_1\,\var_2\hdots\var_n}{\redseq})\,
      \redseqtwo_1\,\redseqtwo_2\hdots\redseqtwo_n
  \\
  & \permeq &
    ((\lam{\var_2\hdots\var_n}{\redseq})
       \subrr{\var_1}{\redseqtwo_1}
    )\,\redseqtwo_2\hdots\redseqtwo_n
    & \text{by \permeqRule{BetaRR}~(\rlem{betaRR})}
  \\
  & = &
    ((\lam{\var_2\hdots\var_n}{\redseq})
       \subt{\var_1}{\tmtwo_1}
     \seq
     (\lam{\var_2\hdots\var_n}{\tm})
       \subtr{\var_1}{\redseqtwo_1}
    )\,\redseqtwo_2\hdots\redseqtwo_n
  \\
  & = &
    ((\lam{\var_2\hdots\var_n}{\redseq\subt{\var_1}{\tmtwo_1}})
     \seq
     (\lam{\var_2\hdots\var_n}{\tm\subtr{\var_1}{\redseqtwo_1}})
    )\,\redseqtwo_2\hdots\redseqtwo_n
  \\
  & \permeq &
    (\lam{\var_2\hdots\var_n}{
       (\redseq\subt{\var_1}{\tmtwo_1}
       \seq
       \tm\subtr{\var_1}{\redseqtwo_1})
     })\,\redseqtwo_2\hdots\redseqtwo_n
    & \text{by \permeqRule{Abs} ($n-1$ times)}
  \\
  & = &
    (\lam{\var_2\hdots\var_n}{
       \redseq\subrr{\var_1}{\redseqtwo_1}
     })\,\redseqtwo_2\hdots\redseqtwo_n
    & \text{by definition}
  \\
  & = &
     \redseq\subrr{\var_1}{\redseqtwo_1}
            \subrr{\var_2}{\redseqtwo_2}
            \hdots
            \subrr{\var_n}{\redseqtwo_n}
    & \text{by \ih}
  \end{array}
\]
\end{proof}

\begin{prop}[Permutation]
\lprop{permutation}
Suppose that:
\begin{itemize}
\item
  $\judgRewr{\tenv}{\redseq}{
     \lam{\var_1\hdots\var_n}{\tm}
    }{
      \lam{\var_1\hdots\var_n}{\tm'}
    }{\typ_1 \imp \hdots \imp \typ_n \imp \typtwo}$
\item
  $\judgRewr{\tenv}{\redseqtwo_i}{\tmtwo_i}{\tmtwo'_i}{\typ_i}$
  for each $1 \leq i \leq n$.
\end{itemize}
Then:
\begin{enumerate}
\item
  $
    \redseq\,\redseqtwo_1\hdots\redseqtwo_n
    \permeq
    \redseq\,\tmtwo_1\hdots\tmtwo_n
    \seq
    \tm'\subrr{\var_1}{\redseqtwo_1}\hdots\subrr{\var_n}{\redseqtwo_n}
  $
\item
  $
    \redseq\,\redseqtwo_1\hdots\redseqtwo_n
    \permeq
    \tm\subrr{\var_1}{\redseqtwo_1}\hdots\subrr{\var_n}{\redseqtwo_n}
    \seq
    \redseq\,\tmtwo'_1\hdots\tmtwo'_n
  $
\end{enumerate}
\end{prop}
\begin{proof}
For item 1.:
\[
  \begin{array}{rcll}
    \redseq\,\redseqtwo_1\hdots\redseqtwo_n
  & \permeq &
    (\redseq\seq\lam{\var_1\hdots\var_n}{\tm'})\,
    \redseqtwo_1\hdots\redseqtwo_n
    & \text{by \permeqRule{IdR}}
  \\
  & \permeq &
    (\redseq\seq\lam{\var_1\hdots\var_n}{\tm'})\,
    (\tmtwo_1\seq\redseqtwo_1)\hdots(\tmtwo_n\seq\redseqtwo_n)
    & \text{by \permeqRule{IdL} ($n$ times)}
  \\
  & \permeq &
    (\redseq\,\tmtwo_1\hdots\tmtwo_n)\seq
    ((\lam{\var_1\hdots\var_n}{\tm'})\,\redseqtwo_1\hdots\redseqtwo_n)
    & \text{by generalized \permeqRule{App} (\rlem{generalized_seqr_transapp_rule})}
  \\
  & \permeq &
    (\redseq\,\tmtwo_1\hdots\tmtwo_n)\seq
    ((\lam{\var_1\hdots\var_n}{\tm'})\,\redseqtwo_1\hdots\redseqtwo_n)
    & \text{by \permeqRule{1Abs} ($n$ times)}
  \\
  & \permeq &
    (\redseq\,\tmtwo_1\hdots\tmtwo_n)\seq
    (\tm'\subrr{\var_1}{\redseqtwo_1}\hdots\subrr{\var_n}{\redseqtwo_n})
    & \text{by generalized \permeqRule{BetaRR} (\rlem{generalized_peqr_beta_rule})}
  \end{array}
\]
Item 2. is similar:
\[
  \begin{array}{rcll}
    \redseq\,\redseqtwo_1\hdots\redseqtwo_n
  & \permeq &
    ((\lam{\var_1\hdots\var_n}{\tm})\seq\redseq)\,
      \redseqtwo_1\hdots\redseqtwo_n
    & \text{by \permeqRule{IdL}}
  \\
  & \permeq &
    ((\lam{\var_1\hdots\var_n}{\tm})\seq\redseq)\,
      (\redseqtwo_1\seq\tmtwo'_1)\hdots(\redseqtwo_n\seq\tmtwo'_n)
    & \text{by \permeqRule{IdR} ($n$ times)}
  \\
  & \permeq &
    ((\lam{\var_1\hdots\var_n}{\tm})\,
     \redseqtwo_1\hdots\redseqtwo_n)
    \seq
    (\redseq\,\tmtwo'_1\hdots\tmtwo'_n)
    & \text{by generalized \permeqRule{App} (\rlem{generalized_seqr_transapp_rule})}
  \\
  & \permeq &
    ((\lam{\var_1\hdots\var_n}{\tm})\,
     \redseqtwo_1\hdots\redseqtwo_n)
    \seq
    (\redseq\,\tmtwo'_1\hdots\tmtwo'_n)
    & \text{by \permeqRule{1Abs} ($n$ times)}
  \\
  & \permeq &
    (\tm\subrr{\var}{\redseqtwo_1}\hdots\subrr{\var}{\redseqtwo_n})
    \seq
    (\redseq\,\tmtwo'_1\hdots\tmtwo'_n)
    & \text{by generalized \permeqRule{BetaRR} (\rlem{generalized_peqr_beta_rule})}
  \end{array}
\]
\end{proof}

\newpage
\subsection{Summary of properties of the substitution operators and $\permeq$}
\begin{framed}
\[
  \begin{array}{lr}
    \tm
      \subtr{\var}{\redseq}
      \subt{\vartwo}{\tmtwo}
    =
    \tm
      \subt{\vartwo}{\tmtwo}
      \subtr{\var}{\redseq\subt{\vartwo}{\tmtwo}}
  &
    (\rlem{subtr_subt_commutation_I})
  \\
    \refl{\tm}\subt{\var}{\tmtwo} = \refl{\tm\subt{\var}{\tmtwo}}
  &
    \text{(trivial)}
  \\
    \refl{\tm\subt{\var}{\tmtwo}} = \tm\subtr{\var}{\refl{\tmtwo}}
  &
    (\rlem{lifting_reflexivity})
  \\
    \tm \termeq \tm'
    \text{ implies }
    \refl{\tm} \permeq \refl{\tm'}
  &
    (\rlem{termeq_implies_permeq})
  \\
    \redseq \permeq \redseqtwo
    \text{ implies }
    \rsrc{\redseq} \termeq \rsrc{\redseqtwo}
    \text{ and }
    \rtgt{\redseq} \termeq \rtgt{\redseqtwo}
  &
    (\rlem{permeq_endpoints_are_termeq})
  \\
    \cctxof{\redseq\seq\redseqtwo} \permeq \cctxof{\redseq}\seq\cctxof{\redseqtwo}
  &
    (\rlem{permeq_distribute_cctx_over_seq})
  \\
    \tm\subtr{\var}{\redseq}\seq\tm\subtr{\var}{\redseqtwo}
    \permeq
    \tm\subtr{\var}{\redseq\seq\redseqtwo}
  &
    (\rlem{transitivity_lifting})
  \\
    (\lam{\var}{\redseq})\,\redseqtwo
    \permeq
    \redseq\subrr{\var}{\redseqtwo}
  &
    (\rlem{betaRR})
  \\
    \redseq\subt{\var}{\tmtwo}
    \permeq
    \redseq\subrr{\var}{\refl{\tmtwo}}
  &
    (\rremark{subrr_refl_R})
  \\
    \tm\subtr{\var}{\redseq}
    \permeq
    \refl{\tm}\subrr{\var}{\redseq}
  &
    (\rremark{subrr_refl_L})
  \\
    \redseq\subrr{\var}{\redseqtwo} \permeq \redseq
    \HS\text{if $\var\notin\fv{\redseq}$}
  &
    (\rlem{trivial_subrr_substitution})
  \\
    (\lam{\vartwo}{\redseq})\subrr{\var}{\redseqtwo}
    \permeq
    \lam{\vartwo}{\redseq\subrr{\vartwo}{\redseqtwo}}
  &
    (\rlem{subrr_recursion})
  \\
    (\redseq_1\,\redseq_2)\subrr{\var}{\redseqtwo}
    \permeq
    \redseq_1\subrr{\var}{\redseqtwo}\,\redseq_2\subrr{\var}{\redseqtwo}
  &
    (\rlem{subrr_recursion})
  \\
    \tm\subt{\var}{\tmfive}\subtr{\vartwo}{\redseqthree}
    \permeq
    \tm\subtr{\vartwo}{\redseqthree}\subrr{\var}{\tmfive\subtr{\vartwo}{\redseqthree}}
  &
    (\rlem{subtr_subt_commutation_II})
  \\
    \tm \termeq \tm'
    \text{ implies }
    \redseq\subt{\var}{\tm} \permeq \redseq\subt{\var}{\tm'}
  &
    (\rlem{congruence_termeq_subrt})
  \\
    \tm \termeq \tm'
    \text{ implies }
    \tm\subtr{\var}{\redseq} \permeq \tm'\subtr{\var}{\redseq}
  &
    (\rlem{congruence_termeq_subtr})
  \\
    \redseq \permeq \redseq'
    \text{ implies }
    \redseq\subt{\var}{\tm} \permeq \redseq'\subt{\var}{\tm}
  &
    (\rlem{congruence_permeq_subrt})
  \\
    \redseq \permeq \redseq'
    \text{ implies }
    \tm\subtr{\var}{\redseq} \permeq \tm\subtr{\var}{\redseq'}
  &
    (\rlem{congruence_permeq_subtr})
  \\
    \redseq \permeq \redseq'
    \text{ and }
    \redseqtwo \permeq \redseqtwo'
    \text{ imply }
    \redseq\subrr{\var}{\redseqtwo} \permeq \redseq'\subrr{\var}{\redseqtwo'}
  &
    (\rprop{congruence_permeq_subrr})
  \\
    \redseq\subt{\var}{\tmfive_0}\seq\tmfour_1\subtr{\var}{\redseqtwo}
    \permeq
    \tmfour_0\subtr{\var}{\redseqtwo}\seq\redseq\subt{\var}{\tmfive_1}
  &
    (\rlem{coherence})
  \\
    (\redseq_1\seq\redseq_2)\subrr{\var}{\redseqtwo_1\seq\redseqtwo_2}
    \permeq
    \redseq_1\subrr{\var}{\redseqtwo_1}\seq\redseq_2\subrr{\var}{\redseqtwo_2}
  &
    (\rprop{transitivity_subrr})
  \\
    \redseq
      \subrr{\var}{\redseqtwo}
      \subrr{\vartwo}{\redseqthree}
    \permeq
    \redseq
      \subrr{\vartwo}{\redseqthree}
      \subrr{\var}{\redseqtwo\subrr{\vartwo}{\redseqthree}}
  &
    (\rprop{substitution_property_for_subrr})
  \\
    (\redseq\,\redseqtwo_1\hdots\redseqtwo_n) \seq
    (\redseq'\,\redseqtwo'_1\hdots\redseqtwo'_n)
    \permeq
    (\redseq\seq\redseq')\,
    (\redseqtwo_1\seq\redseqtwo'_1)\hdots
    (\redseqtwo_n\seq\redseqtwo'_n)
  &
    (\rlem{generalized_seqr_transapp_rule})
  \\
    (\lam{\var_1\hdots\var_n}{\redseq})\,\redseqtwo_1\hdots\redseqtwo_n
    \permeq
    \redseq\subrr{\var_1}{\redseqtwo_1}\hdots\subrr{\var_n}{\redseqtwo_n}
  &
    (\rlem{generalized_peqr_beta_rule})
  \\
    \redseq\,\redseqtwo_1\hdots\redseqtwo_n
    \permeq
    \redseq\,\tmtwo_1\hdots\tmtwo_n
    \seq
    \tm'\subrr{\var_1}{\redseqtwo_1}\hdots\subrr{\var_n}{\redseqtwo_n}
  &
    (\rprop{permutation})
  \\
    \redseq\,\redseqtwo_1\hdots\redseqtwo_n
    \permeq
    \tm\subrr{\var_1}{\redseqtwo_1}\hdots\subrr{\var_n}{\redseqtwo_n}
    \seq
    \redseq\,\tmtwo'_1\hdots\tmtwo'_n
  &
    (\rprop{permutation})
  \end{array}
\]
\end{framed}
\newpage

%%% Local Variables:
%%% mode: latex
%%% TeX-master: "main"
%%% End:
