# Supplementary material for: Reductions in Higher-Order Rewriting and Their Equivalence
Source: arXiv:2210.15654 source file (2023-08-15)
Supplement: Supplementary file 3 [file a03-restricted_eta_expansion.tex]

Recall from~\rdef{notions_of_contexts}
the notions of rewrite context ($\rctx$, $\rctx'$, $\hdots$),
applicative rewrite context and
strongly applicative term context.

\begin{defi}
The relation of {\em restricted $\eta$-expansion}
written $\toetaexp$, is defined as follows.
\smallskip\\
Let $\rctxof{\redseq}$ be a rewrite such that
$\redseq$ is of function type (\ie $\typ \imp \typtwo$),
$\rctx$ is not applicative and
$\redseq$ is not a $\lambda$-abstraction nor a composition~(``$\seq$'').
Then given a variable $\var\notin\fv{\redseq}$: \[
  \rctxof{\redseq} \toetaexp \rctxof{\lam{\var}{\redseq\,\var}}
\]
Observe that this notion is {\bf not} closed by arbitrary contexts.
\end{defi}

\begin{rem}
If $\redseq \toetaexp \redseqtwo$
then $\redseq \permeq \redseqtwo$
using the \permeqRule{Eta} rule.
\end{rem}

\begin{prop}
\lprop{restricted_eta_expansion_sn_cr}
Restricted $\eta$-expansion is SN and CR.
\end{prop}
\begin{proof}
{\bf Strong normalization.}
An {\em $\etalong$-redex occurrence} of a rewrite $\redseq$
is a pair $(\rctx,\redseq')$
such that $\rctxof{\redseq'} = \redseq$
where $\redseq$ is of function type, $\rctx$ is not applicative
and $\redseq'$ is not a $\lambda$-abstraction nor a composition.
The {\em degree} of a redex occurrence is the size of
the type $\typ \imp \typtwo$.
The {\em measure} of a rewrite $\redseq$ is the multiset of
all the degrees of redex occurrences of $\redseq$.
To prove strong normalization,
observe that $\etalong$-expansion decreases the measure of the rewrite.
In fact, suppose that there is a step:
\[
  \rctxof{\redseq} \toetaexp \rctxof{\lam{\var}{\redseq\,\var}}
\]
where the type of $\redseq$ is $\typ \imp \typtwo$.
Consider a redex occurrence $(\rctx',\redseq')$ of the right-hand side,
\ie $\rctxof{\lam{\var}{\redseq\,\var}} = \rctx'\ctxof{\redseq'}$
where $\redseq'$ is of function type,
$\rctx'$ is not applicative,
and $\redseq'$ is not a $\lambda$-abstraction nor a composition.
We claim that either the degree of $(\rctx',\redseq')$
is strictly less than the degree of $(\rctx,\redseq)$
or, otherwise, that $(\rctx',\redseq')$
can be mapped injectively to a redex occurrence $(\rctx'',\redseq'')$
on the left-hand side.
Note that $\rctx \neq \rctx'$ because $\lam{\var}{\redseq\,\var}$
is a $\lambda$-abstraction so $(\rctx,\lam{\var}{\redseq\,\var})$ is not
a redex occurrence.
We consider three cases, depending on whether the contexts
$\rctx$, $\rctx'$ are disjoint,
$\rctx$ is a prefix of $\rctx'$, or
$\rctx'$ is a prefix of $\rctx$:
\begin{enumerate}
\item
  If $\rctx$ and $\rctx'$ are disjoint, then
  there is a two-hole context $\hat{\rctx}$ such that
  $\rctx = \hat{\rctx}\ctxof{\ctxhole,\redseq'}$
  and
  $\rctx' = \hat{\rctx}\ctxof{(\lam{\var}{\redseq\,\var}),\ctxhole}$.
  Then $(\rctx',\redseq')$ can be mapped to the redex occurrence
  $(\hat{\rctx}\ctxof{\redseq,\ctxhole}, \redseq')$ on the left-hand side.
\item
  If $\rctx$ is a prefix of $\rctx'$,
  then $\rctx' = \rctxof{\rctx''}$
  and $\lam{\var}{\redseq\,\var} = \rctx''\ctxof{\redseq'}$.
  Note that $\rctx''$ is not empty because, as we have already argued,
  $\rctx \neq \rctx'$.
  We proceed by case analysis on the shape of $\rctx''$;
  \begin{enumerate}
  \item
    If $\rctx'' = \lam{\var}{\ctxhole}$,
    then $(\rctxof{\lam{\var}{\ctxhole}},\redseq\,\var)$
    is a redex occurrence
    with degree strictly less than the degree of $(\rctx,\redseq)$,
    given that the type of $\redseq\,\var$ is $\typtwo$.
  \item
    If $\rctx'' = \lam{\var}{\rctx'''\,\var}$,
    then $(\rctxof{\lam{\var}{\rctx'''\,\var}},\redseq')$
    can be mapped to the redex occurrence $(\rctxof{\rctx'''},\redseq')$
    on the left-hand side.
    Note that if $\rctxof{\lam{\var}{\rctx'''\,\var}}$
    is not applicative, then $\rctxof{\rctx'''}$ is also not applicative.
  \item
    If $\rctx'' = \lam{\var}{\redseq\,\ctxhole}$,
    then $(\rctxof{\lam{\var}{\redseq\,\ctxhole}},\var)$
    is a redex occurrence
    with degree strictly less than the degree of $(\rctx,\redseq)$,
    given that the type of $\var$ is $\typ$.
  \end{enumerate}
\item
  If $\rctx'$ is a prefix of $\rctx$,
  then $\rctx = \rctx'\ctxof{\rctx''}$
  and $\redseq' = \rctx''\ctxof{\lam{\var}{\redseq\,\var}}$.
  Then $(\rctx',\rctx''\ctxof{\lam{\var}{\redseq\,\var}})$
  can be mapped to the redex occurrence
  $(\rctx',\rctx''\ctxof{\redseq})$
  on the left-hand side.
  Note that if $\rctx''\ctxof{\lam{\var}{\redseq\,\var}}$ is not
  a $\lambda$-abstraction nor a composition
  then $\rctx''$ is non-empty, and the outermost constructor is
  an application,
  hence $\rctx''\ctxof{\redseq}$ is also not a $\lambda$-abstraction nor
  a composition.
\end{enumerate}
The mapping thus defined is injective.
\smallskip\\
{\bf Confluence.}
By Newman's lemma, it suffices to show that restricted $\eta$-expansion is WCR.
Indeed, suppose that $\redseq \toetaexp \redseq_1$
and $\redseq \toetaexp \redseq_2$,
and let us show that there is a rewrite $\redseq_3$
such that $\redseq_1 \toetaexp^* \redseq_3$
and $\redseq_2 \toetaexp^* \redseq_3$.
More precisely, let:
\[
  \begin{array}{rcll}
    \redseq = \rctx_1\ctxof{\redseq'_1}
  & \toetaexp &
    \rctx_1\ctxof{\lam{\var}{\redseq'_1\,\var}} = \redseq_1
    & \text{for $\var \notin \fv{\redseq'_1}$}
  \\
    \redseq = \rctx_2\ctxof{\redseq'_2}
  & \toetaexp &
    \rctx_2\ctxof{\lam{\vartwo}{\redseq'_2\,\vartwo}} = \redseq_2
    & \text{for $\vartwo \notin \fv{\redseq'_2}$}
  \end{array}
\]
where the contexts $\rctx_1,\rctx_2$ are not applicative,
and the rewrites $\redseq_1,\redseq_2$ are of function type
and not abstractions nor compositions.
If $\rctx_1 = \rctx_2$ then it is trivial to conclude in zero
rewriting steps.
Otherwise, there are three subcases,
depending on whether the contexts $\rctx_1,\rctx_2$ are disjoint,
or $\rctx_1$ is a prefix of $\rctx_2$,
or $\rctx_2$ is a prefix of $\rctx_1$.
The last two cases are symmetric so we only consider the first one:
\begin{enumerate}
\item
  If $\rctx_1$ and $\rctx_2$ are disjoint,
  then there is a two-hole context $\hat{\rctx}$
  such that $\rctx_1 = \hat{\rctx}\ctxof{\ctxhole,\redseq'_2}$
  and $\rctx_2 = \hat{\rctx}\ctxof{\redseq'_1,\ctxhole}$.
  Then the situation is:
  \[
    \xymatrix{
      \hat{\rctx}\ctxof{\redseq'_1,\redseq'_2}
      \ar[r] \ar[d]
    &
      \hat{\rctx}\ctxof{(\lam{\var}{\redseq'_1\,\var}),\redseq'_2}
      \ar[d]
    \\
      \hat{\rctx}\ctxof{\redseq'_1,(\lam{\vartwo}{\redseq'_2\,\vartwo})}
      \ar[r]
    &
      \hat{\rctx}\ctxof{(\lam{\var}{\redseq'_1\,\var}),(\lam{\vartwo}{\redseq'_2\,\vartwo)}}
    }
  \]
  To be able to close the diagram,
  note that $\hat{\rctx}\ctxof{\ctxhole,\redseq'_2}$
  is applicative if and only if
  $\hat{\rctx}\ctxof{\ctxhole,(\lam{\vartwo}{\redseq'_2})}$
  is applicative.
  Similarly,
  $\hat{\rctx}\ctxof{\redseq'_1,\ctxhole}$
  is applicative if and only if
  $\hat{\rctx}\ctxof{(\lam{\var}{\redseq'_1\,\var}),\ctxhole}$
  is applicative.
\item
  If $\rctx_1$ is a prefix of $\rctx_2$,
  then $\rctx_2 = \rctx_1\ctxof{\rctx'}$
  and $\redseq'_1 = \rctx'\ctxof{\redseq'_2}$.
  Then the situation is:
  \[
    \xymatrix{
      \rctx_1\ctxof{\rctx'\ctxof{\redseq'_2}}
      \ar[r] \ar[d]
    &
      \rctx_1\ctxof{\lam{\var}{\rctx'\ctxof{\redseq'_2}\,\var}}
      \ar[d]
    \\
      \rctx_1\ctxof{\rctx'\ctxof{\lam{\vartwo}{\redseq'_2\,\vartwo}}}
      \ar[r]
    &
      \rctx_1\ctxof{\lam{\var}{\rctx'\ctxof{\lam{\vartwo}{\redseq'_2\,\vartwo}}\,\var}}
    }
  \]
  To justify the step on the right-hand side of the diagram,
  note that $\rctx'$ is not empty because we already know that
  $\rctx_1 \neq \rctx_2$.
  Moreover, the outermost constructor of $\rctx'$ cannot be a
  $\lambda$-abstraction nor a composition, because
  $\redseq_1 = \rctx'\ctxof{\redseq'_2}$ is not a $\lambda$-abstraction
  nor a composition.
  This means that $\rctx'$ must be either of the form $\rctx''\,\redseqtwo$
  or of the form $\redseqtwo\,\rctx''$ and it is not applicative.
  Hence, in any of these two cases, the context
  $\rctx_1\ctxof{\lam{\var}{\rctx'\,\var}}$ is not applicative.
  \smallskip\\
  To justify the step on the bottom of the diagram,
  note, again, that $\rctx'$ is non-empty and its outermost
  constructor is an application,
  hence
  $\rctx'\ctxof{\lam{\vartwo}{\redseq'_2\,\vartwo}}$
  is not a $\lambda$-abstraction nor a composition.
\end{enumerate}
\end{proof}

\subsection{$\etalong$-normal forms}

\begin{defi}[$\etalong$-normal form]
We recall the standard notion of $\etalong$-normal form
for terms: a typable term $\judgTerm{\tenv}{\tm}{\typ}$.
is in {\em $\etalong$-normal form}
if whenever $\tm$ can be written as of the form
$\tm = \cctxof{\tm'}$ such that $\tm'$ is of function type
(\ie $\typ \imp \typtwo$)
then either $\cctx$ is strongly applicative or
$\tm'$ is a $\lambda$-abstraction.

The notion is extended for rewrites as follows.
A typable rewrite $\judgRewr{\tenv}{\redseq}{\tm}{\tmtwo}{\typ}$
is in {\em $\etalong$-normal form}
if whenever $\redseq$ can be written as of the form
$\redseq = \rctxof{\redseq'}$ such that $\redseq'$ is of function type
(\ie $\typ \imp \typtwo$)
then either $\rctx$ is applicative
or $\redseq'$ is a $\lambda$-abstraction or a composition.
\end{defi}

\begin{rem}
A rewrite is in $\etalong$-normal form precisely
if it is a normal form for $\toetaexp$.
\end{rem}

\begin{rem}
A term $\tm$ is in $\etalong$-normal form in the standard sense
if and only if the corresponding rewrite $\refl{\tm}$
is in $\etalong$-normal form.
This is a consequence of the two following observations:
\begin{enumerate}
\item
  A term context $\cctx$ is applicative
  if and only if it is strongly applicative,
  given that it has no compositions.
\item
  A term $\tm$ has no compositions.
\end{enumerate}
\end{rem}

\begin{defi}[$\etalong$-condition]
The set of rewriting rule symbols $\ruleset$
is said to verify the {\em $\etalong$-condition}
if for every $\rewr{\rulewit}{\tm}{\tmtwo}{\typ} \in \ruleset$.
the terms $\tm$ and $\tmtwo$ are in $\etalong$-normal form.
\end{defi}

\begin{lem}[Endpoints of rewrites in $\etalong$-normal form]
\llem{source_target_of_etalong_rewrite}
Assume that the set of rewriting rule symbols $\ruleset$ verifies the
$\etalong$-condition.
Let $\judgRewr{\tenv}{\redseq}{\tm}{\tmtwo}{\typ}$
be a rewrite in $\etalong$-normal form.
Then $\refl{\rsrc{\redseq}}$ and $\refl{\rtgt{\redseq}}$
are in $\etalong$-normal form.
\end{lem}
\begin{proof}
Let us prove that the source $\refl{\rsrc{\redseq}}$
is in $\etalong$-normal form;
the proof for the target $\refl{\rtgt{\redseq}}$ is similar.
By contradiction, suppose that $\refl{\rsrc{\redseq}}$
is not in $\etalong$-normal form.
Note that $\rsrc{\redseq}$ is of the form $\cctxof{\tm}$
where $\cctx$ is not applicative
and $\tm$ is not a $\lambda$-abstraction nor a composition.
Since $\rsrc{\redseq}$ is a term, without compositions~(``$\seq$''),
this means that $\tm$ is not a $\lambda$-abstraction
and that $\cctx$ is not strongly applicative.
By \rlem{source_target_contextual_decomposition} there are two
possibilities:
\begin{itemize}
\item[(A)]
  In this case, $\redseq = \rctxof{\iredseq}$
  where $\rsrc{\rctx} = \cctx$ and $\rsrc{\iredseq} = \tm$.
  Suppose, without loss of generality,
  that $\iredseq$ is the smallest possible term that satisfies
  these equations.
  In particular, note that $\iredseq$ cannot be a composition
  $(\iredseq_1\seq\iredseq_2)$,
  because this would allow us to write $\redseq = \rctx'\ctxof{\iredseq_1}$
  with $\rctx' := \rctxof{\ctxhole\seq\iredseq_2}$
  and this also verifies the equations.

  Then $\rctx$ is not applicative,
  as this would imply that $\cctx$ is applicative.
  Note that $\iredseq$ is not a $\lambda$-abstraction,
  as this would imply that $\tm$ is a $\lambda$-abstraction.
  Finally, $\iredseq$ is not a composition,
  as we have already noted.
  This contradicts the fact that $\redseq$ is in $\etalong$-normal form.
\item[(B)]
  In this case, $\redseq = \rctxof{\rulewit}$
  where $\rsrc{\rctx} = \cctx_1$ and $\rsrc{\rulewit} = \cctx_2\ctxof{\tm}$
  and $\cctx = \cctx_1\ctxof{\cctx_2}$.
  Note that $\cctx_2$ is not strongly applicative, as this would imply
  that $\cctx$ is strongly applicative.
  Moreover, as already noted before, $\tm$ is not a $\lambda$-abstraction.
  This means that $\rsrc{\rulewit}$ is not in $\etalong$-normal form,
  contradicting the hypothesis that
  the set of rewriting rule symbols $\ruleset$ verifies the $\etalong$-condition.
\end{itemize}
\end{proof}
