# Supplementary material for: Reductions in Higher-Order Rewriting and Their Equivalence
Source: arXiv:2210.15654 source file (2023-08-15)
Supplement: Supplementary file 4 [file a04-flattening.tex]

\begin{lem}[Typing rule for multistep substitution]
If $\judgRewr{\tenv,\var:\typ}{\mstep}{\tm_0}{\tm_1}{\typtwo}$
and $\judgRewr{\tenv}{\msteptwo}{\tmtwo_0}{\tmtwo_1}{\typ}$
then $\judgRewr{\tenv}{
        \mstep\subm{\var}{\msteptwo}
      }{
        \tm_0\subt{\var}{\tmtwo_0}
      }{
        \tm_1\subt{\var}{\tmtwo_1}
      }{\typtwo}$.
\end{lem}
\begin{proof}
Straightforward by induction on the derivation of the judgment.
\end{proof}

\begin{lem}[Substitution lemma for multisteps]
\llem{multistep_substitution_lemma}
The following substitution property holds:
\[
  \mstep\subm{\var}{\msteptwo}\subm{\vartwo}{\msteptwo'}
  =
  \mstep\subm{\vartwo}{\msteptwo'}
        \subm{\var}{\msteptwo\subm{\vartwo}{\msteptwo'}}
\]
Note, in particular, that
$\mstep\subm{\var}{\msteptwo}\subt{\vartwo}{\tm} =
 \mstep\subt{\vartwo}{\tm}\subm{\var}{\msteptwo\subt{\vartwo}{\tm}}$.
\end{lem}
\begin{proof}
Routine by induction on $\mstep$.
\end{proof}

\subsection{Termination of flattening}

% \begin{rem}
% \lremark{flat_not_beta_steps_preserve_endpoints}
% If $\redseq \tof_{\flatRuleAnon} \redseqtwo$
% and $\flatRuleAnon \notin \set{\flatRule{BetaM},\flatRule{EtaM}}$
% then $\rsrc{\redseq} = \rsrc{\redseqtwo}$
% and $\rtgt{\redseq} = \rtgt{\redseqtwo}$.
% \end{rem}

\begin{rem}
\lremark{flatten_not_beta_eta_not_multisteps}
Let $\redseq \tof_{\flatRuleAnon} \redseqtwo$
where $\flatRuleAnon \neq \set{\flatRule{BetaM},\flatRule{EtaM}}$.
Then neither $\redseq$ nor $\redseqtwo$ are multisteps.
Indeed, note that,
in all the rules other than \flatRule{BetaM} and \flatRule{EtaM},
there must be
at least one composition~(``$\seq$'') on the left-hand side,
and
at least one composition on the right-hand side.
\end{rem}

\begin{lem}
\llem{subm_source_target}
Let $\mstep,\msteptwo$ be arbitrary multisteps. Then:
\begin{enumerate}
\item
  $\rsrc{\mstep\subm{\var}{\msteptwo}} =
   \rsrc{\mstep}\subm{\var}{\rsrc{\msteptwo}}$
\item
  $\rtgt{\mstep\subm{\var}{\msteptwo}} =
   \rtgt{\mstep}\subm{\var}{\rtgt{\msteptwo}}$
\end{enumerate}
\end{lem}
\begin{proof}
Straightforward by induction on $\mstep$.
\end{proof}

\begin{lem}
\llem{flatten_beta_eta_source_target}
If $\redseq \tof_{\flatRuleAnon} \redseqtwo$
where $\flatRuleAnon \in \set{\flatRule{BetaM},\flatRule{EtaM}}$,
then $\refl{\rsrc{\redseq}} \tofeqSub{\flatRuleAnon} \refl{\rsrc{\redseqtwo}}$
and $\refl{\rtgt{\redseq}} \tofeqSub{\flatRuleAnon} \refl{\rtgt{\redseqtwo}}$.\\
Here $\tofeqSub{\flatRuleAnon}$ denotes
the {\em reflexive} closure of $\tof_{\flatRuleAnon}$.
\end{lem}
\begin{proof}
By induction on $\redseq$:
\begin{enumerate}
\item
  {\bf Variable ($\redseq = \var$), constant ($\redseq = \cons$),
      or rule symbol ($\redseq = \rulewit$).}
  There cannot be a step $\redseq \tof_{\flatRuleAnon} \redseqtwo$
  using the $\flatRule{BetaM}$ or $\flatRule{EtaM}$
  rules, so this case trivially holds.
\item
  {\bf Abstraction ($\redseq = \lam{\var}{\redseq'}$).}
  There are two subcases, depending on whether the step takes place
  at the root or under the abstraction:
  \begin{enumerate}
  \item Reduction at the root:
    then $\redseq'$ is a multistep of the form $\mstep\,\var$
    where $\var\notin\fv{\mstep}$,
    and the step is of the form
    $\lam{\var}{\mstep\,\var} \tof_{\flatRule{EtaM}} \mstep$.
    Then for the source we have that
    $\lam{\var}{\rsrc{\mstep}\,\var} \tof_{\flatRule{EtaM}} \rsrc{\mstep}$,
    observing that $\var$ cannot occur free in $\rsrc{\mstep}$,
    and similarly for the target.
  \item Under the abstraction:
    then the step is of the form
    $\lam{\var}{\redseq'} \tof_{\flatRuleAnon} \lam{\var}{\redseqtwo'}$
    with $\redseq' \tof_{\flatRuleAnon} \redseqtwo'$.
    By \ih we have that
    $\refl{\rsrc{\redseq'}} \tofeqSub{\flatRuleAnon} \refl{\rsrc{\redseqtwo'}}$
    so also
    $\refl{\lam{\var}{\rsrc{\redseq'}}} \tofeqSub{\flatRuleAnon}
     \refl{\lam{\var}{\rsrc{\redseqtwo'}}}$,
    and similarly for the target.
  \end{enumerate}
\item
  {\bf Application ($\redseq = \redseq_1\,\redseq_2$).}
  There are three subcases, depending on whether the step takes
  place at the root, to the left, or to the right of the application:
  \begin{enumerate}
  \item Reduction at the root:
    then $\redseq_1$ and $\redseq_2$ must be multisteps
    of the forms $\redseq_1 = \lam{\var}{\mstep}$
    and $\redseq_2 = \msteptwo$,
    and the step is of the form
    $(\lam{\var}{\mstep})\,\msteptwo \tof_{\flatRule{BetaM}}
     \mstep\subm{\var}{\msteptwo}$.
    Then for the source we have that 
    $(\lam{\var}{\rsrc{\mstep}})\,\rsrc{\msteptwo}
     \tof_{\flatRule{BetaM}}
     \rsrc{\mstep}\subm{\var}{\rsrc{\msteptwo}} =
     \rsrc{\mstep\subm{\var}{\msteptwo}}$
    by \rlem{subm_source_target},
    and similarly for the target.
  \item Left of the application:
    then the step is of the form
    $\redseq_1\,\redseq_2 \tof_{\flatRuleAnon} \redseq'_1\,\redseq_2$
    with $\redseq_1 \tof_{\flatRuleAnon} \redseq'_1$.
    By \ih we have that
    $\refl{\rsrc{\redseq_1}}
     \tofeqSub{\flatRuleAnon} \refl{\rsrc{{\redseq'_1}}}$
    so also
    $\refl{\rsrc{\redseq_1}}\,\refl{\rsrc{\redseq_2}}
     \tofeqSub{\flatRuleAnon} \refl{\rsrc{{\redseq'_1}}}\,\refl{\rsrc{\redseq_2}}$,
    and similarly for the target.
  \item Right of the application:
    symmetric to the previous case.
  \end{enumerate}
\item
  {\bf Composition, ($\redseq = \redseq_1\seq\redseq_2$).}
  There are two subcases, depending on whether the step takes
  place to the left or to the right of the composition:
  \begin{enumerate}
  \item Left of the composition:
    then the step
    is of the form $\redseq_1\seq\redseq_2
                    \tof_{\flatRuleAnon} \redseq'_1\seq\redseq_2$
    with $\redseq_1 \tof_{\flatRuleAnon} \redseq'_1$.
    For the source,
    note that by \ih we have that
    $\refl{\rsrc{\redseq_1}} \tofeqSub{\flatRuleAnon} \refl{\rsrc{{\redseq'_1}}}$
    so indeed
    $\refl{\rsrc{(\redseq_1\seq\redseq_2)}}
     = \refl{\rsrc{\redseq_1}}
     \tofeqSub{\flatRuleAnon} \refl{\rsrc{{\redseq'_1}}}
     = \refl{\rsrc{(\redseq'_1\seq\redseq_2)}}$.
    For the target,
    simply note that
    $\refl{\rtgt{(\redseq_1\seq\redseq_2)}}
     = \refl{\rtgt{\redseq_2}}
     = \refl{\rtgt{(\redseq'_1\seq\redseq_2)}}$,
    so we conclude in zero reduction steps.
  \item Right of the composition:
    symmetric to the previous case.
  \end{enumerate}
\end{enumerate}
\end{proof}

\begin{rem}
\lremark{rheavy_multisteps_and_terms}
Multisteps and (lifted) terms have no heavy applications,
\ie $\rheavy{\mstep} = 0$ and $\rheavy{\refl{\tm}} = 0$.
\end{rem}

\begin{lem}[Decrease of heavy applications]
\llem{rheavy_decrease}
Let $\redseq \tof_{\flatRuleAnon} \redseqtwo$
where $\flatRuleAnon \notin \set{\flatRule{BetaM},\flatRule{EtaM}}$.
Then $\rheavy{\redseq} \geq \rheavy{\redseqtwo}$.
Furthermore if $\flatRuleAnon = \flatRule{App3}$
then $\rheavy{\redseq} > \rheavy{\redseqtwo}$.
\end{lem}
\begin{proof}
By induction on the context under which the 
step $\redseq \tof_{\flatRuleAnon} \redseqtwo$ takes place.
We consider all the cases for reduction at the root
as well as for congruence closure:
\begin{enumerate}
\item {\bf Root \flatRule{Abs} step.}
  Let $\lam{\var}{(\redseq\seq\redseqtwo)}
       \tof_{\flatRule{Abs}} (\lam{\var}{\redseq})\seq(\lam{\var}{\redseqtwo})$.
  Then
  $\rheavy{\lam{\var}{(\redseq\seq\redseqtwo)}}
   = \rheavy{\redseq} + \rheavy{\redseqtwo}
   = \rheavy{(\lam{\var}{\redseq})\seq(\lam{\var}{\redseqtwo})}$.
\item {\bf Root \flatRule{App1} step.}
  Let $(\redseq\seq\redseqtwo)\,\mstep
       \tof_{\flatRule{App1}}
       (\redseq\,\refl{\rsrc{\mstep}})\seq(\redseqtwo\,\mstep)$.
  Note that all the explicitly written applications,
  \ie $(\redseq\seq\redseqtwo)\,\mstep$,
  and $\redseq\,\refl{\rsrc{\mstep}}$,
  and $\redseqtwo\,\mstep$ are not heavy.
  Hence, using the fact that multisteps and terms have no heavy 
  applications (\rremark{rheavy_multisteps_and_terms})
  we have that
  $\rheavy{(\redseq\seq\redseqtwo)\,\mstep}
   = \rheavy{\redseq} + \rheavy{\redseqtwo}
   = \rheavy{(\redseq\,\refl{\rsrc{\mstep}})\seq(\redseqtwo\,\mstep)}$.
\item {\bf Root \flatRule{App2} step.}
  Symmetric to the previous case.
\item {\bf Root \flatRule{App3} step.}
  Let $(\redseq_1\seq\redseq_2)\,(\redseqtwo_1\seq\redseqtwo_2)
       \tof_{\flatRule{App3}}
       ((\redseq_1\seq\redseq_2)\,\refl{\rsrc{\redseqtwo_1}})\seq
       (\refl{\rtgt{\redseq_2}}\,(\redseqtwo_1\seq\redseqtwo_2))$.
  Note that the explicitly written application on the left-hand side,
  \ie $(\redseq_1\seq\redseq_2)\,(\redseqtwo_1\seq\redseqtwo_2)$
  is heavy, whereas the explicitly written applications
  on the right-hand side, \ie
  $(\redseq_1\seq\redseq_2)\,\refl{\rsrc{\redseqtwo_1}}$
  and
  $\refl{\rtgt{\redseq_2}}\,(\redseqtwo_1\seq\redseqtwo_2)$,
  are not heavy.
  Hence
  $\rheavy{(\redseq_1\seq\redseq_2)\,(\redseqtwo_1\seq\redseqtwo_2)}
   = 1 + \rheavy{\redseq_1} + \rheavy{\redseq_2}
       + \rheavy{\redseqtwo_1} + \rheavy{\redseqtwo_2}
   >   \rheavy{\redseq_1} + \rheavy{\redseq_2}
     + \rheavy{\redseqtwo_1} + \rheavy{\redseqtwo_2}
   = \rheavy{
       ((\redseq_1\seq\redseq_2)\,\refl{\rsrc{\redseqtwo_1}})\seq
       (\refl{\rtgt{\redseq_2}}\,(\redseqtwo_1\seq\redseqtwo_2))
     }$.
\item
  {\bf Congruence, under an abstraction.}
  let $\lam{\var}{\redseq} \tof_{\flatRuleAnon} \lam{\var}{\redseqtwo}$
  with $\redseq \tof_{\flatRuleAnon} \redseqtwo$.
  Note that $\rheavy{\lam{\var}{\redseq}} = \rheavy{\redseq}$
  and $\rheavy{\lam{\var}{\redseqtwo}} = \rheavy{\redseqtwo}$,
  so it is immediate to conclude by resorting to the \ih.
\item
  {\bf Congruence, left of an application.}
  let $\redseq\,\iredseq \tof_{\flatRuleAnon} \redseqtwo\,\iredseq$
  with $\redseq \tof_{\flatRuleAnon} \redseqtwo$.
  Recall that in a reduction step
  (other than \flatRule{BetaM} and \flatRule{EtaM})
  the left and the right-hand sides are not multisteps
  (\rremark{flatten_not_beta_eta_not_multisteps}).
  This implies that $\redseq$ and $\redseqtwo$ are not multisteps.
  This means that the application $\redseq\,\iredseq$ is heavy
  if and only if the application $\redseqtwo\,\iredseq$ is heavy.
  Let $k := 1$ if $\redseq\,\iredseq$ is heavy,
  and $k := 0$ otherwise.
  We have that
  $\rheavy{\redseq\,\iredseq} = k + \rheavy{\redseq} + \rheavy{\iredseq}$
  and
  $\rheavy{\redseqtwo\,\iredseq} = k + \rheavy{\redseqtwo} + \rheavy{\iredseq}$.
  Hence it is immediate to conclude by resorting to the \ih.
\item
  {\bf Congruence, right of an application.}
  Symmetric to the previous case.
\item
  {\bf Congruence, left of a composition.}
  Let $\redseq\seq\iredseq \tof_{\flatRuleAnon} \redseqtwo\seq\iredseq$
  with $\redseq \tof_{\flatRuleAnon} \redseqtwo$.
  Then $\rheavy{\redseq\seq\iredseq} = \rheavy{\redseq}$
  and $\rheavy{\redseqtwo\seq\iredseq} = \rheavy{\redseqtwo}$,
  so it is immediate to conclude by resorting to the \ih.
\item
  {\bf Congruence, right of a composition.}
  Symmetric to the previous case.
\end{enumerate}
\end{proof}

% \begin{defi}
% The {\em weight} of a rewrite $\redseq$
% is a non-negative integer $\rweight{\redseq}$
% defined inductively as follows:
% \[
%   \begin{array}{rcll}
%     \rweight{\var} = \rweight{\cons} = \rweight{\rulewit} & \eqdef & 0 \\
%     \rweight{\lam{\var}{\redseq}} & \eqdef & 2\,\rweight{\redseq} \\
%     \rweight{\redseq\,\redseqtwo} & \eqdef &
%       2\,\rweight{\redseq} + 2\,\rweight{\redseqtwo}
%     \\
%     \rweight{\redseq\seq\redseqtwo} & \eqdef &
%       1 + \rweight{\redseq} + \rweight{\redseqtwo}
%   \end{array}
% \]
% \end{defi}

% \begin{rem}
% \lremark{rweight_multisteps_and_terms}
% Multisteps and (lifted) terms have zero weight,
% \ie $\rweight{\mstep} = 0$ and $\rweight{\refl{\tm}} = 0$.
% \end{rem}

\begin{lem}[Decrease of weight]
\llem{rweight_decrease}
Let $\redseq \tof_{\flatRuleAnon} \redseqtwo$
where $\flatRuleAnon \in \set{\flatRule{Abs},\flatRule{App1},\flatRule{App2}}$.
Then $\rweight{\redseq} > \rweight{\redseqtwo}$.
\end{lem}
\begin{proof}
By induction on the context under which the 
step $\redseq \tof_{\flatRuleAnon} \redseqtwo$ takes place.
We consider all the cases for reduction at the root
as well as for congruence closure:
\begin{enumerate}
\item {\bf Root \flatRule{Abs} step.}
  Let $\lam{\var}{(\redseq\seq\redseqtwo)}
       \tof_{\flatRule{Abs}} (\lam{\var}{\redseq})\seq(\lam{\var}{\redseqtwo})$.
  Then:
  \[
    \begin{array}{rcl}
      \rweight{\lam{\var}{(\redseq\seq\redseqtwo)}}
    & = &
       2\,(1 + \rweight{\redseq} + \rweight{\redseqtwo})
    \\
    & > &
      1 + 2\,\rweight{\redseq} + 2\,\rweight{\redseqtwo}
    \\
    & = &
      \rweight{(\lam{\var}{\redseq})\seq(\lam{\var}{\redseqtwo})}
    \end{array}
  \]
\item {\bf Root \flatRule{App1} step.}
  Let $(\redseq\seq\redseqtwo)\,\mstep
       \tof_{\flatRule{App1}}
       (\redseq\,\refl{\rsrc{\mstep}})\seq(\redseqtwo\,\mstep)$.
  Then:
  \[
    \begin{array}{rcll}
      \rweight{(\redseq\seq\redseqtwo)\,\mstep}
    & = &
      2\,(1 + \rweight{\redseq} + \rweight{\redseqtwo}) + 2\,\rweight{\mstep}
    \\
    & > &
      1 + 2\,\rweight{\redseq} + 2\,\rweight{\redseqtwo} + 2\,\rweight{\mstep}
    \\
    & = &
      1 + 2\,\rweight{\redseq} + 2\,\rweight{\refl{\rsrc{\mstep}}}
        + 2\,\rweight{\redseqtwo} + 2\,\rweight{\mstep}
      & \text{by \rremark{rweight_multisteps_and_terms}}
    \\
    & = &
      \rweight{(\redseq\,\refl{\rsrc{\mstep}})\seq(\redseqtwo\,\mstep)}
    \end{array}
  \]
\item {\bf Root \flatRule{App2} step.}
  Symmetric to the previous case.
\item {\bf Congruence closure.}
  Congruence under abstraction, application and composition
  are straightforward given that
  the functions $\rweight{\lam{\var}{-}}$, $\rweight{--}$,
  and $\rweight{-\seq-}$ are monotonic.
\end{enumerate}
\end{proof}

\subsection{Confluence of flattening}

\begin{defi}
The reduction relation $\tofnoeta$ is defined as $\tof$
but excluding the $\flatRule{EtaM}$ rule.
\end{defi}

\begin{rem}
The reduction relation $\tofnoeta$ is also SN and CR.
Strong normalization is immediate by \rprop{flat_sn},
since $\tofnoeta \subseteq \tof$.
The proof of confluence is the same as in~\rprop{flat_confluent},
ignoring all the cases involving the $\flatRule{EtaM}$ rule,
and observing that peaks not involving the $\flatRule{EtaM}$ rule
may be closed without using the $\flatRule{EtaM}$ rule.
\end{rem}

\subsection{Soundness with respect to permutation equivalence}

\begin{lem}
\llem{subm_permeq_subrr}
Let $\judgRewr{\tenv,\var:\typ}{\mstep}{\tmfour_0}{\tmfour_1}{\typtwo}$
and $\judgRewr{\tenv}{\msteptwo}{\tmfive_0}{\tmfive_1}{\typ}$.
Then $\mstep\subm{\var}{\msteptwo} \permeq \mstep\subrr{\var}{\msteptwo}$.
\end{lem}
\begin{proof}
By induction on the derivation of
$\judgRewr{\tenv,\var:\typ}{\mstep}{\tmfour_0}{\tmfour_1}{\typtwo}$:
\begin{enumerate}
\item
  \indrulename{RVar}:
  Let $\judgRewr{\tenv,\var:\typ}{\vartwo}{\vartwo}{\vartwo}{\typtwo}$
  with $(\vartwo:\typtwo) \in \tenv$.
  There are two subcases, depending on whether $\var = \vartwo$ or not.
  \begin{enumerate}
  \item
    If $\var = \vartwo$ then:
    $
      \var\subm{\var}{\msteptwo}
      = \msteptwo
      \permeq (\refl{\tmtwo_0} \seq \msteptwo)
      = \var\subrr{\var}{\msteptwo}
    $
    by \permeqRule{IdL}.
  \item
    If $\var \neq \vartwo$ then
    $
      \vartwo\subm{\var}{\msteptwo}
      = \vartwo
      \permeq (\vartwo \seq \vartwo)
      = \vartwo\subrr{\var}{\msteptwo}
    $
    by \permeqRule{IdL}.
  \end{enumerate}
\item
  \indrulename{RCon}:
  Let
    $\judgRewr{\tenv,\var:\typ}{\cons}{\cons}{\cons}{\typtwo}$
  with $(\cons:\typtwo) \in \constantset$.
  Then
  $
    \cons\subm{\var}{\msteptwo}
    = \cons
    \permeq (\cons \seq \cons)
    = \cons\subrr{\var}{\msteptwo}
  $
  by \permeqRule{IdL}.
\item
  \indrulename{RRule}:
  Let $\judgRewr{\tenv,\var:\typ}{\rulewit}{\tm_0}{\tm_1}{\typtwo}$
  be derived from
    $\judgTerm{\noenv}{\tm_0}{\typtwo}$
  and
    $\judgTerm{\noenv}{\tm_1}{\typtwo}$
  with
    $(\rewr{\rulewit}{\tm_0}{\tm_1}{\typtwo})\in\ruleset$.
  Then
  $
    \rulewit\subm{\var}{\msteptwo}
    = \rulewit
    \permeq (\rulewit \seq \refl{\tm_1})
    = \rulewit\subrr{\var}{\msteptwo}
  $
  by \permeqRule{IdR}.
  Note that $\tm_1$ is a closed term
  by~\rlem{free_variables_typed},
  so $\tm_1\subtr{\var}{\msteptwo} = \refl{\tm_1}$.
\item
  \indrulename{RAbs}:
  Let
    $\judgRewr{\tenv,\var:\typ}{
      \lam{\vartwo}{\mstep}
    }{
      \lam{\vartwo}{\tm_0}
    }{
      \lam{\vartwo}{\tm_1}
    }{\typtwo \imp \typthree}$
  be derived from
    $\judgRewr{\tenv,\var:\typ,\vartwo:\typtwo}{
      \mstep
    }{
      \tm_0
    }{
      \tm_1
    }{\typthree}$.
  Then:
  \[
    \begin{array}{rcll}
      (\lam{\vartwo}{\mstep})\subm{\var}{\msteptwo}
    & = &
      \lam{\vartwo}{\mstep\subm{\var}{\msteptwo}}
    \\
    & \permeq &
      \lam{\vartwo}{\mstep\subrr{\var}{\msteptwo}}
      & \text{by \ih}
    \\
    & \permeq &
      (\lam{\vartwo}{\mstep})\subrr{\var}{\msteptwo}
      & \text{by \rlem{subrr_recursion}}
    \end{array}
  \]
\item
  \indrulename{RApp}:
  Let
    $\judgRewr{\tenv,\var:\typ}{
      \mstep_1\,\mstep_2
    }{
      \tm_0\,\tmtwo_0
    }{
      \tm_1\,\tmtwo_1
    }{\typthree}$
  be derived from
    $\judgRewr{\tenv,\var:\typ}{
      \mstep_1
    }{
      \tm_0
    }{
      \tm_1
    }{\typtwo \imp \typthree}$
  and
    $\judgRewr{\tenv,\var:\typ}{
      \mstep_2
    }{
      \tmtwo_0
    }{
      \tmtwo_1
    }{\typtwo}$.
  Then:
  \[
    \begin{array}{rcll}
      (\mstep_1\,\mstep_2)\subm{\var}{\msteptwo}
    & = &
      \mstep_1\subm{\var}{\msteptwo}\,\mstep_2\subm{\var}{\msteptwo}
    \\
    & \permeq &
      \mstep_1\subrr{\var}{\msteptwo}\,\mstep_2\subrr{\var}{\msteptwo}
      & \text{by \ih}
    \\
    & \permeq &
      (\mstep_1\,\mstep_2)\subrr{\var}{\msteptwo}
      & \text{by \rlem{subrr_recursion}}
    \end{array}
  \]
\item
  \indrulename{RTrans}:
  Impossible, as $\mstep$ is a multistep without compositions~(``$\seq$''). 
\item
  \indrulename{REq}:
  Let
    $\judgRewr{\tenv,\var:\typ}{
      \mstep
    }{
      \tm_0
    }{
      \tm_1
    }{
      \typtwo
    }$
  be derived from
    $\judgRewr{\tenv,\var:\typ}{
      \mstep
    }{
      \tm_0'
    }{
      \tm_1'
    }{
      \typtwo
    }$
  with
    $\judgTermEq{\tenv,\var:\typ}{\tm_0}{\tm_0'}{\typtwo}$
  and
    $\judgTermEq{\tenv,\var:\typ}{\tm_1'}{\tm_1}{\typtwo}$.
  Then:
  \[
    \begin{array}{rcll}
      \mstep\subm{\var}{\msteptwo}
    & \permeq &
      \mstep\subt{\var}{\refl{\tmfive_0}}\seq
      \tm'_1\subtr{\var}{\msteptwo}
      & \text{by \ih}
    \\
    & \permeq &
      \mstep\subt{\var}{\refl{\tmfive_0}}\seq
      \tm_1\subtr{\var}{\msteptwo}
      & \text{by \rlem{congruence_termeq_subtr}}
    \\
    & = &
      \mstep\subrr{\var}{\msteptwo}
    \end{array}
  \]
\end{enumerate}
\end{proof}

\subsection{Characterization of normal forms}

\begin{lem}[Characterization of normal multisteps]
\llem{normal_multisteps}
\quad
\begin{enumerate}
\item
  The set of multisteps in $\tofnoeta$-normal form
  is exactly the set of (typable) flat multisteps.
\item
  The set of multisteps
  in $\tof$-normal form
  is a subset of the set of (typable) flat multisteps.
\end{enumerate}
\end{lem}
\begin{proof}
Recall that multisteps are only subject
to $\tof_{\flatRule{BetaM},\flatRule{EtaM}}$
reduction~(\rremark{flatten_not_beta_eta_not_multisteps}),
so this result is immediate if typable multisteps are understood
as simply typed $\lambda$-terms where
constants ($\cons,\constwo,\hdots$) and
rule symbols ($\rulewit,\rulewittwo,\hdots$) 
are regarded as free variables of their corresponding types.
\end{proof}

\begin{prop}[Characterization of normal rewrites]
\llem{normal_rewrites}
\quad
\begin{enumerate}
\item
  The set of rewrites in $\tofnoeta$-normal form is exactly
  the set of (typable) flat rewrites.
\item
  The set of rewrites in $\tof$-normal form is a subset of
  the set of (typable) flat rewrites.
\end{enumerate}
\end{prop}
\begin{proof}
Item~2. is an easy consequence of item~1.
For item~1., we prove the two implications:
\begin{itemize}
\item[$(\Rightarrow)$]
  Let $\redseq$ be a rewrite in $\tofnoeta$-normal form,
  and let us show that it is a flat rewrite.
  We proceed by induction on $\redseq$:
  \begin{enumerate}
  \item {\bf Variable ($\redseq = \var$),
             constant ($\redseq = \cons$), or
             rule symbol ($\redseq = \rulewit$).}
    Immediate.
  \item {\bf Abstraction ($\redseq = \lam{\var}{\redseqtwo}$).}
    By \ih $\redseqtwo$ is a flat rewrite.
    If $\redseqtwo = \mstepn$ is a flat multistep,
    it is easy to check that $\lam{\var}{\mstepn}$ is also a
    flat multistep.
    If $\redseqtwo = (\redseqntwo_1\seq\redseqntwo_2)$ is a composition
    then $\redseq = \lam{\var}{(\redseqntwo_1\seq\redseqntwo_2)}
          \tof_{\flatRule{Abs}}
          (\lam{\var}{\redseqntwo_1})\seq(\lam{\var}{\redseqntwo_2})$
    contradicting the fact that it is a $\tofnoeta$-normal form.
  \item {\bf Application ($\redseq = \redseqtwo\,\redseqthree$).}
    By \ih $\redseqtwo$ and $\redseqthree$ are flat rewrites.
    Note that $\redseqtwo$ cannot be a composition of the form
    $\redseqtwo = (\redseqntwo_1\seq\redseqntwo_2)$
    because then $\redseq = (\redseqntwo_1\seq\redseqntwo_2)\,\redseqthree$
    would reduce,
    either applying \flatRule{App1} at the root (if $\redseqthree$ is a multistep)
    or \flatRule{App3} at the root (if $\redseqthree$ is a composition),
    and this would contradict the fact that $\redseq$ is $\tofnoeta$-normal.
    Hence $\redseqtwo = \mstepn$ is a flat multistep.
    Moreover, $\redseqthree$ cannot be a composition of the form
    $\redseqthree = (\redseqnthree_1\seq\redseqnthree_2)$
    because then $\redseq = \mstepn\,(\redseqnthree_1\seq\redseqnthree_2)$
    would reduce applying \flatRule{App2} at the root,
    and this would contradict the fact that $\redseq$ is $\tofnoeta$-normal.
    Hence $\redseqthree = \mstepntwo$ is also a flat multistep.
    Finally, $\redseq = \mstepn\,\mstepntwo$ is a multistep
    in $\tofnoeta$-normal form, so by~\rlem{normal_multisteps}
    it is a flat multistep.
  \item {\bf Composition ($\redseq = \redseqtwo\seq\redseqthree$).}
    By \ih, $\redseqtwo = \redseqntwo$ and $\redseqthree = \redseqnthree$
    are flat rewrites, so $\redseqntwo\seq\redseqnthree$
    is also a flat rewrite.
  \end{enumerate}
\item[$(\Leftarrow)$]
  Let $\redseqn$ be a flat rewrite.
  Let us prove that it is $\tofnoeta$-normal by induction on
  the derivation that it is a flat rewrite.
  \begin{enumerate}
  \item {\bf Flat multistep, $\redseqn = \mstepn$.}
    Then $\mstepn$ is in $\tofnoeta$-normal form by~\rlem{normal_multisteps}.
  \item {\bf Composition, $\redseqn = \redseqn_1\seq\redseqn_2$.}
    Then by \ih $\redseqn_1$ and $\redseqn_2$ are $\tofnoeta$-normal.
    Moreover, there cannot be a reduction step at the root,
    given there are no rewriting rules in
    the flattening system $\flatteningSystem$
    whose left-hand side is a composition~(``$\seq$'').
  \end{enumerate}
\end{itemize}
\end{proof}

\subsection{$\etalong$-normal forms are closed by flattening}

\begin{lem}[Flattening preserves $\etalong$-normal forms]
\llem{flattening_preserves_etalong}
Assume that the set of rewriting rule symbols $\ruleset$
verifies the $\etalong$-condition.
Let $\judgRewr{\tenv}{\redseq}{\tm}{\tmtwo}{\typ}$
be a $\etalong$-normal form,
and suppose that $\redseq \tofnoeta \redseqtwo$
is a step other than an $\flatRule{EtaM}$ step.
Then $\redseqtwo$ is also a $\etalong$-normal form.
\end{lem}
\begin{proof}
The rewriting step must be of the
form $\rctxof{\redseq_1} \tofnoeta \rctxof{\redseq_2}$ 
where $\redseq_1 \tof \redseq_2$ is an instance of one of
the axioms of the flattening system $\flatteningSystem$
other than the \flatRule{EtaM} rule.
By hypothesis, $\rctxof{\redseq_1}$ is in $\etalong$-normal form,
and we are to show that $\rctxof{\redseq_2}$ is also in $\etalong$-normal form.
By contradiction,
suppose that the right-hand side can be written as of the form
$\rctxof{\redseq_2} = \rctx'\ctxof{\iredseq}$
such that $\rctx'$ is not applicative
and $\iredseq$ is not a $\lambda$-abstraction nor a composition.
\smallskip\\
The proof proceeds by case analysis on the
relative positions of the holes of $\rctx$ and $\rctx'$.
We consider three cases,
depending on whether
the holes of $\rctx$ and $\rctx'$ lie at disjoint positions,
or $\rctx'$ is a prefix of $\rctx$ (with $\rctx \neq \rctx'$),
or $\rctx$ is a prefix of $\rctx'$ (including the case $\rctx = \rctx'$).
\begin{enumerate}
\item {\bf $\rctx$ and $\rctx'$ are disjoint.}
  That is, there is a context $\hat{\rctx}$ with two holes
  such that $\rctx = \hat{\rctx}\ctxof{\ctxhole,\iredseq}$
  and $\rctx' = \hat{\rctx}\ctxof{\redseq_2,\ctxhole}$.
  Then the left-hand side of the step is of the form
  $\rctxof{\redseq_1} = \hat{\rctx}\ctxof{\redseq_1,\iredseq}$.
  Take $\rctx'' := \hat{\rctx}\ctxof{\redseq_1,\ctxhole}$.
  Note that $\rctx''$ cannot be applicative, since this would imply
  that $\rctx'$ is applicative.
  Hence the left-hand side of the step can be written as of the form
  $\rctxof{\redseq_1} = \rctx''\ctxof{\iredseq}$
  where $\rctx''$ is not applicative
  and $\iredseq$ is not a $\lambda$-abstraction nor a composition.
  This contradicts the fact that the left-hand side of the step
  is in $\etalong$-normal form.
\item {\bf $\rctx'$ is a strict prefix of $\rctx$.}
  That is, $\rctx = \rctx'\ctxof{\rctx''}$
  with $\rctx'' \neq \ctxhole$
  and $\iredseq = \rctx''\ctxof{\redseq_2}$.
  Then the left-hand side of the step is of the form
  $\rctxof{\redseq_1} = \rctx'\ctxof{\rctx''\ctxof{\redseq_1}}$.
  But $\rctx'$ is not applicative
  and $\rctx''\ctxof{\redseq_1}$ is not a $\lambda$-abstraction nor
  a composition, because we know that $\rctx''$ is non-empty
  and that $\iredseq$ is not a $\lambda$-abstraction nor a composition.
  This contradicts the fact that the left-hand side of the step is in
  $\etalong$-normal form.
\item {\bf $\rctx$ is a non-strict prefix of $\rctx'$.}
  That is, $\rctx' = \rctx\ctxof{\rctx''}$
  with $\redseq_2 = \rctx''\ctxof{\iredseq}$.
  We analyze all the possible cases, depending on the axiom used
  to derive the step $\redseq_1 \tof \redseq_2$.
  Recall that, by hypothesis, the step is not an $\flatRule{EtaM}$ step:
  \begin{enumerate}
  \item \flatRule{Abs}:
    Let
    $
      \redseq_1 =
      \lam{\var}{(\redseqtwo\seq\redseqthree)}
      \tof
      (\lam{\var}{\redseqtwo})\seq(\lam{\var}{\redseqthree})
      = \redseq_2
    $.
    Note that $\iredseq$ cannot be at the root of $\redseq_2$ because
    it is assumed that $\iredseq$ is not a composition.
    Similarly, $\iredseq$ it cannot be immediately to the left or to the right
    of the composition, because it is assumed that $\iredseq$ is not a
    $\lambda$-abstraction.
    Hence there are two subcases, depending on the position of
    $\iredseq$ on the right-hand side, \ie on the shape of $\rctx''$:
    \begin{enumerate}
    \item
      {\em If $\iredseq$ is internal to $\redseqtwo$,
           \ie $\rctx'' = (\lam{\var}{\rctx'''})\seq(\lam{\var}{\redseqthree})$.}
      Note that $\rctx'''$ is not applicative.
      Then the left-hand side of the step is of the form
      $\rctxof{\lam{\var}{(\rctx'''\ctxof{\iredseq}\seq\redseqthree)}}$
      where the context
      $\rctxof{\lam{\var}{(\rctx'''\ctxof{\ctxhole}\seq\redseqthree)}}$
      is still not applicative.
      This contradicts the fact that the left-hand side
      is in $\etalong$-normal form.
    \item
      {\em If $\iredseq$ is internal to $\redseqthree$,
           \ie $\rctx'' = (\lam{\var}{\redseqtwo})\seq(\lam{\var}{\rctx'''})$.}
      Then the proof is similar as for the previous case.
    \end{enumerate}
  \item \flatRule{App1}:
    Let
    $
      \redseq_1 =
      (\redseqtwo\seq\redseqthree)\,\mstep
      \tof
      (\redseqtwo\,\refl{\rsrc{\mstep}})\seq(\redseqthree\,\mstep)
      = \redseq_2
    $.
    Note that $\iredseq$ cannot be at the root of $\redseq_2$,
    \ie it cannot be the case that $\rctx'' = \ctxhole$,
    because $\iredseq$ is assumed not to be a composition.
    We consider six subcases, depending on the position of
    $\iredseq$ on the right-hand side, \ie on the shape of $\rctx''$:
    \begin{enumerate}
    \item {\em If $\iredseq$ is immediately to the left,
               \ie $\rctx'' = \ctxhole\seq(\redseqthree\,\mstep)$.}
      Then the expression $\iredseq = \redseqtwo\,\refl{\rsrc{\mstep}}$
      is of function type, and
      $\rctx' = \rctxof{\ctxhole\seq(\redseqthree\,\mstep)}$
      is not applicative. Hence the expression
      $\redseq_1 = (\redseqtwo\seq\redseqthree)\,\mstep$
      on the left-hand side is also of function type.
      Moreover, it is not a $\lambda$-abstraction nor a composition,
      and it lies below the context $\rctx$, which is not applicative (because 
      this would imply that $\rctx'$ is applicative).
      This contradicts the fact that the left-hand side of the step is in
      $\etalong$-normal form.
    \item {\em If $\iredseq$ is immediately to the right,
               \ie $\rctx'' = (\redseqtwo\,\refl{\rsrc{\mstep}})\seq\ctxhole$.}
      Similar to the previous case.
    \item {\em If $\iredseq$ is internal to $\redseqtwo$,
               \ie $\rctx'' = (\rctx'''\,\refl{\rsrc{\mstep}})\seq(\redseqthree\,\mstep)$.}
      \label{flattening_preserves_etalong__case_App1_internal1}
      Then $\redseqtwo = \rctx'''\ctxof{\iredseq}$
      and $\rctx''$ is not applicative.
      So the left-hand side is of the form
      $\rctxof{\rctx'''\ctxof{\iredseq}\,\mstep}$.
      Note that the context
      $\rctxof{\rctx'''\,\mstep}$ cannot be applicative,
      for this would imply that $\rctx''$ is applicative.
      This contradicts the fact that the left-hand side of the step is in
      $\etalong$-normal form.
    \item {\em If $\iredseq$ is internal to $\refl{\rsrc{\mstep}}$,
               \ie $\rctx'' = (\redseqtwo\,\rctx''')\seq(\redseqthree\,\mstep)$.}
      Then $\refl{\rsrc{\mstep}} = \rctx'''\ctxof{\iredseq}$
      and $\rctx''$ is not applicative. In particular, $\rctx'''$ is not
      applicative.
      This means that $\refl{\rsrc{\mstep}}$ is not in $\etalong$-normal form.
      We claim that this is impossible.
      To justify the claim,
      it suffices to show that $\mstep$ is in $\etalong$-normal form,
      since by \rlem{source_target_of_etalong_rewrite} this implies that
      $\refl{\rsrc{\mstep}}$ is in $\etalong$-normal form.
      Indeed, suppose that $\mstep = \rctx^*\ctxof{\iredseqtwo}$
      where $\rctx^*$ is not applicative and
      $\iredseqtwo$ is not a $\lambda$-abstraction nor a composition.
      Then the left-hand side of the step is of the form
      $\rctxof{(\redseqtwo\seq\redseqthree)\,\rctx^*\ctxof{\iredseqtwo}}$.
      Note that $\rctxof{(\redseqtwo\seq\redseqthree)\,\rctx^*}$
      is not applicative given that $\rctx^*$ is not applicative.
      This contradicts the fact that the left-hand side of the step
      is in $\etalong$-normal form.
    \item {\em If $\iredseq$ is internal to $\redseqthree$,
               \ie $\rctx'' = (\redseqtwo\,\refl{\rsrc{\mstep}})\seq(\rctx'''\,\mstep)$.}
      Similar to the case in which $\iredseq$ is internal to $\redseqtwo$
      (subcase~\ref{flattening_preserves_etalong__case_App1_internal1}).
    \item {\em If $\iredseq$ is internal to $\mstep$,
               \ie $\rctx'' = (\redseqtwo\,\refl{\rsrc{\mstep}})\seq(\redseqthree\,\rctx''')$.}
      Similar to the case in which $\iredseq$ is internal to $\redseqtwo$
      (subcase~\ref{flattening_preserves_etalong__case_App1_internal1}).
    \end{enumerate}
  \item \flatRule{App2}:
    Let
    $
      \redseq_1 =
      \mstep\,(\redseqtwo\seq\redseqthree)
      \tof
      (\mstep\,\redseqtwo)\seq(\refl{\rtgt{\mstep}}\,\redseqthree)
      = \redseq_2
    $.
    The proof is similar as for the previous case.
  \item \flatRule{App3}:
    Let
    $
      \redseq_1 =
      (\redseqtwo_1\seq\redseqtwo_2)\,(\redseqthree_1\seq\redseqthree_2)
      \tof
      ((\redseqtwo_1\seq\redseqtwo_2)\,\refl{\rsrc{\redseqthree_1}})\seq
      (\refl{\rtgt{\redseqtwo_2}}\,(\redseqthree_1\seq\redseqthree_2))
      = \redseq_2
    $.
    The proof is similar as for the previous case.
  \item \flatRule{BetaM}:
    Let
    $
      \redseq_1 =
      (\lam{\var}{\mstep})\,\msteptwo
      \tof
      \mstep\subm{\var}{\msteptwo}
      = \redseq_2
    $.
    Note that $\redseq_2$ has no compositions~(``$\seq$''),
    so the proof of this case is a straightforward adaptation
    of the proof that $\beta$-reduction preserves $\etalong$-normal forms
    in the simply typed $\lambda$-calculus.
  \end{enumerate}
\end{enumerate}
\end{proof}

\subsection{More properties of flattening}

The following properties are used
to prove completeness of flat permutation equivalence.

\begin{defi}[Flattening to normal form]
If $\redseq$ is a rewrite,
we write $\flatten{\redseq}$ to denote the
$\tof$-normal form of $\redseq$.
Note that the $\flatRule{EtaM}$ {\em reduction} rule is included.
The expressions
$\fsrc{\redseq}$ and $\ftgt{\redseq}$
denote the $\tof$-normal forms of the source and target, respectively,
that is, $\flatten{(\refl{\rsrc{\redseq}})}$
and $\flatten{(\refl{\rtgt{\redseq}})}$.
\end{defi}

\begin{lem}[Coherence of the flat source and target]
\llem{coherence_of_flat_source_and_target}
\quad
\begin{enumerate}
\item $\fsrc{\redseq} \permeq \refl{\rsrc{(\flatten{\redseq})}}$
      and, even more strongly,
      $\refl{\rsrc{(\flatten{\redseq})}} \tofs \fsrc{\redseq}$.
\item $\ftgt{\redseq} \permeq \refl{\rtgt{(\flatten{\redseq})}}$
      and, even more strongly,
      $\refl{\rtgt{(\flatten{\redseq})}} \tofs \ftgt{\redseq}$.
\end{enumerate}
\end{lem}
\begin{proof}
We prove item~1, the proof for item~2. is similar.
By definition, $\fsrc{\redseq} = \flatten{(\refl{\rsrc{\redseq}})}$.
Note that $\redseq \tofs \flatten{\redseq}$.
Recall by \rremark{flat_not_beta_steps_preserve_endpoints}
that steps other than \flatRule{BetaM} and \flatRule{EtaM}
preserve the endpoints,
while by \rlem{flatten_beta_eta_source_target} we know that
\flatRule{BetaM} and \flatRule{EtaM} reduction steps commute
with taking the endpoints.
Hence we have that
$\refl{\rsrc{\redseq}} \tofs \refl{\rsrc{(\flatten{\redseq})}}$.
By confluence of flattening~\rprop{flat_confluent},
$\refl{\rsrc{(\flatten{\redseq})}} \tofs \flatten{(\refl{\rsrc{\redseq}})}
                                       = \fsrc{\redseq}$.
Moreover, by soundness of flattening~(\rlem{flattening_sound_wrt_permeq})
we have that $\refl{\rsrc{(\flatten{\redseq})}} \permeq \fsrc{\redseq}$
as required.
\end{proof}

\begin{lem}[Generalized flattening for composition trees]
\llem{generalized_flattening_kctx}
\quad
\begin{enumerate}
\item {\bf Generalized \flatRule{Abs}.}
  $\lam{\var}{\kctxof{\redseq_1,\hdots,\redseq_n}} \tofs
   \kctxof{\lam{\var}{\redseq_1},\hdots,\lam{\var}{\redseq_n}}$.
\item {\bf Generalized \flatRule{App1}.}
  $\kctxof{\redseq_1,\hdots,\redseq_{n-1},\redseq_n}\,\mstep \tofs
   \kctxof{
     (\redseq_1\,\refl{\rsrc{\mstep}}),
     \hdots,
     (\redseq_{n-1}\,\refl{\rsrc{\mstep}}),
     (\redseq_n\,\mstep)
   }$.
\item {\bf Generalized \flatRule{App2}.}
  $\mstep\,\kctxof{\redseq_1,\redseq_2,\hdots,\redseq_n} \tofs
   \kctxof{
     (\mstep\,\redseq_1),
     (\refl{\rtgt{\mstep}}\,\redseq_2),
     \hdots,
     (\refl{\rtgt{\mstep}}\,\redseq_n)
   }$.
\item {\bf Generalized \flatRule{App3}.}
  If $n, m > 1$ then:
  \[
    \kctxof{\redseq_1,\hdots,\redseq_n}\,
    \kctx'\ctxof{\redseqtwo_1,\hdots,\redseqtwo_m}
    \tofs
    \kctxof{
      (\redseq_1\,\refl{\rsrc{\redseqtwo_1}}),\hdots,
      (\redseq_n\,\refl{\rsrc{\redseqtwo_1}})
    }
    \seq
    \kctx'\ctxof{
      (\refl{\rtgt{\redseq_n}}\,\redseqtwo_1),\hdots,
      (\refl{\rtgt{\redseq_n}}\,\redseqtwo_m)
    }
  \]
\end{enumerate}
\end{lem}
\begin{proof}
We prove each item:
\begin{enumerate}
\item {\bf Generalized \flatRule{Abs}.}
  By induction on $\kctx$.
  If $\kctx = \ctxhole$, then $n = 1$ and
  we have that $\lam{\var}{\redseq_1} \tofs \lam{\var}{\redseq_1}$
  in zero reduction steps.
  If $\kctx = \kctx_1\,\kctx_2$
  then $\kctx_1$ and $\kctx_2$
  have at least one hole each,
  so there is an index $1 \leq i \leq n - 1$ such that
  $\kctxof{\redseq_1,\hdots,\redseq_n} =
   \kctx_1\ctxof{\redseq_1,\hdots,\redseq_{i}}\seq
   \kctx_2\ctxof{\redseq_{i+1},\hdots,\redseq_n}$.
  Then:
  \[
    \begin{array}{rlll}
    &&
      \lam{\var}{\kctxof{\redseq_1,\hdots,\redseq_n}}
    \\
    & = &
      \lam{\var}{
        (\kctx_1\ctxof{\redseq_1,\hdots,\redseq_i}\seq
         \kctx_2\ctxof{\redseq_{i+1},\hdots,\redseq_n})
      }
    \\
    & \tof &
      (\lam{\var}{\kctx_1\ctxof{\redseq_1,\hdots,\redseq_i}})
      \seq
      (\lam{\var}{\kctx_2\ctxof{\redseq_{i+1},\hdots,\redseq_n}})
      & \text{by \flatRule{Abs}}
    \\
    & \tofs &
      \kctx_1\ctxof{\lam{\var}{\redseq_1},\hdots,\lam{\var}{\redseq_i}}
      \seq
      (\lam{\var}{\kctx_2\ctxof{\redseq_{i+1},\hdots,\redseq_n}})
      & \text{by \ih}
    \\
    & \tofs &
      \kctx_1\ctxof{\lam{\var}{\redseq_1},\hdots,\lam{\var}{\redseq_i}}
      \seq
      \kctx_2\ctxof{\lam{\var}{\redseq_{i+1}},\hdots,\lam{\var}{\redseq_n}}
      & \text{by \ih}
    \\
    & = &
      \kctx\ctxof{\lam{\var}{\redseq_1},\hdots,\lam{\var}{\redseq_n}}
    \end{array}
  \]
\item {\bf Generalized \flatRule{App1}.}
  By induction on $\kctx$.
  If $\kctx = \ctxhole$, then $n = 1$ and
  we have that $\redseq_1\,\mstep \tofs \redseq_1\,\mstep$
  in zero reduction steps.
  If $\kctx = \kctx_1\,\kctx_2$ then $\kctx_1$ and $\kctx_2$
  have at least one hole each,
  so there is an index $1 \leq i \leq n - 1$ such that
  $\kctxof{\redseq_1,\hdots,\redseq_{n-1},\redseq_n} =
   \kctx_1\ctxof{\redseq_1,\hdots,\redseq_{i}}\seq
   \kctx_2\ctxof{\redseq_{i+1},\hdots,\redseq_{n-1},\redseq_n}$.
  Then:
  \[
    \begin{array}{rlll}
    &&
      \kctxof{\redseq_1,\hdots,\redseq_{n-1},\redseq_n}\,\mstep
    \\
    & = &
      (\kctx_1\ctxof{\redseq_1,\hdots,\redseq_{i}}\seq
       \kctx_2\ctxof{\redseq_{i+1},\hdots,\redseq_{n-1},\redseq_n})\,\mstep
    \\
    & \tof &
      (\kctx_1\ctxof{\redseq_1,\hdots,\redseq_{i}}\,\refl{\rsrc{\mstep}})\seq
      (\kctx_2\ctxof{\redseq_{i+1},\hdots,\redseq_{n-1},\redseq_n}\,\mstep)
      & \text{by \flatRule{App1}}
    \\
    & \tofs &
      \kctx_1\ctxof{(\redseq_1\,\refl{\rsrc{\mstep}}),
                    \hdots,
                    (\redseq_{i}\,\refl{\rsrc{\mstep}})}\seq
      (\kctx_2\ctxof{\redseq_{i+1},\hdots,\redseq_{n-1},\redseq_n}\,\mstep)
      & \text{by \ih}
    \\
    & \tofs &
      \kctx_1\ctxof{(\redseq_1\,\refl{\rsrc{\mstep}}),
                    \hdots,
                    (\redseq_{i}\,\refl{\rsrc{\mstep}})}\seq
      \kctx_2\ctxof{(\redseq_{i+1},\refl{\rsrc{\mstep}}),
                    \hdots,
                    (\redseq_{n-1}\,\refl{\rsrc{\mstep}}),
                    (\redseq_n\,\mstep)}
      & \text{by \ih}
    \\
    & = &
      \kctx\ctxof{(\redseq_1\,\refl{\rsrc{\mstep}}),
                  \hdots,
                  (\redseq_{n-1}\,\refl{\rsrc{\mstep}}),
                  (\redseq_n\,\mstep)}
    \end{array}
  \]
\item {\bf Generalized \flatRule{App2}.}
  By induction on $\kctx$.
  If $\kctx = \ctxhole$, then $n = 1$ and we have that
  $\mstep\,\redseq_1 \tofs \mstep\,\redseq_1$ in zero reduction steps.
  If $\kctx = \kctx_1\,\kctx_2$ then $\kctx_1$ and $\kctx_2$
  have at least one hole each, so there is an index $1 \leq i \leq n - 1$
  such that
  $\kctxof{\redseq_1,\redseq_2,\hdots,\redseq_n} =
   \kctx_1\ctxof{\redseq_1,\redseq_2,\hdots,\redseq_i}\seq
   \kctx_2\ctxof{\redseq_{i+1},\hdots,\redseq_n}$.
  Then:
  \[
    \begin{array}{rlll}
    && \mstep\,\kctxof{\redseq_1,\redseq_2,\hdots,\redseq_n}
    \\
    & = &
      \mstep\,(\kctx_1\ctxof{\redseq_1,\redseq_2,\hdots,\redseq_i}\seq
                  \kctx_2\ctxof{\redseq_{i+1},\hdots,\redseq_n})
    \\
    & \tof &
      (\mstep\,\kctx_1\ctxof{\redseq_1,\redseq_2,\hdots,\redseq_i})\seq
      (\refl{\rtgt{\mstep}}\,\kctx_2\ctxof{\redseq_{i+1},\hdots,\redseq_n})
      & \text{by \flatRule{App2}}
    \\
    & \tofs &
      \kctx_1\ctxof{
        (\mstep\,\redseq_1),
        (\refl{\rtgt{\mstep}}\,\redseq_2),
        \hdots,
        (\refl{\rtgt{\mstep}}\,\redseq_i)
      }\seq
      (\refl{\rtgt{\mstep}}\,\kctx_2\ctxof{\redseq_{i+1},\hdots,\redseq_n})
      & \text{by \ih}
    \\
    & \tofs &
      \kctx_1\ctxof{
        (\mstep\,\redseq_1),
        (\refl{\rtgt{\mstep}}\,\redseq_2),
        \hdots,
        (\refl{\rtgt{\mstep}}\,\redseq_i)
      }\seq
      \kctx_2\ctxof{
        (\refl{\rtgt{\mstep}}\,\redseq_{i+1}),
        \hdots,
        (\refl{\rtgt{\mstep}}\,\redseq_n)
      }
      & \text{by \ih}
    \\
    & = &
      \kctx\ctxof{
        (\mstep\,\redseq_1),
        (\refl{\rtgt{\mstep}}\,\redseq_2),
        \hdots,
        (\refl{\rtgt{\mstep}}\,\redseq_n)
      }
    \end{array}
  \]
\item {\bf Generalized \flatRule{App3}.}
  Let $n, m > 1$.
  Since $n > 1$,
  the composition tree $\kctx$ has at least two holes,
  so it must be of the form $\kctx = \kctx_1\seq\kctx_2$.
  Similarly, since $m > 1$,
  the composition tree $\kctx'$ has at least two holes,
  so it must be of the form $\kctx' = \kctx'_1\seq\kctx'_2$.
  Moreover, since each of
  $\kctx_1$, $\kctx_2$ $\kctx'_1$, and $\kctx'_2$
  have at least one hole, there must be indices
  $1 \leq i \leq n - 1$ and $1 \leq j \leq n - 1$
  such that:
  \[
    \begin{array}{rcl}
      \kctxof{\redseq_1,\hdots,\redseq_n}
    & = &
      \kctx_1\ctxof{\redseq_1,\hdots,\redseq_i}\seq
      \kctx_2\ctxof{\redseq_{i+1},\hdots,\redseq_n}
    \\
      \kctx'\ctxof{\redseqtwo_1,\hdots,\redseqtwo_n}
    & = &
      \kctx'_1\ctxof{\redseqtwo_1,\hdots,\redseqtwo_j}\seq
      \kctx'_2\ctxof{\redseqtwo_{j+1},\hdots,\redseqtwo_m}
    \end{array}
  \]
  Hence we have that:
  \[
    \begin{array}{rcll}
    &&
      \kctxof{\redseq_1,\hdots,\redseq_n}\,
      \kctx'\ctxof{\redseqtwo_1,\hdots,\redseqtwo_n}
    \\
    & = &
      (\kctx_1\ctxof{\redseq_1,\hdots,\redseq_i}\seq
       \kctx_2\ctxof{\redseq_{i+1},\hdots,\redseq_n})
      \,
      (\kctx'_1\ctxof{\redseqtwo_1,\hdots,\redseqtwo_j}\seq
       \kctx'_2\ctxof{\redseqtwo_{j+1},\hdots,\redseqtwo_m})
    \\
    & \tof &
      (
        (\kctx_1\ctxof{\redseq_1,\hdots,\redseq_i}
        \seq
        \kctx_2\ctxof{\redseq_{i+1},\hdots,\redseq_n})
       \,
         \refl{\rsrc{\redseqtwo_1}}
      )
      \seq
      (
         \refl{\rtgt{\redseq_n}}
       \,
         (\kctx'_1\ctxof{\redseqtwo_1,\hdots,\redseqtwo_j}
         \seq
         \kctx'_2\ctxof{\redseqtwo_{j+1},\hdots,\redseqtwo_m})
      )
      \\&&\HS\text{by \flatRule{App3}}
    \\
    & = &
      (
        \kctxof{\redseq_1,\hdots,\redseq_n}\,
        \refl{\rsrc{\redseqtwo_1}}
      )
      \seq
      (
         \refl{\rtgt{\redseq_n}}
       \,
         \kctx'\ctxof{\redseqtwo_1,\hdots,\redseqtwo_m}
      )
    \\
    & \tofs &
        \kctxof{(\redseq_1\,\refl{\rsrc{\redseqtwo_1}}),
                \hdots,
                (\redseq_n\,\refl{\rsrc{\redseqtwo_1}})}\,
      \seq
      (
         \refl{\rtgt{\redseq_n}}
       \,
         \kctx'\ctxof{\redseqtwo_1,\hdots,\redseqtwo_m}
      )
      \hfill\text{by generalized \flatRule{App1}}
    \\
    & \tofs &
      \kctxof{(\redseq_1\,\refl{\rsrc{\redseqtwo_1}}),
              \hdots,
              (\redseq_n\,\refl{\rsrc{\redseqtwo_1}})}\,
      \seq
      \kctx'\ctxof{
        (\refl{\rtgt{\redseq_n}}\,\redseqtwo_1),
        \hdots,
        (\refl{\rtgt{\redseq_n}}\,\redseqtwo_m)
      }
      \hfill\text{by generalized \flatRule{App2}}
    \end{array}
  \]
  We implicitly use the fact that, in general,
  $\rsrc{\kctxof{\redseq_1,\hdots,\redseq_n}} = \rsrc{\redseq_1}$
  and
  $\rtgt{\kctxof{\redseq_1,\hdots,\redseq_n}} = \rtgt{\redseq_n}$,
  which is easy to check by induction on $\kctx$.
\end{enumerate}
\end{proof}

\begin{lem}[Flattening term/rewrite substitution of a composition]
\llem{flattening_subtr_composition}
Let $\tm$ be a term with $n$ free occurrences of $\var$,
that is $\tm = \tm\ctxof{\var,\var,\hdots,\var}$
where, by abuse of notation, we write $\tm$ for the term itself
and also for a context with $n$ holes that do not bind $\var$.
Moreover, let $\redseq_1,\hdots,\redseq_m$ be fixed rewrites with $m > 0$.
If $i$ is an index $1 \leq i \leq n$, and $\redseqthree$ is a rewrite,
we write $\tm\ctxof{\redseqthree}_i$ for the rewrite
that results from replacing the $i$-th
free occurrence of $\var$ in $\tm$ by $\redseqthree$,
the free occurrences of $\var$
at positions $j < i$ by $\refl{\rtgt{\redseq_m}}$,
and the free occurrences of $\var$
at positions $j > i$ by $\refl{\rsrc{\redseq_1}}$.
That is:
\[
  \tm\ctxof{\redseqthree}^\var_i :=
  \tm\ctxof{
    \underbrace{
      \refl{\rtgt{\redseq_m}},\hdots,\refl{\rtgt{\redseq_m}}
    }_{\text{$i-1$}},
    \redseqthree,
    \underbrace{
      \refl{\rsrc{\redseq_1}},\hdots,\refl{\rsrc{\redseq_1}}
    }_{\text{$n-i$}}
  }
\]
Then, if $n > 0$, for any $m$-hole composition tree $\kctx$
there exists an $(n \cdot m)$-hole composition tree $\kctx'$ such that:
\[
  \tm\subtr{\var}{\kctxof{\redseq_1,\hdots,\redseq_m}}
  \tofs
  \kctx'\ctxof{
    \underbrace{
      \tm\ctxof{\redseq_1}^\var_1,\hdots
      \tm\ctxof{\redseq_m}^\var_1
    }_{\text{($m$ rewrites)}},
    \underbrace{
      \tm\ctxof{\redseq_1}^\var_2,\hdots
      \tm\ctxof{\redseq_m}^\var_2,
    }_{\text{($m$ rewrites)}}
    \hdots
    \underbrace{
      \tm\ctxof{\redseq_1}^\var_n,\hdots
      \tm\ctxof{\redseq_m}^\var_n
    }_{\text{($m$ rewrites)}}
  }
\]
Informally, this expresses that the flattening of
$\tm\subtr{\var}{\kctxof{\redseq_1,\hdots,\redseq_m}}$
is the composition
of substituting first the first occurrence of $\var$
by $\redseq_1,\hdots,\redseq_m$, leaving the remaining ocurrences fixed,
then substituting the second occurrence of $\var$
by $\redseq_1,\hdots,\redseq_m$,
and so on.
\end{lem}
\begin{proof}
We proceed by induction on $\tm$.
If $\tm$ is a variable other than $\var$,
a constant, or a rule symbol, then $n = 0$ and the implication
holds vacuously. The remaining cases are:
\begin{enumerate}
\item {\bf Substituted variable, $\tm = \var$.}
  Taking $\kctx' := \kctx$
  we have that
  \[
    \var\subtr{\var}{\kctxof{\redseq_1,\hdots,\redseq_m}}
    = \kctxof{\redseq_1,\hdots,\redseq_m}
    = \kctxof{\var\ctxof{\redseq_1}^\var_1,\hdots,
              \var\ctxof{\redseq_m}^\var_1}
  \]
\item {\bf Abstraction, $\lam{\vartwo}{\tm}$.}
  Note that there are $n$ free occurrences of $\var$ in $\tm$. Then:
  \[
    \begin{array}{rlll}
      \lam{\vartwo}{\tm\subtr{\var}{\kctxof{\redseq_1,\hdots,\redseq_m}}}
    & \tofs &
      \lam{\vartwo}{
        \kctx'\ctxof{
          \tm\ctxof{\redseq_1}^\var_1,
          \hdots
          \tm\ctxof{\redseq_m}^\var_1,
          \hdots
          \tm\ctxof{\redseq_1}^\var_n,
          \tm\ctxof{\redseq_m}^\var_n
        }
      }
      \\&&\HS\text{by \ih}
    \\
    & \tofs &
      \kctx'\ctxof{
        \lam{\vartwo}{\tm\ctxof{\redseq_1}^\var_1},
        \hdots
        \lam{\vartwo}{\tm\ctxof{\redseq_m}^\var_1},
        \hdots
        \lam{\vartwo}{\tm\ctxof{\redseq_1}^\var_n},
        \hdots
        \lam{\vartwo}{\tm\ctxof{\redseq_m}^\var_n}
      }
      \\&&\HS\text{by generalized
                   \flatRule{Abs}~\rlem{generalized_flattening_kctx}}
    \end{array}
  \]
\item {\bf Application, $\tm\,\tmtwo$.}
  Then $n = i + j$
  where $i$ is the number of free occurrences of $\var$ in $\tm$,
  and $j$ is the number of free occurrences of $\var$ in $\tmtwo$.
  By hypothesis, $n > 0$. We consider three subcases, depending
  on whether $i = 0$, or $j = 0$, or both $i$ and $j$ are strictly positive:
  \begin{enumerate}
  \item
    If $i = 0$ and $j = n$, then:
    \[
      \begin{array}{rlll}
      &&
        \tm\subtr{\var}{\kctxof{\redseq_1,\hdots,\redseq_m}}\,
        \tmtwo\subtr{\var}{\kctxof{\redseq_1,\hdots,\redseq_m}}
      \\
      & = &
        \tm\,
        \tmtwo\subtr{\var}{\kctxof{\redseq_1,\hdots,\redseq_m}}
      \\
      & \tofs &
        \tm\,
        \kctx'\ctxof{
          \tmtwo\ctxof{\redseq_1}^\var_1,
          \hdots,
          \tmtwo\ctxof{\redseq_m}^\var_1,
          \hdots
          \tmtwo\ctxof{\redseq_1}^\var_n,
          \hdots,
          \tmtwo\ctxof{\redseq_m}^\var_n
        }
        & \text{by \ih}
      \\
      & \tofs &
        \kctx'\ctxof{
          (\tm\,\tmtwo\ctxof{\redseq_1}^\var_1),
          \hdots,
          (\tm\,\tmtwo\ctxof{\redseq_m}^\var_1),
          \hdots
          (\tm\,\tmtwo\ctxof{\redseq_1}^\var_n),
          \hdots,
          (\tm\,\tmtwo\ctxof{\redseq_m}^\var_n)
        }
        \\&&\HS\text{by generalized
                     \flatRule{App2}~\rlem{generalized_flattening_kctx}}
      \end{array}
    \]
  \item
    If $j = 0$ and $i = n$,
    the proof is symmetric to the previous case.
  \item
    If $i > 0$ and $j > 0$,
    note that
    $\rsrc{(\tmtwo\ctxof{\redseq_1}^\var_1)} = \tmtwo\subtr{\var}{\rsrc{\redseq_1}}$
    and that
    $\rtgt{(\tm\ctxof{\redseq_m}^\var_i)} = \tm\subtr{\var}{\rtgt{\redseq_m}}$.
    Then:
    \[
    {\small
      \begin{array}{rlll}
      &&
        \tm\subtr{\var}{\kctxof{\redseq_1,\hdots,\redseq_m}}\,
        \tmtwo\subtr{\var}{\kctxof{\redseq_1,\hdots,\redseq_m}}
      \\
      & \tofs &
        \kctx_1\ctxof{
          \tm\ctxof{\redseq_1}^\var_1,
          \hdots,
          \tm\ctxof{\redseq_m}^\var_1,
          \hdots,
          \tm\ctxof{\redseq_1}^\var_i,
          \hdots,
          \tm\ctxof{\redseq_m}^\var_i
        }
        \,\\&&
        \kctx_2\ctxof{
          \tmtwo\ctxof{\redseq_1}^\var_1,
          \hdots,
          \tmtwo\ctxof{\redseq_m}^\var_1,
          \hdots,
          \tmtwo\ctxof{\redseq_1}^\var_j,
          \hdots,
          \tmtwo\ctxof{\redseq_m}^\var_j
        }
        \\&&\HS\text{by \ih}
      \\
      & \tofs &
        \kctx_1\ctxof{
          \tm\ctxof{\redseq_1}^\var_1\,\tmtwo\subtr{\var}{\refl{\rsrc{\redseq_1}}},
          \hdots,
          \tm\ctxof{\redseq_m}^\var_1\,\tmtwo\subtr{\var}{\refl{\rsrc{\redseq_1}}},
          \hdots,
          \tm\ctxof{\redseq_1}^\var_i\,\tmtwo\subtr{\var}{\refl{\rsrc{\redseq_1}}},
          \hdots,
          \tm\ctxof{\redseq_m}^\var_i\,\tmtwo\subtr{\var}{\refl{\rsrc{\redseq_1}}}
        }
        \seq\\&&
        \kctx_2\ctxof{
          \tm\subtr{\var}{\refl{\rtgt{\redseq_m}}}\,\tmtwo\ctxof{\redseq_1}^\var_1,
          \hdots,
          \tm\subtr{\var}{\refl{\rtgt{\redseq_m}}}\,\tmtwo\ctxof{\redseq_m}^\var_1,
          \hdots,
          \tm\subtr{\var}{\refl{\rtgt{\redseq_m}}}\,\tmtwo\ctxof{\redseq_1}^\var_j,
          \hdots,
          \tm\subtr{\var}{\refl{\rtgt{\redseq_m}}}\,\tmtwo\ctxof{\redseq_m}^\var_j
        }
      \\&&\HS\text{by generalized
                   \flatRule{App3}~\rlem{generalized_flattening_kctx}}
      \\
      & = &
        \kctx_1\ctxof{
          (\tm\,\tmtwo)\ctxof{\redseq_1}^\var_1,
          \hdots,
          (\tm\,\tmtwo)\ctxof{\redseq_m}^\var_1,
          \hdots,
          (\tm\,\tmtwo)\ctxof{\redseq_1}^\var_i,
          \hdots,
          (\tm\,\tmtwo)\ctxof{\redseq_m}^\var_i
        }
        \seq\\&&
        \kctx_2\ctxof{
          (\tm\,\tmtwo)\ctxof{\redseq_1}^\var_{i+1},
          \hdots,
          (\tm\,\tmtwo)\ctxof{\redseq_m}^\var_{i+1},
          \hdots,
          (\tm\,\tmtwo)\ctxof{\redseq_1}^\var_n,
          \hdots,
          (\tm\,\tmtwo)\ctxof{\redseq_m}^\var_n
        }
      \end{array}
    }
    \]
    Taking $\kctx' := \kctx_1\seq\kctx_2$ we conclude.
  \end{enumerate}
\end{enumerate}
\end{proof}

\begin{lem}[Flattening of $\eta$-expanded multisteps]
\llem{flattening_of_eta_expanded_multisteps}
Let $\mstep,\msteptwo$
be multisteps in $\etalong$-normal form
such that
$\flatten{\mstep} = \flatten{\msteptwo}$.
Then $\flattennoeta{\mstep} = \flattennoeta{\msteptwo}$.
\end{lem}
\begin{proof}
Consider the reduction sequences
$\mstep \tofs \flatten{\mstep}$ and
$\msteptwo \tofs \flatten{\msteptwo}$.
Since \flatRule{EtaM}-redexes
may be postponed after \flatRule{BetaM}-redexes
(a standard result, regarding multisteps
as terms of the simply-typed $\lambda$-calculus),
these reductions factorize as
$\mstep
 \tofs_{\flatRule{BetaM}} \flattennoeta{\mstep}
 \tofs_{\flatRule{EtaM}} \flatten{\mstep}$
and
$\msteptwo
 \tofs_{\flatRule{BetaM}} \flattennoeta{\msteptwo}
 \tofs_{\flatRule{EtaM}} \flatten{\msteptwo}$.
Moreover, recall that
flattening preserves
$\etalong$-normal forms~(\rlem{flattening_preserves_etalong}),
so $\flattennoeta{\mstep}$ and $\flattennoeta{\msteptwo}$
are $\etalong$-normal forms.
As an auxiliary claim,
observe that if $\mstepthree$ is a multistep in
\flatRule{BetaM}-normal form
then any \flatRule{EtaM} reduction step
$\mstepthree \tof_{\flatRule{EtaM}} \mstepthree'$
corresponds to a backwards expansion step
$\mstepthree' \toetaexp \mstepthree$;
this can be easily checked by induction on $\mstepthree$
following the characterization
of flat multisteps~(\rlem{normal_multisteps}).
Hence
$\flatten{\mstep} \toetaexp \flattennoeta{\mstep}$
and
$\flatten{\mstep} = \flatten{\msteptwo} \toetaexp \flattennoeta{\msteptwo}$.
Finally, since $\flattennoeta{\mstep}$
and $\flattennoeta{\msteptwo}$ are $\etalong$-normal
forms and the expansion relation $\toetaexp$
is confluent~(\rprop{restricted_eta_expansion_sn_cr}),
we obtain that $\flattennoeta{\mstep} = \flattennoeta{\msteptwo}$,
as required.
\end{proof}

\subsection{Flat permutation equivalence}

\begin{rem}
Every time that flattening $\flatten{-}$ is used in the
rules defining $\flateq$, it operates over a multistep.
So the only rules that are needed are the \flatRule{BetaM} and \flatRule{EtaM}
rules.
\end{rem}

\begin{rem}
Recall that, by definition, flat rewrites are given by the grammar
$\redseqn ::= \mstepn \mid \redseqn\seq\redseqn$.
This corresponds to the set of all and only
the rewrites of the form $\kctxof{\mstepn_1,\hdots,\mstepn_n}$.
\end{rem}

\begin{lem}[Soundness of splitting with respect to permutation equivalence]
\llem{splitting_sound_wrt_permeq}
Let $\judgRewr{\tenv}{\mstep}{\tm}{\tmtwo}{\typ}$
and $\judgRewr{\tenv}{\mstep_1}{\tm'}{\tmthree_1}{\typ}$
and $\judgRewr{\tenv}{\mstep_2}{\tmthree_2}{\tmtwo'}{\typ}$
be such that $\judgSplit{\mstep}{\mstep_1}{\mstep_2}$.
Then $\mstep \permeq \mstep_1\seq\mstep_2$
\end{lem}
\begin{proof}
By induction on the derivation of $\judgSplit{\mstep}{\mstep_1}{\mstep_2}$:
\begin{enumerate}
\item \indrulename{SVar}:
  Let $\judgSplit{\var}{\var}{\var}$.
  Then $\var \permeq \var\seq\var$
  by \permeqRule{IdL}.
\item \indrulename{SCon}:
  Let $\judgSplit{\cons}{\cons}{\cons}$.
  Then $\cons \permeq \cons\seq\cons$
  by \permeqRule{IdL}.
\item \indrulename{SRuleL}:
  Let $\judgSplit{\rulewit}{\rulewit}{\refl{\rtgt{\rulewit}}}$.
  Then $\rulewit \permeq \rulewit\seq\refl{\rtgt{\rulewit}}$
  by \permeqRule{IdR}.
\item \indrulename{SRuleR}:
  Let $\judgSplit{\rulewit}{\refl{\rsrc{\rulewit}}}{\rulewit}$.
  Then $\rulewit \permeq \refl{\rsrc{\rulewit}}\seq\rulewit$
  by \permeqRule{IdL}.
\item \indrulename{SAbs}:
  Let
  $\judgSplit{\lam{\var}{\mstep}}{\lam{\var}{\mstep_1}}{\lam{\var}{\mstep_2}}$
  be derived from
  $\judgSplit{\mstep}{\mstep_1}{\mstep_2}$.
  Then:
  \[
    \begin{array}{rcll}
      \lam{\var}{\mstep}
    & \permeq &
      \lam{\var}{(\mstep_1\seq\mstep_2)}
      & \text{by \ih}
    \\
    & \permeq &
      (\lam{\var}{\mstep_1})\seq(\lam{\var}{\mstep_2})
      & \text{by \permeqRule{Abs}}
    \end{array}
  \]
\item \indrulename{SApp}:
  Let
  $\judgSplit{\mstep\,\msteptwo}{\mstep_1\,\msteptwo_1}{\mstep_2\,\msteptwo_2}$
  be derived from
  $\judgSplit{\mstep}{\mstep_1}{\mstep_2}$
  and
  $\judgSplit{\msteptwo}{\msteptwo_1}{\msteptwo_2}$.
  Then: 
  \[
    \begin{array}{rcll}
      \mstep\,\msteptwo
    & \permeq &
      (\mstep_1\seq\mstep_2)\,\msteptwo
      & \text{by \ih}
    \\
    & \permeq &
      (\mstep_1\seq\mstep_2)\,(\msteptwo_1\seq\msteptwo_2)
      & \text{by \ih}
    \\
    & \permeq &
      (\mstep_1\,\msteptwo_1)\seq(\mstep_2\,\msteptwo_2)
      & \text{by \permeqRule{App}}
    \end{array}
  \]
\end{enumerate}
\end{proof}

\begin{lem}[Soundness of flat permutation equivalence with respect to permutation equivalence]
\llem{flateq_sound_wrt_permeq}
Let $\judgRewr{\tenv}{\redseq}{\tm}{\tmtwo}{\typ}$
and $\judgRewr{\tenv}{\redseqtwo}{\tm'}{\tmtwo'}{\typ}$
be such that $\redseq \flateq \redseqtwo$.
Then $\redseq \permeq \redseqtwo$.
\end{lem}
\begin{proof}
By induction on the derivation of $\redseq \flateq \redseqtwo$.
Reflexivity, transitivity, symmetry, and closure under composition
contexts is immediate.
The interesting case is when an axiom is applied at the root:
\begin{enumerate}
\item
  \flateqRule{Assoc}:
  Let $(\redseq\seq\redseqtwo)\seq\redseqthree \flateq
       \redseq\seq(\redseqtwo\seq\redseqthree)$.
  Then by \permeqRule{Assoc}
  also $(\redseq\seq\redseqtwo)\seq\redseqthree \permeq
       \redseq\seq(\redseqtwo\seq\redseqthree)$.
\item
  \flateqRule{Perm}:
  Let $\mstep \flateq \mstep_1\seq\mstep_2$ where
  $\judgSplit{\mstep}{\mstep_1}{\mstep_2}$.
  Then by \rlem{splitting_sound_wrt_permeq}
  we have that $\mstep \permeq \mstep_1\seq\mstep_2$.
\end{enumerate}
\end{proof}

\subsection{Completeness of flat permutation equivalence with respect to permutation equivalence}
\lsec{appendix:flattening_completeness}

Before proving completeness, we need a few auxiliary results.

\begin{lem}[Generalized \flateqRule{Assoc} rule]
\llem{generalized_flateq_assoc}
Let $\mstep,\msteptwo_1,\hdots,\msteptwo_n$ be multisteps
where $n \geq 1$,
and let $\kctx$ be a composition tree. Then:
\begin{enumerate}
\item $\mstep\seq\kctxof{\msteptwo_1,\msteptwo_2,\hdots,\msteptwo_n}
       \flateq
       \kctxof{(\mstep\seq\msteptwo_1),\msteptwo_2,\hdots,\msteptwo_n}$
\item $\kctxof{\msteptwo_1,\msteptwo_2,\hdots,\msteptwo_n}\seq\mstep
       \flateq
       \kctxof{\msteptwo_1,\msteptwo_2,\hdots,(\msteptwo_n\seq\mstep)}$
\end{enumerate}
\end{lem}
\begin{proof}
We only prove item 1. (item 2. is similar). We proceed by induction
on $\kctx$:
\begin{enumerate}
\item {\bf Empty, $\kctx = \ctxhole$.}
  Then
  $\mstep\seq\msteptwo_1 \flateq \mstep\seq\msteptwo_1$
  by reflexivity.
\item {\bf Composition, $\kctx = \kctx_1\seq\kctx_2$.}
  Then $n > 1$ and there is an index $1 \leq i \leq n$
  such that
  $\kctxof{\msteptwo_1,\hdots,\msteptwo_n} =
   \kctx_1\ctxof{\msteptwo_1,\msteptwo_2,\hdots,\msteptwo_i}
   \seq
   \kctx_2\ctxof{\msteptwo_{i+1},\hdots,\msteptwo_n}$.
  Hence:
  \[
    \begin{array}{rcll}
      \mstep\seq\kctxof{\msteptwo_1,\hdots,\msteptwo_n}
    & = &
      \mstep\seq
      (
       \kctx_1\ctxof{\msteptwo_1,\msteptwo_2,\hdots,\msteptwo_i}
       \seq
       \kctx_2\ctxof{\msteptwo_{i+1},\hdots,\msteptwo_n}
      )
    \\
    & \flateq &
      (\mstep
       \seq
       \kctx_1\ctxof{\msteptwo_1,\msteptwo_2,\hdots,\msteptwo_i})
      \seq \kctx_2\ctxof{\msteptwo_{i+1},\hdots,\msteptwo_n}
      & \text{by \flateqRule{Assoc}}
    \\
    & \flateq &
      \kctx_1\ctxof{(\mstep\seq\msteptwo_1),\msteptwo_2,\hdots,\msteptwo_i}
      \seq \kctx_2\ctxof{\msteptwo_{i+1},\hdots,\msteptwo_n}
      & \text{by \ih}
    \\
    & = &
      \kctxof{(\mstep\seq\msteptwo_1),\msteptwo_2,\hdots,\msteptwo_n}
    \end{array}
  \]
\end{enumerate}
\end{proof}

\begin{lem}[Left/right splitting]
\llem{left_right_splitting}
Let $\mstep$ be a multistep. Then:
\begin{enumerate}
\item $\judgSplit{\mstep}{\mstep}{\refl{\rtgt{\mstep}}}$
\item $\judgSplit{\mstep}{\refl{\rsrc{\mstep}}}{\mstep}$
\end{enumerate}
\end{lem}
\begin{proof}
We only prove item 1. (item 2. is similar). We proceed by induction
on $\mstep$:
\begin{enumerate}
\item {\bf Variable, $\mstep = \var$.}
  By \indrulename{SVar}, $\judgSplit{\var}{\var}{\var}$.
\item {\bf Constant, $\mstep = \cons$.}
  By \indrulename{SCon}, $\judgSplit{\cons}{\cons}{\cons}$.
\item {\bf Rule symbol, $\mstep = \rulewit$.}
  By \indrulename{SRuleL},
  $\judgSplit{\rulewit}{\rulewit}{\refl{\rtgt{\rulewit}}}$.
\item {\bf Abstraction, $\mstep = \lam{\var}{\msteptwo}$.}
  By \ih $\judgSplit{\msteptwo}{\msteptwo}{\refl{\rtgt{\msteptwo}}}$
  so by \indrulename{SAbs},
  $\judgSplit{
     \lam{\var}{\msteptwo}
   }{
     \lam{\var}{\msteptwo}
   }{
     \lam{\var}{\refl{\rtgt{\msteptwo}}}
   }$.
\item {\bf Application, $\mstep = \msteptwo_1\,\msteptwo_2$.}
  By \ih $\judgSplit{\msteptwo_1}{\msteptwo_1}{\refl{\rtgt{\msteptwo_1}}}$
  and $\judgSplit{\msteptwo_2}{\msteptwo_2}{\refl{\rtgt{\msteptwo_2}}}$
  so
  $\judgSplit{
     \msteptwo_1\,\msteptwo_2
   }{
     \msteptwo_1\,\msteptwo_2
   }{
     \refl{\rtgt{\msteptwo_1}}\,\refl{\rtgt{\msteptwo_2}}
   }$.
\end{enumerate}
\end{proof}

\begin{lem}[Free variables of splitting]
\llem{splitting_free_variables}
If $\judgSplit{\mstep}{\mstep_1}{\mstep_2}$
then $\fv{\mstep} = \fv{\mstep_1} \cup \fv{\mstep_2}$.
\end{lem}
\begin{proof}
Straightforward by induction on the derivation of
$\judgSplit{\mstep}{\mstep_1}{\mstep_2}$.
The interesting cases are the \indrulename{SRuleL}
and \indrulename{SRuleR} rules.
For example, for the \indrulename{SRuleL} case, note that
$\fv{\rulewit} = \fv{\rulewit} \cup \fv{\rtgt{\rulewit}}$
given that $\fv{\rtgt{\rulewit}} = \emptyset$,
as the source and the target of a given rule symbol are
closed terms.
\end{proof}

\begin{lem}[Splitting commutes with substitution]
\llem{splitting_substitution}
If $\judgSplit{\mstep}{\mstep_1}{\mstep_2}$
and $\judgSplit{\msteptwo}{\msteptwo_1}{\msteptwo_2}$
then
$\judgSplit{
   \mstep\subm{\var}{\msteptwo}
 }{
   \mstep_1\subm{\var}{\msteptwo_1}
 }{
   \mstep_2\subm{\var}{\msteptwo_2}
 }$.
\end{lem}
\begin{proof}
By induction on the derivation of
$\judgSplit{\mstep}{\mstep_1}{\mstep_2}$:
\begin{enumerate}
\item \indrulename{SVar}:
  Let $\judgSplit{\vartwo}{\vartwo}{\vartwo}$.
  If $\var \neq \vartwo$, it is immediate.
  If $\var = \vartwo$,
  then indeed $\judgSplit{\msteptwo}{\msteptwo_1}{\msteptwo_2}$.
\item \indrulename{SCon}:
  Immediate. 
\item \indrulename{SRuleL}:
  Let $\judgSplit{\rulewit}{\rulewit}{\refl{\rtgt{\rulewit}}}$.
  Recall that the target of a rule symbol is always a closed term,
  so $\refl{\rtgt{\rulewit}}\subm{\var}{\mstepthree} = \refl{\rtgt{\rulewit}}$.
  Then it is immediate, given that
  $\judgSplit{\rulewit}{\rulewit}{\refl{\rtgt{\rulewit}}}$.
\item \indrulename{SRuleR}:
  Similar to the previous case.
\item \indrulename{SAbs}:
  Let
  $\judgSplit{
     \lam{\vartwo}{\mstep}
   }{
     \lam{\vartwo}{\mstep_1}
   }{
     \lam{\vartwo}{\mstep_2}
   }$
  be derived from
  $\judgSplit{\mstep}{\mstep_1}{\mstep_2}$.
  Then by \ih we have that
  $\judgSplit{
     \mstep\subm{\var}{\msteptwo}
   }{
     \mstep_1\subm{\var}{\msteptwo_1}
   }{
     \mstep_2\subm{\var}{\msteptwo_2}
   }$,
  so applying the \indrulename{SAbs} rule
  $\judgSplit{
     \lam{\vartwo}{\mstep\subm{\var}{\msteptwo}}
   }{
     \lam{\vartwo}{\mstep_1\subm{\var}{\msteptwo_1}}
   }{
     \lam{\vartwo}{\mstep_2\subm{\var}{\msteptwo_2}}
   }$.
\item \indrulename{SApp}:
  Let
  $\judgSplit{
     \mstep_1\,\mstep_2
   }{
     \mstep_{11}\,\mstep_{21}
   }{
     \mstep_{12}\,\mstep_{22}
   }$
  be derived from
  $\judgSplit{\mstep_1}{\mstep_{11}}{\mstep_{12}}$
  and
  $\judgSplit{\mstep_1}{\mstep_{21}}{\mstep_{22}}$.
  Then by \ih we have that
  $\judgSplit{
     \mstep_1\subm{\var}{\msteptwo}
   }{
     \mstep_{11}\subm{\var}{\msteptwo_1}
   }{
     \mstep_{12}\subm{\var}{\msteptwo_2}
   }$
  and
  $\judgSplit{
     \mstep_2\subm{\var}{\msteptwo}
   }{
     \mstep_{21}\subm{\var}{\msteptwo_1}
   }{
     \mstep_{22}\subm{\var}{\msteptwo_2}
   }$,
  so applying the \indrulename{SApp} rule
  $\judgSplit{
     (\mstep_1\,\mstep_2)\subm{\var}{\msteptwo}
   }{
     (\mstep_{11}\,\mstep_{21})\subm{\var}{\msteptwo_1}
   }{
     (\mstep_{12}\,\mstep_{22})\subm{\var}{\msteptwo_2}
   }$.
\end{enumerate}
\end{proof}

\begin{lem}[Coherence of splitting and flattening]
\llem{coherence_splitting_flattening}
Let $\mstep,\mstep_1,\mstep_2$ be multisteps not necessarily in normal form,
and suppose that $\judgSplit{\mstep}{\mstep_1}{\mstep_2}$.
Then $\judgSplit{\flatten{\mstep}}{\mstep'_1}{\mstep'_2}$
where $\mstep'_1$ and $\mstep'_2$ are such that
$\mstep_1 \tofs \mstep'_1$ and $\mstep_2 \tofs \mstep'_2$.
\end{lem}
\begin{proof}
It suffices to show that if $\mstep \tof \msteptwo$
then there exist multisteps $\msteptwo_1$ and $\msteptwo_2$
such that $\mstep_1 \tofs \msteptwo_1$
and $\mstep_2 \tofs \msteptwo_2$
and $\judgSplit{\msteptwo}{\msteptwo_1}{\msteptwo_2}$.
With this property, the proof of the lemma
is immediate by induction on the length of a reduction
to normal form $\mstep \tofs \flatten{\mstep}$.

We proceed by induction on $\mstep$.
If $\mstep$ is a variable, a constant, or a rule symbol,
it is immediate as there cannot be a reduction step $\mstep \tof \msteptwo$.
There are two remaining cases:
\begin{enumerate}
\item {\bf Abstraction, $\mstep = \lam{\var}{\mstepthree}$.}
  Then note that
  $\judgSplit{\mstep}{\mstep_1}{\mstep_2}$
  must be derived using the \indrulename{SAbs} rule,
  so $\judgSplit{\mstepthree}{\mstepthree_1}{\mstepthree_2}$
  where $\mstep_1 = \lam{\var}{\mstepthree_1}$
  and $\mstep_2 = \lam{\var}{\mstepthree_2}$.
  We consider two subcases, depending on whether 
  the step $\mstep = \lam{\var}{\mstepthree} \tof \msteptwo$,
  is internal to $\mstepthree$ or an \flatRule{EtaM} step at the root:
  \begin{enumerate}
  \item
    If the step is internal to $\mstepthree$,
    \ie $\mstepthree \tof \mstepfour$
    and $\msteptwo = \lam{\var}{\mstepfour}$,
    then by \ih we have that
    $\judgSplit{\mstepfour}{\mstepfour_1}{\mstepfour_2}$
    such that $\mstepthree_1 \tofs \mstepfour_1$
    and $\mstepthree_2 \tofs \mstepfour_2$.
    Therefore, by the \indrulename{SAbs} rule,
    $\judgSplit{\msteptwo}{\lam{\var}{\mstepfour_1}}{\lam{\var}{\mstepfour_2}}$
    where $\mstep_1 = \lam{\var}{\mstepthree_1} \tofs \lam{\var}{\mstepfour_1}$
    and $\mstep_2 = \lam{\var}{\mstepthree_2} \tofs \lam{\var}{\mstepfour_2}$,
    as required.
  \item
    If the step is an \flatRule{EtaM} step at the root,
    \ie $\mstepthree = \msteptwo\,\var$
    with $\var \notin \fv{\msteptwo}$,
    then note that $\judgSplit{\mstepthree}{\mstepthree_1}{\mstepthree_2}$
    must be derived using the \indrulename{SApp} rule,
    so $\judgSplit{\msteptwo}{\msteptwo_1}{\msteptwo_2}$
    where $\mstepthree_1 = \msteptwo_1\,\var$
    and $\mstepthree_2 = \msteptwo_2\,\var$.
    To conclude, note that
    $\mstep_1 = \lam{\var}{\msteptwo_1\,\var}
     \tof_{\flatRule{EtaM}} \msteptwo_1$
    and
    $\mstep_2 = \lam{\var}{\msteptwo_2\,\var}
     \tof_{\flatRule{EtaM}} \msteptwo_2$
    noting that $\fv{\msteptwo_1},\fv{\msteptwo_2} \subseteq \fv{\msteptwo}$
    by \rlem{splitting_free_variables}.
  \end{enumerate}
\item
  {\bf Application, $\mstep = \mstepthree_1\,\mstepthree_2$.}
  Then note that $\judgSplit{\mstep}{\mstep_1}{\mstep_2}$
  must be derived using the \indrulename{SApp} rule,
  so $\judgSplit{\mstepthree_1}{\mstepthree_{11}}{\mstepthree_{12}}$
  and $\judgSplit{\mstepthree_2}{\mstepthree_{21}}{\mstepthree_{22}}$
  where $\mstep_1 = \mstepthree_{11}\,\mstepthree_{21}$
  and $\mstep_2 = \mstepthree_{12}\,\mstepthree_{22}$.
  We consider three subcases, depending on whether the step
  $\mstep = \mstepthree_1\,\mstepthree_2 \tof \msteptwo$
  is internal to $\mstepthree_1$,
  internal to $\mstepthree_2$,
  or a \flatRule{Beta} step at the root:
  \begin{enumerate}
  \item
    If the step is internal to $\mstepthree_1$,
    \ie $\mstepthree_1 \tof \mstepfour_1$
    and $\msteptwo = \mstepfour_1\,\mstepthree_2$,
    then by \ih we have that
    $\judgSplit{\mstepfour_1}{\mstepfour_{11}}{\mstepfour_{12}}$
    such that $\mstepthree_{11} \tofs \mstepfour_{11}$
    and $\mstepthree_{12} \tofs \mstepfour_{12}$.
    Therefore, by the \indrulename{SApp} rule,
    $\judgSplit{
       \msteptwo
     }{
       \mstepfour_{11}\,\mstepthree_{21}
     }{
       \mstepfour_{12}\,\mstepthree_{22}
     }$
    where
    $\mstep_1 = \mstepthree_{11}\,\mstepthree_{21} \tofs
                \mstepfour_{11}\,\mstepthree_{21}$
    and
    $\mstep_2 = \mstepthree_{12}\,\mstepthree_{22} \tofs
                \mstepfour_{12}\,\mstepthree_{22}$.
  \item
    If the step is internal to $\mstepthree_2$,
    \ie $\mstepthree_2 \tof \mstepfour_2$
    then by \ih we have that
    $\judgSplit{\mstepfour_2}{\mstepfour_{21}}{\mstepfour_{22}}$
    such that $\mstepthree_{21} \tofs \mstepfour_{21}$
    and $\mstepthree_{22} \tofs \mstepfour_{22}$.
    Therefore, by the \indrulename{SApp} rule,
    $\judgSplit{
       \msteptwo
     }{
       \mstepthree_{11}\,\mstepfour_{21}
     }{
       \mstepthree_{12}\,\mstepfour_{22}
     }$
    where
    $\mstep_1 = \mstepthree_{11}\,\mstepthree_{21} \tofs
                \mstepthree_{11}\,\mstepfour_{21}$
    and
    $\mstep_2 = \mstepthree_{12}\,\mstepthree_{22} \tofs
                \mstepthree_{12}\,\mstepfour_{22}$.
  \item
    If the step is a \flatRule{Beta} step at the root,
    \ie the step is of the form
    $\mstep = (\lam{\var}{\mstepthree'_1})\,\mstepthree_2
     \tof \mstepthree'_1\subm{\var}{\mstepthree_2} = \msteptwo$
    with $\mstepthree_1 = \lam{\var}{\mstepthree'_1}$,
    then note that
    $\judgSplit{\mstepthree_1}{\mstepthree_{11}}{\mstepthree_{12}}$
    must be derived using the \indrulename{SAbs} rule,
    so $\judgSplit{\mstepthree'_1}{\mstepthree'_{11}}{\mstepthree'_{12}}$
    with $\mstepthree_{11} = \lam{\var}{\mstepthree'_{11}}$
    and $\mstepthree_{12} = \lam{\var}{\mstepthree'_{12}}$.
    Then by \rlem{splitting_substitution} we have that
    $\judgSplit{
       \msteptwo
     }{
       \mstepthree'_{11}\subm{\var}{\mstepthree_{21}}
     }{
       \mstepthree'_{12}\subm{\var}{\mstepthree_{22}}
     }$
    where, moreover, we have that
    $\mstep_1 = (\lam{\var}{\mstepthree'_{11}})\,\mstepthree_{21}
     \tof_{\flatRule{Beta}} \mstepthree'_{11}\subm{\var}{\mstepthree_{21}}$
    and
    $\mstep_2 = (\lam{\var}{\mstepthree'_{12}})\,\mstepthree_{22}
     \tof_{\flatRule{Beta}} \mstepthree'_{12}\subm{\var}{\mstepthree_{22}}$.
  \end{enumerate}
\end{enumerate}
\end{proof}

%% No entiendo por qué no acepta el macro \tofnoeta en el título del lema,
%% lo reemplacé por \mapsto^\circ que no se ve exactamente igual.
\begin{lem}[Canonical $\mapsto^\circ,\etalong$-normal splitting]
\llem{canonical_splitting}
If $\judgSplit{\mstep_1}{\mstep_2}{\mstep_3}$
then there exist $\mstep'_1,\mstep'_2,\mstep'_3$
such that $\judgSplit{\mstep'_1}{\mstep'_2}{\mstep'_3}$
where
$\flatten{\mstep_1} = \flatten{(\mstep'_1)}$
and
$\flatten{\mstep_2} = \flatten{(\mstep'_2)}$
and
$\flatten{\mstep_3} = \flatten{(\mstep'_3)}$,
and moreover $\mstep'$ is in $\tofnoeta,\etalong$-normal form.
\end{lem}
\begin{proof}
By~\rlem{coherence_splitting_flattening},
we know that
$\judgSplit{\mstep''_1}{\mstep''_2}{\mstep''_3}$
where
$\mstep''_1 = \flatten{\mstep_1}$
and $\mstep_2 \tof \mstep''_2$
and $\mstep_3 \tof \mstep''_3$.
By induction on the shape of $\mstep''_1$,
it suffices to show that there exist $\mstep'_1,\mstep'_2,\mstep'_3$
such that
$\judgSplit{\mstep'_1}{\mstep'_2}{\mstep'_3}$
where $\flatten{(\mstep'_1)} = \flatten{(\mstep''_1)}$
and $\flatten{(\mstep'_2)} = \flatten{(\mstep''_2)}$
and $\flatten{(\mstep'_3)} = \flatten{(\mstep''_3)}$,
and moreover $\mstep'_1$ is in $\tofnoeta,\etalong$-normal form:
\begin{enumerate}
\item {\bf $\mstep''_1$ headed by a variable.}
  Then
  $\mstep''_1 =
   \lam{\var_1\hdots\var_n}{\vartwo\,\mstep''_{11}\hdots\mstep''_{1m}}$
  and
  $\mstep''_2 =
   \lam{\var_1\hdots\var_n}{\vartwo\,\mstep''_{21}\hdots\mstep''_{2m}}$
  and
  $\mstep''_3 =
    \lam{\var_1\hdots\var_n}{\vartwo\,\mstep''_{31}\hdots\mstep''_{3m}}$
  where $\judgSplit{\mstep''_{1i}}{\mstep''_{2i}}{\mstep''_{3i}}$
  for each $1 \leq i \leq m$.
  By \ih there are multisteps such that
  $\judgSplit{\mstep'_{1i}}{\mstep'_{2i}}{\mstep'_{3i}}$
  where $\flatten{(\mstep''_{1i})} = \flatten{(\mstep'_{1i})}$
  and $\flatten{(\mstep''_{2i})} = \flatten{(\mstep'_{2i})}$
  and $\flatten{(\mstep''_{3i})} = \flatten{(\mstep'_{3i})}$,
  and moreover $\mstep'_{1i}$ is in $\tofnoeta,\etalong$-normal form.
  Suppose that $\mstep''_1$ is of arity $N$,
  \ie that its type is
  of the form $\typ_1 \imp \hdots \imp \typ_N \imp \btyp$
  with $\btyp$ a base type.
  Take:
  \[
    \begin{array}{rll}
      \mstep'_1
    & := &
      \lam{\var_1\hdots\var_n\var_{n+1}\hdots\var_N}{
        \vartwo\,\mstep'_{11}\hdots\mstep'_{1m}\,\var_{n+1}\hdots\var_N
      }
    \\
      \mstep'_2
    & := &
      \lam{\var_1\hdots\var_n\var_{n+1}\hdots\var_N}{
        \vartwo\,\mstep'_{21}\hdots\mstep'_{2m}\,\var_{n+1}\hdots\var_N
      }
    \\
      \mstep'_3
    & := &
      \lam{\var_1\hdots\var_n\var_{n+1}\hdots\var_N}{
        \vartwo\,\mstep'_{31}\hdots\mstep'_{3m}\,\var_{n+1}\hdots\var_N
      }
    \end{array}
  \]
  Then it is straightforward to check that
  $\judgSplit{\mstep'_1}{\mstep'_2}{\mstep'_3}$
  and $\flatten{(\mstep'_1)} = \flatten{(\mstep''_1)}$
  and $\flatten{(\mstep'_2)} = \flatten{(\mstep''_2)}$
  and $\flatten{(\mstep'_3)} = \flatten{(\mstep''_3)}$,
  and moreover $\mstep'_1$ is in $\tofnoeta,\etalong$-normal form.
\item {\bf $\mstep''_1$ headed by a constant.}
  Similar to the previous case.
\item {\bf $\mstep''_1$ headed by a rule symbol.}
  Similar to the previous case.
\end{enumerate}
\end{proof}

\begin{prop}[Generalized \flateqRule{Perm} rule]
\lprop{generalized_flateq_perm}
If $\judgSplit{\mstep}{\mstep_1}{\mstep_2}$
then $\flatten{\mstep} \flateq \flatten{\mstep_1}\seq\flatten{\mstep_2}$.
\\
Note that this generalizes the \flateqRule{Perm} rule,
which requires $\mstep$ to be in $\tof$-normal form.
\end{prop}
\begin{proof}
By the previous coherence lemma~(\rlem{coherence_splitting_flattening}),
we have that
$\judgSplit{\flatten{\mstep}}{\mstep'_1}{\mstep'_2}$
such that $\mstep_1 \tofs \mstep'_1$
and $\mstep_2 \tofs \mstep'_2$.
By the \flateqRule{Perm} rule,
$\flatten{\mstep} \flateq \flatten{(\mstep'_1)} \seq \flatten{(\mstep'_2)}$.
Moreover, by strong normalization~(\rprop{flat_sn})
and confluence~(\rprop{flat_confluent}) of flattening,
$\flatten{\mstep_1} = \flatten{(\mstep'_1)}$
and
$\flatten{\mstep_2} = \flatten{(\mstep'_2)}$,
which means that
$\flatten{\mstep} \flateq \flatten{\mstep_1} \seq \flatten{\mstep_2}$.
\end{proof}

\begin{lem}[Swap]
\llem{flateq_swap}
\quad
\begin{enumerate}
\item $\flatten{(\mstep\,\msteptwo)}
       \flateq
       \flatten{(\refl{\rsrc{\mstep}}\,\msteptwo)}
       \seq
       \flatten{(\mstep\,\refl{\rtgt{\msteptwo}})}$
\item $\flatten{(\mstep\,\msteptwo)}
       \flateq
       \flatten{(\mstep\,\refl{\rsrc{\msteptwo}})}
       \seq
       \flatten{(\refl{\rtgt{\mstep}}\,\msteptwo)}$
\end{enumerate}
In particular, combining items~1. and~2. one has:
\[
  \flatten{(\refl{\rsrc{\mstep}}\,\msteptwo)}
  \seq
  \flatten{(\mstep\,\refl{\rtgt{\msteptwo}})}
  \flateq
  \flatten{(\mstep\,\refl{\rsrc{\msteptwo}})}
  \seq
  \flatten{(\refl{\rtgt{\mstep}}\,\msteptwo)}
\]
\end{lem}
\begin{proof}
For item~1. note that, by~\rprop{generalized_flateq_perm},
it suffices to show that
$\judgSplit{
   \mstep\,\msteptwo
 }{
   \refl{\rsrc{\mstep}}\,\msteptwo
 }{
   \mstep\,\refl{\rtgt{\msteptwo}}
 }$.
Indeed,
by \rlem{left_right_splitting} we have that
$\judgSplit{\mstep}{\refl{\rsrc{\mstep}}}{\mstep}$
and that
$\judgSplit{\msteptwo}{\msteptwo}{\refl{\rtgt{\msteptwo}}}$,
so by \indrulename{SApp}
$\judgSplit{
   \mstep\,\msteptwo
 }{
   \refl{\rsrc{\mstep}}\,\msteptwo
 }{
   \mstep\,\refl{\rtgt{\msteptwo}}
 }$.
The proof of item~2. is symmetric.
\end{proof}

\begin{lem}[Generalized swap]
\llem{flateq_generalized_swap}
The following equivalence holds
for arbitrary composition trees $\kctx_1,\kctx_2$
and arbitrary multisteps
$\mstep_1,\hdots,\mstep_n,\msteptwo_1,\hdots,\msteptwo_m$:
\[
  \begin{array}{rcll}
  &
    \kctx_1\ctxof{
      \flatten{(\mstep_1\,\refl{\rsrc{\msteptwo_1}})},
      \hdots,
      \flatten{(\mstep_n\,\refl{\rsrc{\msteptwo_1}})}
    }
    \seq
    \kctx_2\ctxof{
      \flatten{(\refl{\rtgt{\mstep_n}}\,\msteptwo_1)},
      \hdots,
      \flatten{(\refl{\rtgt{\mstep_n}}\,\msteptwo_m)}
    }
  \\
  \flateq &
    \kctx_2\ctxof{
      \flatten{(\refl{\rsrc{\mstep_1}}\,\msteptwo_1)},
      \hdots,
      \flatten{(\refl{\rsrc{\mstep_1}}\,\msteptwo_m)}
    }
    \seq
    \kctx_1\ctxof{
      \flatten{(\mstep_1\,\refl{\rtgt{\msteptwo_m}})},
      \hdots,
      \flatten{(\mstep_n\,\refl{\rtgt{\msteptwo_m}})}
    }
  \end{array}
\]
\end{lem}
\begin{proof}
We proceed by induction on $\kctx_1$.
To alleviate the notation
we use the associativity rule (\flateqRule{Assoc}) implicitly.
\begin{enumerate}
\item {\bf Empty, $\kctx_1 = \ctxhole$.}
  Then $n = 1$. We proceed by a nested induction on $\kctx_2$:
  \begin{enumerate}
  \item {\bf Empty, $\kctx_2 = \ctxhole$.}
    Then $m = 1$ and the following equivalence holds by~\rlem{flateq_swap}:
    \[
      \flatten{(\mstep_1\,\refl{\rsrc{\msteptwo_1}})}
      \seq
      \flatten{(\refl{\rtgt{\mstep_1}}\,\msteptwo_1)}
      \flateq
      \flatten{(\refl{\rsrc{\mstep_1}}\,\msteptwo_1)}
      \seq
      \flatten{(\mstep_1\,\refl{\rtgt{\msteptwo_1}})}
    \]
  \item {\bf Composition, $\kctx_2 = \kctx_{21}\seq\kctx_{22}$.}
    Then $m > 1$ and there is an index $1 \leq j \leq m$
    such that $\kctx_{21}$ has $j$ holes and $\kctx_{22}$ has $m-j$ holes.
    Then:
    \[
      \begin{array}{rcll}
      &&
        \flatten{(\mstep_1\,\refl{\rsrc{\msteptwo_1}})}
        \seq
        \kctx_2\ctxof{
          \flatten{(\refl{\rtgt{\mstep_1}}\,\msteptwo_1)},
          \hdots,
          \flatten{(\refl{\rtgt{\mstep_1}}\,\msteptwo_m)}
        }
      \\
      & = &
        \flatten{(\mstep_1\,\refl{\rsrc{\msteptwo_1}})}
        \seq
        \kctx_{21}\ctxof{
          \flatten{(\refl{\rtgt{\mstep_1}}\,\msteptwo_1)},
          \hdots,
          \flatten{(\refl{\rtgt{\mstep_1}}\,\msteptwo_j)}
        }
        \seq
        \kctx_{22}\ctxof{
          \flatten{(\refl{\rtgt{\mstep_1}}\,\msteptwo_{j+1})},
          \hdots,
          \flatten{(\refl{\rtgt{\mstep_1}}\,\msteptwo_m)}
        }
      \\
      & \flateq &
        \kctx_{21}\ctxof{
          \flatten{(\refl{\rsrc{\mstep_1}}\,\msteptwo_1)},
          \hdots,
          \flatten{(\refl{\rsrc{\mstep_1}}\,\msteptwo_j)}
        }
        \seq
        \flatten{(\mstep_1\,\refl{\rtgt{\msteptwo_j}})}
        \seq
        \kctx_{22}\ctxof{
          \flatten{(\refl{\rtgt{\mstep_1}}\,\msteptwo_{j+1})},
          \hdots,
          \flatten{(\refl{\rtgt{\mstep_1}}\,\msteptwo_m)}
        }
        \\&&\HS\text{by \ih}
      \\
      & = &
        \kctx_{21}\ctxof{
          \flatten{(\refl{\rsrc{\mstep_1}}\,\msteptwo_1)},
          \hdots,
          \flatten{(\refl{\rsrc{\mstep_1}}\,\msteptwo_j)}
        }
        \seq
        \flatten{(\mstep_1\,\refl{\rsrc{\msteptwo_{j+1}}})}
        \seq
        \kctx_{22}\ctxof{
          \flatten{(\refl{\rtgt{\mstep_1}}\,\msteptwo_{j+1})},
          \hdots,
          \flatten{(\refl{\rtgt{\mstep_1}}\,\msteptwo_m)}
        }
        \\&&\HS\text{as $\rtgt{\msteptwo_j} \termeq \rsrc{\msteptwo_{j+1}}$}
      \\
      & \flateq &
        \kctx_{21}\ctxof{
          \flatten{(\refl{\rsrc{\mstep_1}}\,\msteptwo_1)},
          \hdots,
          \flatten{(\refl{\rsrc{\mstep_1}}\,\msteptwo_j)}
        }
        \seq
        \kctx_{22}\ctxof{
          \flatten{(\refl{\rsrc{\mstep_1}}\,\msteptwo_{j+1})},
          \hdots,
          \flatten{(\refl{\rsrc{\mstep_1}}\,\msteptwo_m)}
        }
        \seq
        \flatten{(\mstep_1\,\refl{\rtgt{\msteptwo_m}})}
        \\&&\HS\text{by \ih}
      \\
      & = &
        \kctx_2\ctxof{
          \flatten{(\refl{\rsrc{\mstep_1}}\,\msteptwo_1)},
          \hdots,
          \flatten{(\refl{\rsrc{\mstep_1}}\,\msteptwo_m)}
        }
        \seq
        \flatten{(\mstep_1\,\refl{\rtgt{\msteptwo_m}})}
      \end{array}
    \]
  \end{enumerate}
\item {\bf Composition, $\kctx_1 = \kctx_{11}\seq\kctx_{12}$.}
  Then $n > 1$ and there is an index $1 \leq i \leq n$ such that
  $\kctx_{11}$ has $i$ holes and $\kctx_{12}$ has $n-i$ holes.
  Then:
  \[
    \begin{array}{rcll}
    &&
      \kctx_1\ctxof{
        \flatten{(\mstep_1\,\refl{\rsrc{\msteptwo_1}})},
        \hdots,
        \flatten{(\mstep_n\,\refl{\rsrc{\msteptwo_1}})}
      }
      \seq
      \kctx_2\ctxof{
        \flatten{(\refl{\rtgt{\mstep_n}}\,\msteptwo_1)},
        \hdots,
        \flatten{(\refl{\rtgt{\mstep_n}}\,\msteptwo_m)}
      }
    \\
    & = &
      \kctx_{11}\ctxof{
        \flatten{(\mstep_1\,\refl{\rsrc{\msteptwo_1}})},
        \hdots,
        \flatten{(\mstep_i\,\refl{\rsrc{\msteptwo_1}})}
      }
      \seq
      \\&&
      \kctx_{12}\ctxof{
        \flatten{(\mstep_{i+1}\,\refl{\rsrc{\msteptwo_1}})},
        \hdots,
        \flatten{(\mstep_n\,\refl{\rsrc{\msteptwo_1}})}
      }
      \seq
      \kctx_2\ctxof{
        \flatten{(\refl{\rtgt{\mstep_n}}\,\msteptwo_1)},
        \hdots,
        \flatten{(\refl{\rtgt{\mstep_n}}\,\msteptwo_m)}
      }
    \\
    & \flateq &
      \kctx_{11}\ctxof{
        \flatten{(\mstep_1\,\refl{\rsrc{\msteptwo_1}})},
        \hdots,
        \flatten{(\mstep_i\,\refl{\rsrc{\msteptwo_1}})}
      }
      \seq
      \\&&
      \kctx_2\ctxof{
        \flatten{(\refl{\rsrc{\mstep_{i+1}}}\,\msteptwo_1)},
        \hdots,
        \flatten{(\refl{\rsrc{\mstep_{i+1}}}\,\msteptwo_m)}
      }
      \seq
      \kctx_{12}\ctxof{
        \flatten{(\mstep_{i+1}\,\refl{\rtgt{\msteptwo_m}})},
        \hdots,
        \flatten{(\mstep_n\,\refl{\rtgt{\msteptwo_m}})}
      }
      \\&&\HS\text{by \ih}
    \\
    & = &
      \kctx_{11}\ctxof{
        \flatten{(\mstep_1\,\refl{\rsrc{\msteptwo_1}})},
        \hdots,
        \flatten{(\mstep_i\,\refl{\rsrc{\msteptwo_1}})}
      }
      \seq
      \\&&
      \kctx_2\ctxof{
        \flatten{(\refl{\rtgt{\mstep_i}}\,\msteptwo_1)},
        \hdots,
        \flatten{(\refl{\rtgt{\mstep_i}}\,\msteptwo_m)}
      }
      \seq
      \kctx_{12}\ctxof{
        \flatten{(\mstep_{i+1}\,\refl{\rtgt{\msteptwo_m}})},
        \hdots,
        \flatten{(\mstep_n\,\refl{\rtgt{\msteptwo_m}})}
      }
      \\&&\HS\text{since $\rtgt{\mstep_i} \termeq \rsrc{\mstep_{i+1}}$}
    \\
    & \flateq &
      \kctx_2\ctxof{
        \flatten{(\refl{\rsrc{\mstep_1}}\,\msteptwo_1)},
        \hdots,
        \flatten{(\refl{\rsrc{\mstep_1}}\,\msteptwo_m)}
      }
      \seq
      \\&&
      \kctx_{11}\ctxof{
        \flatten{(\mstep_1\,\refl{\rtgt{\msteptwo_m}})},
        \hdots,
        \flatten{(\mstep_i\,\refl{\rtgt{\msteptwo_m}})}
      }
      \seq
      \kctx_{12}\ctxof{
        \flatten{(\mstep_{i+1}\,\refl{\rtgt{\msteptwo_m}})},
        \hdots,
        \flatten{(\mstep_n\,\refl{\rtgt{\msteptwo_m}})}
      }
      \\&&\HS\text{by \ih}
    \\
    & = &
      \kctx_2\ctxof{
        \flatten{(\refl{\rsrc{\mstep_1}}\,\msteptwo_1)},
        \hdots,
        \flatten{(\refl{\rsrc{\mstep_1}}\,\msteptwo_m)}
      }
      \seq
      \kctx_1\ctxof{
        \flatten{(\mstep_1\,\refl{\rtgt{\msteptwo_m}})},
        \hdots,
        \flatten{(\mstep_n\,\refl{\rtgt{\msteptwo_m}})}
      }
    \end{array}
  \]
\end{enumerate}
\end{proof}

\begin{lem}[Flattening of an application, up to $\flateq$]
\llem{flattening_of_application_up_to_flateq}
Let $\redseq = \kctx_1\ctxof{\mstep_1,\hdots,\mstep_n}$
and $\redseqtwo = \kctx_2\ctxof{\msteptwo_1,\hdots,\msteptwo_m}$
be flat rewrites.
Then
\[
  \redseq\,\redseqtwo
  \ \tofs\flateq\ %
  \kctx_1\ctxof{
    \flatten{(\mstep_1\,\fsrc{\msteptwo_1})},
    \hdots,
    \flatten{(\mstep_n\,\fsrc{\msteptwo_1})}
  }
  \seq
  \kctx_2\ctxof{
    \flatten{(\ftgt{\mstep_n}\,\msteptwo_1)},
    \hdots,
    \flatten{(\ftgt{\mstep_n}\,\msteptwo_m)}
  }
\]
\end{lem}
\begin{proof}
We consider four subcases, depending on whether
$n = 1$ or $n > 1$, and on whether $m = 1$ or $m > 1$:
\begin{enumerate}
\item If $n = 1$ and $m = 1$, then:
  \[
    \begin{array}{rcll}
      \redseq\,\redseqtwo
    & \tofs &
      \flatten{(\mstep_1\,\msteptwo_1)}
    \\
    & \flateq &
      \flatten{(\mstep_1\,\refl{\rsrc{\msteptwo_1}})}
      \seq
      \flatten{(\refl{\rtgt{\mstep_1}}\,\msteptwo_1)}
      & \text{by \rlem{flateq_swap}}
    \\
    & = &
      \flatten{(\mstep_1\,\fsrc{\msteptwo_1})}
      \seq
      \flatten{(\ftgt{\mstep_1}\,\msteptwo_1)}
      & \text{by confluence of flattening~(\rprop{flat_confluent})}
    \end{array}
  \]
\item If $n = 1$ and $m > 1$, then:
  \[
    \begin{array}{rcll}
    &&
      \redseq\,\redseqtwo
    \\
    & \tofs &
      \mstep_1\,
      \kctx_2\ctxof{\msteptwo_1,\msteptwo_2,\hdots,\msteptwo_m}
    \\
    & \tofs &
      \kctx_2\ctxof{
        \mstep_1\,\msteptwo_1,
        \refl{\rtgt{\mstep_1}}\,\msteptwo_2,
        \hdots,
        \refl{\rtgt{\mstep_1}}\,\msteptwo_m
      }
      \\&&\HS\text{by generalized
                   \flatRule{App2}~(\rlem{generalized_flattening_kctx})}
    \\
    & \tofs &
      \kctx_2\ctxof{
        \flatten{(\mstep_1\,\msteptwo_1)},
        \flatten{(\refl{\rtgt{\mstep_1}}\,\msteptwo_2)},
        \hdots,
        \flatten{(\refl{\rtgt{\mstep_1}}\,\msteptwo_m)}
      }
    \\
    & \flateq &
      \kctx_2\ctxof{
        (
          \flatten{(\mstep_1\,\refl{\rsrc{\msteptwo_1}})}
          \seq
          \flatten{(\refl{\rtgt{\mstep_1}}\,\msteptwo_1)}
        ),
        \flatten{(\refl{\rtgt{\mstep_1}}\,\msteptwo_2)},
        \hdots,
        \flatten{(\refl{\rtgt{\mstep_1}}\,\msteptwo_m)}
      }
      & \text{by \rlem{flateq_swap}}
    \\
    & \flateq &
      \flatten{(\mstep_1\,\refl{\rsrc{\msteptwo_1}})}
      \seq
      \kctx_2\ctxof{
        \flatten{(\refl{\rtgt{\mstep_1}}\,\msteptwo_1)},
        \flatten{(\refl{\rtgt{\mstep_1}}\,\msteptwo_2)},
        \hdots,
        \flatten{(\refl{\rtgt{\mstep_1}}\,\msteptwo_m)}
      }
      & \text{by \rlem{generalized_flateq_assoc}}
    \\
    & = &
      \flatten{(\mstep_1\,\fsrc{\msteptwo_1})}
      \seq
      \kctx_2\ctxof{
        \flatten{(\ftgt{\mstep_1}\,\msteptwo_1)},
        \flatten{(\ftgt{\mstep_1}\,\msteptwo_2)},
        \hdots,
        \flatten{(\ftgt{\mstep_1}\,\msteptwo_m)}
      }
      & \text{by confluence of flattening~(\rprop{flat_confluent})}
    \end{array}
  \]
\item If $n > 1$ and $m = 1$, the proof is symmetric to the previous case.
\item If $n > 1$ and $m > 1$, then:
  \[
    \begin{array}{rcll}
      \redseq\,\redseqtwo
    & \tofs &
      \kctx_1\ctxof{\mstep_1,\hdots,\mstep_n}\,
      \kctx_2\ctxof{\msteptwo_1,\hdots,\msteptwo_m}
    \\
    & \tofs &
      \kctx_1\ctxof{
        \mstep_1\,\refl{\rsrc{\msteptwo_1}},
        \hdots,
        \mstep_n\,\refl{\rsrc{\msteptwo_1}}
      }
      \seq
      \kctx_2\ctxof{
        \refl{\rtgt{\mstep_n}}\,\msteptwo_1,
        \hdots,
        \refl{\rtgt{\mstep_n}}\,\msteptwo_m
      }
      \\&&\HS\text{by generalized 
                   \flatRule{App3}~(\rlem{generalized_flattening_kctx})}
    \\
    & \tofs &
      \kctx_1\ctxof{
        \flatten{(\mstep_1\,\refl{\rsrc{\msteptwo_1}})},
        \hdots,
        \flatten{(\mstep_n\,\refl{\rsrc{\msteptwo_1}})}
      }
      \seq
      \kctx_2\ctxof{
        \flatten{(\refl{\rtgt{\mstep_n}}\,\msteptwo_1)},
        \hdots,
        \flatten{(\refl{\rtgt{\mstep_n}}\,\msteptwo_m)}
      }
    \\
    & = &
      \kctx_1\ctxof{
        \flatten{(\mstep_1\,\fsrc{\msteptwo_1})},
        \hdots,
        \flatten{(\mstep_n\,\fsrc{\msteptwo_1})}
      }
      \seq
      \kctx_2\ctxof{
        \flatten{(\ftgt{\mstep_n}\,\msteptwo_1)},
        \hdots,
        \flatten{(\ftgt{\mstep_n}\,\msteptwo_m)}
      }
      \\&&\HS\text{by confluence of flattening~(\rprop{flat_confluent})}
    \end{array}
  \]
\end{enumerate}
\end{proof}

\begin{lem}[Composition of a term with itself]
\llem{flateq_composing_term_with_itself}
If $\tm$ is a term such that $\refl{\tm}$ is in $\tof$-normal form,
then
$\refl{\tm} \flateq \kctxof{\refl{\tm},\hdots,\refl{\tm}}$
for any composition tree $\kctx$.
\end{lem}
\begin{proof}
By induction on $\kctx$.
The key observation is that $\refl{\tm} \flateq \refl{\tm}\seq\refl{\tm}$
given that $\judgSplit{\tm}{\tm}{\tm}$, as can be checked easily by
induction on $\tm$.
\end{proof}

\begin{lem}[Arbitrary association]
\llem{flateq_arbitrary_association}
$\kctxof{\redseq_1,\redseq_2,\hdots,\redseq_n}
 \flateq
 \redseq_1\seq\redseq_2\hdots\seq\redseq_n$
where, on the right hand side, we assume that $\seq$ is right-associative.
\end{lem}
\begin{proof}
Straightforward by induction on $\kctx$ using the
\flateqRule{Assoc} rule.
\end{proof}

\begin{lem}[Equivalence for term/rewrite substitution of a composition]
\llem{flatten_equiv_subtr_composition}
Let $\tm$ be a term,
let $\mstep_1,\hdots,\mstep_n$ arbitrary multisteps,
and let $\kctx$ a composition tree.
Then:
\[
  \tm\subtr{\var}{\kctxof{\mstep_1,\hdots,\mstep_n}}
  \,\tofs\flateq\,
  \flatten{\kctxof{\tm\subtr{\var}{\mstep_1},\hdots,\tm\subtr{\var}{\mstep_n}}}
\]
\end{lem}
\begin{proof}
If $\tm$ has no free occurrences of $\var$,
the result holds trivially by~\rlem{flateq_composing_term_with_itself}.
The interesting case is when $\tm$ has $m > 0$ free occurrences of $\var$.
Following the notation of \rlem{flattening_subtr_composition},
let $\tm = \tm\ctxof{\var,\hdots,\var}$ where, by abuse of notation,
we write $\tm$ for the term itself and also for an $m$-hole context
that does not bind $\var$.

Recall from the notation introduced in~\rlem{flattening_subtr_composition}
that given indices $1 \leq i \leq m$
and $1 \leq j \leq n$
we write
$\tm\ctxof{\mstep_j}^\var_i$
to stand for the rewrite that results from
substituting the $i$-th free occurrence of $\var$ by $\mstep_j$,
the free occurrences of $\var$
at positions $i' < i$ by $\refl{\rtgt{\mstep_n}}$,
and the free occurrences of $\var$
at positions $i' > i$ by $\refl{\rsrc{\mstep_1}}$,
\ie
\[
  \tm\ctxof{\mstep_j}^\var_i =
  \tm\ctxof{
    \refl{\rtgt{\mstep_n}},\hdots,\refl{\rtgt{\mstep_n}},
    \underbrace{\mstep_j}_{\text{($i$-th position)}},
    \refl{\rsrc{\mstep_1}},\hdots,\refl{\rsrc{\mstep_1}}
  }
\]
In order to prove this lemma, we first prove two auxiliary results.
Intuitively, the first result allows one to swap consecutive multisteps
that perform work at the positions of two different free occurrences of $\var$.
The second result allows one to join consecutive multisteps
performing the same work for every position of $\var$.
Before we need to introduce some auxiliary notation:
\begin{enumerate}
\item[] {\bf Notation.}
  Given a sequence of $m$
  indices $(j_1,\hdots,j_m)$ such that $0 \leq j_k \leq n$
  for all $1 \leq k \leq m$ and an index $1 \leq i \leq m$
  such that $j_i > 0$,
  we write
  $\auxstep{i}{(j_1,\hdots,j_m)}$
  and
  $\auxstepf{i}{(j_1,\hdots,j_m)}$
  for the following multisteps:
  \[
    \begin{array}{rcl}
      \auxstep{i}{(j_1,\hdots,j_m)} & \eqdef &
      \tm\ctxof{
        \refl{\rtgt{\mstep_{j_1}}},\hdots,\refl{\rtgt{\mstep_{j_{i-1}}}},
        \underbrace{\mstep_{j_i}}_{\text{($i$-th position)}},
        \refl{\rtgt{\mstep_{j_{i+1}}}},\hdots,\refl{\rtgt{\mstep_{j_m}}}
      }
    \\
      \auxstepf{i}{(j_1,\hdots,j_m)} & \eqdef &
      \flatten{(\auxstep{i}{(j_1,\hdots,j_m)})}
    \end{array}
  \]
  where by convention $\rtgt{\mstep_0} := \rsrc{\mstep_1}$.
  Note that
  $\flatten{(\tm\ctxof{\mstep_j}^\var_i)} =
   \auxstepf{i}{(n,\hdots,n,j,0,\hdots,0)}$
  with $j$ in the $i$-th position.
  Intuitively,
  $\auxstep{i}{(j_1,\hdots,j_m)}$
  represents the transition from a state in which,
  for each $1 \leq k \leq m$,
  the $k$-th free ocurrence of $\var$
  has been replaced by the sequence $(\mstep_1\seq\hdots\seq\mstep_{j_k})$,
  and to a state in which the sequence in the $i$-th free occurrence of $\var$
  has been extended with the multistep $\mstep_{j_i+1}$.
\item[] {\bf Swapping consecutive steps.}
  Consecutive multisteps affecting different positions can be swapped.
  More precisely, we claim that
  if $1 \leq i < k \leq m$ then:
  \begin{equation}
  \leqn{flatten_equiv_subtr_composition_swap_equation}
    \auxstepf{i}{(j_1,\hdots,j_m)}
    \seq
    \auxstepf{k}{(j_1,\hdots,j_{(i-1)},j_i+1,j_{(i+1)},\hdots,j_m)}
    \flateq
    \auxstepf{k}{(j_1,\hdots,j_m)}
    \seq
    \auxstepf{i}{(j_1,\hdots,j_{(k-1)},j_k+1,j_{(k+1)},\hdots,j_m)}
  \end{equation}
  Indeed,
  if we let $\auxstep{(i,k)}{(j_1,\hdots,j_m)}$
  denote the step which, intuitively, combines the computational works
  of $\auxstep{i}{(j_1,\hdots,j_m)}$ and $\auxstep{k}{(j_1,\hdots,j_m)}$:
  \[
    \auxstep{(i,k)}{(j_1,\hdots,j_m)} \eqdef
      \tm\ctxof{
        \refl{\rtgt{\mstep_{j_1}}},\hdots,\refl{\rtgt{\mstep_{j_{i-1}}}},
        \mstep_{j_i},
        \refl{\rtgt{\mstep_{j_{i+1}}}},\hdots,\refl{\rtgt{\mstep_{j_{k-1}}}},
        \mstep_{j_k},
        \refl{\rtgt{\mstep_{j_{k+1}}}},\refl{\rtgt{\mstep_{j_m}}}
      }
  \]
  then we may justify
  equation \reqn{flatten_equiv_subtr_composition_swap_equation}
  by applying the
  generalized \flateqRule{Perm} rule~(\rprop{generalized_flateq_perm})
  and observing that the two following splittings hold:
  \[
   \judgSplit{
    \auxstep{(i,k)}{(j_1,\hdots,j_m)}
   }{
    \auxstep{i}{(j_1,\hdots,j_m)}
   }{
    \auxstep{k}{(j_1,\hdots,j_{(i-1)},j_i+1,j_{(i+1)},\hdots,j_m)}
   }
  \]
  \[
   \judgSplit{
    \auxstep{(i,k)}{(j_1,\hdots,j_m)}
   }{
    \auxstep{k}{(j_1,\hdots,j_m)}
   }{
    \auxstep{i}{(j_1,\hdots,j_{(k-1)},j_k+1,j_{(k+1)},\hdots,j_m)}
   }
  \]
\item[] {\bf Joining consecutive steps.}
  Consecutive multisteps performing the same computational work
  in the positions of all the free occurrences of $\var$ can be joined.
  More precisely, we claim that if $1 \leq i < n$ then:
  \begin{equation}
  \leqn{flatten_equiv_subtr_composition_join_equation}
    \auxstepf{1}{(i+1,i,\hdots,i)}
    \seq
    \auxstepf{2}{(i+1,i+1,i,\hdots,i)}
    \seq
    \hdots
    \seq
    \auxstepf{m}{(i+1,i+1,\hdots,i+1)}
    \flateq
    \flatten{\tm\subt{\var}{\mstep_{i+1}}}
  \end{equation}
  Indeed, if for each $0 \leq i < n$ and each $0 \leq j \leq m$
  we let $\auxstep{0..j}{i}$
  denote the step which, intuitively, combines the computational works
  of the first $j$ steps above:
  \[
    \auxstep{0..j}{i}
    \eqdef
      \tm\ctxof{
        \underbrace{
          \mstep_{(i+1)},\hdots,\mstep_{(i+1)}
        }_{\text{($j$)}},
        \underbrace{
          \refl{\rtgt{\mstep_{i}}},\hdots,\refl{\rtgt{\mstep_{i}}}
        }_{\text{($m-j$)}}
      }
  \]
  Then we may observe that the following splitting holds for every
  $0 \leq j < m$:
  \[
    \judgSplit{
      \auxstep{0..(j+1)}{i}
    }{
      \auxstep{0..j}{i}
    }{
      \auxstep{j+1}{(\underbrace{i+1,\hdots,i+1}_{\text{($j+1$)}},
                     \underbrace{i,\hdots,i}_{\text{($m-j-1$)}})}
    }
  \]
  Thus applying
  the generalized \flateqRule{Perm} rule~(\rprop{generalized_flateq_perm}),
  and using the \flateqRule{Assoc} rule implicitly,
  we have that:
  \[
    \begin{array}{rlll}
    &&
      \auxstepf{1}{(i+1,i,\hdots,i)}
      \seq
      \auxstepf{2}{(i+1,i+1,i,\hdots,i)}
      \seq
      \hdots
      \seq
      \auxstepf{m}{(i+1,\hdots,i+1,i+1)}
    \\
    & = &
      \flatten{(\auxstep{0..1}{i})}
      \seq
      \auxstepf{2}{(i+1,i+1,i,\hdots,i)}
      \seq
      \hdots
      \seq
      \auxstepf{m}{(i+1,\hdots,i+1,i+1)}
    \\
      & \flateq &
      \flatten{(\auxstep{0..2}{i})}
      \seq
      \auxstepf{3}{(i+1,i+1,i+1,i,\hdots,i)}
      \seq
      \hdots
      \seq
      \auxstepf{m}{(i+1,\hdots,i+1,i+1)}
      & \text{by \rprop{generalized_flateq_perm}}
    \\
      & \hdots &
    \\
      & \flateq &
      \flatten{(\auxstep{0..j}{i})}
      \seq
      \auxstepf{j+1}{(\underbrace{i+1,\hdots,i+1}_{\text{($j+1$)}},
                      \underbrace{i,\hdots,i}_{\text{($m-j-1$)}})}
      \seq
      \hdots
      \seq
      \auxstepf{m}{(i+1,i+1,\hdots,i+1,i)}
      & \text{by \rprop{generalized_flateq_perm}}
    \\
      & \hdots &
    \\
      & \flateq &
      \flatten{(\auxstep{0..m}{i})}
      & \text{by \rprop{generalized_flateq_perm}}
    \\
      & = &
      \flatten{\tm\subtr{\var}{\mstep_{i+1}}}
    \end{array}
  \]
\end{enumerate}
To conclude the proof of this lemma,
using the \flateqRule{Assoc} rule implicitly,
note that:
\[
{\small
  \begin{array}{rcll}
  &&
    \tm\subtr{\var}{\kctxof{\mstep_1,\hdots,\mstep_n}}
  \\
  & \tofs &
    \kctx'\ctxof{
      \tm\ctxof{\mstep_1}^\var_1,
      \hdots,
      \tm\ctxof{\mstep_n}^\var_1,
      \hdots,
      \tm\ctxof{\mstep_1}^\var_m,
      \hdots,
      \tm\ctxof{\mstep_n}^\var_m
    }
    \\&&\HS\text{by \rlem{flattening_subtr_composition}}
  \\
  & \tofs &
    \kctx'\ctxof{
      \flatten{(\tm\ctxof{\mstep_1}^\var_1)},
      \hdots,
      \flatten{(\tm\ctxof{\mstep_n}^\var_1)},
      \hdots,
      \flatten{(\tm\ctxof{\mstep_1}^\var_m)},
      \hdots,
      \flatten{(\tm\ctxof{\mstep_n}^\var_m)}
    }
  \\
  & \flateq &
    \flatten{(\tm\ctxof{\mstep_1}^\var_1)}
    \seq\hdots\seq
    \flatten{(\tm\ctxof{\mstep_n}^\var_1)}
    \seq\hdots\seq
    \flatten{(\tm\ctxof{\mstep_1}^\var_m)}
    \seq\hdots\seq
    \flatten{(\tm\ctxof{\mstep_n}^\var_m)}
    \\&&\HS\text{by \rlem{flateq_arbitrary_association}}
  \\
  & = &
    \auxstepf{1}{(1,0,\hdots,0)}\seq
    \auxstepf{1}{(2,0,\hdots,0)}
    \seq\hdots\seq
    \auxstepf{1}{(n,0,\hdots,0)}
    \seq\hdots\seq
    \auxstepf{m}{(n,\hdots,n,1)}\seq
    \auxstepf{m}{(n,\hdots,n,2)}
    \seq\hdots\seq
    \auxstepf{m}{(n,\hdots,n,n)}
  \\
  & \flateq &
    \auxstepf{1}{(1,0,\hdots,0)}\seq
    \auxstepf{2}{(1,1,0,\hdots,0)}
    \seq\hdots\seq
    \auxstepf{m}{(1,1,\hdots,1)}
    \seq\hdots\seq
    \auxstepf{1}{(n,n-1,\hdots,n-1)}\seq
    \auxstepf{2}{(n,n,n-1,\hdots,n-1)}
    \seq\hdots\seq
    \auxstepf{m}{(n,n,\hdots,n)}
    \\&&\HS\text{
             reordering the steps
             with equation \reqn{flatten_equiv_subtr_composition_swap_equation}
           }
  \\
  & \flateq &
    \flatten{\tm\subtr{\var}{\mstep_1}}
    \seq\hdots\seq
    \flatten{\tm\subtr{\var}{\mstep_n}}
    \\&&\HS\text{
             joining the steps
             with equation \reqn{flatten_equiv_subtr_composition_join_equation}
           }
  \\
  & \flateq &
    \kctxof{
      \flatten{\tm\subtr{\var}{\mstep_1}},
      \hdots,
      \flatten{\tm\subtr{\var}{\mstep_n}}
    }
    \\&&\HS\text{by \rlem{flateq_arbitrary_association}}
  \end{array}
}
\]
\end{proof}

\begin{lem}[Congruence for $\flateq$ below abstraction]
\llem{flateq_congruence_below_abstraction}
Let
$\kctx_1\ctxof{\mstep_1,\hdots,\mstep_n} \flateq
 \kctx_2\ctxof{\msteptwo_1,\hdots,\msteptwo_m}$.
Then:
\[
  \kctx_1\ctxof{
    \flatten{(\lam{\var}{\mstep_1})},
    \hdots,
    \flatten{(\lam{\var}{\mstep_n})}
  }
  \flateq
  \kctx_2\ctxof{
    \flatten{(\lam{\var}{\msteptwo_1})},
    \hdots,
    \flatten{(\lam{\var}{\msteptwo_m})}
  }
\]
{\bf Note.} The multisteps $\mstep_i$ and $\msteptwo_i$ are in
$\tof$-normal form because the $\flateq$ relation only relates
flat rewrites.
But observe that $\lam{\var}{\mstep_i}$ and $\lam{\var}{\msteptwo_i}$
may not necessarily be in $\tof$-normal form because
there may be an \flatRule{EtaM} redex at the root.
\end{lem}
\begin{proof}
If $\redseq$ is a flat rewrite, we define $\LAM{\var}{\redseq}$
as follows:
\[
  \begin{array}{rll}
    \LAM{\var}{\mstep}
  & \eqdef &
    \flatten{(\lam{\var}{\mstep})}
  \\
    \LAM{\var}{(\redseq\seq\redseqtwo)}
  & \eqdef &
    (\LAM{\var}{\redseq})\seq(\LAM{\var}{\redseqtwo})
  \end{array}
\]
Another way to state this lemma is to say that
$\redseq \flateq \redseqtwo$
implies
$\LAM{\var}{\redseq} \flateq \LAM{\var}{\redseqtwo}$.
The proof proceeds by induction on the derivation of
$\redseq \flateq \redseqtwo$.
The reflexivity, symmetry, and transitivity cases are immediate.
We analyze the cases in which an axiom is applied at the root,
as well as closure under composition contexts:
\begin{enumerate}
\item {\bf Rule \flateqRule{Assoc}.}
  Let
  $\redseq
   = ((\redseq_1\seq\redseq_2)\seq\redseq_3)
   \flateq (\redseq_1\seq(\redseq_2\seq\redseq_3)) = \redseqtwo$.
  Then
  $\LAM{\var}{\redseq}
   = ((\LAM{\var}{\redseq_1}\seq\LAM{\var}{\redseq_2})
     \seq\LAM{\var}{\redseq_3})
   \flateq (\LAM{\var}{\redseq_1}\seq
             (\LAM{\var}{\redseq_2}\seq\LAM{\var}{\redseq_3}))
  = \LAM{\var}{\redseqtwo}$
  can be derived applying the \flateqRule{Assoc} rule.
\item {\bf Rule \flateqRule{Perm}.}
  Let $\mstep \flateq \flatten{\mstep_1}\seq\flatten{\mstep_2}$
  be derived from $\judgSplit{\mstep}{\mstep_1}{\mstep_2}$.
  Then note that
  $\judgSplit{
     \lam{\var}{\mstep}
   }{
     \lam{\var}{\mstep_1}
   }{
     \lam{\var}{\mstep_2}
   }$
  holds by the \indrulename{SAbs} rule.
  Hence by the
  generalized \flateqRule{Perm} rule~(\rprop{generalized_flateq_perm})
  we have that
  $
    \flatten{(\lam{\var}{\mstep})}
    \flateq
    \flatten{(\lam{\var}{\mstep_1})}
    \seq
    \flatten{(\lam{\var}{\mstep_2})}
  $.
  Moreover,
  by confluence of flattening~(\rprop{flat_confluent}),
  we have that
  $
    \flatten{(\lam{\var}{\mstep})}
    \flateq
    \flatten{(\lam{\var}{\flatten{\mstep_1}})}
    \seq
    \flatten{(\lam{\var}{\flatten{\mstep_2}})}
  $.
\item {\bf Congruence (left of a composition).}
  Let
  $\redseq = (\redseq'\seq\redseqthree)
   \flateq (\redseqtwo'\seq\redseqthree) = \redseqtwo$
  be derived from $\redseq' \flateq \redseqtwo'$.
  Then by \ih we have that
  $\LAM{\var}{\redseq'} \flateq \LAM{\var}{\redseqtwo'}$,
  so
  $\LAM{\var}{\redseq}
   = (\LAM{\var}{\redseq'}\seq\LAM{\var}{\redseqthree})
   \flateq (\LAM{\var}{\redseqtwo'}\seq\LAM{\var}{\redseqthree})
   = \LAM{\var}{\redseqtwo}$.
\item {\bf Congruence (right of a composition).}
  Similar to the previous case.
\end{enumerate}
\end{proof}

\begin{lem}[Congruence for $\flateq$ below application]
\llem{flateq_congruence_below_application}
Let
$\kctx_1\ctxof{\mstep_1,\hdots,\mstep_n} \flateq
 \kctx_2\ctxof{\msteptwo_1,\hdots,\msteptwo_m}$
and let $\tm$ be an arbitrary term.
Then:
\begin{enumerate}
\item
  $
    \kctx_1\ctxof{
      \flatten{(\mstep_1\,\refl{\tm})},
      \hdots,
      \flatten{(\mstep_n\,\refl{\tm})}
    }
    \flateq
    \kctx_2\ctxof{
      \flatten{(\msteptwo_1\,\refl{\tm})},
      \hdots,
      \flatten{(\msteptwo_m\,\refl{\tm})}
    }
  $
\item
  $
    \kctx_1\ctxof{
      \flatten{(\refl{\tm}\,\mstep_1)},
      \hdots,
      \flatten{(\refl{\tm}\,\mstep_n)}
    }
    \flateq
    \kctx_2\ctxof{
      \flatten{(\refl{\tm}\,\msteptwo_1)},
      \hdots,
      \flatten{(\refl{\tm}\,\msteptwo_m)}
    }
  $
\end{enumerate}
\end{lem}
\begin{proof}
We only prove item~1. (item~2. is symmetric).
If $\redseq$ is a flat rewrite, we define $\APP{\redseq}{\tm}$
as follows:
\[
  \begin{array}{rcl}
    \APP{\mstep}{\tm}
  & \eqdef &
    \flatten{(\mstep\,\refl{\tm})}
  \\
    \APP{(\redseq\seq\redseqtwo)}{\tm}
  & \eqdef &
    (\APP{\redseq}{\tm})\seq(\APP{\redseqtwo}{\tm})
  \end{array}
\]
Another way to state item~1. is to say that
$\redseq \flateq \redseqtwo$
implies $\APP{\redseq}{\tm} \flateq \APP{\redseqtwo}{\tm}$.
The proof proceeds by induction on the derivation of
$\redseq \flateq \redseqtwo$.
The reflexivity, symmetry, and transitivity cases are immediate.
We analyze the cases in which an axiom is applied at the root,
as well as closure under composition contexts:
\begin{enumerate}
\item {\bf Rule $\flateqRule{Assoc}$.}
  Let
  $\redseq = ((\redseq_1\seq\redseq_2)\seq\redseq_3)
   \flateq (\redseq_1\seq(\redseq_2\seq\redseq_3)) = \redseqtwo$.
  Then
  $\APP{\redseq}{\tm}
   = ((\APP{\redseq_1}{\tm}\seq\APP{\redseq_2}{\tm})\seq\APP{\redseq_3}{\tm})
   \flateq
     (\APP{\redseq_1}{\tm}\seq(\APP{\redseq_2}{\tm}\seq\APP{\redseq_3}{\tm}))
   = \APP{\redseqtwo}{\tm}$
  can be derived applying the \flateqRule{Assoc} rule.
\item {\bf Rule $\flateqRule{Perm}$.}
  Let $\mstep \flateq \flatten{\mstep_1}\seq\flatten{\mstep_2}$
  be derived from $\judgSplit{\mstep}{\mstep_1}{\mstep_2}$.
  Then note that
  $\judgSplit{
     \mstep\,\refl{\tm}
   }{
     \mstep_1\,\refl{\tm}
   }{
     \mstep_2\,\refl{\tm}
    }$ holds by the \indrulename{SApp} rule,
  also using the straightforward fact that
  $\judgSplit{\refl{\tm}}{\refl{\tm}}{\refl{\tm}}$,
  given that $\tm$ is a term, \ie it has no occurrences of rule symbols.
  Then by the
  generalized \flateqRule{Perm} rule~(\rprop{generalized_flateq_perm})
  we have that
  $\flatten{(\mstep\,\refl{\tm})} \flateq
   \flatten{(\mstep_1\,\refl{\tm})}\seq\flatten{(\mstep_2\,\refl{\tm})}$.
  Moreover,
  by confluence of flattening~(\rprop{flat_confluent}),
  we have that
  $\flatten{(\mstep\,\refl{\tm})} \flateq
   \flatten{(\flatten{\mstep_1}\,\refl{\tm})}\seq
   \flatten{(\flatten{\mstep_2}\,\refl{\tm})}$,
  as required.
\item {\bf Congruence (left of a composition).}
  Let
  $\redseq
   = (\redseq'\seq\redseqthree)
   \flateq (\redseqtwo'\seq\redseqthree)
   = \redseqtwo$
  be derived from $\redseq' \flateq \redseqtwo'$.
  Then by \ih we have that $\APP{\redseq'}{\tm} \flateq \APP{\redseqtwo'}{\tm}$,
  so 
  $\APP{\redseq}{\tm}
   = (\APP{\redseq'}{\tm}\seq\APP{\redseqthree}{\tm})
   \flateq (\APP{\redseqtwo'}{\tm}\seq\APP{\redseqthree}{\tm})
   = \APP{\redseqtwo}{\tm}$.
\item {\bf Congruence (right of a composition).}
  Similar to the previous case.
\end{enumerate}
\end{proof}

\begin{thm}[Soundness and completeness of flat permutation equivalence]
\lthm{soundness_completeness_flateq}
Let $\judgRewr{\tenv}{\redseq}{\tm}{\tmtwo}{\typ}$
and $\judgRewr{\tenv}{\redseqtwo}{\tm'}{\tmtwo'}{\typ}$.
The following are equivalent:
\begin{enumerate}
\item $\redseq \permeq \redseqtwo$
\item $\flatten{\redseq} \flateq \flatten{\redseqtwo}$
\end{enumerate}
\end{thm}
\begin{proof}
The implication ($2 \implies 1$) is immediate,
given that reduction $\tof$ in the flattening system $\flatteningSystem$
is included in permutation equivalence~(\rlem{flattening_sound_wrt_permeq})
and, similarly, flat permutation equivalence
is included in permutation equivalence~(\rlem{flateq_sound_wrt_permeq}).
\smallskip\\
For the implication ($1 \implies 2$),
we proceed by induction on the derivation of $\redseq \permeq \redseqtwo$.
In the proof, sometimes we implicitly use the fact that $\tof$ is
strongly normalizing~(\rprop{flat_sn})
and confluent~(\rprop{flat_confluent}).
In particular, note that
$\flatten{(\redseq\seq\redseqtwo)} = \flatten{\redseq}\seq\flatten{\redseqtwo}$
and more in general
$\flatten{\kctxof{\redseq_1,\hdots,\redseq_n}} =
 \kctxof{\flatten{\redseq_1},\hdots,\flatten{\redseq_n}}$.
In the inductive proof, the cases for reflexivity,
symmetry, and transitivity are immediate. We analyze the cases when
a rule is applied at the root, as well as congruence closure under
rewrite constructors:
\begin{enumerate}
\item {\bf \permeqRule{IdL}.}
  Let $\refl{\rsrc{\redseq}}\seq\redseq \permeq \redseq$.
  Let $\flatten{\redseq} = \kctxof{\mstep_1,\hdots,\mstep_n}$.
  Note that $\rsrc{(\flatten{\redseq})} = \rsrc{\mstep_1}$.
  Then:
  \[
    \begin{array}{rcll}
      \flatten{(\refl{\rsrc{\redseq}}\seq\redseq)}
    & = &
      \flatten{(\refl{\rsrc{\redseq}})} \seq \flatten{\redseq}
    \\
    & = &
      \flatten{(\refl{\rsrc{(\flatten{\redseq})}})} \seq \flatten{\redseq}
      & \text{since by \rlem{coherence_of_flat_source_and_target}
          $\refl{\rsrc{(\flatten{\redseq})}} \tofs \flatten{(\refl{\rsrc{\redseq}})}$
        }
    \\
    & = &
      \flatten{(\refl{\rsrc{\mstep_1}})} \seq \flatten{\redseq}
      & \text{since $\rsrc{(\flatten{\redseq})} = \rsrc{\mstep_1}$}
    \\
    & = &
      \flatten{(\refl{\rsrc{\mstep_1}})} \seq \kctxof{\mstep_1,\hdots,\mstep_n}
    \\
    & = &
      \kctxof{(\flatten{(\refl{\rsrc{\mstep_1}})}\seq\mstep_1),\hdots,\mstep_n}
      & \text{by \rlem{generalized_flateq_assoc}}
    \\
    & \flateq &
      \kctxof{\mstep_1,\hdots,\mstep_n}
      & \text{since $\judgSplit{\mstep_1}{\refl{\rsrc{\mstep_1}}}{\mstep_1}$
              by \rlem{left_right_splitting}}
    \\
    & = &
      \flatten{\redseq}
    \end{array}
  \]
\item {\bf \permeqRule{IdR}.}
  Similar to the previous case.
  Let $\redseq\seq\refl{\rtgt{\redseq}} \permeq \redseq$.
  Let $\flatten{\redseq} = \kctxof{\mstep_1,\hdots,\mstep_n}$.
  Note that $\rtgt{(\flatten{\redseq})} = \rtgt{\mstep_n}$.
  \[
    \begin{array}{rcll}
      \flatten{\redseq\seq\refl{\rtgt{\redseq}}}
    & = &
      \flatten{\redseq}\seq\flatten{(\refl{\rtgt{\redseq}})}
    \\
    & = &
      \flatten{\redseq}\seq\flatten{(\refl{\rtgt{(\flatten{\redseq})}})}
      & \text{since by \rlem{coherence_of_flat_source_and_target}
          $\refl{\rtgt{(\flatten{\redseq})}}
           \tofs \flatten{(\refl{\rtgt{\redseq}})}$
        }
    \\
    & = &
      \flatten{\redseq}\seq\flatten{(\refl{\rtgt{\mstep_n}})}
      & \text{since $\rtgt{(\flatten{\redseq})} = \rtgt{\mstep_n}$}
    \\
    & = &
      \kctxof{\mstep_1,\hdots,\mstep_n}\seq\flatten{(\refl{\rtgt{\mstep_n}})}
      & \text{since $\rtgt{(\flatten{\redseq})} = \rtgt{\mstep_n}$}
    \\
    & \flateq &
      \kctxof{\mstep_1,\hdots,(\mstep_n\seq\flatten{(\refl{\rtgt{\mstep_n}})})}
      & \text{by \rlem{generalized_flateq_assoc}}
    \\
    & \flateq &
      \kctxof{\mstep_1,\hdots,\mstep_n}
      & \text{since $\judgSplit{\mstep_n}{\mstep_n}{\refl{\rtgt{\mstep_n}}}$
                 by \rlem{left_right_splitting}}
    \\
    & = &
      \flatten{\redseq}
    \end{array}
  \]
\item {\bf \permeqRule{Assoc}.}
  Let $(\redseq\seq\redseqtwo)\seq\redseqthree \permeq
       \redseq\seq(\redseqtwo\seq\redseqthree)$.
  Then
  \[
    \begin{array}{rlll}
      \flatten{((\redseq\seq\redseqtwo)\seq\redseqthree)}
    & = &
      (\flatten{\redseq}\seq\flatten{\redseqtwo})\seq\flatten{\redseqthree}
    \\
    & \flateq &
      \flatten{\redseq}\seq(\flatten{\redseqtwo}\seq\flatten{\redseqthree})
      & \text{by \flateqRule{Assoc}}
    \\
    & = &
      \flatten{(\redseq\seq(\redseqtwo\seq\redseqthree))}
    \end{array}
  \]
\item {\bf \permeqRule{Abs}.}
  Let $(\lam{\var}{\redseq})\seq(\lam{\var}{\redseqtwo})
       \permeq
       \lam{\var}{(\redseq\seq\redseqtwo)}$.
  It suffices to show that
  $\flatten{((\lam{\var}{\redseq})\seq(\lam{\var}{\redseqtwo}))} =
   \flatten{\lam{\var}{(\redseq\seq\redseqtwo)}}$.
  Indeed:
  \[
    \begin{array}{rlll}
      \lam{\var}{(\redseq\seq\redseqtwo)}
    & \tof &
      (\lam{\var}{\redseq})\seq(\lam{\var}{\redseqtwo})
      & \text{by \flatRule{Abs}}
    \\
    & \tofs &
      (\lam{\var}{\flatten{\redseq}})\seq(\lam{\var}{\flatten{\redseqtwo}})
    \\
    & = &
      \flatten{((\lam{\var}{\redseq})\seq(\lam{\var}{\redseqtwo}))}
    \end{array}
  \]
\item {\bf \permeqRule{App}.}
  Let $(\redseq_1\,\redseq_2)\seq(\redseqtwo_1\,\redseqtwo_2)
       \permeq
       (\redseq_1\seq\redseqtwo_1)\,(\redseq_2\seq\redseqtwo_2)$.
  Consider the $\tof$-normal forms of each rewrite:
  \[
    \begin{array}{ll}
      \flatten{\redseq_1} = \kctx_1\ctxof{\mstep_1,\hdots,\mstep_n}
    &
      \flatten{\redseq_2} = \kctx_2\ctxof{\msteptwo_1,\hdots,\msteptwo_m}
    \\
      \flatten{\redseqtwo_1} = \kctxB_1\ctxof{\mstepB_1,\hdots,\mstepB_p}
    &
      \flatten{\redseqtwo_2} = \kctxB_2\ctxof{\msteptwoB_1,\hdots,\msteptwoB_q}
    \end{array}
  \]
  Before going on, we make the following claim:
  \[
  \ftgt{\mstep_n} = \fsrc{\mstepB_1}
  \HS\text{ and }\HS
  \ftgt{\msteptwo_m} = \fsrc{\msteptwoB_1}
  \HS\HS\text{$(\star)$}
  \]
  For the first equality,
  note that $\redseq_1$ and $\redseqtwo_1$ are composable,
  so $\rtgt{\redseq_1} \termeq \rsrc{\redseqtwo_2}$
  are $\beta\eta$-equivalent terms.
  Moreover, by \rremark{flat_not_beta_steps_preserve_endpoints}
  and \rlem{flatten_beta_eta_source_target}
  we have that $\rtgt{(\flatten{\redseq_1})} \termeq \rtgt{\redseq_1}$
  and $\rsrc{(\flatten{\redseqtwo_1})} \termeq \rsrc{\redseqtwo_1}$.
  This means that $\rtgt{\mstep_n} \termeq \rsrc{\mstepB_1}$,
  so by confluence and strong normalization of flattening
  $\ftgt{\mstep_n} = \fsrc{\mstepB_1}$.
  Similarly, for the second equality,
  since $\redseq_2$ and $\redseqtwo_2$ are composable,
  we have that $\ftgt{\msteptwo_m} = \fsrc{\msteptwoB_1}$.

  Furthermore, we claim that the two following conditions hold:
  \begin{enumerate}
  \item[{\bf (I)}]
        $\redseq_1\,\redseq_2 \tofs\flateq
          \kctx_1\ctxof{
            \flatten{(\mstep_1\,\fsrc{\msteptwo_1})},
            \hdots,
            \flatten{(\mstep_n\,\fsrc{\msteptwo_1})}
          }
          \seq
          \kctx_2\ctxof{
            \flatten{(\fsrc{\mstepB_1}\,\msteptwo_1)},
            \hdots,
            \flatten{(\fsrc{\mstepB_1}\,\msteptwo_m)}
          }$
  \item[{\bf (II)}]
        $\redseqtwo_1\,\redseqtwo_2 \tofs\flateq
          \kctxB_1\ctxof{
            \flatten{(\mstepB_1\,\ftgt{\msteptwo_m})},
            \hdots,
            \flatten{(\mstepB_p\,\ftgt{\msteptwo_m})}
          }
          \seq
          \kctxB_2\ctxof{
            \flatten{(\ftgt{\mstepB_p}\,\msteptwoB_1)},
            \hdots,
            \flatten{(\ftgt{\mstepB_p}\,\msteptwoB_q)}
          }$
  \end{enumerate}
  To prove {\bf (I)}, note that:
  \[
    \begin{array}{rlll}
    &&
      \redseq_1\,\redseq_2
    \\
    & \tofs\flateq &
      \kctx_1\ctxof{
        \flatten{(\mstep_1\,\fsrc{\msteptwo_1})},
        \hdots,
        \flatten{(\mstep_n\,\fsrc{\msteptwo_1})}
      }
      \seq
      \kctx_2\ctxof{
        \flatten{(\ftgt{\mstep_n}\,\msteptwo_1)},
        \hdots,
        \flatten{(\ftgt{\mstep_n}\,\msteptwo_m)}
      }
      & \text{by \rlem{flattening_of_application_up_to_flateq}}
    \\
    & = &
      \kctx_1\ctxof{
        \flatten{(\mstep_1\,\fsrc{\msteptwo_1})},
        \hdots,
        \flatten{(\mstep_n\,\fsrc{\msteptwo_1})}
      }
      \seq
      \kctx_2\ctxof{
        \flatten{(\fsrc{\mstepB_1}\,\msteptwo_1)},
        \hdots,
        \flatten{(\fsrc{\mstepB_1}\,\msteptwo_m)}
      }
      & \text{by the claim $(\star)$ above}
    \end{array}
  \]
  The proof of {\bf (II)} is symmetric to the proof of {\bf (I)}.

  To conclude the proof of the \flateqRule{App} case,
  let us rewrite the left-hand side.
  We use the associativity rule (\flateqRule{Assoc}) implicitly:
    \[
      \begin{array}{rlll}
      &&
        (\redseq_1\,\redseq_2)\seq(\redseqtwo_1\,\redseqtwo_2)
      \\
      & \tofs\flateq &
        \kctx_1\ctxof{
          \flatten{(\mstep_1\,\fsrc{\msteptwo_1})},
          \hdots,
          \flatten{(\mstep_n\,\fsrc{\msteptwo_1})}
        }
        \seq
        \kctx_2\ctxof{
          \flatten{(\fsrc{\mstepB_1}\,\msteptwo_1)},
          \hdots,
          \flatten{(\fsrc{\mstepB_1}\,\msteptwo_m)}
        }
        \seq \\
        &&
        \kctxB_1\ctxof{
          \flatten{(\mstepB_1\,\ftgt{\msteptwo_m})},
          \hdots,
          \flatten{(\mstepB_p\,\ftgt{\msteptwo_m})}
        }
        \seq
        \kctxB_2\ctxof{
          \flatten{(\ftgt{\mstepB_p}\,\msteptwoB_1)},
          \hdots,
          \flatten{(\ftgt{\mstepB_p}\,\msteptwoB_q)}
        }
        \\&&\HS\text{by claims {\bf (I)} and {\bf (II)}}
      % (Missing associativity step)
      \\
      & \flateq &
         \kctx_1\ctxof{
           \flatten{(\mstep_1\,\fsrc{\msteptwo_1})},
           \hdots,
           \flatten{(\mstep_n\,\fsrc{\msteptwo_1})}
         }
         \seq
         \kctxB_1\ctxof{
           \flatten{(\mstepB_1\,\fsrc{\msteptwo_1})},
           \hdots,
           \flatten{(\mstepB_p\,\fsrc{\msteptwo_1})}
         }
         \seq
         \\&&
         \kctx_2\ctxof{
           \flatten{(\ftgt{\mstepB_p}\,\msteptwo_1)},
           \hdots,
           \flatten{(\ftgt{\mstepB_p}\,\msteptwo_m)}
         }
         \seq
         \kctxB_2\ctxof{
           \flatten{(\ftgt{\mstepB_p}\,\msteptwoB_1)},
           \hdots,
           \flatten{(\ftgt{\mstepB_p}\,\msteptwoB_q)}
         }
         \\&&\HS\text{by \rlem{flateq_generalized_swap}}
      \end{array}
    \]
    On the other hand, rewriting the right-hand side:
    \[
      \begin{array}{rcll}
      &&
        (\redseq_1\seq\redseqtwo_1)\,(\redseq_2\seq\redseqtwo_2)
      \\
      & \tofs &
        (
          \kctx_1\ctxof{\mstep_1,\hdots,\mstep_n}
          \seq
          \kctxB_1\ctxof{\mstepB_1,\hdots,\mstepB_p}
        )
        \,
        (
          \kctx_2\ctxof{\msteptwo_1,\hdots,\msteptwo_m}
          \seq
          \kctxB_2\ctxof{\msteptwoB_1,\hdots,\msteptwoB_q}
        )
      \\
        & \tofs &
        \kctx_1\ctxof{
          (\mstep_1\,\refl{\rsrc{\msteptwo_1}}),
          \hdots,
          (\mstep_n\,\refl{\rsrc{\msteptwo_1}})
        }
        \seq
        \kctxB_1\ctxof{
          (\mstepB_1\,\refl{\rsrc{\msteptwo_1}}),
          \hdots,
          (\mstepB_p\,\refl{\rsrc{\msteptwo_1}})
        }
        \seq
        \\&&
        \kctx_2\ctxof{
          (\refl{\rtgt{\mstepB_p}}\,\msteptwo_1),
          \hdots,
          (\refl{\rtgt{\mstepB_p}}\,\msteptwo_m)
        }
        \seq
        \kctxB_2\ctxof{
          (\refl{\rtgt{\mstepB_p}}\,\msteptwoB_1),
          \hdots,
          (\refl{\rtgt{\mstepB_p}}\,\msteptwoB_q)
        }
        \\&&\HS\text{by generalized
                     \flatRule{App3}~(\rlem{generalized_flattening_kctx})}
      \\
      & \tofs &
         \kctx_1\ctxof{
           \flatten{(\mstep_1\,\fsrc{\msteptwo_1})},
           \hdots,
           \flatten{(\mstep_n\,\fsrc{\msteptwo_1})}
         }
         \seq
         \kctxB_1\ctxof{
           \flatten{(\mstepB_1\,\fsrc{\msteptwo_1})},
           \hdots,
           \flatten{(\mstepB_p\,\fsrc{\msteptwo_1})}
         }
         \seq
         \\&&
         \kctx_2\ctxof{
           \flatten{(\ftgt{\mstepB_p}\,\msteptwo_1)},
           \hdots,
           \flatten{(\ftgt{\mstepB_p}\,\msteptwo_m)}
         }
         \seq
         \kctxB_2\ctxof{
           \flatten{(\ftgt{\mstepB_p}\,\msteptwoB_1)},
           \hdots,
           \flatten{(\ftgt{\mstepB_p}\,\msteptwoB_q)}
         }
      \end{array}
    \]

\item {\bf \permeqRule{BetaTR}.}
  Let $(\lam{\var}{\refl{\tm}})\,\redseq \permeq \tm\subtr{\var}{\redseq}$,
  and suppose that $\flatten{\redseq} = \kctxof{\mstep_1,\hdots,\mstep_n}$.
  First note that,
  $(\lam{\var}{\refl{\tm}})\,\redseq
   \tofs
   \kctxof{
     ((\lam{\var}{\refl{\tm}})\,\mstep_1),
     \hdots,
     ((\lam{\var}{\refl{\tm}})\,\mstep_n)
   }$.
  Indeed, if $n = 1$ this is immediate, and if $n > 1$
  this is a consequence of
  the generalized \flatRule{App2} rule~(\rlem{generalized_flattening_kctx}).
  Hence:
  \[
    \begin{array}{rlll}
      (\lam{\var}{\refl{\tm}})\,\redseq
    & \tofs &
      \kctxof{
        ((\lam{\var}{\refl{\tm}})\,\mstep_1),
        \hdots,
        ((\lam{\var}{\refl{\tm}})\,\mstep_n)
      }
    \\
    & \tofs &
      \kctxof{
        \tm\subm{\var}{\mstep_1},
        \hdots,
        \tm\subm{\var}{\mstep_n}
      }
      & \text{by \flatRule{BetaM} ($n$ times)}
    \\
    & = &
      \kctxof{
        \tm\subtr{\var}{\mstep_1},
        \hdots,
        \tm\subtr{\var}{\mstep_n}
      }
      & \text{by \rremark{multistep_substitution_vs_subtr_subrt}}
    \\
    & \tofs &
      \flatten{
        \kctxof{\tm\subtr{\var}{\mstep_1},\hdots,\tm\subtr{\var}{\mstep_n}}
      }
    \\
    & \flateq\tofsinv &
      \tm\subtr{\var}{\kctxof{\mstep_1,\hdots,\mstep_n}}
      & \text{by \rlem{flatten_equiv_subtr_composition}}
    \\
    & \tofsinv &
      \tm\subtr{\var}{\redseq}
      & \text{by \rlem{flattening_below_subtr}}
    \end{array}
  \]
\item {\bf \permeqRule{BetaRT}.}
  Let $(\lam{\var}{\redseq})\,\refl{\tm} \permeq \redseq\subt{\var}{\tm}$,
  and suppose that $\flatten{\redseq} = \kctxof{\mstep_1,\hdots,\mstep_n}$.
  First note that
  $(\lam{\var}{\redseq})\,\refl{\tm} \tofs
   \kctxof{(\lam{\var}{\mstep_1})\,\refl{\tm},\hdots,
           (\lam{\var}{\mstep_n})\,\refl{\tm}}$.
  Indeed, if $n = 1$ this is immediate, and if $n > 1$ this is a
  consequence of the generalized \flatRule{Abs}
  and \flatRule{App1} rules~(\rlem{generalized_flattening_kctx}).
  Hence:
  \[
    \begin{array}{rlll}
      (\lam{\var}{\redseq})\,\refl{\tm}
    & \tofs &
      \kctxof{(\lam{\var}{\mstep_1})\,\refl{\tm},\hdots,
              (\lam{\var}{\mstep_n})\,\refl{\tm}}
    \\
    & \tofs &
      \kctxof{
        \mstep_1\subm{\var}{\refl{\tm}},
        \hdots,
        \mstep_n\subm{\var}{\refl{\tm}}
      }
      & \text{by \flatRule{BetaM} ($n$ times)}
    \\
    & = &
      \kctxof{
        \mstep_1\subt{\var}{\tm},
        \hdots,
        \mstep_n\subt{\var}{\tm}
      }
      & \text{by \rremark{multistep_substitution_vs_subtr_subrt}}
    \\
    & = &
      \kctxof{\mstep_1,\hdots,\mstep_n}\subt{\var}{\tm}
    \\
    & \tofsinv &
      \redseq\subt{\var}{\tm}
      & \text{by \rlem{flattening_below_subrt}}
    \end{array}
  \]
\item {\bf \permeqRule{Eta}.}
  Let $\lam{\var}{\redseq\,\var} \permeq \redseq$
  where $\var\notin\fv{\redseq}$.
  Let $\flatten{\redseq} = \kctxof{\mstep_1,\hdots,\mstep_n}$.
  It suffices to note that
  $\flatten{(\lam{\var}{\redseq\,\var})} = \flatten{\redseq}$. Indeed:
  \[
    \begin{array}{rlll}
      \lam{\var}{\redseq\,\var}
    & \tofs &
      \lam{\var}{\flatten{\redseq}\,\var}
    \\
    & = &
      \lam{\var}{\kctxof{\mstep_1,\hdots,\mstep_n}\,\var}
    \\
    & \tofs &
      \lam{\var}{
        \kctxof{(\mstep_1\,\var),\hdots,(\mstep_n\,\var)}
      }
      & \text{by generalized
              \flatRule{App1}~(\rlem{generalized_flattening_kctx})}
    \\
    & \tofs &
      \kctxof{\lam{\var}{(\mstep_1\,\var)},\hdots,\lam{\var}{(\mstep_n\,\var)}}
      & \text{by generalized
              \flatRule{Abs}~(\rlem{generalized_flattening_kctx})}
    \\
    & \tofs &
      \kctxof{\mstep_1,\hdots,\mstep_n}
      & \text{by \flatRule{EtaM} ($n$ times)}
    \\
    & = &
      \flatten{\redseq}
    \end{array}
  \]
  Note that we may apply the \flatRule{EtaM} rule
  because, for each $1 \leq i \leq n$,
  we have that $\var \notin \fv{\mstep_i}$.
  This in turn is justified by noting that
  $\var \notin \fv{\kctxof{\mstep_1,\hdots,\mstep_n}}
             = \fv{\flatten{\redseq}}$,
  which is a consequence of the fact that
  flattening does not create free variables.
\item {\bf Congruence under an abstraction.}
  Let $\lam{\var}{\redseq} \permeq \lam{\var}{\redseqtwo}$
  be derived from $\redseq \permeq \redseqtwo$.
  Consider their $\tof$-normal forms,
  $\flatten{\redseq} = \kctx_1\ctxof{\mstep_1,\hdots,\mstep_n}$
  and $\flatten{\redseqtwo} = \kctx_2\ctxof{\msteptwo_1,\hdots,\msteptwo_m}$.
  By \ih we have that $\flatten{\redseq} \flateq \flatten{\redseqtwo}$.
  Then:
  \[
    \begin{array}{rlll}
      \lam{\var}{\redseq}
    & \tofs &
      \lam{\var}{\kctx_1\ctxof{\mstep_1,\hdots,\mstep_n}}
    \\
    & \tofs & 
      \kctx_1\ctxof{\lam{\var}{\mstep_1},\hdots,\lam{\var}{\mstep_n}}
      & \text{by generalized \flatRule{Abs} (\rlem{generalized_flattening_kctx})}
    \\
    & \tofs & 
      \kctx_1\ctxof{
        \flatten{(\lam{\var}{\mstep_1})},
        \hdots,
        \flatten{(\lam{\var}{\mstep_n})}
      }
    \\
    & \flateq &
      \kctx_2\ctxof{
        \flatten{(\lam{\var}{\msteptwo_1})},
        \hdots,
        \flatten{(\lam{\var}{\msteptwo_m})}
      }
      & \text{by \rlem{flateq_congruence_below_abstraction},
              as $\flatten{\redseq} \flateq \flatten{\redseqtwo}$}
    \\
    & \tofsinv &
      \kctx_2\ctxof{\lam{\var}{\msteptwo_1},\hdots,\lam{\var}{\msteptwo_m}}
    \\
    & \tofsinv &
      \lam{\var}{\kctx_2\ctxof{\msteptwo_1,\hdots,\msteptwo_m}}
      & \text{by generalized \flatRule{Abs} (\rlem{generalized_flattening_kctx})}
    \\
    & \tofsinv &
      \lam{\var}{\redseqtwo}
    \end{array}
  \]
\item {\bf Congruence under an application.}
  Let $\redseq_1\,\redseq_2 \permeq \redseqtwo_1\,\redseqtwo_2$
  be derived from $\redseq_1 \permeq \redseqtwo_1$
  and $\redseq_2 \permeq \redseqtwo_2$.
  Consider the $\tof$-normal forms of each rewrite:
  \[
    \begin{array}{ll}
      \flatten{\redseq_1} = \kctx_1\ctxof{\mstep_1,\hdots,\mstep_n}
    &
      \flatten{\redseq_2} = \kctx_2\ctxof{\msteptwo_1,\hdots,\msteptwo_m}
    \\
      \flatten{\redseqtwo_1} = \kctxB_1\ctxof{\mstepB_1,\hdots,\mstepB_p}
    &
      \flatten{\redseqtwo_2} = \kctxB_2\ctxof{\msteptwoB_1,\hdots,\msteptwoB_q}
    \end{array}
  \]
  By \ih we have that
  $\flatten{\redseq_1} \flateq \flatten{\redseqtwo_1}$
  and
  $\flatten{\redseq_2} \flateq \flatten{\redseqtwo_2}$.
  Before going on, we make the following claim:
  \[
    \fsrc{\msteptwo_1} = \fsrc{\msteptwoB_1}
    \HS\text{ and }\HS
    \fsrc{\mstep_n} = \fsrc{\mstepB_p}
    \HS\HS(\star)
  \]
  For the first equality, note that
  $\redseq_2 \permeq \redseqtwo_2$,
  so $\rsrc{\redseq_2} \termeq \rsrc{\redseqtwo_2}$
  are $\beta\eta$-equivalent terms by \rlem{permeq_endpoints_are_termeq}.
  Moreover, by \rremark{flat_not_beta_steps_preserve_endpoints}
  and \rlem{flatten_beta_eta_source_target}
  we have that $\rsrc{(\flatten{\redseq_2})} \termeq \rsrc{\redseq_2}$
  and $\rsrc{(\flatten{\redseqtwo_2})} \termeq \rsrc{\redseqtwo_2}$.
  This means that $\rsrc{\msteptwo_1} \termeq \rsrc{\msteptwoB_1}$,
  so by confluence and strong normalization of flattening
  $\fsrc{\msteptwo_1} = \fsrc{\msteptwoB_1}$.
  Similarly, for the second equality,
  since $\redseq_1 \permeq \redseqtwo_1$,
  we have that $\ftgt{\mstep_n} = \ftgt{\mstepB_p}$.
  Then:
  \[
    \begin{array}{rlll}
    &&
      \redseq_1\,\redseq_2
    \\
    & \tofs\flateq &
      \kctx_1\ctxof{
        \flatten{(\mstep_1\,\fsrc{\msteptwo_1})},
        \hdots,
        \flatten{(\mstep_n\,\fsrc{\msteptwo_1})}
      }
      \seq
      \kctx_2\ctxof{
        \flatten{(\ftgt{\mstep_n}\,\msteptwo_1)},
        \hdots,
        \flatten{(\ftgt{\mstep_n}\,\msteptwo_m)}
      }
      & \text{by \rlem{flattening_of_application_up_to_flateq}}
    \\
    & \flateq &
      \kctxB_1\ctxof{
        \flatten{(\mstepB_1\,\fsrc{\msteptwo_1})},
        \hdots,
        \flatten{(\mstepB_p\,\fsrc{\msteptwo_1})}
      }
      \seq
      \kctx_2\ctxof{
        \flatten{(\ftgt{\mstep_n}\,\msteptwo_1)},
        \hdots,
        \flatten{(\ftgt{\mstep_n}\,\msteptwo_m)}
      }
      & \text{by \rlem{flateq_congruence_below_application}
              as $\flatten{\redseq_1} \flateq \flatten{\redseqtwo_1}$}
    \\
    & \flateq &
      \kctxB_1\ctxof{
        \flatten{(\mstepB_1\,\fsrc{\msteptwo_1})},
        \hdots,
        \flatten{(\mstepB_p\,\fsrc{\msteptwo_1})}
      }
      \seq
      \kctxB_2\ctxof{
        \flatten{(\ftgt{\mstep_n}\,\msteptwoB_1)},
        \hdots,
        \flatten{(\ftgt{\mstep_n}\,\msteptwoB_q)}
      }
      & \text{by \rlem{flateq_congruence_below_application}
              as $\flatten{\redseq_2} \flateq \flatten{\redseqtwo_2}$}
    \\
    & = &
      \kctxB_1\ctxof{
        \flatten{(\mstepB_1\,\fsrc{\msteptwoB_1})},
        \hdots,
        \flatten{(\mstepB_p\,\fsrc{\msteptwoB_1})}
      }
      \seq
      \kctxB_2\ctxof{
        \flatten{(\ftgt{\mstepB_p}\,\msteptwoB_1)},
        \hdots,
        \flatten{(\ftgt{\mstepB_p}\,\msteptwoB_q)}
      }
      & \text{by the claim $(\star)$ above}
    \\
    & \tofsinv &
      \redseqtwo_1\,\redseqtwo_2
      & \text{by \rlem{flattening_of_application_up_to_flateq}}
    \end{array}
  \]
\item {\bf Congruence under a composition.}
  Let $\redseq_1\seq\redseq_2 \permeq \redseqtwo_1\seq\redseqtwo_2$
  be derived from
  $\redseq_1 \permeq \redseqtwo_1$ and $\redseq_2 \permeq \redseqtwo_2$.
  Then:
  \[
    \begin{array}{rlll}
      \flatten{(\redseq_1\seq\redseq_2)}
    & = &
      \flatten{\redseq_1}\seq\flatten{\redseq_2}
    \\
    & \flateq &
      \flatten{\redseqtwo_1}\seq\flatten{\redseqtwo_2}
      & \text{by \ih}
    \\
    & = &
      \flatten{(\redseqtwo_1\seq\redseqtwo_2)}
    \end{array}
  \]
\end{enumerate}
\end{proof}

%%% Local Variables:
%%% mode: latex
%%% TeX-master: "main"
%%% End:
