# Supplementary material for: Reductions in Higher-Order Rewriting and Their Equivalence
Source: arXiv:2210.15654 source file (2023-08-15)
Supplement: Supplementary file 5 [file a05-projection.tex]

\subsection{Projection for multisteps}

\begin{lem}[Matching]
\llem{matching}
If $\flatten{(\rsrc{\rulewit}\,\mstep_1\hdots\mstep_n)} =
    \flatten{(\rsrc{\rulewit}\,\msteptwo_1\hdots\msteptwo_n)}$
then $\flatten{\mstep_i} = \flatten{\msteptwo_i}$
for all $1 \leq i \leq n$.
\end{lem}
\begin{proof}
We begin with a few auxiliary definitions.
Let $\nctx$ be the set of $n$-hole term contexts generated by the
following grammar:
\[
  \nctx := \ctxhole
      \mid \lam{\var}{\nctx}
      \mid \var\,\nctx_1\hdots\nctx_n
      \mid \cons\,\nctx_1\hdots\nctx_n
\]
%Observe that a context $\nctx$ in this grammar is in $\beta$-normal form,
%and that all terms in $\beta$-normal form are $0$-hole contexts in this grammar.
Moreover,
if $\vec{\vartwo} = \vartwo_1,\hdots,\vartwo_n$ is a sequence of variables,
we write $\var\,\vec{\vartwo}$
for the application $\var\,\vartwo_1\hdots\vartwo_n$.
We prove an auxiliary result.

\begin{itemize}
\item[]
  {\bf Claim.}
  Let $V$ be a set of variables, and
  let $\nctx\ctxof{\var_1\vec{\vartwo_1},\hdots,\var_n\vec{\vartwo_n}}$
  be a term such that, for all $1 \leq i \leq n$,
  the variable $\var_i$ is not in $V$ nor bound by the context $\nctx$,
  and furthermore all the variables in the sequence $\vec{\vartwo_i}$
  are either in $V$ or bound by the context $\nctx$.
  Suppose moreover that
  $\mstep_1,\hdots,\mstep_n,\msteptwo_1,\hdots,\msteptwo_m$
  are multisteps
  whose free variables are disjoint from $V$, and such that
  $
    \flatten{
      \nctx\ctxof{
        \mstep_1\vec{\vartwo_1},
        \hdots,
        \mstep_n\vec{\vartwo_n}
      }
    }
  =
    \flatten{
      \nctx\ctxof{
        \msteptwo_1\vec{\vartwo_1},
        \hdots,
        \msteptwo_n\vec{\vartwo_n}
      }
    }
  $.
  Then $\flatten{\mstep_i} = \flatten{\msteptwo_i}$ for all $1 \leq i \leq n$.
\item[]
  {\em Proof of the claim.}
  By induction on $\nctx$:
  \begin{enumerate}
  \item $\nctx = \ctxhole$:
    Then $n = 1$ and by hypothesis
    $\flatten{(\mstep_1\,\vec{\vartwo_1})}
     = \flatten{(\msteptwo_1\,\vec{\vartwo_1})}$.
    Note that the variables in $\vec{\vartwo_1}$ do not occur
    free in $\mstep_1$ nor in $\msteptwo_2$.
    Then:
    \[
      \begin{array}{rlll}
        \mstep_1
      & \tofsinv &
        \lam{\vec{\vartwo_1}}{\mstep_1\,\vec{\vartwo_1}}
        & \text{repeatedly applying \flatRule{EtaM}}
      \\
      & \tofs &
        \lam{\vec{\vartwo_1}}{\flatten{(\mstep_1\,\vec{\vartwo_1})}}
      \\
      & = &
        \lam{\vec{\vartwo_1}}{\flatten{(\msteptwo_1\,\vec{\vartwo_1})}}
        & \text{by hypothesis}
      \\
      & \tofsinv &
        \lam{\vec{\vartwo_1}}{\msteptwo_1\,\vec{\vartwo_1}}
      \\
      & \tofs &
        \msteptwo_1
        & \text{repeatedly applying \flatRule{EtaM}}
      \end{array}
    \]
    Hence by confluence of flattening~(\rprop{flat_confluent})
    we have that $\flatten{\mstep_1} = \flatten{\msteptwo_1}$,
    as required.
  \item $\nctx = \lam{\varthree}{\nctx'}$:
    By hypothesis, we have that
    $
      \flatten{(
        \lam{\varthree}{
          \nctx'\ctxof{
            \mstep_1\,\vec{\vartwo_1},
            \hdots,
            \mstep_n\,\vec{\vartwo_n}
          }
        }
       )}
       =
      \flatten{(
        \lam{\varthree}{
          \nctx'\ctxof{
            \mstep_1\,\vec{\vartwo_1},
            \hdots,
            \mstep_n\,\vec{\vartwo_n}
          }
        }
       )}
     $.
     Then:
     \[
       \begin{array}{rlll}
         \nctx'\ctxof{
           \mstep_1\,\vec{\vartwo_1},
           \hdots,
           \mstep_n\,\vec{\vartwo_n}
         }
       & \tofinv &
         (\lam{\varthree}{\nctx'\ctxof{
           \mstep_1\,\vec{\vartwo_1},
           \hdots,
           \mstep_n\,\vec{\vartwo_n}
         }})\,\varthree
         & \text{by \flatRule{BetaM}}
       \\
       & \tofs &
         \flatten{(\lam{\varthree}{\nctx'\ctxof{
           \mstep_1\,\vec{\vartwo_1},
           \hdots,
           \mstep_n\,\vec{\vartwo_n}
         }})}\,\varthree
       \\
       & = &
         \flatten{(\lam{\varthree}{\nctx'\ctxof{
           \msteptwo_1\,\vec{\vartwo_1},
           \hdots,
           \msteptwo_n\,\vec{\vartwo_n}
         }})}\,\varthree
         & \text{by hypothesis}
       \\
       & \tofsinv &
         (\lam{\varthree}{\nctx'\ctxof{
           \msteptwo_1\,\vec{\vartwo_1},
           \hdots,
           \msteptwo_n\,\vec{\vartwo_n}
         }})\,\varthree
       \\
       & \tof &
         \nctx'\ctxof{
           \msteptwo_1\,\vec{\vartwo_1},
           \hdots,
           \msteptwo_n\,\vec{\vartwo_n}
         }
         & \text{by \flatRule{BetaM}}
       \end{array}
     \]
     Hence by confluence of flattening~(\rprop{flat_confluent})
     we have that:
     \[
       \flatten{
         \nctx'\ctxof{
           \mstep_1\,\vec{\vartwo_1},
           \hdots,
           \mstep_n\,\vec{\vartwo_n}
         }
       }
     = \flatten{
         \nctx'\ctxof{
           \msteptwo_1\,\vec{\vartwo_1},
           \hdots,
           \msteptwo_n\,\vec{\vartwo_n}
         }
       }
     \]
     Applying the \ih with the set of variables $V \cup \set{\varthree}$
     we conclude that $\flatten{\mstep_i} = \flatten{\msteptwo_i}$
     for all $1 \leq i \leq n$.
  \item $\nctx = \varthree\,\nctx_1\hdots\nctx_m$:
    Then there exist non-negative integers
    $0 = i_0 \leq i_1 \leq i_2 \leq \hdots \leq i_m = n$
    such that $\varthree\,\nctx_1\hdots\nctx_k$ has $i_k$ holes
    for every $1 \leq k \leq m$.
    In particular:
    \[
      \flatten{\nctxof{
        \mstep_1\,\vec{\vartwo_1},
        \hdots,
        \mstep_n\,\vec{\vartwo_n}
      }}
      =
      \varthree\,
        \flatten{\nctx_1\ctxof{
          \mstep_{i_0}\,\vec{\vartwo_{i_0}},
          \hdots,
          \mstep_{i_1}\,\vec{\vartwo_{i_1}}
        }}
        \hdots
        \flatten{\nctx_m\ctxof{
          \mstep_{i_{(m-1)}}\,\vec{\vartwo_{i_{(m-1)}}},
          \hdots,
          \mstep_{i_m}\,\vec{\vartwo_{i_m}}
        }}
    \]
    And similarly:
    \[
      \flatten{\nctxof{
        \msteptwo_1\,\vec{\vartwo_1},
        \hdots,
        \msteptwo_n\,\vec{\vartwo_n}
      }}
      =
      \varthree\,
        \flatten{\nctx_1\ctxof{
          \msteptwo_{i_0}\,\vec{\vartwo_{i_0}},
          \hdots,
          \msteptwo_{i_1}\,\vec{\vartwo_{i_1}}
        }}
        \hdots
        \flatten{\nctx_m\ctxof{
          \msteptwo_{i_{(m-1)}}\,\vec{\vartwo_{i_{(m-1)}}},
          \hdots,
          \msteptwo_{i_m}\,\vec{\vartwo_{i_m}}
        }}
    \]
    So for each $1 \leq k \leq m$ we have that
    \[
      \flatten{\nctx_k\ctxof{
        \mstep_{i_{(k-1)}}\,\vec{\vartwo_{i_{(k-1)}}},
        \hdots,
        \mstep_{i_k}\,\vec{\vartwo_{i_k}}
      }}
      =
      \flatten{\nctx_k\ctxof{
        \msteptwo_{i_{(k-1)}}\,\vec{\vartwo_{i_{(k-1)}}},
        \hdots,
        \msteptwo_{i_k}\,\vec{\vartwo_{i_k}}
      }}
    \]
    Applying the \ih for each value of $k$, we conclude
    $\flatten{\mstep_i} = \flatten{\msteptwo_i}$
    for all $1 \leq i \leq n$.
  \item $\nctx = \cons\,\nctx_1\hdots\nctx_m$:
    Similar to the previous case.
  \end{enumerate}
\end{itemize}
To conclude the proof of the lemma using the claim, recall that
$\rsrc{\rulewit}$ is in normal form and a rule-pattern,
so it can be written as
$\rsrc{\rulewit} =
 \lam{\var_1\hdots\var_n}{
   \nctxof{
     (\var_1\,\vec{\vartwo_{1}}),
     \hdots,
     (\var_n\,\vec{\vartwo_{n}})
   }
 }$.
Note that all of the variables in $\vec{\vartwo_i}$ are bound by $\nctx$
because $\rsrc{\rulewit}$ is a rule-pattern.
Moreover note that
  $\flatten{(\rsrc{\rulewit}\,\mstep_1\hdots\mstep_n)} =
   \flatten{
     \nctxof{
       \mstep_1\,\vec{\vartwo_{1}},
       \hdots,
       \mstep_n\,\vec{\vartwo_{n}}
     }
   }
   =
   \flatten{
     \nctxof{
       \msteptwo_1\,\vec{\vartwo_{1}},
       \hdots,
       \msteptwo_n\,\vec{\vartwo_{n}}
     }
   }
   = \flatten{(\rsrc{\rulewit}\,\msteptwo_1\hdots\msteptwo_n)}$.
By the claim, taking the set $V = \emptyset$,
we obtain that
$\flatten{\mstep_i} = \flatten{\msteptwo_i}$
for all $1 \leq i \leq n$, as required.
\end{proof}

\begin{lem}[Projection for compatible multisteps]
\llem{projection_for_compatible_multisteps}
Let $\judgCompat{\mstep}{\msteptwo}$.
Then there exists a unique $\mstepthree$
such that $\judgProj{\mstep}{\msteptwo}{\mstepthree}$.
\end{lem}
\begin{proof}
Straightforward
by induction on the derivation of $\judgCompat{\mstep}{\msteptwo}$.
\end{proof}

\begin{lem}[Projection of variables]
\llem{projection_of_variables}
Let $\mstep$ and $\msteptwo$ be multisteps such that
$\flatten{\mstep} = \flatten{\msteptwo} = \var$
and $\judgCompat{\mstep}{\msteptwo}$.
Moreover, let $\judgProj{\mstep}{\msteptwo}{\mstepthree}$.
Then $\flatten{\mstepthree} = \var$.
\end{lem}
\begin{proof}
By induction on the derivation of $\judgCompat{\mstep}{\msteptwo}$.
Note that this judgment can only be derived by the \indrulename{CVar} rule,
given that, in any other case, the head of $\mstep$
is either a constant $\cons$ or a rule symbol $\rulewit$,
which in turn implies that the head of $\flatten{\mstep}$
is either a constant or a rule symbol, contradicting the fact that
$\flatten{\mstep} = \var$.

This means that $\mstep = \lam{\vartwo_1\hdots\vartwo_n}{\varthree\,\mstep_1\hdots\mstep_m}$
and $\msteptwo = \lam{\vartwo_1\hdots\vartwo_n}{\varthree\,\msteptwo_1\hdots\msteptwo_m}$
where $\judgCompat{\mstep_i}{\msteptwo_i}$ for all $1 \leq i \leq n$.
Note that the head of $\flatten{\mstep}$ must be $\varthree$,
so $\varthree = \var$.
Moreover, by confluence of flattening~(\rprop{flat_confluent}),
$\flatten{\mstep} = \flatten{(\lam{\vartwo_1\hdots\vartwo_n}{\var\,\flatten{\mstep_1}\hdots\flatten{\mstep_m}})}$.
The term $\lam{\vartwo_1\hdots\vartwo_n}{\var\,\flatten{\mstep_1}\hdots\flatten{\mstep_m}}$
is already in \flatRule{BetaM}-normal form
so, given that the contraction of an \flatRule{EtaM} redex
does not create \flatRule{BetaM} redexes,
there is a reduction sequence
$\lam{\vartwo_1\hdots\vartwo_n}{\var\,\flatten{\mstep_1}\hdots\flatten{\mstep_m}} \tofs_{\flatRule{EtaM}} \var$
using only the \flatRule{EtaM} rule.
Given that each \flatRule{EtaM}-reduction step erases
exactly one abstraction and exactly one application,
it must be the case that $n = m$
and $\flatten{\mstep_i} = \vartwo_i$ for all $1 \leq i \leq n$.
Using a symmetric argument,
we have that $\flatten{\msteptwo_i} = \vartwo_i$ for all $1 \leq i \leq n$.

To sum up, the situation is that
$\mstep = \lam{\vartwo_1\hdots\vartwo_n}{\var\,\mstep_1\hdots\mstep_n}$
and
$\msteptwo = \lam{\vartwo_1\hdots\vartwo_n}{\var\,\msteptwo_1\hdots\msteptwo_n}$
with $\flatten{\mstep_i} = \flatten{\msteptwo_i} = \vartwo_i$ for all $1 \leq i \leq n$.
Note that $\judgProj{\mstep}{\msteptwo}{\mstepthree}$
where $\mstepthree$
must be of the form $\lam{\vartwo_1\hdots\vartwo_n}{\var\,\mstepthree_1\hdots\mstepthree_n}$
and $\judgProj{\mstep_i}{\msteptwo_i}{\mstepthree_i}$ for all $1 \leq i \leq n$.
By \ih, for each $1 \leq i \leq n$ we have that $\flatten{\mstepthree_i} = \vartwo_i$.
To conclude, note that:
\[
  \begin{array}{rlll}
        \flatten{\mstepthree}
  & = & \flatten{(\lam{\vartwo_1\hdots\vartwo_n}{\var\,\mstepthree_1\hdots\mstepthree_n})}
  \\
  & = & \flatten{(\lam{\vartwo_1\hdots\vartwo_n}{\var\,\vartwo_1\hdots\vartwo_n})}
      & \text{by confluence of flattening~(\rprop{flat_confluent})}
  \\
  & = & \var
      & \text{using the \flatRule{EtaM} rule ($n$ times)}
  \end{array}
\]
\end{proof}

\begin{defi}[Compatibility]
We give explicit names for the compatibility rules given in the
body:
\[
  \begin{array}{c}
  \indrule{CVar}{
    (\judgCompat{\mstep_i}{\msteptwo_i})_{i=1}^{m}
  }{
    \judgCompat{
      \lam{\varseq{\var}}{\vartwo\,\varseq{\mstep}}
    }{
      \lam{\varseq{\var}}{\vartwo\,\varseq{\msteptwo}}
    }
  }
  \indrule{CCon}{
    (\judgCompat{\mstep_i}{\msteptwo_i})_{i=1}^{m}
  }{
    \judgCompat{
      \lam{\varseq{\var}}{\cons\,\varseq{\mstep}}
    }{
      \lam{\varseq{\var}}{\cons\,\varseq{\msteptwo}}
    }
  }
  \indrule{CRule}{
    (\judgCompat{\mstep_i}{\msteptwo_i})_{i=1}^{m}
  }{
    \judgCompat{
      \lam{\varseq{\var}}{\rulewit\,\varseq{\mstep}}
    }{
      \lam{\varseq{\var}}{\rulewit\,\varseq{\msteptwo}}
    }
  }
  \\
  \\
  \indrule{CRuleL}{
    (\judgCompat{\mstep_i}{\msteptwo_i})_{i=1}^{m}
  }{
    \judgCompat{
      \lam{\varseq{\var}}{\rulewit\,\varseq{\mstep}}
    }{
      \lam{\varseq{\var}}{\rsrc{\rulewit}\,\varseq{\msteptwo}}
    }
  }
  \indrule{CRuleR}{
    (\judgCompat{\mstep_i}{\msteptwo_i})_{i=1}^{m}
  }{
    \judgCompat{
      \lam{\varseq{\var}}{\rsrc{\rulewit}\,\varseq{\mstep}}
    }{
      \lam{\varseq{\var}}{\rulewit\,\varseq{\msteptwo}}
    }
  }
  \end{array}
\]
\end{defi}

\begin{lem}[Coherence of projection]
\llem{coherence_of_projection}
Let $\mstep_1,\msteptwo_1,\mstep_2,\msteptwo_2$ be multisteps
such that:
\begin{enumerate}
\item
  $\judgCompat{\mstep_1}{\msteptwo_1}$
  and
  $\judgCompat{\mstep_2}{\msteptwo_2}$
\item
  $\flatten{\mstep_1} = \flatten{\mstep_2}$
  and
  $\flatten{\msteptwo_1} = \flatten{\msteptwo_2}$
\item
  $\judgProj{\mstep_1}{\msteptwo_1}{\mstepthree_1}$
  and
  $\judgProj{\mstep_2}{\msteptwo_2}{\mstepthree_2}$
\end{enumerate}
Then $\flatten{\mstepthree_1} = \flatten{\mstepthree_2}$.
\end{lem}
\begin{proof}
During this proof we use the following notion of {\bf arity}:
a multistep $\mstep$ is said to be {\em $n$-ary}
if its type, under the corresponding typing context,
is of the form $\typ_1\imp\hdots\imp\typ_n\imp\btyp$
where $\btyp$ is a base type.

The proof proceeds by induction on the
derivation of $\judgCompat{\mstep_1}{\msteptwo_1}$.
Note that the last rule used
to derive $\judgCompat{\mstep_2}{\msteptwo_2}$
must be the same as the last rule used
to derive $\judgCompat{\mstep_1}{\msteptwo_1}$.
For instance,
it cannot be the case that $\judgCompat{\mstep_1}{\msteptwo_1}$
is derived using the \indrulename{CVar} rule
and $\judgCompat{\mstep_2}{\msteptwo_2}$
is derived using the \indrulename{CCon} rule,
because this would mean that
$\mstep_1 = \lam{\var_1\hdots\var_n}{\vartwo\,\mstep_{11}\hdots\mstep_{1m}}$
and
$\mstep_2 = \lam{\var_1\hdots\var_n}{\cons\,\mstep_{21}\hdots\mstep_{2p}}$
and furthermore, by hypothesis,
$\flatten{\mstep_1} = \flatten{\mstep_2}$,
which is impossible,
given that the head of $\flatten{\mstep_1}$ is a variable $\vartwo$
whereas the head of $\flatten{\mstep_2}$ is a constant~$\cons$.
Recall that the left-hand side of a rule must be headed by a constant,
so using similar arguments
this can be shown for all the other cases as well. 

The only remaining possibilities are when
$\judgCompat{\mstep_1}{\msteptwo_1}$
and
$\judgCompat{\mstep_2}{\msteptwo_2}$
are derived using the same rule.
The core of the argument in these cases is to apply the \ih
using the matching lemma~(\rlem{matching}).
The difficulty is that, in the equalities
$\flatten{\mstep_1} = \flatten{\mstep_2}$ and
$\flatten{\msteptwo_1} = \flatten{\msteptwo_2}$,
flattening includes \flatRule{EtaM} reduction,
so we need to provide extra arguments to be able ``align''
the normal forms.

We only study the \indrulename{CRuleL} case
(the remaining cases are similar).
That is, suppose that
$\judgCompat{\mstep_1}{\msteptwo_1}$
and
$\judgCompat{\mstep_2}{\msteptwo_2}$
are derived by the \indrulename{CRuleL} rule.
Then:
\begin{itemize}
\item
  We have that
  $\mstep_1 =
   \lam{\var_1\hdots\var_n}{\rulewit\,\mstep_{11}\hdots\mstep_{1m}}$
  and
  $\msteptwo_1 =
   \lam{\var_1\hdots\var_n}{
     \rsrc{\rulewit}\,\msteptwo_{11}\hdots\msteptwo_{1m}}$
  where $\judgCompat{\mstep_{1i}}{\msteptwo_{1i}}$
  for all $1 \leq i \leq n$.
\item
  We have that
  $\mstep_2 =
   \lam{\var_1\hdots\var_p}{\rulewittwo\,\mstep_{21}\hdots\mstep_{2q}}$
  and
  $\msteptwo_2 =
   \lam{\var_1\hdots\var_p}{
     \rsrc{\rulewittwo}\,\msteptwo_{21}\hdots\msteptwo_{2q}}$
  where $\judgCompat{\mstep_{2i}}{\msteptwo_{2i}}$ for all $1 \leq i \leq q$.
\item
  Note that
  $\judgProj{\mstep_1}{\msteptwo_1}{
     \lam{\var_1\hdots\var_n}{
       \rulewit\,\mstepthree_{11}\hdots\mstepthree_{1m}
     }
   }$
  where $\judgProj{\mstep_{1i}}{\msteptwo_{1i}}{\mstepthree_{1i}}$
  for all $1 \leq i \leq n$.
\item
  Note that
  $\judgProj{\mstep_2}{\msteptwo_2}{
     \lam{\var_1\hdots\var_p}{
       \rulewit\,\mstepthree_{21}\hdots\mstepthree_{2q}
     }
   }$
  where $\judgProj{\mstep_{2i}}{\msteptwo_{2i}}{\mstepthree_{2i}}$
  for all $1 \leq i \leq q$.
\end{itemize}
Given that, by hypothesis, $\flatten{\mstep_1} = \flatten{\mstep_2}$,
we know that $\rulewit = \rulewittwo$.
Suppose that $\mstep_1$ is $N$-ary for some $N \geq 0$
and that $\rulewit$ is $M$-ary for some $M \geq 0$.
Then, since they all have the same types as $\mstep_1$,
we know that $\msteptwo_1,\mstep_2,\msteptwo_2$ must also be $N$-ary.
Similarly,
since $\rsrc{\rulewit}$ has the same type as $\rulewit$,
we know that it is $M$-ary.
Note that $n,p \leq N$ and $m,q \leq M$.
Moreover, note that $\mstep_1$ has $n$ explicit abstractions,
it is $N$-ary, and its body is $(M-m)$-ary,
so $n + M - m \leq N$.
Similarly, $p + M - q \leq N$.
Consider the multisteps $\mstep'_1,\msteptwo'_1,\mstep'_2,\msteptwo'_2$
that result from $\mstep_1,\msteptwo_1,\mstep_2,\msteptwo_2$
by performing $\eta$-expansions in order to ``complete''
the number of arguments in the body, to match the arity $M$:
\begin{itemize}
\item
  $\mstep'_1 = \lam{\var_1\hdots\var_n\var_{(n+1)}\hdots\var_{(n+M-m)}}{\rulewit\,\mstep_{11}\hdots\mstep_{1m}\,\var_{(n+1)}\hdots\var_{(n+M-m)}}$
\item
  $\msteptwo'_1 = \lam{\var_1\hdots\var_n\var_{(n+1)}\hdots\var_{(n+M-m)}}{\rsrc{\rulewit}\,\msteptwo_{11}\hdots\msteptwo_{1m}\,\var_{(n+1)}\hdots\var_{(n+M-m)}}$
\item
  $\mstep'_2 = \lam{\var_1\hdots\var_p\var_{(p+1)}\hdots\var_{(p+M-q)}}{\rulewit\,\mstep_{21}\hdots\mstep_{2q}\,\var_{(p+1)}\hdots\var_{(p+M-q)}}$
\item
  $\msteptwo'_2 = \lam{\var_1\hdots\var_p\var_{(p+1)}\hdots\var_{(p+M-q)}}{\rsrc{\rulewit}\,\msteptwo_{21}\hdots\msteptwo_{2q}\,\var_{(p+1)}\hdots\var_{(p+M-q)}}$
\end{itemize}
Note that by defining:
\[
  \begin{array}{rcll}
    \mstep_{1i} = \msteptwo_{1i} & \eqdef & \var_{n+i-m} & \text{for all $m + 1 \leq i \leq M$} \\
    \mstep_{2i} = \msteptwo_{2i} & \eqdef & \var_{p+i-q} & \text{for all $q + 1 \leq i \leq M$} \\
  \end{array}
\]
we have that the following equalities hold:
\[
  \begin{array}{rcll}
    \mstep'_1 & = & \lam{\var_1\hdots\var_{(n+M-m)}}{\redseq\,\mstep_{11}\hdots\mstep_{1M}}
  \\
    \msteptwo'_1 & = & \lam{\var_1\hdots\var_{(n+M-m)}}{\rsrc{\redseq}\,\msteptwo_{11}\hdots\msteptwo_{1M}}
  \\
    \mstep'_2 & = & \lam{\var_1\hdots\var_{(p+M-q)}}{\redseq\,\mstep_{21}\hdots\mstep_{2M}}
  \\
    \msteptwo'_2 & = & \lam{\var_1\hdots\var_{(p+M-q)}}{\rsrc{\redseq}\,\msteptwo_{21}\hdots\msteptwo_{2M}}
  \end{array}
\]
Before going on, we need to establish two auxiliary facts:
\begin{itemize}
\item[{\bf [A]}]
  Note that
  $\flatten{(\mstep'_1)} = \flatten{\mstep_1} = \flatten{\mstep_2} = \flatten{(\mstep'_2)}$.
  Then we have that:
  \[
    \begin{array}{rlll}
    &&
      \redseq\,\mstep_{11}\hdots\mstep_{1M}\,\var_{(n+M-m+1)}\hdots\var_N
    \\
    & \tofsinv &
      \mstep'_1\,\var_1\hdots\var_N
      & \text{by \flatRule{BetaM} ($N$ times)}
    \\
    & \tofs &
      \flatten{(\mstep'_1)}\,\var_1\hdots\var_N
    \\
    & = &
      \flatten{(\mstep'_2)}\,\var_1\hdots\var_N
      & \text{as remarked}
    \\
    & \tofs &
      \redseq\,\mstep_{21}\hdots\mstep_{2M}\,\var_{(p+M-q+1)}\hdots\var_N
      & \text{by \flatRule{BetaM} ($N$ times)}
    \end{array}
  \]
  By confluence of flattening~(\rprop{flat_confluent})
  this implies that:
  \[
    \flatten{(\redseq\,\mstep_{11}\hdots\mstep_{1M}\,\var_{(n+M-m+1)}\hdots\var_N)}
    =
    \flatten{(\redseq\,\mstep_{21}\hdots\mstep_{2M}\,\var_{(p+M-q+1)}\hdots\var_N)}
  \]
  Since $\rulewit$ is a ``rigid'' symbol,
  from this we obtain that $\flatten{\mstep_{1i}} = \flatten{\mstep_{2i}}$
  holds for all $1 \leq i \leq M$.
\item[{\bf [B]}]
  On the other hand, note that
  $\flatten{(\msteptwo'_1)} = \flatten{\msteptwo_1} = \flatten{\msteptwo_2} = \flatten{(\msteptwo'_2)}$
  so we have that:
  \[
    \begin{array}{rlll}
    &&
      \rsrc{\redseq}\,\msteptwo_{11}\hdots\msteptwo_{1M}\,\var_{(n+M-m+1)}\hdots\var_N
    \\
    & \tofsinv &
      \msteptwo'_1\,\var_1\hdots\var_N
      & \text{by \flatRule{BetaM} ($N$ times)}
    \\
    & \tofs &
      \flatten{(\msteptwo'_1)}\,\var_1\hdots\var_N
    \\
    & = &
      \flatten{(\msteptwo'_2)}\,\var_1\hdots\var_N
      & \text{as remarked}
    \\
    & \tofs &
      \rsrc{\redseq}\,\msteptwo_{21}\hdots\msteptwo_{2M}\,\var_{(p+M-q+1)}\hdots\var_N
      & \text{by \flatRule{BetaM} ($N$ times)}
    \end{array}
  \]
  By confluence of flattening~(\rprop{flat_confluent})
  this implies that:
  \[
    \flatten{(\rsrc{\redseq}\,\msteptwo_{11}\hdots\msteptwo_{1M}\,\var_{(n+M-m+1)}\hdots\var_N)}
    =
    \flatten{(\rsrc{\redseq}\,\msteptwo_{21}\hdots\msteptwo_{2M}\,\var_{(p+M-q+1)}\hdots\var_N)}
  \]
  By the matching lemma~(\rlem{matching}),
  from this we obtain that $\flatten{\msteptwo_{1i}} = \flatten{\msteptwo_{2i}}$
  holds for all $1 \leq i \leq M$.
\end{itemize}
\noindent
To conclude the proof, we consider two symmetric cases,
depending on whether $m \leq q$ or $q \leq m$.
Without loss of generality, suppose that $m \leq q$.
Note that:
\begin{itemize}
\item[{\bf [C]}]
  For every $i$ such that $1 \leq i \leq m$
  all of the following conditions hold:
  \[
    \begin{array}{l@{\hspace{1cm}}ll}
      \judgCompat{\mstep_{1i}}{\msteptwo_{1i}}
    &
      \judgCompat{\mstep_{2i}}{\msteptwo_{2i}}
    \\
      \flatten{\mstep_{1i}} = \flatten{\mstep_{2i}}
    &
      \flatten{\msteptwo_{1i}} = \flatten{\msteptwo_{2i}}
    &
      \text{by {\bf [A]} and {\bf [B]}}
    \\
      \judgProj{\mstep_{1i}}{\msteptwo_{1i}}{\mstepthree_{1i}}
    &
      \judgProj{\mstep_{2i}}{\msteptwo_{2i}}{\mstepthree_{2i}}
    \end{array}
  \]
  so by \ih we have that $\flatten{\mstepthree_{1i}} = \flatten{\mstepthree_{2i}}$.
\item[{\bf [D]}]
  For every $i$ such that $m < i \leq q$
  we have that $\flatten{\mstep_{1i}} = \flatten{\msteptwo_{1i}} = \var_{(n+i-m)}$
  by definition,
  and therefore $\flatten{\mstep_{2i}} = \flatten{\msteptwo_{2i}} = \var_{(n+i-m)}$
  by {\bf [A]} and {\bf [B]}.
  Hence by \rlem{projection_of_variables}
  we have that $\flatten{\mstepthree_{2i}} = \var_{(n+i-m)}$.
\item[{\bf [E]}]
  Thus we may build the following chain of reductions:
  \[
    \begin{array}{rlll}
    &&
      (\lam{\var_1\hdots\var_n}{\rulewit\,\mstepthree_{11}\hdots\mstepthree_{1m}})\,\var_1\hdots\var_N
    \\
    & \tofs &
      \rulewit\,\mstepthree_{11}\hdots\mstepthree_{1m}\,\var_{(n+1)}\hdots\var_N
      & \text{by \flatRule{BetaM} ($n$ times)}
    \\
    & \tofs &
      \rulewit\,\flatten{\mstepthree_{11}}\hdots\flatten{\mstepthree_{1m}}\,\var_{(n+1)}\hdots\var_N
    \\
    & \tofs &
      \rulewit\,\flatten{\mstepthree_{21}}\hdots\flatten{\mstepthree_{2m}}\,\var_{(n+1)}\hdots\var_N
      & \text{by {\bf [C]}}
    \\
    & = &
      \rulewit\,\flatten{\mstepthree_{21}}\hdots\flatten{\mstepthree_{2m}}\,\flatten{\mstepthree_{2(m+1)}}\hdots\flatten{\mstepthree_{2q}}\,\var_{(p+1)}\hdots\var_N
      & \text{by {\bf [D]}}
    \\
    & \tofsinv &
      \rulewit\,\mstepthree_{21}\hdots\mstepthree_{2q}\,\var_{(p+1)}\hdots\var_N
    \\
    & \tofsinv &
      (\lam{\var_1\hdots\var_p}{\rulewit\,\mstepthree_{21}\hdots\mstepthree_{2q}})\,\var_1\hdots\var_N
      & \text{by \flatRule{BetaM} ($p$ times)}
    \end{array}
  \]
\end{itemize}
Finally, we have:
\[
  \begin{array}{rlll}
    \flatten{\mstepthree_1}
  & = &
    \flatten{(\lam{\var_1\hdots\var_n}{\rulewit\,\mstepthree_{11}\hdots\mstepthree_{1m}})}
  \\
  & = &
    \flatten{(\lam{\var_1\hdots\var_N}{(\lam{\var_1\hdots\var_n}{\rulewit\,\mstepthree_{11}\hdots\mstepthree_{1m}})}\,\var_1\hdots\var_N)}
    & \text{by confluence using \flatRule{EtaM}}
  \\
  & = &
    \flatten{(\lam{\var_1\hdots\var_N}{(\lam{\var_1\hdots\var_p}{\rulewit\,\mstepthree_{21}\hdots\mstepthree_{2q}})}\,\var_1\hdots\var_N)}
    & \text{by confluence and {\bf [E]}}
  \\
  & = &
    \flatten{(\lam{\var_1\hdots\var_p}{\rulewit\,\mstepthree_{21}\hdots\mstepthree_{2q}})}
    & \text{by confluence using \flatRule{EtaM}}
  \\
  & = &
    \flatten{\mstepthree_2}
  \end{array}
\]
\end{proof}

\begin{defi}[$\eta$-expanded source]
If $\mstep$ is a multistep in $\etalong$-normal form,
we write $\altsrc{\mstep}$ for the source of $\mstep$
in which the sources of rule symbols are also $\eta$-expanded.
More precisely:
\[
  \begin{array}{rcll}
    \altsrc{\var} & \eqdef & \var \\
    \altsrc{\cons} & \eqdef & \cons \\
    \altsrc{\rulewit} & \eqdef & \tm'
    & \text{
        if $\rewr{\rulewit}{\tm}{\tmtwo}{\typ} \in \ruleset$
        and $\tm'$ is the $\etalong$-normal form of $\tm$
      } \\
    \altsrc{(\lam{\var}{\mstep})} & \eqdef & \lam{\var}{\altsrc{\tm}} \\
    \altsrc{(\mstep\,\msteptwo)} & \eqdef & \altsrc{\mstep}\,\altsrc{\msteptwo}
  \end{array}
\]
Note that $\altsrc{\mstep} \tofs \rsrc{\mstep}$
so, in particular,
$\flatten{(\altsrc{\mstep})} = \flatten{(\rsrc{\mstep})} = \fsrc{\mstep}$.
\end{defi}

\begin{lem}[Constructor/rule matching]
\llem{coinitial_cons_rule}
Let $\mstep = \lam{\var_1\hdots\var_n}{\cons\,\mstep_1\hdots\mstep_m}$
and $\msteptwo = \lam{\vartwo_1\hdots\vartwo_p}{
                   \rulewit\,\msteptwo_1\hdots\msteptwo_q}$.
Let $\rewr{\rulewit}{l_0}{r_0}{\typ}\in\ruleset$
and let $l,r$ be the $\toetaexp$-normal forms of $l_0,r_0$ respectively.
Suppose that $\rsrc{\mstep} \termeq \rsrc{\msteptwo}$
and, moreover, that $\mstep$ and $\msteptwo$ are in
$\tofnoeta,\etalong$-normal form. Then there exist multisteps
$\mstepthree_1,\ldots,\mstepthree_q$ such that:
\[
  \mstep = \flattennoeta{
             (\lam{\var_1\hdots\var_n}{
                \refl{l}\,\mstepthree_1\hdots\mstepthree_q})
           }
\]
and
$\flattennoeta{(\altsrc{\mstepthree_i})}
 = \flattennoeta{(\altsrc{\msteptwo_i})}$
for all $1 \leq i \leq q$.\smallskip\\
Furthermore, the multisteps $\mstepthree_i$
can be chosen in such a way that they are in $\tofnoeta,\etalong$-normal form,
and the number of applications in each
multistep $\mstepthree_i$, for all $1 \leq i \leq k$,
is strictly less than the number of applications in $\mstep$.
\end{lem}
\begin{proof}
Note that the condition $\rsrc{\mstep} \termeq \rsrc{\msteptwo}$
implies that $\flatten{(\rsrc{\mstep})} = \flatten{(\rsrc{\msteptwo})}$.
Then also $\flatten{(\altsrc{\mstep})} = \flatten{(\altsrc{\msteptwo})}$.
By \rlem{flattening_of_eta_expanded_multisteps} this implies that:
\begin{equation}
  \flattennoeta{(\altsrc{\mstep})} = \flattennoeta{(\altsrc{\msteptwo})}
  \label{eq:orthogonal:multisteps}
\end{equation}
Suppose
$l=\lam{\varthree_1}{\ldots \lam{\varthree_k}{\constwo\,r_1\ldots r_{k'}}}$.
From~(\ref{eq:orthogonal:multisteps}) we have:
\[
  \flattennoeta{(\lam{\var_1\hdots\var_n}{
                  \cons\,\altsrc{\mstep_1}\hdots\altsrc{\mstep_m}})}
  =
  \flattennoeta{(\lam{\vartwo_1\hdots\vartwo_p}{
                  l\,\altsrc{\msteptwo}_1\hdots\altsrc{\msteptwo_q}})}
\]
Since
$\cons\,\altsrc{\mstep_1}\hdots\altsrc{\mstep_m}$ and
$l\,\altsrc{\msteptwo}_1\hdots\altsrc{\msteptwo_q}$ have base
types, then $n=p$
and we may assume that $\var_i=\vartwo_i$, for all $1 \leq i \leq p$.
Moreover,
\[
  \flattennoeta{(\cons\,\altsrc{\mstep_1}\hdots\altsrc{\mstep_m})}
  = \flattennoeta{(l\,\altsrc{\msteptwo}_1\hdots\altsrc{\msteptwo_q})}
\]
Therefore $\constwo=\cons$, $q=k$ and $m=k'$, and:
\[
  \flattennoeta{(\altsrc{\mstep_i})}
  =
  \flattennoeta{
    (r_i\subm{\varthree_1}{\altsrc{\msteptwo}_1}
        \ldots
        \subm{\varthree_k}{\altsrc{\msteptwo_k}})
  }
\]
for all $1 \leq i \leq m$.
Note that each $r_i$ is part of the pattern of
the rewrite rule $l$. By orthogonality of $\ruleset$,
there exist $\mstepthree_1,\hdots,\mstepthree_k$ such that:
\[
  \mstep_i =
  \flattennoeta{(r_i\subm{\varthree_1}{\mstepthree_1}
                    \ldots
                    \subm{\varthree_k}{\mstepthree_k})}
  \HS\text{for all $1 \leq i \leq m$}
\]
and 
\[
  \flattennoeta{(\altsrc{\mstepthree_i})} 
  = \flattennoeta{(\altsrc{\msteptwo_i})}
  \HS\text{for all $1 \leq i \leq k$}
\]
Therefore:
\[
  \mstep
  = \lam{\var_1\hdots\var_n}{\cons\,\mstep_1\ldots \mstep_m}
  =
  \flattennoeta{
    (\lam{\var_1\hdots\var_n}{l\,\mstepthree_1\hdots\mstepthree_k})
  }
\]

Furthermore, we claim that each $\mstepthree_i$, for $1 \leq i \leq k$,
can be chosen in such a way that it is in $\tofnoeta,\etalong$-normal form
and with strictly less applications than $\mstep$.
First, note that if the $\mstepthree_i$ are not in $\tofnoeta$-normal form,
then we may take $\mstepthreeB_i := \flattennoeta{\mstepthree_i}$
instead, and we still have that
$
  \mstep
  =
  \flattennoeta{
    (\lam{\var_1\hdots\var_n}{l\,\mstepthree_1\hdots\mstepthree_k})
  }
  =
  \flattennoeta{
    (\lam{\var_1\hdots\var_n}{
       l\,\mstepthreeB_1
          \hdots
          \mstepthreeB_k
     }
    )
  }
$
by confluence of flattening~(\rprop{flat_confluent}).
So let us assume that the $\mstepthree_i$ are in $\tofnoeta$-normal form.
Furthermore, suppose that
$\mstepthree_i$ is of arity $N$,
\ie its type is of the form
$\typ_{1} \imp \hdots \imp \typ_{N} \imp \btyp$
with $\btyp$ a base type,
and suppose that
$\mstepthree_i = \lam{\varfour_1\hdots\varfour_M}{\mstepthree'_i}$
where $\mstepthree'_i$ is not a $\lambda$-abstraction.
Note that $M \leq N$.
Take
$\mstepthreeB_i :=
 \lam{\varfour_1\hdots\varfour_M\varfour_{M+1}\hdots\varfour_{N}}{
   \mstepthree'_i\,\varfour_{M+1}\hdots\varfour_{N}
 }$.
Note that each $\mstepthreeB_i$ is in $\tofnoeta$-normal form.

To conclude, we claim that
$
  \mstep
  =
  \flattennoeta{
    (\lam{\var_1\hdots\var_n}{\refl{l}\,\mstepthreeB_1\hdots\mstepthreeB_k})
  }
$
and that each $\mstepthreeB_i$
has strictly less applications than $\mstep$.
To see this, note that
each variable $\varthree_1,\hdots,\varthree_k$.
occurs free exactly once in the body of $l$,
applied to different bound variables.
More precisely, for a fixed index $1 \leq i_0 \leq k$
there is exactly one $1 \leq j_0 \leq m$
such that $\varthree_{i_0}$ occurs free in $r_j$.
Then the multistep that results from substituting in $r_j$
each $\varthree_i$ by $\mstepthreeB_i$ other than for $i = i_0$
contains exactly one occurrence of $\varthree_{i_0}$
applied to $N$ variables, where $N$ is the arity of $\mstepthreeB_{i_0}$,
that is, it is of the form:
\[
  r_j\subm{\varthree_1}{\mstepthree_1}
     \hdots
     \subm{\varthree_{(i_0-1)}}{\mstepthree_{(i_0-1)}}
     \subm{\varthree_{(i_0+1)}}{\mstepthree_{(i_0+1)}}
     \hdots
     \subm{\varthree_k}{\mstepthree_k}
  =
  \cctxof{\varthree_{i_0}\,\varfour_1 \hdots \varfour_N}
\]
where $\varfour_1,\hdots,\varfour_N$ are bound by $\cctx$
and the hole of $\cctx$ is not applied.
As a consequence, we have that:
\[
  \begin{array}{rll}
    \mstep
  & = &
    \lam{\var_1\hdots\var_n}{
      \cons\mstep_1
           \hdots
           \mstep_{i_0-1}\,
           \cctxof{\flattennoeta{(\mstepthreeB_{i_0}\,\varfour_1\hdots\,\varfour_N)}}\,
           \mstep_{i_0+1}
           \hdots
           \mstep_m
    }
  \\
  & = &
    \lam{\var_1\hdots\var_n}{
      \cons\mstep_1
           \hdots
           \mstep_{i_0-1}\,
           \cctxof{
             \flattennoeta{
               ((\lam{\varfour_1\hdots\varfour_N}{
                   \mstepthree_{i_0}\,\varfour_{M+1}\hdots\varfour_{N}
                 })
                 \,\varfour_1\hdots\,\varfour_N)
             }
           }\,
           \mstep_{i_0+1}
           \hdots
           \mstep_m
    }
  \\
  & = &
    \lam{\var_1\hdots\var_n}{
      \cons\mstep_1
           \hdots
           \mstep_{i_0-1}\,
           \cctxof{
             \mstepthree_{i_0}\,\varfour_{M+1}\hdots\varfour_{N}
           }\,
           \mstep_{i_0+1}
           \hdots
           \mstep_m
    }
  \end{array}
\]
Hence, since $\mstep$ is in $\etalong$-normal form,
and $\mstepthree_{i_0}\,\varfour_{M+1}\hdots\varfour_{N}$
is a subterm of $\mstep$ which is not applied,
we know that $\mstepthree_{i_0}\,\varfour_{M+1}\hdots\varfour_{N}$
is in $\etalong$-normal form.
Hence
$\mstepthreeB_{i_0} =
 \lam{\varfour_1\hdots\varfour_n}{
   \mstepthree_{i_0}\,\varfour_{M+1}\hdots\varfour_{N}
 }$
is also in $\etalong$-normal form.

Finally,
note that
$
  \flattennoeta{
    (\lam{\var_1\hdots\var_n}{\refl{l}\,\mstepthreeB_1\hdots\mstepthreeB_k})
  }
$
is in $\tofnoeta,\etalong$-normal form
and that
$\flatten{\mstep} =
 \flatten{
   (\lam{\var_1\hdots\var_n}{\refl{l}\,\mstepthree_1\hdots\mstepthree_k})
 }
 =
 \flatten{
   (\lam{\var_1\hdots\var_n}{\refl{l}\,\mstepthreeB_1\hdots\mstepthreeB_k})
 }$
so by \rlem{flattening_of_eta_expanded_multisteps}
$\flattennoeta{\mstep} =
 \flattennoeta{
   (\lam{\var_1\hdots\var_n}{\refl{l}\,\mstepthreeB_1\hdots\mstepthreeB_k})
 }$.
Moreover, for each $1 \leq i_0 \leq k$
the multistep
$\mstepthreeB_{i_0} =
 \lam{\var_1\hdots\var_N}{\mstepthree_{i_0}\,\var_{M+1}\hdots\var_N}$
has the same number of applications as
$\mstepthree_{i_0}\,\var_{M+1}\hdots\var_M$,
which is a subterm of $\mstep$,
and has strictly less applications than $\mstep$.
\end{proof}

\begin{lem}[Compatibilization of coinitial multisteps]
\llem{compatibilization_of_coinitial_multisteps}
Let $\mstep,\msteptwo$ be multisteps
such that $\fsrc{\mstep} = \fsrc{\msteptwo}$.
Then there exist multisteps $\mstepB,\msteptwoB$
such that $\judgCompat{\mstepB}{\msteptwoB}$
and moreover $\flatten{\mstepB} = \flatten{\mstep}$
and $\flatten{\msteptwoB} = \flatten{\msteptwo}$.
\end{lem}
\begin{proof}
We begin with a few observations.
Recall that if $\mstep \tofs \mstep'$
then $\rsrc{\mstep} \termeq \rsrc{\mstep'}$,
which is a consequence of
\rremark{flat_not_beta_steps_preserve_endpoints}
and \rlem{flatten_beta_eta_source_target}.
This means that, without loss of generality, we may assume that
$\mstep,\msteptwo$ are in $\tofnoeta,\etalong$-normal form.
Note that, given this assumption,
we have that $\altsrc{\mstep}$ and $\altsrc{\mstep}$ are
in $\etalong$-normal form.
Moreover,
$\flatten{(\altsrc{\mstep})}
 = \flatten{(\rsrc{\mstep})}
 = \flatten{(\rsrc{\msteptwo})}
 = \flatten{(\altsrc{\msteptwo})}$.
From this,
by \rlem{flattening_of_eta_expanded_multisteps},
we have that
$\flattennoeta{(\altsrc{\mstep})}
 = \flattennoeta{(\altsrc{\msteptwo})}$.

The proof proceeds by induction
on the sum of the number of applications in $\mstep$ and $\msteptwo$,
using the characterization of flat multisteps~(\rlem{normal_multisteps}).
We consider three cases, depending on whether the head of $\mstep$
is a variable, a constant, or a rule symbol:
\begin{enumerate}
\item
  \label{compatibilization_of_coinitial_multisteps__case_var}
  {\bf Variable,
       $\mstep = \lam{\var_1\hdots\var_n}{\vartwo\,\mstep_1\hdots\mstep_m}$.}
  Note that
  $\flattennoeta{(\altsrc{\mstep})} =
   \lam{\var_1\hdots\var_n}{
     \vartwo\,\flattennoeta{(\altsrc{\mstep_1})}
              \hdots
              \flattennoeta{(\altsrc{\mstep_m})}
   }$.
  Since $\flattennoeta{(\altsrc{\mstep})} =
         \flattennoeta{(\altsrc{\msteptwo})}$,
  the head of $\msteptwo$ cannot be a constant or a rule symbol.
  Hence the only possibility is that
  $\msteptwo = \lam{\var_1\hdots\var_p}{\vartwo\,\msteptwo_1\hdots\msteptwo_q}$.
  Furthermore, it can only be the case that $p = n$ and $q = m$
  and $\flattennoeta{(\altsrc{\mstep_i})} =
       \flattennoeta{(\altsrc{\msteptwo_i})}$
  for all $1 \leq i \leq m$.
  This in turn implies that
  $\fsrc{\mstep_i} = \fsrc{\msteptwo_i}$ for all $1 \leq i \leq m$.
  Hence, by \ih, for each $1 \leq i \leq m$,
  there exist multisteps such that
  $\judgCompat{\mstepB_i}{\msteptwoB_i}$
  where $\flatten{\mstepB_i} = \flatten{\mstep_i}$
  and $\flatten{\msteptwoB_i} = \flatten{\msteptwo_i}$.
  To conclude, note that
  taking
  $\mstepB := \lam{\var_1\hdots\var_n}{\vartwo\,\mstepB_1\hdots\mstepB_m}$
  and
  $\msteptwoB := \lam{\var_1\hdots\var_n}{\vartwo\,\msteptwoB_1\hdots\msteptwoB_m}$
  we have that
  $\judgCompat{\mstepB}{\msteptwoB}$ by the \indrulename{CVar} rule,
  and moreover
  $\flatten{\mstepB} = \flatten{\mstep}$
  and
  $\flatten{\msteptwoB} = \flatten{\msteptwo}$.
\item
  {\bf Constant,
    $\mstep = \lam{\var_1\hdots\var_n}{\cons\,\mstep_1\hdots\mstep_m}$.
  }
  Note that
  $\flattennoeta{(\altsrc{\mstep})} =
   \lam{\var_1\hdots\var_n}{
     \cons\,\flattennoeta{(\altsrc{\mstep_1})}\hdots
            \flattennoeta{(\altsrc{\mstep_m})}
   }$.
  Since $\flattennoeta{(\altsrc{\msteptwo})} =
         \flattennoeta{(\altsrc{\mstep})}$,
  the head of $\msteptwo$ cannot be a variable.
  We consider two cases, depending on whether the head of $\msteptwo$
  is a constant or a rule symbol:
  \begin{enumerate}
  \item
    {\bf Constant,
      $\msteptwo = \lam{\var_1\hdots\var_p}{
                     \cons\,\msteptwo_1\hdots\msteptwo_q
                   }$.}
    The proof of this case proceeds similarly
    as for case~\ref{compatibilization_of_coinitial_multisteps__case_var},
    when the heads of $\mstep$ and $\msteptwo$ are both variables.
  \item
    \label{compatibilization_of_coinitial_multisteps__case_cons_rule}
    {\bf Rule symbol,
      $\msteptwo = \lam{\var_1\hdots\var_p}{\rulewit\,\msteptwo_1\hdots\msteptwo_q}$.
    }
    Recall that we assume that $\mstep$ and $\msteptwo$ are
    in $\etalong$-normal form. This implies that $n = p$.
    Then
    $\flattennoeta{(\altsrc{\msteptwo})} =
     \flattennoeta{
       (\lam{\var_1\hdots\var_n}{
         \altsrc{\rulewit}\,\altsrc{\msteptwo_1}\hdots\altsrc{\msteptwo_q}
       })
     }$.
    By \rlem{coinitial_cons_rule}, there exist multisteps
    $\mstepthree_1,\hdots,\mstepthree_q$
    such that
    $\mstep =
     \flattennoeta{
       (\lam{\var_1\hdots\var_n}{
         \altsrc{\rulewit}\,\mstepthree_1\hdots\mstepthree_q
       })
     }$
    and $\flattennoeta{(\altsrc{\mstepthree_i})} =
         \flattennoeta{(\altsrc{\msteptwo_i})}$
    for all $1 \leq i \leq q$.
    Moreover, each $\mstepthree_i$ has less applications than $\mstep$.
    So by \ih, for each $1 \leq i \leq q$
    there exist multisteps such that
    $\judgCompat{\mstepthreeB_i}{\msteptwoB_i}$
    where
    $\flatten{\mstepthreeB_i} = \flatten{\mstepthree_i}$.
    and
    $\flatten{\msteptwoB_i} = \flatten{\msteptwo_i}$.
    Taking
      $\mstepB :=
       \lam{\var_1\hdots\var_n}{
         \altsrc{\rulewit}\,\mstepthreeB_1\hdots\mstepthreeB_q
       }$
    and
      $\msteptwoB :=
       \lam{\var_1\hdots\var_n}{
         \rulewit\,\msteptwoB_1\hdots\msteptwoB_q
       }$
    we have that $\judgCompat{\mstepB}{\msteptwoB}$.
    It is easy to note that $\flatten{\msteptwoB} = \flatten{\msteptwo}$.
    Moreover:
    \[
      \begin{array}{rlll}
        \flatten{\mstepB}
      & = &
        \flatten{(\lam{\var_1\hdots\var_n}{
          \altsrc{\rulewit}\,\mstepthreeB_1\hdots\mstepthreeB_q
        })}
      \\
      & = &
        \flatten{(\lam{\var_1\hdots\var_n}{
          \altsrc{\rulewit}\,\mstepthree_1\hdots\mstepthree_q
        })}
        & \text{by confluence of flattening~(\rprop{flat_confluent})}
      \\
      & = &
        \flatten{(\flattennoeta{(\lam{\var_1\hdots\var_n}{
          \altsrc{\rulewit}\,\mstepthree_1\hdots\mstepthree_q
        })})}
        & \text{by confluence of flattening~(\rprop{flat_confluent})}
      \\
      & = &
        \flatten{\mstep}
      \end{array}
    \]
  \end{enumerate}
\item
  {\bf Rule symbol,
    $\mstep = \lam{\var_1\hdots\var_n}{\rulewit\,\mstep_1\hdots\mstep_m}$.
  }
  Note that
  $\flattennoeta{(\altsrc{\mstep})} =
   \lam{\var_1\hdots\var_n}{
     \flattennoeta{(
       \altsrc{\rulewit}\,\altsrc{\mstep_1}\hdots
                          \altsrc{\mstep_m}
     )}
   }$.
  Since $\flattennoeta{(\altsrc{\msteptwo})} =
         \flattennoeta{(\altsrc{\mstep})}$,
  the head of $\msteptwo$ cannot be a variable.
  We consider two cases, depending on whether the head of $\msteptwo$
  is a constant or a rule symbol:
  \begin{enumerate}
  \item
    {\bf Constant,
      $\msteptwo = \lam{\var_1\hdots\var_p}{\cons\,\msteptwo_1\hdots\msteptwo_q}$.}
    The proof of this case proceeds symmetrically
    as for case~\ref{compatibilization_of_coinitial_multisteps__case_cons_rule},
    when the head of $\mstep$ is a constant
    and the head of $\msteptwo$ is a rule symbol.
  \item
    {\bf Rule symbol,
      $\msteptwo = \lam{\var_1\hdots\var_p}{\rulewittwo\,\msteptwo_1\hdots\msteptwo_q}$.
    }
    Recall that we assume that $\mstep$ and $\msteptwo$ are in
    $\etalong$-normal form. This implies that $n = p$.
    Then
    $\flattennoeta{(\altsrc{\msteptwo})} =
     \lam{\var_1\hdots\var_n}{
       \flattennoeta{(
         \altsrc{\rulewittwo}\,\altsrc{\msteptwo_1}\hdots\altsrc{\msteptwo_q}
       )}
     }$.
    Note that this implies that
    $\flattennoeta{(\altsrc{\rulewit}\,\altsrc{\mstep_1}\hdots\altsrc{\msteptwo_m})}
     =
     \flattennoeta{(\altsrc{\rulewittwo}\,\altsrc{\msteptwo_1}\hdots\altsrc{\msteptwo_q})}$.
    By orthogonality,
    this means that $\rulewit = \rulewittwo$
    and $m = q$, and moreover
    $\flattennoeta{(\altsrc{\mstep_i})} = \flattennoeta{(\altsrc{\msteptwo_i})}$
    for all $1 \leq i \leq m$.
    By \ih, for each $1 \leq i \leq m$,
    there exist multisteps such that
    $\judgCompat{\mstepB_i}{\msteptwoB_i}$,
    where $\flatten{\mstepB_i} = \flatten{\mstep_i}$
    and $\flatten{\msteptwoB_i} = \flatten{\msteptwo_i}$.
    Taking
    $\mstepB =
     \lam{\var_1\hdots\var_n}{\rulewit\,\mstepB_1\hdots\mstepB_m}$
    and
    $\msteptwoB =
     \lam{\var_1\hdots\var_n}{\rulewit\,\msteptwoB_1\hdots\msteptwoB_m}$
    it is then easy to check that
    $\judgCompat{\mstepB}{\msteptwoB}$,
    and moreover $\flatten{\mstepB} = \flatten{\mstep}$
    and $\flatten{\msteptwoB} = \flatten{\msteptwo}$.
  \end{enumerate}
\end{enumerate}
\end{proof}

\begin{lem}[Projection of a substitution]
\llem{projection_of_substitution}
Let $\judgProj{\mstep_1}{\msteptwo_1}{\mstepthree_1}$
and $\judgProj{\mstep_2}{\msteptwo_2}{\mstepthree_2}$.
Then $\judgProj{
        \mstep_1\subm{\var}{\mstep_2}
      }{
        \msteptwo_1\subm{\var}{\msteptwo_2}
      }{
        \mstepthree_1\subm{\var}{\mstepthree_2}
      }$
\end{lem}
\begin{proof}
By induction on the derivation
of $\judgProj{\mstep_1}{\msteptwo_1}{\mstepthree_1}$:
\begin{enumerate}
\item \indrulename{ProjVar}:
  Let $\judgProj{\vartwo}{\vartwo}{\vartwo}$.
  If $\vartwo \neq \var$, it is immediate.
  If $\vartwo = \var$,
  note that $\judgProj{\mstep_2}{\msteptwo_2}{\mstepthree_2}$ by hypothesis.
\item \indrulename{ProjCon}:
  Let $\judgProj{\cons}{\cons}{\cons}$.
  This case is immediate, as
  $\cons\subm{\var}{\mstep_2}
  = \cons\subm{\var}{\msteptwo_2}
  = \cons\subm{\var}{\mstepthree_2}
  = \cons$.
\item \indrulename{ProjRule}:
  Let $\judgProj{\rulewit}{\rulewit}{\rtgt{\rulewit}}$.
  This case is immediate, as $\rtgt{\rulewit}$ is closed,
  so
  $\rulewit\subm{\var}{\mstep_2}
  = \rulewit\subm{\var}{\msteptwo_2} = \rulewit$
  and
  $\rtgt{\rulewit}\subm{\var}{\mstepthree_2} = \rtgt{\rulewit}$.
\item \indrulename{ProjRuleL}:
  Let $\judgProj{\rulewit}{\rsrc{\rulewit}}{\rulewit}$.
  This case is immediate, as $\rsrc{\rulewit}$ is closed,
  so
  $\rulewit\subm{\var}{\mstep_2}
  = \rulewit\subm{\var}{\mstepthree_2} = \rulewit$
  and
  $\rsrc{\rulewit}\subm{\var}{\msteptwo_2} = \rsrc{\rulewit}$.
\item \indrulename{ProjRuleR}:
  Let $\judgProj{\rsrc{\rulewit}}{\rulewit}{\rtgt{\rulewit}}$.
  This case is immediate, as $\rsrc{\rulewit}$ and $\rtgt{\rulewit}$ are closed,
  so $\rsrc{\rulewit}\subm{\var}{\mstep_2} = \rsrc{\rulewit}$
  and $\rulewit\subm{\var}{\msteptwo_2} = \rulewit$
  and $\rtgt{\rulewit}\subm{\var}{\mstepthree_2} = \rtgt{\rulewit}$.
\item \indrulename{ProjAbs}:
  Let
  $\judgProj{
     \lam{\vartwo}{\mstep_1}
   }{
     \lam{\vartwo}{\msteptwo_1}
   }{
     \lam{\vartwo}{\mstepthree_1}
   }$
  be derived from
  $\judgProj{
     \mstep_1
   }{
     \msteptwo_1
   }{
     \mstepthree_1
   }$.
  By \ih
  $\judgProj{
     \mstep_1\subm{\var}{\mstep_2}
   }{
     \msteptwo_1\subm{\var}{\msteptwo_2}
   }{
     \mstepthree_1\subm{\var}{\mstepthree_2}
   }$,
  so applying the \indrulename{ProjAbs} rule
  $\judgProj{
     \lam{\vartwo}{\mstep_1\subm{\var}{\mstep_2}}
   }{
     \lam{\vartwo}{\msteptwo_1\subm{\var}{\msteptwo_2}}
   }{
     \lam{\vartwo}{\mstepthree_1\subm{\var}{\mstepthree_2}}
   }$.
\item \indrulename{ProjApp}:
  Let
  $\judgProj{
    \mstep_{11}\,\mstep_{12}
  }{
    \msteptwo_{11}\,\msteptwo_{12}
  }{
    \mstepthree_{11}\,\mstepthree_{12}
  }$
  be derived from
  $\judgProj{
    \mstep_{11}
  }{
    \msteptwo_{11}
  }{
    \mstepthree_{11}
  }$
  and
  $\judgProj{
    \mstep_{12}
  }{
    \msteptwo_{12}
  }{
    \mstepthree_{12}
  }$.
  Then by \ih
    $\judgProj{
      \mstep_{11}\subm{\var}{\mstep_2}
    }{
      \msteptwo_{11}\subm{\var}{\msteptwo_2}
    }{
      \mstepthree_{11}\subm{\var}{\mstepthree_2}
    }$
  and
    $\judgProj{
      \mstep_{12}\subm{\var}{\mstep_2}
    }{
      \msteptwo_{12}\subm{\var}{\msteptwo_2}
    }{
      \mstepthree_{12}\subm{\var}{\mstepthree_2}
    }$,
  so applying the \indrulename{ProjApp} rule
    $\judgProj{
      (\mstep_{11}\,\mstep_{12})\subm{\var}{\mstep_2}
    }{
      (\msteptwo_{11}\,\msteptwo_{12})\subm{\var}{\msteptwo_2}
    }{
      (\mstepthree_{11}\,\mstepthree_{12})\subm{\var}{\mstepthree_2}
    }$.
\end{enumerate}
\end{proof}

\begin{lem}[Compatibilization of projection]
\llem{compatibilization_of_projection}
Let $\judgProj{\mstep}{\msteptwo}{\mstepthree}$.
Then there exist multisteps
$\mstepB,\msteptwoB,\mstepthreeB$
such that:
\begin{enumerate}
\item
  $\mstep \tofs \mstepB$
  and
  $\msteptwo \tofs \msteptwoB$
  and
  $\mstepthree \tofs \mstepthreeB$
\item
  $\judgCompat{\mstepB}{\msteptwoB}$
\item
  $\judgProj{\mstepB}{\msteptwoB}{\mstepthreeB}$
\end{enumerate}
\end{lem}
\begin{proof}
If $\judgCompat{\mstep}{\msteptwo}$ holds, we are done.
By strong normalization of flattening~(\rprop{flat_sn})
it suffices to show that
if $\judgProj{\mstep}{\msteptwo}{\mstepthree}$
and $\judgCompat{\mstep}{\msteptwo}$ does {\em not} hold,
then there exist steps
$\mstep \tof \mstepB$
and
$\msteptwo \tof \msteptwoB$
and
$\mstepthree \tof \mstepthreeB$
such that $\judgProj{\mstepB}{\msteptwoB}{\mstepthreeB}$.
The proof proceeds by induction on the derivation of
$\judgProj{\mstep}{\msteptwo}{\mstepthree}$.
Note that rules
\indrulename{ProjVar}, \indrulename{ProjCon}, \indrulename{ProjRule},
\indrulename{ProjRuleL}, and \indrulename{ProjRuleR} cannot apply,
as then we would have that $\judgCompat{\mstep}{\msteptwo}$.
The remaining possibilities are:
\begin{enumerate}
\item
  \indrulename{ProjAbs}:
  Let
  $\judgProj{\lam{\var}{\mstep}}{\lam{\var}{\msteptwo}}{\lam{\var}{\mstepthree}}$
  be derived from
  $\judgProj{\mstep}{\msteptwo}{\mstepthree}$.
  By \ih there exist steps
  $\mstep \tof \mstepB$
  and
  $\msteptwo \tof \msteptwoB$
  and
  $\msteptwo \tof \mstepthreeB$
  such that
  $\judgProj{\mstepB}{\msteptwoB}{\mstepthreeB}$.
  Applying the \indrulename{ProjAbs} rule, we obtain that
  $\judgProj{\lam{\var}{\mstepB}}{\lam{\var}{\msteptwoB}}{\lam{\var}{\mstepthreeB}}$
  as required.
\item
  \indrulename{ProjApp}:
  Let
  $\judgProj{\mstep_1\,\mstep_2}{\msteptwo_1\,\msteptwo_2}{\mstepthree_1\,\mstepthree_2}$
  be derived from
  $\judgProj{\mstep_1}{\msteptwo_1}{\mstepthree_1}$
  and
  $\judgProj{\mstep_2}{\msteptwo_2}{\mstepthree_2}$.
  We consider three subcases:
  \begin{enumerate}
  \item
    {\bf If $\judgCompat{\mstep_1}{\msteptwo_1}$ does not hold.}
    Then by \ih there exist steps
    $\mstep_1 \tof \mstepB_1$
    and $\msteptwo_1 \tof \msteptwoB_1$
    and $\mstepthree_1 \tof \mstepthreeB_1$
    such that $\judgProj{\mstepB_1}{\msteptwoB_1}{\mstepthreeB_1}$.
    Then we have that
    $\mstep_1\,\mstep_2 \tof \mstepB_1\,\mstep_2$
    and $\msteptwo_1\,\msteptwo_2 \tof \msteptwoB_1\,\msteptwo_2$
    and $\mstepthree_1\,\mstepthree_2 \tof \mstepthreeB_1\,\mstepthree_2$
    and, applying the \indrulename{ProjApp} rule,
    $\judgProj{\mstepB_1\,\mstep_2}{\msteptwoB_1\,\msteptwo_2}{\mstepthreeB_1\,\mstepthree_2}$.
  \item
    {\bf If $\judgCompat{\mstep_1}{\msteptwo_1}$ holds
         and $\judgCompat{\mstep_2}{\msteptwo_2}$ does not hold.}
    Similar to the previous case.
  \item
    {\bf If both $\judgCompat{\mstep_1}{\msteptwo_1}$
         and $\judgCompat{\mstep_2}{\msteptwo_2}$ hold.}
    If $\mstep_1$ and $\msteptwo_1$ do not start with a $\lambda$-abstraction, 
    then it can be checked by case analysis on the rules
    defining the judgment $\judgCompat{\mstep_1}{\msteptwo_1}$
    that
    $\judgCompat{\mstep_1\,\mstep_2}{\msteptwo_1\,\msteptwo_2}$ holds,
    contradicting the hypothesis.
    For example, if
    $\judgCompat{\mstep_1}{\msteptwo_1}$ is derived using the
    \indrulename{CVar} rule,
    with the assumption that $\mstep_1$ does not start with
    a $\lambda$-abstraction, we would have that
    $\mstep_1 = \vartwo\,\mstep_{11}\hdots\mstep_{1n}$
    and
    $\msteptwo_1 = \vartwo\,\msteptwo_{11}\hdots\msteptwo_{1n}$
    with $\judgCompat{\mstep_{1i}}{\msteptwo_{1i}}$ for all $1 \leq i \leq n$.
    And from this we would have, using the \indrulename{CVar} rule,
    that
    $\judgCompat{
       \vartwo\,\mstep_{11}\hdots\mstep_{1n}\,\mstep_2
     }{
       \vartwo\,\msteptwo_{11}\hdots\msteptwo_{1n}\,\msteptwo_2
     }$.
    The argument is similar for the other rules besides \indrulename{CVar}.

    This means that $\mstep_1 = \lam{\var}{\mstep'_1}$
    and $\msteptwo_1 = \lam{\var}{\msteptwo'_1}$.
    Note, moreover, that the judgment
    $\judgProj{\mstep_1}{\msteptwo_1}{\mstepthree_1}$
    can only be derived by the \indrulename{ProjAbs} rule,
    so $\mstepthree_1 = \lam{\var}{\mstepthree'_1}$ 
    with $\judgProj{\mstep'_1}{\msteptwo'_1}{\mstepthree'_1}$.
    To conclude note that by taking
    $\mstepB := \mstep'_1\subm{\var}{\mstep_2}$
    and $\msteptwoB := \msteptwo'_1\subm{\var}{\msteptwo_2}$
    and $\mstepthreeB := \mstepthree'_1\subm{\var}{\mstepthree_2}$
    we have that
    $\mstep = (\lam{\var}{\mstep'_1})\,\mstep_2 \tofs \mstepB$
    and
    $\msteptwo = (\lam{\var}{\msteptwo'_1})\,\msteptwo_2 \tofs \msteptwoB$
    and
    $\mstepthree = (\lam{\var}{\mstepthree'_1})\,\mstepthree_2 \tofs \mstepthreeB$.
    Moreover,
    $\judgProj{\mstepB}{\msteptwoB}{\mstepthreeB}$
    is a consequence of \rlem{projection_of_substitution}.
  \end{enumerate}
\end{enumerate}
\end{proof}

\begin{prop}[Existence and uniqueness of projection]
\lprop{existence_uniqueness_projection}
Let $\mstep,\msteptwo$ be such that $\rsrc{\mstep} \termeq \rsrc{\msteptwo}$.
Then:
\begin{enumerate}
\item
  {\bf Existence.}
  There exist $\mstepB,\msteptwoB,\mstepthreeB$
  such that $\flatten{\mstepB} = \flatten{\mstep}$
  and $\flatten{\msteptwoB} = \flatten{\msteptwo}$
  and $\judgProj{\mstepB}{\msteptwoB}{\mstepthreeB}$.
\item
  {\bf Compatibility.}
  Furthermore, $\mstepB$ and $\msteptwoB$ can
  be chosen in such a way that $\judgCompat{\mstepB}{\msteptwoB}$.
\item
  {\bf Uniqueness.}
  If
  $\flatten{(\mstepB')} = \flatten{\mstep}$
  and
  $\flatten{(\msteptwoB')} = \flatten{\msteptwo}$
  and
  $\judgProj{\mstepB'}{\msteptwoB'}{\mstepthreeB'}$
  then $\flatten{(\mstepthreeB')} = \flatten{\mstepthree}$.
\end{enumerate}
\end{prop}
\begin{proof}
Note that $\fsrc{\mstep} = \fsrc{\msteptwo}$,
so by \rlem{compatibilization_of_coinitial_multisteps}
there exist multisteps $\mstepB,\msteptwoB$
such that $\judgCompat{\mstepB}{\msteptwoB}$
and moreover $\flatten{\mstepB} = \flatten{\mstep}$
and $\flatten{\msteptwoB} = \flatten{\msteptwo}$.
By \rlem{projection_for_compatible_multisteps}
this implies that there exists a multistep $\mstepthreeB$
such that $\judgProj{\mstepB}{\msteptwoB}{\mstepthreeB}$.
This proves items~1. and~2.

For item~3.,
suppose that
$\mstepB',\msteptwoB',\mstepthreeB'$ are such that
$\flatten{(\mstepB')} = \flatten{\mstep}$
and
$\flatten{(\msteptwoB')} = \flatten{\msteptwo}$
and
$\judgProj{\mstepB'}{\msteptwoB'}{\mstepthreeB'}$.
By \rlem{compatibilization_of_projection}
this implies that
there exist multisteps $\mstepB'',\msteptwoB'',\mstepthreeB''$
such that
$\mstepB' \tofs \mstepB''$
and
$\msteptwoB' \tofs \msteptwoB''$
and
$\mstepthreeB' \tofs \mstepthreeB''$,
and moreover
$\judgCompat{\mstepB''}{\msteptwoB''}$
and $\judgProj{\mstepB''}{\msteptwoB''}{\mstepthreeB''}$.
Note that
$\flatten{\mstepB'} = \flatten{\mstepB''}$
given that $\mstepB' \tofs \mstepB''$.
Similarly,
$\flatten{\msteptwoB'} = \flatten{\msteptwoB''}$
and
$\flatten{\mstepthreeB'} = \flatten{\mstepthreeB''}$.
Hence by \rlem{coherence_of_projection}
we may conclude that
$\flatten{\mstepthreeB} = \flatten{\mstepthreeB'}$,
as required.
\end{proof}

\begin{prop}[Properties of the projection operator]
\lprop{properties_of_projection}
\quad
\begin{enumerate}
\item $\mstep/\msteptwo = \flatten{(\mstep/\msteptwo)}$
\item $\mstep/\msteptwo = \flatten{\mstep}/\flatten{\msteptwo}$
\item $\mstep/\mstep = \ftgt{\mstep}$
      and, as particular cases:
      \[
        \refl{\tm}/\refl{\tm} = \flatten{\refl{\tm}}
        \HS
        \var/\var = \var
        \HS
        \cons/\cons = \cons
        \HS
        \rulewit/\rulewit = \ftgt{\rulewit}
      \]
\item $\mstep/\fsrc{\mstep} = \flatten{\mstep}$
      and, as a particular case,
      $\rulewit/\fsrc{\rulewit} = \rulewit$
\item $\fsrc{\mstep}/\mstep = \ftgt{\mstep}$
      and, as a particular case,
      $\fsrc{\rulewit}/\rulewit = \ftgt{\rulewit}$
\item $(\lam{\var}{\mstep})/(\lam{\var}{\msteptwo})
      = \flatten{(\lam{\var}{(\mstep/\msteptwo)})}$
\item $(\mstep_1\,\mstep_2)/(\msteptwo_1\,\msteptwo_2) =
       \flatten{((\mstep_1/\msteptwo_1)\,(\mstep_2/\msteptwo_2))}$
      provided that
      $\mstep_1/\msteptwo_1$ and $\mstep_2/\msteptwo_2$
      are defined.
\end{enumerate}
\end{prop}
\begin{proof}
We prove each item:
\begin{enumerate}
\item $\mstep/\msteptwo = \flatten{(\mstep/\msteptwo)}$:
  By definition
  there exist $\mstepB,\msteptwoB,\mstepthreeB$
  such that $\flatten{\mstepB} = \flatten{\mstep}$
  and $\flatten{\msteptwoB} = \flatten{\msteptwo}$
  and $\judgProj{\mstepB}{\msteptwoB}{\mstepthreeB}$
  where $\mstep/\msteptwo = \flatten{\mstepthreeB}$.
  Then
  $\mstep/\msteptwo
  = \flatten{\hat{\mstepthree}}
  = \flatten{(\flatten{\hat{\mstepthree}})}
  = \flatten{(\mstep/\msteptwo)}$.
\item $\mstep/\msteptwo = \flatten{\mstep}/\flatten{\msteptwo}$:
  By definition of $\mstep/\msteptwo$
  there exist $\mstepB,\msteptwoB,\mstepthreeB$
  such that $\flatten{\mstepB} = \flatten{\mstep}$
  and $\flatten{\msteptwoB} = \flatten{\msteptwo}$
  and $\judgProj{\mstepB}{\msteptwoB}{\mstepthreeB}$
  where $\mstep/\msteptwo = \flatten{\mstepthreeB}$.
  Then since $\flatten{\mstep} = \flatten{(\flatten{\mstep})}$
  and $\flatten{\msteptwo} = \flatten{(\flatten{\msteptwo})}$,
  the triple $\mstepB,\msteptwoB,\mstepthreeB$
  also fulfills the conditions for the definition of
  $\flatten{\mstep}/\flatten{\msteptwo}$.
  But~\rprop{existence_uniqueness_projection} ensures uniqueness,
  so
  $\mstep/\msteptwo
  = \flatten{\mstepthreeB}
  = \flatten{\mstep}/\flatten{\msteptwo}$.
\item $\mstep/\mstep = \ftgt{\mstep}$:
  It suffices to note that $\judgProj{\mstep}{\mstep}{\rtgt{\mstep}}$ 
  holds, as can be checked by induction on $\mstep$.
\item $\mstep/\fsrc{\mstep} = \flatten{\mstep}$:
  It suffices to note that
  $\judgProj{\mstep}{\rsrc{\mstep}}{\mstep}$,
  as can be checked by induction on $\mstep$.
\item $\fsrc{\mstep}/\mstep = \ftgt{\mstep}$:
  It suffices to note that
  $\judgProj{\rsrc{\mstep}}{\mstep}{\rtgt{\mstep}}$,
  as can be checked by induction on $\mstep$.
\item $(\lam{\var}{\mstep})/(\lam{\var}{\msteptwo})
      = \flatten{(\lam{\var}{(\mstep/\msteptwo)})}$:
  Observe that the left-hand side of the equation
  is defined if and only if the right-hand
  side is defined, given that
  $\rsrc{(\lam{\var}{\mstep})} \termeq \rsrc{(\lam{\var}{\msteptwo})}$
  if and only if $\rsrc{\mstep} \termeq \rsrc{\msteptwo}$,
  which is easy to check.

  By definition of $\mstep/\msteptwo$
  there exist $\mstepB,\msteptwoB,\mstepthreeB$
  such that $\flatten{\mstepB} = \flatten{\mstep}$
  and $\flatten{\msteptwoB} = \flatten{\msteptwo}$
  and $\judgProj{\mstepB}{\msteptwoB}{\mstepthreeB}$
  where $\mstep/\msteptwo = \flatten{\mstepthreeB}$.
  Then note, by confluence of flattening~(\rprop{flat_confluent}),
  that
  $\flatten{(\lam{\var}{\mstepB})}
   = \flatten{(\lam{\var}{\flatten{\mstepB}})}
   = \flatten{(\lam{\var}{\flatten{\mstep}})}
   = \flatten{(\lam{\var}{\mstep})}$
  and, similarly,
  $\flatten{(\lam{\var}{\msteptwoB})} = \flatten{(\lam{\var}{\msteptwo})}$.
  Moreover, by the \indrulename{ProjAbs} rule,
  $\judgProj{
     \lam{\var}{\mstepB}
   }{
     \lam{\var}{\msteptwoB}
   }{
     \lam{\var}{\mstepthreeB}
   }$.
  By uniqueness of projection~(\rprop{existence_uniqueness_projection})
  this means that
  $(\lam{\var}{\mstep})/(\lam{\var}{\msteptwo})
  = \flatten{(\lam{\var}{\mstepthreeB})}
  = \flatten{(\lam{\var}{\flatten{\mstepthreeB}})}
  = \flatten{(\lam{\var}{(\mstep/\msteptwo)})}$.
\item $(\mstep_1\,\mstep_2)/(\msteptwo_1\,\msteptwo_2) =
       \flatten{((\mstep_1/\msteptwo_1)\,(\mstep_2/\msteptwo_2))}$:
  Observe that, if the right-hand side of the equation is defined,
  then the left-hand side is also defined, given that
  if $\rsrc{\mstep_1} \termeq \rsrc{\msteptwo_1}$ 
  and $\rsrc{\mstep_2} \termeq \rsrc{\msteptwo_2}$
  then
  $\rsrc{(\mstep_1\,\mstep_2)} \termeq \rsrc{(\msteptwo_1\,\msteptwo_2)}$.

  Note that, by hypothesis, the right-hand side of the equation is defined.
  By definition of $\mstep_1/\msteptwo_1$
  there exist $\mstepB_1,\msteptwoB_1,\mstepthreeB_1$
  such that $\flatten{\mstepB_1} = \flatten{\mstep_1}$
  and $\flatten{\msteptwoB_1} = \flatten{\msteptwo_1}$
  and $\judgProj{\mstepB_1}{\msteptwoB_1}{\mstepthreeB_1}$
  where $\mstep_1/\msteptwo_1 = \flatten{\mstepthreeB_1}$.
  Similarly,
  by definition of $\mstep_2/\msteptwo_2$
  there exist $\mstepB_2,\msteptwoB_2,\mstepthreeB_2$
  such that $\flatten{\mstepB_2} = \flatten{\mstep_2}$
  and $\flatten{\msteptwoB_2} = \flatten{\msteptwo_2}$
  and $\judgProj{\mstepB_2}{\msteptwoB_2}{\mstepthreeB_2}$
  where $\mstep_2/\msteptwo_2 = \flatten{\mstepthreeB_2}$.

  Note, by confluence of flattening~(\rprop{flat_confluent}),
  $\flatten{(\mstepB_1\,\mstepB_2)}
  = \flatten{(\flatten{\mstepB_1}\,\flatten{\mstepB_2})}
  = \flatten{(\flatten{\mstep_1}\,\flatten{\mstep_2})}
  = \flatten{(\mstep_1\,\mstep_2)}$ and,
  similarly,
  $\flatten{(\msteptwoB_1\,\msteptwoB_2)}
  = \flatten{(\msteptwo_1\,\msteptwo_2)}$.
  Moreover, by the \indrulename{ProjApp} rule,
  $\judgProj{
     \mstepB_1\,\mstepB_2
   }{
     \msteptwoB_1\,\msteptwoB_2
   }{
     \mstepthreeB_1\,\mstepthreeB_2
   }$.
  By uniqueness of projection~\rprop{existence_uniqueness_projection}
  this means that
  $\mstep_1\,\mstep_2/\msteptwo_1\,\msteptwo_2
  = \flatten{(\mstepthreeB_1\,\mstepthreeB_2)}
  = \flatten{(\flatten{\mstepthreeB_1}\,\flatten{\mstepthreeB_2})}
  = \flatten{((\mstep_1/\msteptwo_1)\,(\mstep_2/\msteptwo_2))}$.
\end{enumerate}
\end{proof}

\begin{exa}
Let $\rulewit : \lam{\var}{\cons\,\var} \to \lam{\var}{\constwo\,\var}$.
Then:
\[
  \begin{array}{lll}
    (\lam{\var}{(\lam{\var}{\cons\,\var})\,\var})/(\lam{\var}{\rulewit\,\var})
  & = &
    \flatten{(
      \lam{\var}{
          ((\lam{\var}{\cons\,\var})\,\var)/(\rulewit\,\var)
      }
    )}
  \\
  & = &
    \flatten{(
      \lam{\var}{
        \flatten{(
          ((\lam{\var}{\cons\,\var})/\rulewit)
          (\var/\var)
        )}
      }
    )}
  \\
  & = &
    \flatten{(
      \lam{\var}{
        \flatten{(
          (\lam{\var}{\constwo\,\var})\,\var
        )}
      }
    )}
  \\
  & = &
    \flatten{(
      \lam{\var}{
        \constwo\,\var
      }
    )}
  \\
  & = &
    \constwo
  \end{array}
\]
\end{exa}

\begin{lem}[Cube lemma]
\llem{cube_lemma}
Given multisteps $\mstep,\msteptwo,\mstepthree$
such that $\rsrc{\mstep} \termeq \rsrc{\msteptwo} \termeq \rsrc{\mstepthree}$,
the following equality holds:
\[
  (\mstep/\msteptwo)/(\mstepthree/\msteptwo) =
  (\mstep/\mstepthree)/(\msteptwo/\mstepthree)
\]
\end{lem}
\begin{proof}
The proof proceeds by induction on the number of applications in the
$\tofnoeta,\etalong$-normal form of $\mstep$.
Note by~\rprop{properties_of_projection}
that, without loss of generality,
we may assume that $\mstep$, $\msteptwo$, and $\mstepthree$
are in $\tofnoeta,\etalong$-normal form.
The head of $\mstep$
may be a variable, a constant, or a rule symbol.
We consider three cases:
\begin{enumerate}
\item {\bf $\mstep$ headed by a variable,
           $\mstep = \lam{\vec{\var}}{\vartwo\,\mstep_1\hdots\mstep_n}$.}
  \label{cube_lemma__case_variable}
  Then since $\mstep$ and $\msteptwo$ are coinitial,
  the head of $\msteptwo$ must be $\vartwo$,
  and since we assume that the multisteps are in $\etalong$-normal form,
  $\msteptwo = \lam{\vec{\var}}{\vartwo\,\msteptwo_1\hdots\msteptwo_n}$.
  Similarly, since $\mstep$ and $\mstepthree$ are coinitial,
  $\mstepthree = \lam{\vec{\var}}{\vartwo\,\mstepthree_1\hdots\mstepthree_n}$.
  Then:
  \[
    \begin{array}{rlll}
      (\mstep/\msteptwo)/(\mstepthree/\msteptwo)
    & = &
      \flatten{
        (\lam{\vec{\var}}{
          \vartwo\,
          ((\mstep_1/\msteptwo_1)/(\mstepthree_1/\msteptwo_1))
          \hdots
          ((\mstep_n/\msteptwo_n)/(\mstepthree_n/\msteptwo_n))
        })
      }
      & \text{by~\rprop{properties_of_projection}}
    \\
    & = &
      \flatten{
        (\lam{\vec{\var}}{
          \vartwo\,
          ((\mstep_1/\mstepthree_1)/(\msteptwo_1/\mstepthree_1))
          \hdots
          ((\mstep_n/\mstepthree_n)/(\msteptwo_n/\mstepthree_n))
        })
      }
      & \text{by \ih}
    \\
    & = &
      (\mstep/\mstepthree)/(\msteptwo/\mstepthree)
    \end{array}
  \]
\item {\bf $\mstep$ headed by a constant,
           $\mstep = \lam{\vec{\var}}{\cons\,\mstep_1\hdots\mstep_n}$.}
  Then since $\mstep$ and $\msteptwo$ are coinitial,
  the head of $\msteptwo$ may be a constant or a rule symbol.
  We consider are two subcases:
  \begin{enumerate}
  \item {\bf $\msteptwo$ headed by a constant.}
    Then the head of $\msteptwo$ must be the constant $\cons$,
    and since the multisteps are in $\etalong$-normal form,
    $\msteptwo = \lam{\vec{\var}}{\cons\,\msteptwo_1\hdots\msteptwo_n}$.
    Note that, in turn, as $\mstep$ and $\mstepthree$ are coinitial,
    the head of $\mstepthree$ may be a constant or a rule symbol.
    So we consider two further subcases:
    \begin{enumerate}
    \item {\bf $\mstepthree$ headed by a constant.}
      Then the head of $\mstepthree$ must be the constant $\cons$,
      and since the multisteps are in $\etalong$-normal form,
      $\mstepthree = \lam{\vec{\var}}{\cons\,\mstepthree_1\hdots\mstepthree_n}$.
      The proof of this case is similar to
      case~\ref{cube_lemma__case_variable}, when the heads of all three
      multisteps are variables.
    \item {\bf $\mstepthree$ headed by a rule symbol.}
      \label{cube_lemma__case_cons_cons_rule}
      Then since the multisteps are in $\etalong$-normal form,
      $\mstepthree = \lam{\vec{\var}}{\rulewit\,\mstepthree_1\hdots\mstepthree_q}$.
      Since $\mstep$ and $\mstepthree$ are coinitial,
      by \rlem{coinitial_cons_rule}
      there exist multisteps $\mstep'_1,\hdots,\mstep'_q$
      in $\tofnoeta,\etalong$-normal form such that
      $\mstep =
       \flattennoeta{(\lam{\vec{\var}}{\rsrc{\rulewit}\,\mstep'_1\hdots\mstep'_q})}$
      where each $\mstep'_i$ has strictly less applications
      than $\mstep$,
      and such that $\mstep'_i$ and $\mstepthree_i$ are coinitial.
      Similarly, since
      $\msteptwo$ and $\mstepthree$ are coinitial,
      by \rlem{coinitial_cons_rule}
      there exist multisteps $\msteptwo'_1,\hdots,\msteptwo'_q$
      in $\tofnoeta,\etalong$-normal form such that
      $\msteptwo =
       \flattennoeta{(\lam{\vec{\var}}{\rsrc{\rulewit}\,\msteptwo'_1\hdots\msteptwo'_q})}$
      and such that,
      for each $1 \leq i \leq q$,
      $\msteptwo'_i$ and $\mstepthree_i$ are coinitial.

      Before proceeding, note that,
      using \rprop{properties_of_projection}, we have:
      \[
        \begin{array}{rlll}
          (\rsrc{\rulewit}/\rsrc{\rulewit})/(\rulewit/\rsrc{\rulewit})
        & = &
          (\fsrc{\rulewit}/\fsrc{\rulewit})/(\rulewit/\fsrc{\rulewit})
        \\
        & = &
          \fsrc{\rulewit}/\rulewit
        \\
        & = &
          \ftgt{\rulewit}
        \\
        & = &
          \ftgt{\rulewit}/\ftgt{\rulewit}
        \\
        & = &
          (\fsrc{\rulewit}/\rulewit)/(\fsrc{\rulewit}/\rulewit)
        \\
        & = &
          (\rsrc{\rulewit}/\rulewit)/(\rsrc{\rulewit}/\rulewit)
        \end{array}
      \]

      Then:
      \[
        \begin{array}{rlll}
        &&
          (\mstep/\msteptwo)/(\mstepthree/\msteptwo)
        \\
        & = &
          (
            (\lam{\vec{\var}}{\rsrc{\rulewit}\,\mstep'_1\hdots\mstep'_q})
            /
            (\lam{\vec{\var}}{\rsrc{\rulewit}\,\msteptwo'_1\hdots\msteptwo'_q})
          ) / (
            (\lam{\vec{\var}}{\rulewit\,\mstepthree_1\hdots\mstepthree_q})
            /
            (\lam{\vec{\var}}{\rsrc{\rulewit}\,\msteptwo'_1\hdots\msteptwo'_q})
          )
          \\&&\HS\text{by~\rprop{properties_of_projection}}
        \\
        & = &
          \flatten{
            (\lam{\vec{\var}}{
              ((\rsrc{\rulewit}/\rsrc{\rulewit})/(\rulewit/\rsrc{\rulewit}))\,
              ((\mstep'_1/\msteptwo'_1)/(\mstepthree_1/\msteptwo'_1))
              \hdots
              ((\mstep'_q/\msteptwo'_q)/(\mstepthree_q/\msteptwo'_q))
            })
          }
          \\&&\HS\text{by~\rprop{properties_of_projection}}
        \\
        & = &
          \flatten{
            (\lam{\vec{\var}}{
              ((\rsrc{\rulewit}/\rulewit)/(\rsrc{\rulewit}/\rulewit))\,
              ((\mstep'_1/\msteptwo'_1)/(\mstepthree_1/\msteptwo'_1))
              \hdots
              ((\mstep'_q/\msteptwo'_q)/(\mstepthree_q/\msteptwo'_q))
            })
          }
          \\&&\HS\text{by the preceding remark}
        \\
        & = &
          \flatten{
            (\lam{\vec{\var}}{
              ((\rsrc{\rulewit}/\rulewit)/(\rsrc{\rulewit}/\rulewit))\,
              ((\mstep'_1/\mstepthree_1)/(\msteptwo'_1/\mstepthree_1))
              \hdots
              ((\mstep'_q/\mstepthree_q)/(\msteptwo'_q/\mstepthree_q))
            })
          }
          \\&&\HS\text{by \ih}
        \\
        & = &
          (
            (\lam{\vec{\var}}{\rsrc{\rulewit}\,\mstep'_1\hdots\mstep'_q})/
            (\lam{\vec{\var}}{\rulewit\,\mstepthree_1\hdots\mstepthree_q})
          ) / (
            (\lam{\vec{\var}}{\rsrc{\rulewit}\,\msteptwo'_1\hdots\msteptwo'_q})/
            (\lam{\vec{\var}}{\rulewit\,\mstepthree_1\hdots\mstepthree_q})
          )
          \\&&\HS\text{by~\rprop{properties_of_projection}}
        \\
        & = &
          (\mstep/\mstepthree)/(\msteptwo/\mstepthree)
          \\&&\HS\text{by~\rprop{properties_of_projection}}
        \end{array}
      \]
    \end{enumerate}
  \item {\bf $\msteptwo$ headed by a rule symbol.}
    Then since the multisteps are in $\etalong$-normal form,
    $\msteptwo = \lam{\vec{\var}}{\rulewit\,\msteptwo_1\hdots\msteptwo_q}$
    Note that, in turn, as $\mstep$ and $\mstepthree$ are coinitial,
    the head of $\mstepthree$ may be a constant or a rule symbol.
    If the head of $\mstepthree$ is a constant, this case is symmetric
    to case~\ref{cube_lemma__case_cons_cons_rule},
    when $\msteptwo$ is headed by a constant
    and $\mstepthree$ by a rule symbol.
    If the head of $\mstepthree$ is a rule symbol,
    then since the multisteps are in $\etalong$-normal form,
    $\mstepthree = \lam{\vec{\var}}{\rulewit\,\mstepthree_1\hdots\mstepthree_q}$.
    Since $\mstep$ and $\msteptwo$ are coinitial,
    by \rlem{coinitial_cons_rule}
    there exist multisteps $\mstep'_1,\hdots,\mstep'_q$
    in $\tofnoeta,\etalong$-normal form such that
    $\mstep =
     \flattennoeta{(\lam{\vec{\var}}{\rsrc{\rulewit}\,\mstep'_1\hdots\mstep'_q})}$
    where each $\mstep'_i$ has strictly less applications
    than $\mstep$,
    and such that $\mstep'_i$ and $\msteptwo_i$ are coinitial.
    Then:
    \[
      \begin{array}{rlll}
      &&
        (\mstep/\msteptwo)/(\mstepthree/\msteptwo)
      \\
      & = &
        (
          (\lam{\vec{\var}}{\rsrc{\rulewit}\,\mstep'_1\hdots\mstep'_q})
          /
          (\lam{\vec{\var}}{\rulewit\,\msteptwo_1\hdots\msteptwo_q})
        ) / (
          (\lam{\vec{\var}}{\rulewit\,\mstepthree_1\hdots\mstepthree_q})
          /
          (\lam{\vec{\var}}{\rulewit\,\msteptwo_1\hdots\msteptwo_q})
        )
        \\&&\HS\text{by~\rprop{properties_of_projection}}
      \\
      & = &
        \flatten{
          (\lam{\vec{\var}}{
            ((\rsrc{\rulewit}/\rulewit)/(\rulewit/\rulewit))\,
            ((\mstep'_1/\msteptwo_1)/(\mstepthree_1/\msteptwo_1))
            \hdots
            ((\mstep'_q/\msteptwo_q)/(\mstepthree_q/\msteptwo_q))
          })
        }
        \\&&\HS\text{by~\rprop{properties_of_projection}}
      \\
      & = &
        \flatten{
          (\lam{\vec{\var}}{
            ((\rsrc{\rulewit}/\rulewit)/(\rulewit/\rulewit))\,
            ((\mstep'_1/\mstepthree_1)/(\msteptwo_1/\mstepthree_1))
            \hdots
            ((\mstep'_q/\mstepthree_q)/(\msteptwo_q/\mstepthree_q))
          })
        }
        \\&&\HS\text{by \ih}
      \\
      & = &
        (
          (\lam{\vec{\var}}{\rsrc{\rulewit}\,\mstep'_1\hdots\mstep'_q})/
          (\lam{\vec{\var}}{\rulewit\,\mstepthree_1\hdots\mstepthree_q})
        ) / (
          (\lam{\vec{\var}}{\rulewit\,\msteptwo_1\hdots\msteptwo_q})/
          (\lam{\vec{\var}}{\rulewit\,\mstepthree_1\hdots\mstepthree_q})
        )
        \\&&\HS\text{by~\rprop{properties_of_projection}}
      \\
      & = &
        (\mstep/\mstepthree)/(\msteptwo/\mstepthree)
        \\&&\HS\text{by~\rprop{properties_of_projection}}
      \end{array}
    \]
  \end{enumerate}
\item {\bf $\mstep$ headed by a rule symbol,
           $\mstep = \lam{\vec{\var}}{\rulewit\,\mstep_1\hdots\mstep_n}$.}
  Then since $\mstep$ and $\msteptwo$ are coinitial, the head
  of $\msteptwo$ may be a constant or a rule symbol.
  We consider two subcases:
  \begin{enumerate}
  \item {\bf $\msteptwo$ headed by a constant.}
    Then since the multisteps are in $\etalong$-normal form,
    $\msteptwo = \lam{\vec{\var}}{\cons\,\msteptwo_1\hdots\msteptwo_m}$.
    By \rlem{coinitial_cons_rule}
    there exist multisteps $\msteptwo'_1,\hdots,\msteptwo'_n$
    in $\tofnoeta,\etalong$-normal form such that
    $\msteptwo =
     \flattennoeta{(\lam{\vec{\var}}{\rsrc{\rulewit}\,\msteptwo'_1\hdots\msteptwo'_n})}$
    where $\mstep_i$ and $\msteptwo'_i$ are coinitial.
    Moreover, since $\mstep$ and $\mstepthree$ are coinitial,
    the head of $\mstepthree$ may be a constant or a rule symbol.
    We consider two further subcases:
    \begin{enumerate}
    \item {\bf $\mstepthree$ headed by a constant.}
      Then since the multisteps are in $\etalong$-normal form,
      $\mstepthree = \lam{\vec{\var}}{\cons\,\mstepthree_1\hdots\mstepthree_m}$.
      By \rlem{coinitial_cons_rule}
      there exist multisteps $\mstepthree'_1,\hdots,\mstepthree'_n$
      in $\tofnoeta,\etalong$-normal form such that
      $\mstepthree =
       \flattennoeta{(\lam{\vec{\var}}{\rsrc{\rulewit}\,\mstepthree'_1\hdots\mstepthree'_n})}$
      where $\mstep_i$ and $\mstepthree'_i$ are coinitial.
      Then the proof proceeds similarly as for case
      \ref{cube_lemma__case_cons_cons_rule}.
    \item {\bf $\mstepthree$ headed by a rule symbol.}
      \label{cube_lemma__case_rule_cons_rule}
      Then since the multisteps are in $\etalong$-normal form
      and by orthogonality,
      $\mstepthree = \lam{\vec{\var}}{\rulewit\,\mstepthree_1\hdots\mstepthree_n}$.
      Then the proof proceeds similarly as for case
      \ref{cube_lemma__case_cons_cons_rule},
      noting that, by~\rprop{properties_of_projection}:
      \[
        \begin{array}{rcll}
          (\rulewit/\rsrc{\rulewit})/(\rulewit/\rsrc{\rulewit})
        & = &
          \flatten{\rulewit}/\flatten{\rulewit}
        \\
        & = &
          \ftgt{\rulewit}
        \\
        & = &
          \ftgt{\rulewit}/\ftgt{\rulewit}
        \\
        & = &
          (\rulewit/\rulewit)/(\rsrc{\rulewit}/\rulewit)
        \end{array}
      \]
    \end{enumerate}
  \item {\bf $\msteptwo$ headed by a rule symbol.}
    Then since the multisteps are in $\etalong$-normal form,
    the head of $\mstepthree$ may be a constant or a rule symbol.
    If the head of $\mstepthree$ is a constant,
    this case is symmetric
    to case~\ref{cube_lemma__case_rule_cons_rule},
    when $\msteptwo$ is headed by a constant
    and $\mstepthree$ by a rule symbol.
    If the head of $\mstepthree$ is a rule symbol,
    then by orthogonality,
    $\mstepthree = \lam{\vec{\var}}{\rulewit\,\mstepthree_1\hdots\mstepthree_n}$.
    Then the proof proceeds similarly as
    for case~\ref{cube_lemma__case_cons_cons_rule}.
  \end{enumerate}
\end{enumerate}
\end{proof}

\subsection{Projection for rewrites}

\begin{lem}[Rewrite/rewrite generalizes rewrite/multistep and multistep/rewrite projections]
\llem{projrr_generalizes_projrm_and_projmr}
If $\mstep$ is a flat multistep
and $\redseq$ a coinitial flat rewrite
then:
\begin{enumerate}
\item $\mstep\projmr\redseq = \mstep\projrr\redseq$
\item $\redseq\projrm\mstep = \redseq\projrr\mstep$
\end{enumerate}
\end{lem}
\begin{proof}
Item~2. is immediate by definition of $\redseq\projrr\mstep$.
For item~1, we proceed by induction on $\redseq$:
\begin{enumerate}
\item
  {\bf Multistep, $\redseq = \msteptwo$.}
  Then
  $\mstep\projmr\msteptwo
   = \mstep/\msteptwo
   = \mstep\projrm\msteptwo
   = \mstep\projrr\msteptwo$.
\item
  {\bf Composition, $\redseq = \redseq_1\seq\redseq_2.$}
  Then:
  \[
    \begin{array}{rlll}
    \mstep\projmr(\redseq_1\seq\redseq_2)
    & = & (\mstep\projmr\redseq_1)\projmr\redseq_2 \\
    & = & (\mstep\projmr\redseq_1)\projrr\redseq_2 & \text{by \ih} \\
    & = & (\mstep\projrr\redseq_1)\projrr\redseq_2 & \text{by \ih} \\
    & = & \mstep\projrr(\redseq_1\seq\redseq_2) \\
    \end{array}
  \]
\end{enumerate}
\end{proof}

\begin{defi}[Size of a flat rewrite]
If $\redseq$ is a flat rewrite,
we write $\sz{\redseq}$ for the number of multisteps in $\redseq$.
More precisely:
\[
  \begin{array}{rll}
    \sz{\mstep}                & \eqdef & 1 \\
    \sz{\redseq\seq\redseqtwo} & \eqdef & \sz{\redseq} + \sz{\redseqtwo} \\
  \end{array}
\]
\end{defi}

\begin{lem}[Size of a projection]
\llem{size_of_a_projection}
\quad
\begin{enumerate}
\item $\sz{\mstep\projmr\redseq} = \sz{\mstep}$
\item $\sz{\redseq\projrm\mstep} = \sz{\redseq}$
\item $\sz{\redseq\projrr\redseqtwo} = \sz{\redseq}$
\end{enumerate}
\end{lem}
\begin{proof}
\quad
\begin{enumerate}
\item
  By induction on $\redseq$.
  If $\redseq = \msteptwo$,
  then
  $\sz{\mstep\projmr\msteptwo} = \sz{\mstep/\msteptwo} = 1 = \sz{\mstep}$.
  If $\redseq = \redseq_1\seq\redseq_2$,
  then by \ih we have that
  $\sz{\mstep\projmr(\redseq_1\seq\redseq_2)}
  = \sz{(\mstep\projmr\redseq_1)\projmr\redseq_2}
  = \sz{\mstep\projmr\redseq_1}
  = \sz{\mstep}$.
\item
  By induction on $\redseq$.
  If $\redseq = \msteptwo$,
  then
  $\sz{\msteptwo\projrm\mstep} = \sz{\msteptwo/\mstep} = 1 = \sz{\msteptwo}$.
  If $\redseq = \redseq_1\seq\redseq_2$,
  then by \ih we have that
  $\sz{(\redseq_1\seq\redseq_2)\projrm\mstep}
  = \sz{(\redseq_1\projrm\mstep)\seq(\redseq_2\projrm(\mstep\projmr\redseq_1))}
  = \sz{\redseq_1\projrm\mstep} + \sz{\redseq_2\projrm(\mstep\projmr\redseq_1)}
  = \sz{\redseq_1} + \sz{\redseq_2}
  = \sz{\redseq_1 \seq \redseq_2}$.
\item
  By induction on $\redseqtwo$.
  If $\redseqtwo = \mstep$,
  then by item~2.
  $\sz{\redseq\projrr\mstep}
  = \sz{\redseq\projrm\mstep}
  = \sz{\redseq}$.
  If $\redseqtwo = \redseqtwo_1\seq\redseqtwo_2$
  then by \ih we have that
  $\sz{\redseq\projrr(\redseqtwo_1\seq\redseqtwo_2)}
  = \sz{(\redseq\projrr\redseqtwo_1)\projrr\redseqtwo_2}
  = \sz{\redseq\projrr\redseqtwo_1}
  = \sz{\redseq}$.
\end{enumerate}
\end{proof}

\begin{lem}[Rewrite/rewrite projection of a sequence]
\llem{projrr_sequence}
If $(\redseq_1\seq\redseq_2)$ and $\redseqtwo$ are coinitial flat
rewrites, then:
\[
  (\redseq_1\seq\redseq_2)\projrr\redseqtwo =
  (\redseq_1\projrr\redseqtwo)\seq(\redseq_2\projrr(\redseqtwo\projrr\redseq_1))
\]
\end{lem}
\begin{proof}
We proceed by induction on $\sz{\redseq_1} + \sz{\redseq_2} + \sz{\redseqtwo}$.
We consider two cases, depending on whether
$\redseqtwo$ is a multistep or a composition:
\begin{enumerate}
\item {\bf Multistep, $\redseqtwo = \mstep$.}
  Then:
  \[
    \begin{array}{rlll}
      (\redseq_1\seq\redseq_2)\projrr\mstep
    & = &
      (\redseq_1\seq\redseq_2)\projrm\mstep
    \\
    & = &
      (\redseq_1\projrm\mstep)\seq(\redseq_2\projrm(\mstep\projmr\redseq_1))
    \\
    & = &
      (\redseq_1\projrr\mstep)\seq(\redseq_2\projrr(\mstep\projrr\redseq_1))
      & \text{by \rlem{projrr_generalizes_projrm_and_projmr}}
    \end{array}
  \]
\item {\bf Composition, $\redseqtwo = \redseqtwo_1\seq\redseqtwo_2$.}
  Then:
  \[
    \begin{array}{rlll}
    &&
      (\redseq_1\seq\redseq_2)\projrr(\redseqtwo_1\seq\redseqtwo_2)
    \\
    & = &
      ((\redseq_1\seq\redseq_2)\projrr\redseqtwo_1)\projrr\redseqtwo_2
    \\
    & = &
      (
        (\redseq_1\projrr\redseqtwo_1)
        \seq
        (\redseq_2\projrr(\redseqtwo_1\projrr\redseq_1))
      )
      \projrr\redseqtwo_2
      & \text{by \ih}
    \\
    & = &
      ((\redseq_1\projrr\redseqtwo_1)
       \projrr\redseqtwo_2)
      \seq
      ((\redseq_2\projrr(\redseqtwo_1\projrr\redseq_1))
       \projrr(\redseqtwo_2\projrr(\redseq_1\projrr\redseqtwo_1)))
      & \text{by \ih}
    \\
    & = &
      (\redseq_1\projrr(\redseqtwo_1\seq\redseqtwo_2))
      \seq
      (\redseq_2\projrr
       ((\redseqtwo_1\projrr\redseq_1)
        \seq
        (\redseqtwo_2\projrr(\redseq_1\projrr\redseqtwo_1))))
      & \text{by definition}
    \\
    & = &
      (\redseq_1\projrr(\redseqtwo_1\seq\redseqtwo_2))
      \seq
      (\redseq_2\projrr
       ((\redseqtwo_1\seq\redseqtwo_2)\projrr\redseq_1))
      & \text{by \ih}
    \end{array}
  \]
  To apply the \ih the first time,
  note that
  $\sz{\redseq_1} + \sz{\redseq_2} + \sz{\redseqtwo_1} <
   \sz{\redseq_1} + \sz{\redseq_2} + \sz{\redseqtwo_1\seq\redseqtwo_2}$.
  To apply the \ih the second time,
  note that by \rlem{size_of_a_projection}
  we have that
  $\sz{\redseq_1\projrr\redseqtwo_1} +
   \sz{\redseq_2\projrr(\redseqtwo_1\projrr\redseq_1)} +
   \sz{\redseqtwo_2}
  =
   \sz{\redseq_1} + \sz{\redseq_2} + \sz{\redseqtwo_2}
  <
   \sz{\redseq_1} + \sz{\redseq_2} + \sz{\redseqtwo_1\seq\redseqtwo_2}$.
  To apply the \ih the third time,
  note that
  $\sz{\redseqtwo_1} + \sz{\redseqtwo_2} + \sz{\redseq_1} <
   \sz{\redseq_1} + \sz{\redseq_2} + \sz{\redseqtwo_1\seq\redseqtwo_2}$.
\end{enumerate}
\end{proof}

\begin{convention}
From this point on, we overload $\redseq/\redseqtwo$
to stand for
$\redseq \projmr \redseqtwo$ (if $\redseq$ is a multistep),
$\redseq \projrm \redseqtwo$ (if $\redseqtwo$ is a multistep),
or $\redseq \projrr \redseqtwo$ (in the general case).
Note that \rlem{projrr_generalizes_projrm_and_projmr}
and \rlem{projrr_sequence} ensure that this overloading
is ``safe''.
\end{convention}
