# Supplementary material for: Reductions in Higher-Order Rewriting and Their Equivalence
Source: arXiv:2210.15654 source file (2023-08-15)
Supplement: Supplementary file 8 [file a08-standardization.tex]

\subsection{Standardization of rewrites}

\begin{lem}[Strong equivalence is a strong bisimulation]
\llem{streq_strong_bisimulation}
If $\redseq \streq \redseq' \tostd \redseqtwo$
then there exists $\redseqtwo'$ such that
$\redseq \tostd \redseqtwo' \streq \redseqtwo$.
\end{lem}
\begin{proof}
By induction on the derivation of $\redseq' \tostd \redseqtwo$.
\begin{enumerate}
\item \stdrule{Del}:
  Then
  $\redseq' = \refl{\tm}\seq\redseqtwo \tostd \redseqtwo$.
  Moreover we have that $\redseq \streq \redseq' = \refl{\tm}\seq\redseqtwo$.
  Hence $\redseq$ must be of the form $\redseq = \mstep\seq\redseqtwo'$
  with $\mstep \flateq \refl{\tm}$ and $\redseqtwo' \streq \redseqtwo$.
  By \rlem{characterization_of_empty_multisteps}
  note that $\mstep = \refl{\tm}$.
  To conclude, note that $\redseq = \mstep\seq\redseqtwo' \tostd \redseqtwo'$
  applying the \stdrule{Del} rule.
\item \stdrule{Pull}:
  Then
  $\redseq' =
   \mstep_1\seq\mstep_{23}\seq\redseqthree
   \tostd
   \mstep_{12}\seq\mstep_3\seq\redseqthree
   = \redseqtwo$
  where $\mstep_{12} \flateq \mstep_1\seq\mstep_2$
  and $\mstep_{23} \flateq \mstep_2\seq\mstep_3$
  and $\mstep_2$ is non-empty.
  Moreover, we have that
  $\redseq \streq \redseq' = \mstep_1\seq\mstep_{23}\seq\redseqthree$.
  Hence $\redseq$ must be of the form
  $\redseq = \msteptwo_1\seq\msteptwo_{23}\seq\redseqthree'$
  with $\msteptwo_1 \flateq \mstep_1$
  and $\msteptwo_{23} \flateq \mstep_{23}$
  and $\redseqthree' \streq \redseqthree$.
  Then we have that
  $\mstep_{12} \flateq \msteptwo_1\seq\mstep_2$
  and
  $\msteptwo_{23} \flateq \mstep_2\seq\mstep_3$,
  so we may apply the \stdrule{Pull} rule to conclude that
  $\redseq = \msteptwo_1\seq\msteptwo_{23}\seq\redseqthree'
   \tostd \mstep_{12}\seq\mstep_3\seq\redseqthree'$.
  To conclude, take $\redseqtwo' := \mstep_{12}\seq\mstep_3\seq\redseqthree'$
  and note that
  $\redseqtwo' = \mstep_{12}\seq\mstep_3\seq\redseqthree'
   \streq \mstep_{12}\seq\mstep_3\seq\redseqthree = \redseqtwo$
  given that $\redseqthree' \streq \redseqthree$.
\item
  \indrulename{StdCong}:
  Then $\redseq' = \mstep\seq\redseqthree'_1
        \tostd \mstep\seq\redseqthree_2 = \redseqtwo$
  is derived from $\redseqthree'_1 \tostd \redseqthree_2$.
  Moreover, we have that $\redseq \streq \redseq' = \mstep\seq\redseqthree'_1$.
  Hence $\redseq$ must be of the form $\redseq = \mstep'\seq\redseqthree_1$
  where $\mstep' \flateq \mstep$ and $\redseqthree_1 \streq \redseqthree'_1$.
  Note that $\redseqthree_1 \streq \redseqthree'_1 \tostd \redseqthree_2$
  so by \ih there exists $\redseqthree'_2$ such that
  $\redseqthree_1 \tostd \redseqthree'_2 \streq \redseqthree_2$.
  Applying the \indrulename{StdCong} rule,
  we obtain that
  $\redseq = \mstep'\seq\redseqthree_1 \tostd \mstep'\seq\redseqthree'_2$.
  To conclude, take $\redseqtwo' := \mstep'\seq\redseqthree'_2$
  and note that
  $\redseqtwo' = \mstep'\seq\redseqthree'_2
   \streq \mstep\seq\redseqthree_2 = \redseqtwo$
  given that
  $\mstep' \flateq \mstep$ and $\redseqthree'_2 \streq \redseqthree_2$.
\end{enumerate}
\end{proof}

\begin{lem}[Local confluence of standardization, up to strong equivalence]
\llem{standardization_wcr}
If $\redseq_1 \tostd \redseq_2$ 
and $\redseq_1 \tostd \redseq_3$ 
then there exists $\redseq_4$ such
that $\redseq_2 \tostd^*\streq \redseq_4$
and $\redseq_3 \tostd^*\streq \redseq_4$.
\end{lem}
\begin{proof}
It suffices to study the cases in which the rewriting rules
\stdrule{Del} and \stdrule{Pull} overlap.
The overlapping of \stdrule{Del} with itself is trivial.
The remaining cases are:
\begin{enumerate}
\item \stdrule{Del}/\stdrule{Pull} (1):
  Consider a \stdrule{Pull} step
  $\mstep_1\seq\mstep_{23}\seq\redseq
   \tostd
   \mstep_{12}\seq\mstep_3\seq\redseq$
  where
  $\mstep_{12} \flateq \mstep_1\seq\mstep_2$
  and
  $\mstep_{23} \flateq \mstep_2\seq\mstep_3$,
  with $\mstep_2$ a non-empty multistep.
  Moreover, suppose that there is a \stdrule{Del} step at
  the root, that is, that $\mstep_1$ is empty
  and
  $\mstep_1\seq\mstep_{23}\seq\redseq
   \tostd
   \mstep_{23}\seq\redseq$.
  We consider two subcases, depending on whether
  $\mstep_3$ is empty or not.
  \begin{enumerate}
  \item
    {\bf If $\mstep_3$ is empty.}
    Note that $\mstep_{23} \flateq \mstep_2$.
    Moreover, since $\mstep_1$ and $\mstep_3$ are empty:
    \[
      \mstep_{23}
      \flateq \mstep_2\seq\mstep_3
      \flateq \mstep_2
      \flateq \mstep_1\seq\mstep_2
      \flateq \mstep_{12}
    \]
    Then:
    \[
      \xymatrix{
        \mstep_1\seq\mstep_{23}\seq\redseq
        \ar[r]^-{\stdrule{Pull}}
        \ar[d]_-{\stdrule{Del}}
      &
        \mstep_{12}\seq\mstep_3\seq\redseq
        \ar@{.>}[d]^-{\stdrule{Del}}
      \\
        \mstep_{23}\seq\redseq
        \ar@{.}[r]_-{\streq}
      &
        \mstep_{12}\seq\redseq
      }
    \]
  \item
    {\bf If $\mstep_3$ is non-empty.}
    Then, note that since $\mstep_1$ is empty we have that:
    \[
      \mstep_{23}
      \flateq \mstep_2\seq\mstep_3
      \flateq \mstep_1\seq\mstep_2\seq\mstep_3
      \flateq \mstep_{12}\seq\mstep_3
    \]
    and
    $\mstep_{3} \flateq \mstep_3\seq\ftgt{\mstep_3}$
    where $\mstep_3$ is non-empty,
    applying the \indrulename{Pull} rule we have that
    $\mstep_{12}\seq\mstep_3 \tostd \mstep_{23}\seq\ftgt{\mstep_3}\seq\redseq$.
    Hence:
    \[
      \xymatrix{
        \mstep_1\seq\mstep_{23}\seq\redseq
        \ar[r]^-{\stdrule{Pull}}
        \ar[d]_-{\stdrule{Del}}
      &
        \mstep_{12}\seq\mstep_3\seq\redseq
        \ar@{.>}[d]^-{\stdrule{Pull}}
      \\
        \mstep_{23}\seq\redseq
      &
        \mstep_{23}\seq\ftgt{\mstep_3}\seq\redseq
        \ar@{.>}[l]^-{\stdrule{Del}}
      }
    \]
  \end{enumerate}
\item \stdrule{Del}/\stdrule{Pull} (2):
  Consider a \stdrule{Pull} step
  $\mstep_1\seq\mstep_{23}\seq\redseq
   \tostd
   \mstep_{12}\seq\mstep_3\seq\redseq$
  where
  $\mstep_{12} \flateq \mstep_1\seq\mstep_2$
  and
  $\mstep_{23} \flateq \mstep_2\seq\mstep_3$,
  with $\mstep_2$ a non-empty multistep.
  Moreover, suppose that there is a \stdrule{Del} step
  erasing $\mstep_{23}$,
  that is, that $\mstep_{23}$ is empty
  and $\mstep_1\seq\mstep_{23}\seq\redseq \tostd \mstep_1\seq\redseq$.
  We claim that this case is impossible.
  Indeed, we know that $\mstep_{23}$ is empty
  and $\mstep_{23} \flateq \mstep_2\seq\mstep_3$.
  By \rlem{characterization_of_empty_multisteps}, this implies that
  $\mstep_2$ is empty, a contradiction.
\item \stdrule{Pull}/\stdrule{Pull} (1):
  Consider a \stdrule{Pull} step
  $\mstep_1\seq\mstep_{23}\seq\redseq
   \tostd
   \mstep_{12}\seq\mstep_3\seq\redseq$
  where $\mstep_{12} \flateq \mstep_1\seq\mstep_2$
  and $\mstep_{23} \flateq \mstep_2\seq\mstep_3$
  with $\mstep_2$ a non-empty multistep.
  Moreover, suppose that there is
  another \stdrule{Pull} step at the root,
  of the form
  $\mstep_1\seq\mstep_{23}\seq\redseq
   \tostd
   \mstep'_{12}\seq\mstep'_3\seq\redseq$
  where $\mstep'_{12} \flateq \mstep_1\seq\mstep'_2$
  and $\mstep_{23} \flateq \mstep'_2\seq\mstep'_3$,
  with $\mstep'_2$ a non-empty multistep.

  Note that
  $\mstep_2\seq\mstep_3
   \flateq \mstep_{23}
   \flateq \mstep'_2\seq\mstep'_3$.
  Hence:
  \[
    \begin{array}{rlll}
      \mstep_3
    & \flateq &
      \ftgt{\mstep_2} \seq \mstep_3
      & \text{by \rthm{soundness_completeness_flateq} using \permeqRule{IdL}}
    \\
    & \flateq &
      \ftgt{\mstep_2} \seq (\mstep_3/\ftgt{\mstep_2})
      & \text{by \rprop{properties_of_projection}}
    \\
    & \flateq &
      (\mstep_2/\mstep_2)\seq(\mstep_3/(\mstep_2/\mstep_2))
      & \text{by \rlem{self_erasure} and \rprop{congruence_flateq_projection}}
    \\
    & = &
      (\mstep_2\seq\mstep_3)/\mstep_2
      & \text{by definition of projection}
    \\
    & \flateq &
      (\mstep'_2\seq\mstep'_3)/\mstep_2
      & \text{by \rprop{congruence_flateq_projection}}
    \\
    & = &
      (\mstep'_2/\mstep_2)\seq(\mstep'_3/(\mstep_2/\mstep'_2))
      & \text{by definition of projection}
    \end{array}
  \]
  Symmetrically,
  $\mstep'_3 \flateq
   (\mstep_2/\mstep'_2)\seq(\mstep_3/(\mstep'_2/\mstep_2))$.

  The proof proceeds by case analysis, depending on whether
  $\mstep'_2/\mstep_2$ and $\mstep_2/\mstep'_2$
  are empty or not. There are four subcases:
  \begin{enumerate} 
  \item {\bf $\mstep'_2/\mstep_2$ and $\mstep_2/\mstep'_2$ are both empty.}
    Then, note that $\mstep_{12} \flateq \mstep'_{12}$
    and $\mstep_3 \flateq \mstep'_3$. Indeed:
    \[
      \begin{array}{rlll}
        \mstep_{12}
      & \flateq &
        \mstep_1\seq\mstep_2
      \\
      & \flateq &
        \mstep_1\seq\mstep'_2
        & \text{by \rthm{projection_equivalence}}
      \\
      & \flateq &
        \mstep'_{12}
      \end{array}
    \]
    \[
      \begin{array}{rlll}
        \mstep_3
      & \flateq &
        (\mstep'_2/\mstep_2)\seq(\mstep'_3/(\mstep_2/\mstep'_2))
        & \text{as shown above}
      \\
      & = &
        \ftgt{\mstep_2}\seq(\mstep'_3/\ftgt{(\mstep'_2)})
        & \text{as $\mstep_2/\mstep'_2$ is empty}
      \\
      & \permeq &
        \mstep'_3
        & \text{by \rthm{soundness_completeness_flateq},
                   \rprop{properties_of_projection}}
      \end{array}
    \]
    Hence the diagram may be closed as follows:
    \[
      \xymatrix{
        \mstep_1\seq\mstep_{23}\seq\redseq
        \ar[r]^-{\stdrule{Pull}}
        \ar[d]_-{\stdrule{Pull}}
      &
        \mstep_{12}\seq\mstep_3\seq\redseq
      \\
        \mstep'_{12}\seq\mstep'_3\seq\redseq
        \ar@{.}[ru]_-{\streq}
      }
    \]
  \item {\bf $\mstep'_2/\mstep_2$ is empty and
             $\mstep_2/\mstep'_2$ is non-empty.}
    Let $\msteptwo := \mstep_{12}$.
    First note that:
    \[
      \begin{array}{rcll}
        \msteptwo
      & = &
        \mstep_{12}
      \\
      & \flateq &
        \mstep_1\seq\mstep_2
      \\
      & \flateq &
        \mstep_1\seq\mstep_2\seq\ftgt{\mstep_2}
        & \text{by \rprop{properties_of_projection}}
      \\
      & \flateq &
        \mstep_1\seq\mstep_2\seq(\mstep'_2/\mstep_2)
        & \text{as $\mstep'_2/\mstep_2$ is empty}
      \\
      & \flateq &
        \mstep_1\seq\mstep'_2\seq(\mstep_2/\mstep'_2)
        & \text{by \rlem{multistep_permutation}}
      \\
      & \flateq &
        \mstep'_{12}\seq(\mstep_2/\mstep'_2)
      \end{array}
    \]
    Moreover, note that:
    \[
      \begin{array}{rlll}
        \mstep'_3
      & \flateq &
        (\mstep_2/\mstep'_2)\seq(\mstep_3/(\mstep'_2/\mstep_2))
        & \text{as shown above}
      \\
      & \flateq &
        (\mstep_2/\mstep'_2)\seq(\mstep_3/\ftgt{\mstep_2})
        & \text{as $\mstep'_2/\mstep_2$ is empty}
      \\
      & \flateq &
        (\mstep_2/\mstep'_2)\seq\mstep_3
        & \text{by \rprop{properties_of_projection}}
      \end{array}
    \]
    Since $\mstep_2/\mstep'_2$ is non-empty,
    this means that there is a \stdrule{Pull} step
    $\mstep'_{12}\seq\mstep'_3\seq\redseq
     \tostd
     \msteptwo\seq\mstep_3\seq\redseq$.

    Then:
    \[
      \xymatrix{
        \mstep_1\seq\mstep_{23}\seq\redseq
        \ar[r]^-{\stdrule{Pull}}
        \ar[d]_-{\stdrule{Pull}}
      &
        \mstep_{12}\seq\mstep_3\seq\redseq
        \ar@{.}[d]^-{\streq}
      \\
        \mstep'_{12}\seq\mstep'_3\seq\redseq
        \ar@{.>}[r]_-{\stdrule{Pull}}
      &
        \msteptwo\seq\mstep_3\seq\redseq
      }
    \]
  \item {\bf $\mstep'_2/\mstep_2$ is non-empty and
             $\mstep_2/\mstep'_2$ is empty.}
    Symmetric to the previous case.
  \item {\bf $\mstep'_2/\mstep_2$ and $\mstep_2/\mstep'_2$ are non-empty.}
    Let $\msteptwo := \mstep_{12} \join \mstep'_{12}$
    and $\mstepthree := \mstep'_3/(\mstep_2/\mstep'_2)$.
    We claim that there are two \stdrule{Pull} steps,
    $\mstep_{12}\seq\mstep_3\seq\redseq
     \tostd \msteptwo\seq\mstepthree\seq\redseq$
    and
    $\mstep'_{12}\seq\mstep'_3\seq\redseq
     \tostd \msteptwo\seq\mstepthree\seq\redseq$.
    We prove these two facts:
    \begin{enumerate}
    \item
      First, note that:
      \[
        \begin{array}{rlll}
          \msteptwo
        & = &
          \mstep_{12} \join \mstep'_{12}
        \\
        & \flateq &
          \mstep_{12} \seq (\mstep'_{12}/\mstep_{12})
          & \text{by \rlem{basic_property_of_join}}
        \\
        & \flateq &
          \mstep_{12} \seq ((\mstep_1\seq\mstep'_2)/(\mstep_1\seq\mstep_2))
          & \text{by \rprop{congruence_flateq_projection}}
        \\
        & \flateq &
          \mstep_{12}\seq(\mstep'_2/\mstep_2)
          & \text{by \rlem{self_erasure} and \rprop{properties_of_projection}}
        \end{array}
      \]
      and recall that, as shown above
      $
        \mstep_3
        \flateq (\mstep'_2/\mstep_2)\seq(\mstep'_3/(\mstep_2/\mstep'_2))
        = (\mstep'_2/\mstep_2)\seq\mstepthree
      $.
      Hence, since $\mstep'_2/\mstep_2$ is non-empty,
      there is a \stdrule{Pull} step
      $\mstep_{12}\seq\mstep_3\seq\redseq
       \tostd \msteptwo\seq\mstepthree\seq\redseq$.
    \item
      Second, note that:
      \[
        \begin{array}{rlll}
          \msteptwo
        & \flateq &
          \mstep_{12}\seq(\mstep'_2/\mstep_2)
          & \text{as already shown}
        \\
        & \flateq &
          \mstep_1\seq\mstep_2\seq(\mstep'_2/\mstep_2)
        \\
        & \flateq &
          \mstep_1\seq\mstep'_2\seq(\mstep_2/\mstep'_2)
          & \text{by \rlem{multistep_permutation}}
        \\
        & \flateq &
          \mstep'_{12}\seq(\mstep_2/\mstep'_2)
        \end{array}
      \]
      Moreover, recall that, as shown above,
      $\mstep'_3 \flateq (\mstep_2/\mstep'_2)\seq(\mstep_3/(\mstep'_2/\mstep_2))$.
      Therefore:
      \[
        \begin{array}{rlll}
          (\mstep_2/\mstep'_2)/\mstep'_3
        & = &
          (\mstep_2/\mstep'_2)/((\mstep_2/\mstep'_2)\seq
                                (\mstep_3/(\mstep'_2/\mstep_2)))
          & \text{by \rprop{congruence_flateq_projection}}
        \\
        & = &
          ((\mstep_2/\mstep'_2)/(\mstep_2/\mstep'_2))/
          (\mstep_3/(\mstep'_2/\mstep_2))
          & \text{by definition of projection}
        \\
        & \flateq &
          \ftgt{(\mstep'_2)}/
          (\mstep_3/(\mstep'_2/\mstep_2))
          & \text{by \rlem{self_erasure} and \rprop{congruence_flateq_projection}}
        \\
        & \flateq &
          \ftgt{(\mstep_3/(\mstep'_2/\mstep_2))}
          & \text{by \rprop{properties_of_projection}}
        \end{array}
      \]
      This means that $(\mstep_2/\mstep'_2)/\mstep'_3$ is equivalent
      to an empty multistep.
      By \rlem{characterization_of_empty_multisteps}, this implies
      that $(\mstep_2/\mstep'_2)/\mstep'_3$ itself has to be empty.
      As a consequence, we have that:
      \[
        \begin{array}{rlll}
          \mstep'_3
        & \flateq &
          \mstep'_3\seq((\mstep_2/\mstep'_2)/\mstep'_3)
          & \text{as $(\mstep_2/\mstep'_2)/\mstep'_3$ is empty}
        \\
        & \flateq &
          (\mstep_2/\mstep'_2)\seq(\mstep'_3/(\mstep_2/\mstep'_2))
          & \text{by \rlem{multistep_permutation}}
        \\
        & = &
          (\mstep_2/\mstep'_2)\seq\mstepthree
        \end{array}
      \]
      Since $\mstep_2/\mstep'_2$ is non-empty,
      there is a \stdrule{Pull} step
      $\mstep'_{12}\seq\mstep'_3\seq\redseq
       \tostd
       \msteptwo\seq\mstepthree\seq\redseq$.
    \end{enumerate}
    With these two \stdrule{Pull} steps, we are able to close the diagram:
    \[
      \xymatrix{
        \mstep_1\seq\mstep_{23}\seq\redseq
        \ar[r]^-{\stdrule{Pull}}
        \ar[d]_-{\stdrule{Pull}}
      &
        \mstep_{12}\seq\mstep_3\seq\redseq
        \ar@{.>}[d]^-{\stdrule{Pull}}
      \\
        \mstep'_{12}\seq\mstep'_3\seq\redseq
        \ar@{.>}[r]_-{\stdrule{Pull}}
      &
        \msteptwo\seq\mstepthree\seq\redseq
      }
    \]
  \end{enumerate} 
\item \stdrule{Pull}/\stdrule{Pull} (2):
  Consider two overlapping \stdrule{Pull} steps,
  the first one of the form
  \[
    \mstep_1\seq\mstep_{23}\seq\mstep_{45}\seq\redseq
    \tostd
    \mstep_{12}\seq\mstep_3\seq\mstep_{45}\seq\redseq
  \]
  where
  $\mstep_{12} \flateq \mstep_1\seq\mstep_2$
  and
  $\mstep_{23} \flateq \mstep_2\seq\mstep_3$
  with $\mstep_2$ a non-empty multistep,
  and the second one of the form
  \[
    \mstep_1\seq\mstep_{23}\seq\mstep_{45}\seq\redseq
    \tostd
    \mstep_1\seq\mstep_{234}\seq\mstep_5\seq\redseq
  \]
  where $\mstep_{234} \flateq \mstep_{23}\seq\mstep_4$ 
  and $\mstep_{45} \flateq \mstep_4\seq\mstep_5$,
  with $\mstep_4$ a non-empty multistep.

  Let $\mstep_{34} := \mstep_{234}/\mstep_2$.
  We claim that there are two \stdrule{Pull} steps,
  $\mstep_{12}\seq\mstep_3\seq\mstep_{45} \tostd
   \mstep_{12}\seq\mstep_{34}\seq\mstep_5$
  and
  $\mstep_1\seq\mstep_{234}\seq\mstep_5 \tostd
   \mstep_{12}\seq\mstep_{34}\seq\mstep_5$.

  \begin{enumerate}
  \item
    First, note that:
    \[
      \begin{array}{rlll}
        \mstep_{34}
      & = &
        \mstep_{234}/\mstep_2
      \\
      & \flateq &
        ((\mstep_2 \seq \mstep_3)\seq\mstep_4)/\mstep_2
        & \text{by \rprop{congruence_flateq_projection}}
      \\
      & \flateq &
        \mstep_3\seq\mstep_4
        & \text{by \rlem{self_erasure} and \rprop{properties_of_projection}}
      \end{array}
    \]
    and recall that
    $\mstep_{45} \flateq \mstep_4\seq\mstep_5$.
    Since $\mstep_4$ is non-empty,
    this gives us a \stdrule{Pull} step
    $\mstep_{12}\seq\mstep_3\seq\mstep_{45} \tostd
     \mstep_{12}\seq\mstep_{34}\seq\mstep_5$.
  \item
    Second, recall that $\mstep_{12} \flateq \mstep_1\seq\mstep_2$
    and note that:
    \[
      \begin{array}{rlll}
        \mstep_{234}
      & \flateq &
        \mstep_{23}\seq\mstep_4
      \\
      & \flateq &
        \mstep_2\seq\mstep_3\seq\mstep_4
      \\
      & \flateq &
        \mstep_2\seq\mstep_{34}
        & \text{as $\mstep_{34} \flateq \mstep_3\seq\mstep_4$,
                as shown above}
      \end{array}
    \]
    Since $\mstep_2$ is non-empty,
    this gives us a \stdrule{Pull} step
    $\mstep_1\seq\mstep_{234}\seq\mstep_5 \tostd
     \mstep_{12}\seq\mstep_{34}\seq\mstep_5$.
  \end{enumerate}
  With these two \stdrule{Pull} steps, we are able to close the diagram:
  \[
    \xymatrix{
      \mstep_1\seq\mstep_{23}\seq\mstep_{45}\seq\redseq
      \ar[r]^-{\stdrule{Pull}}
      \ar[d]_-{\stdrule{Pull}}
    &
      \mstep_{12}\seq\mstep_3\seq\mstep_{45}\seq\redseq
      \ar@{.>}[d]^-{\stdrule{Pull}}
    \\
      \mstep_1\seq\mstep_{234}\seq\mstep_5\seq\redseq
      \ar@{.>}[r]_-{\stdrule{Pull}}
    &
      \mstep_{12}\seq\mstep_{34}\seq\mstep_5\seq\redseq
    }
  \]
\end{enumerate}
\end{proof}

\begin{lem}[Standardization decresases the Sekar--Ramakrishnan measure]
\llem{standardization_decreases_SR}
The following hold:
\begin{enumerate}
\item If $\redseq \streq \redseqtwo$ then $\SR{\redseq} = \SR{\redseqtwo}$.
\item If $\redseq \tostd \redseqtwo$ then $\SR{\redseq} \srgt \SR{\redseqtwo}$.
\end{enumerate}
\end{lem}
\begin{proof}
Item~1. is straightforward,
noting that if $\mstep \flateq \msteptwo$
then $\depth{\mstep} = \depth{\msteptwo}$,
given that a rewrite $\redseq$ is an unfolding of $\mstep$
if and only if it is an unfolding of $\msteptwo$,

For item~2, we show that \stdrule{Del} and \stdrule{Pull} steps strictly
decrease the Sekar--Ramakrishnan measure:
\begin{enumerate}
\item \stdrule{Del}:
  Then the step is of the form:
  \[
    \redseq =
    \mstepthree_1\seq\hdots\seq\mstepthree_{i}\seq
    \mstep
    \seq\mstepthree_{i+1}\seq\hdots\seq\mstepthree_n\seq\refl{\tm}
    \tostd
    \mstepthree_1\seq\hdots\seq\mstepthree_{i}\seq
    \mstepthree_{i+1}\seq\hdots\seq\mstepthree_n\seq\refl{\tm}
    = \redseqtwo
  \]
  where $\mstep$ is empty.
  Then:
  \[
    \begin{array}{rllll}
      \SR{\redseq}
    & = &
      (n + 1,
        \depth{\mstepthree_n}, \hdots, \depth{\mstepthree_{i+1}},
        \depth{\mstep},
        \depth{\mstepthree_i}, \hdots, \depth{\mstepthree_1})
    \\
    & \srgt &
      (n,
        \depth{\mstepthree_n}, \hdots, \depth{\mstepthree_{i+1}},
        \depth{\mstepthree_i}, \hdots, \depth{\mstepthree_1})
      & = & \SR{\redseqtwo}
    \end{array}
  \]
  given that $n + 1 > n$.
\item \stdrule{Pull}:
  Then the step is of the form:
  \[
    \redseq =
    \mstepthree_1\seq\hdots\seq\mstepthree_{i}\seq
    \mstep_1\seq\mstep_{23}
    \seq\mstepthree_{i+1}\seq\hdots\seq\mstepthree_n\seq\refl{\tm}
    \tostd
    \mstepthree_1\seq\hdots\seq\mstepthree_{i}\seq
    \mstep_{12}\seq\mstep_{3}
    \mstepthree_{i+1}\seq\hdots\seq\mstepthree_n\seq\refl{\tm}
    = \redseqtwo
  \]
  where $\mstep_{12} \flateq \mstep_1\seq\mstep_2$
  and $\mstep_{23} \flateq \mstep_2\seq\mstep_3$
  and $\mstep_2$ is non-empty.
  Then note that:
  \[
    \begin{array}{rll}
      \SR{\redseq}
    & = &
      (n + 2,
        \depth{\mstepthree_n}, \hdots, \depth{\mstepthree_{i+1}},
        \depth{\mstep_{23}},\depth{\mstep_1},
        \depth{\mstepthree_i}, \hdots, \depth{\mstepthree_1})
    \\
      \SR{\redseqtwo}
    & = &
      (n + 2,
        \depth{\mstepthree_n}, \hdots, \depth{\mstepthree_{i+1}},
        \depth{\mstep_3},\depth{\mstep_{12}},
        \depth{\mstepthree_i}, \hdots, \depth{\mstepthree_1})
    \end{array}
  \]
  In order to show that $\SR{\redseq} \srgt \SR{\redseqtwo}$,
  it suffices to show that
  \[
    (\depth{\mstep_{23}},\depth{\mstep_1}) >
    (\depth{\mstep_3},\depth{\mstep_{12}})
  \]
  according to the usual lexicographic order.
  In fact, we argue that a stronger property holds,
  namely $\depth{\mstep_{23}} > \depth{\mstep_3}$.

  To establish this inequality, it suffices to show that
  if $\redseqthree$ is an unfolding of $\mstep_3$
  then there is an unfolding $\redseqthree'$ of $\mstep_{23}$
  which is longer than $\redseqthree$,
  that is, $\len{\redseqthree'} \geq \len{\redseqthree}$.
  Indeed, suppose that
  $\mstep_3 \flateq \redseqthree$ where
  $\redseqthree$ contains no empty steps (other than the last one).
  Then
  $\mstep_{23} \flateq \mstep_2\seq\mstep_3
   \flateq \mstep_2\seq\redseqthree$.
  To conclude, take $\redseqthree' := \mstep_2\seq\redseqthree$.
  Note that
  $\len{\redseqthree'} = 1 + \len{\redseqthree}$
  and that $\redseqthree'$ is an unfolding of $\mstep_{23}$,
  because $\mstep_2$ is non-empty.
\end{enumerate}
\end{proof}

\begin{cor}[Standardization is SN and CR up to strong equivalence]
\lcoro{standardization_sn_cr}
\quad
\begin{enumerate}
\item
  $\tostd$ is SN.
\item
  $\tostd$ is CR up to $\streq$,
  that is,
  if $\redseq \tostd^* \redseq_1$
  and $\redseq \tostd^* \redseq_2$
  then there exist $\redseq'_1,\redseq'_2$
  such that $\redseq_1 \tostd^* \redseq'_1$
  and $\redseq_2 \tostd^* \redseq'_2$
  and $\redseq'_1 \streq \redseq'_2$.
\end{enumerate}
\end{cor}
\begin{proof}
First, the fact that $\tostd$ decreases the
Sekar--Ramakrishnan measure~(\rlem{standardization_decreases_SR})
entails that $\tostd$ is SN.

Second, let us write $[\redseq]$ for the $\streq$-equivalence class of a
sequential rewrite $\redseq$
and consider the rewriting system
whose objects are $\streq$-equivalence classes
of sequential rewrites, with the rewriting relation $\tostd'$
that results from
lifting $\tostd$ to equivalence classes,
\ie $[\redseq] \tostd' [\redseqtwo]$
if and only if $\redseq \tostd\streq \redseqtwo$.
The fact that $\streq$ is a strong bisimulation
with respect to $\tostd$~(\rlem{streq_strong_bisimulation})
implies that $\tostd'$ is well-defined.
Also, note that~\rlem{standardization_decreases_SR}
guarantees that the Sekar--Ramakrishnan measure is
well-defined over $\streq$-equivalence classes,
and that $\tostd'$ decreases the measure,
which implies that $\tostd'$ is also SN.
Moreover, from \rlem{standardization_wcr}
we know that $\tostd$ is locally confluent up to $\streq$,
which means that $\tostd'$ is locally confluent.
Thus, by Newman's Lemma, $\tostd'$ is confluent.

Finally, note that $\tostd'$ being confluent
implies that $\tostd$ is confluent up to $\streq$,
using the fact that
$\streq$ is a strong bisimulation with respect to $\tostd$
(\rlem{streq_strong_bisimulation}).
\end{proof}

\begin{thm}[Standardization theorem]
Let $\redseq,\redseqtwo$ be sequential rewrites.
The following are equivalent:
\begin{enumerate}
\item $\redseq \flateq \redseqtwo$
\item $\redseq \mathrel{(\tostd \cup \tostd^{-1} \cup \streq)^*} \redseqtwo$
\item There exist rewrites $\redseq',\redseqtwo'$ in $\tostd$-normal form
      such that $\redseq \tostd^* \redseq'$
      and $\redseqtwo \tostd^* \redseqtwo'$
      and $\redseq' \streq \redseqtwo'$.
\end{enumerate}
\end{thm}
\begin{proof}
\quad
\begin{itemize}
\item $(1 \implies 2)$
  Since $\redseq,\redseqtwo$ are sequential,
  we may work implicitly up to the \flateqRule{Assoc} rule.
  Doing this, it can be shown
  that the equivalence $\redseq \flateq \redseqtwo$
  must be derived from the reflexive, symmetric, and transitive closure
  of following variant of the \flateqRule{Perm} rule:
  \[
    \begin{array}{rllr}
        \mstepthree_1\seq\hdots\mstepthree_i\seq
        \mstep
        \seq\mstepthree_{i+1}\seq\hdots\mstepthree_n\seq\refl{\tm}
      & \flateq &
        \mstepthree_1\seq\hdots\mstepthree_i\seq
        \flatten{\mstep_1}\seq\flatten{\mstep_2}
        \seq\mstepthree_{i+1}\seq\hdots\mstepthree_n\seq\refl{\tm}
      &
        \flateqRule{Perm'}
      \\
      &&&\text{if $\judgSplit{\mstep}{\mstep_1}{\mstep_2}$}
    \end{array}
  \]
  It suffices to show that if $\redseq \flateq \redseqtwo$
  is derived using the \flateqRule{Perm'} axiom,
  then $\redseq \mathrel{(\tostd \cup \tostd^{-1} \cup \streq)^*} \redseqtwo$.

  Indeed, let $\judgSplit{\mstep}{\mstep_1}{\mstep_2}$.
  We consider two cases, depending on whether $\flatten{\mstep_2}$
  is empty or not:
  \begin{enumerate}
  \item {\bf If $\flatten{\mstep_2}$ is empty.}
    Then $\flatten{\mstep_2} = \ftgt{\mstep_2} = \fsrc{\mstep_1}$.
    Note that
    $\mstep \flateq \flatten{\mstep_1}\seq\flatten{\mstep_2}
            \flateq \flatten{\mstep_1}$
    holds by \rthm{soundness_completeness_flateq}, using \permeqRule{IdR}.
    Then:
    \[
      \begin{array}{rlll}
        \mstepthree_1\seq\hdots\mstepthree_i\seq
        \mstep
        \seq\mstepthree_{i+1}\seq\hdots\mstepthree_n\seq\refl{\tm}
      & \streq &
        \mstepthree_1\seq\hdots\mstepthree_i\seq
        \flatten{\mstep_1}
        \seq\mstepthree_{i+1}\seq\hdots\mstepthree_n\seq\refl{\tm}
      \\
      & \tostdinv &
        \mstepthree_1\seq\hdots\mstepthree_i\seq
        \flatten{\mstep_1}\seq\flatten{\mstep_2}
        \seq\mstepthree_{i+1}\seq\hdots\mstepthree_n\seq\refl{\tm}
        & \text{by \stdrule{Del}}
      \end{array}
    \]
  \item {\bf If $\flatten{\mstep_2}$ is non-empty.}
    On one hand,
    $\mstep \flateq \flatten{\mstep_1}\seq\flatten{\mstep_2}$.
    Moreover,
    $\flatten{\mstep_2} \flateq \flatten{\mstep_2}\seq\ftgt{\mstep_2}$
    holds by \rthm{soundness_completeness_flateq}, using \permeqRule{IdR}.
    Then:
    \[
      \begin{array}{rlll}
        \mstepthree_1\seq\hdots\mstepthree_i\seq
        \mstep
        \seq\mstepthree_{i+1}\seq\hdots\mstepthree_n\seq\refl{\tm}
      & \tostdinv &
        \mstepthree_1\seq\hdots\mstepthree_i\seq
        \mstep\seq\ftgt{\mstep_2}
        \seq\mstepthree_{i+1}\seq\hdots\mstepthree_n\seq\refl{\tm}
        & \text{by \stdrule{Del}}
      \\
      & \tostdinv &
        \mstepthree_1\seq\hdots\mstepthree_i\seq
        \flatten{\mstep_1}\seq\flatten{\mstep_2}
        \seq\mstepthree_{i+1}\seq\hdots\mstepthree_n\seq\refl{\tm}
        & \text{by \stdrule{Pull}}
      \end{array}
    \]
  \end{enumerate}
\item $(2 \implies 3)$
  This is an immediate consequence of~\rcoro{standardization_sn_cr}.
\item $(3 \implies 1)$
  It suffices to show that $\tostd \ \subseteq\ \flateq$
  and $\streq\ \subseteq\ \flateq$:
  \begin{enumerate}
  \item $\tostd\ \subseteq\ \flateq$:
    Let $\redseq \tostd \redseqtwo$ and
    let us check that $\redseq \flateq \redseqtwo$.
    We consider two subcases, depending on whether
    $\redseq \tostd \redseqtwo$ is derived from
    \stdrule{Del} or \stdrule{Pull}:
    \begin{enumerate}
    \item \stdrule{Del}:
      The step is of the form:
      \[
        \mstepthree_1\seq\hdots\seq\mstepthree_i\seq
        \mstep
        \seq\mstepthree_{i+1}\seq\hdots\seq\mstepthree_n\seq\refl{\tm}
        \tostd
        \mstepthree_1\seq\hdots\seq\mstepthree_i
        \seq\mstepthree_{i+1}\seq\hdots\seq\mstepthree_n\seq\refl{\tm}
      \]
      where $\mstep$ is empty.
      Then note that $\mstep = \ftgt{\mstep} = \fsrc{\mstepthree_{i+1}}$,
      so by \rthm{soundness_completeness_flateq}, using \permeqRule{IdR}, 
      we have that:
      \[
        \mstepthree_1\seq\hdots\seq\mstepthree_i\seq
        \mstep
        \seq\mstepthree_{i+1}\seq\hdots\seq\mstepthree_n\seq\refl{\tm}
        \flateq
        \mstepthree_1\seq\hdots\seq\mstepthree_i
        \seq\mstepthree_{i+1}\seq\hdots\seq\mstepthree_n\seq\refl{\tm}
      \]
    \item \stdrule{Pull}:
      The step is of the form:
      \[
        \mstepthree_1\seq\hdots\seq\mstepthree_i\seq
        \mstep_1\seq\mstep_{23}
        \seq\mstepthree_{i+1}\seq\hdots\seq\mstepthree_n\seq\refl{\tm}
        \tostd
        \mstepthree_1\seq\hdots\seq\mstepthree_i\seq
        \mstep_{12}\seq\mstep_3
        \seq\mstepthree_{i+1}\seq\hdots\seq\mstepthree_n\seq\refl{\tm}
      \]
      where $\mstep_{12} \flateq \mstep_1\seq\mstep_2$
      and $\mstep_{23} \flateq \mstep_2\seq\mstep_3$
      and $\mstep_2$ is non-empty.
      Then:
      \[
        \begin{array}{rll}
        &&
          \mstepthree_1\seq\hdots\seq\mstepthree_i\seq
          \mstep_1\seq\mstep_{23}
          \seq\mstepthree_{i+1}\seq\hdots\seq\mstepthree_n\seq\refl{\tm}
        \\
        & \flateq &
          \mstepthree_1\seq\hdots\seq\mstepthree_i\seq
          \mstep_1\seq\mstep_2\seq\mstep_3
          \seq\mstepthree_{i+1}\seq\hdots\seq\mstepthree_n\seq\refl{\tm}
        \\
        & \flateq &
          \mstepthree_1\seq\hdots\seq\mstepthree_i\seq
          \mstep_{12}\seq\mstep_3
          \seq\mstepthree_{i+1}\seq\hdots\seq\mstepthree_n\seq\refl{\tm}
        \\
        \end{array}
      \]
    \end{enumerate}
  \item $\streq\ \subseteq\ \flateq$:
    Suppose that $\redseq \streq \redseqtwo$.
    This means that
    $\redseq = \mstep_1\seq\hdots\seq\mstep_n\seq\refl{\tm}$
    and $\redseqtwo = \msteptwo_1\seq\hdots\seq\msteptwo_n\seq\refl{\tm}$
    where $\mstep_i \flateq \msteptwo_i$ for all $1 \leq i \leq n$.
    Then it is immediate to conclude that
    $\mstep_1\seq\hdots\seq\mstep_n\seq\refl{\tm}
    \flateq \msteptwo_1\seq\hdots\seq\msteptwo_n\seq\refl{\tm}$.
  \end{enumerate}
\end{itemize}
\end{proof}
